# Supplementary material for: Design-based theory for covariate adjustment in generalized pairwise comparisons
Source: arXiv:2602.18383 ancillary file (2026-10-10)
Supplement: Supplementary file 1 [file Supplementary_Materials.pdf]

# Supplementary Materials of
# "Design-based inference for generalized causal effects in randomized experiments"

Xinyuan Chen* and Fan Li†

Section S1 presents some basic lemmas
Section S2 proves the consistency and asymptotic normality of estimators using individual pairs.
Section S3 proves the consistency and asymptotic normality of estimators using per-unit pair averages.
Section S4 proves the results of the PIM estimators for estimating the net benefit.
Section S5 proves the results of the variance estimators.
Section S6 proves the lemmas.
Section S7 provides the additional simulation results.

## S1 Some basic lemmas

**Lemma S1.** *Let* $\mathbb{1}_i(a) = \mathbb{1}(A_i = a)$ *for* $a = 0, 1$. *Suppose the deterministic sequence* $\{b_{i,j}, 1 \leq i \neq j \leq N\}$ *satisfies* $\{N(N-1)\}^{-1}\sum_{i\neq j} b_{i,j}^2 = O(1)$. *Define*

$$\bar{b} = \frac{1}{N(N-1)}\sum_{i\neq j}\mathbb{1}_i(a)\mathbb{1}_j(1-a)b_{i,j}.$$

*Under Condition 1 in the main article and complete randomization,* $\mathbb{V}\mathrm{ar}(\bar{b}) = O(N^{-1})$.

**Lemma S2.** *Under Condition 1 in the main article and complete randomization,* $\bar{b} - \mathbb{E}(\bar{b}) = O_{\mathbb{P}}(N^{-1/2})$, *where* $\bar{b}$ *is defined in Lemma S1.*

Lemma S2 is an implication from Chebyshev's inequality. The proof is thus omitted.

**Lemma S3.** *If* $\boldsymbol{\Lambda} = \boldsymbol{O}_{\mathbb{P}}(\varrho)$ *with* $\varrho = o(1)$, *and* $\boldsymbol{\Gamma}$ *converges in probability to a finite and invertible matrix, then* $(\boldsymbol{\Gamma}+\boldsymbol{\Lambda})^{-1} - \boldsymbol{\Gamma}^{-1} = \boldsymbol{O}_{\mathbb{P}}(\varrho)$.

Lemma S3 is Lemma A5 of Su and Ding (2021). The proof is thus omitted.

**Lemma S4.** *Recall that* $\mathcal{S}(a, 1-a) = \{(i,j) | A_i = a, A_j = 1-a, 1 \leq i \neq j \leq N\}$ *and*

$$\bar{b}_{\mathcal{S}(a,1-a)} = \frac{1}{|\mathcal{S}(a,1-a)|}\sum_{i\neq j}\mathbb{1}_i(a)\mathbb{1}_j(1-a)b_{i,j},$$

*where* $b_{i,j}$ *satisfies the condition in Lemma S1. Under Condition 1 in the main article and complete randomization,*

$$\bar{b}_{\mathcal{S}(a,1-a)} - \frac{1}{N(N-1)}\sum_{i\neq j} b_{i,j} = O_{\mathbb{P}}\left(\frac{1}{N^{1/2}}\right).$$

Lemma S4 is implied by Lemmas S2 and S3 and Slutsky's Theorem. The proof is thus omitted.

*xchen@math.msstate.edu
†fan.f.li@yale.edu

**Lemma S5.** *Suppose* $\{b_{i,j}, i, j = 1, \dots, N\}$ *satisfies* $\{N(N-1)\}^{-1} \sum_{i \neq j} b_{i,j}^4 = o(N)$. *Define*

$$\overline{b^2} = \frac{1}{N(N-1)} \sum_{i \neq j} \mathbb{1}_i(a) \mathbb{1}_j(1-a) b_{i,j}^2.$$

*Under Condition 1 in the main article and complete randomization,* $\mathbb{V}\text{ar}(\overline{b^2}) = o(1)$.

**Lemma S6.** *Consider two deterministic sequences* $\{b_{i,j}, 1 \leq i \neq j \leq N\}$ *and* $\{c_{i,j}, 1 \leq i \neq j \leq N\}$. *Define* $\overline{b}_{i,\cdot}^A = N_{1-A_i}^{-1} \sum_{j:A_j = 1-A_i} b_{i,j}$ *and* $\overline{c}_{i,\cdot}^A = N_{1-A_i}^{-1} \sum_{j:A_j=1-A_i} c_{i,j}$. *Also,* $\overline{b}_{i,\cdot} = (N-1)^{-1} \sum_{j:j\neq i} b_{i,j}$ *and* $\overline{c}_{i,\cdot} = (N-1)^{-1} \sum_{j:j \neq i} c_{i,j}$. *The sequences satisfy* $N^{-1} \sum_{i=1}^N \overline{b}_{i,\cdot}^4 = O(1)$, $\max_{1 \leq i \leq N} \overline{b}_{i,\cdot}^2 = o(1)$, $N^{-1} \sum_{i=1}^N \overline{c}_{i,\cdot}^4 = O(1)$, $\max_{1 \leq i \leq N} \overline{c}_{i,\cdot}^2 = o(N)$. *Then, under Condition 1 in the main article and complete randomization,*

$$\mathbb{V}\text{ar}\left\{ \frac{1}{N_a} \sum_{i=1}^N \mathbb{1}_i(a) \overline{b}_{i,\cdot}^A \overline{c}_{i,\cdot}^A \right\} = O_{\mathbb{P}}\left(\frac{1}{N}\right).$$

# S2 Estimators using individual pairs

Recall that

$$\begin{aligned}
\overline{\epsilon}_{i,\cdot}(a, 1-a) &= \frac{1}{N-1} \sum_{j:j \neq i} \epsilon_{i,j}(a, 1-a) \\
&= \frac{1}{N-1} \sum_{j:j\neq i} \left\{ W_{i,j}(a,1-a) - \overline{W}(a,1-a) \right\} = \overline{W}_{i,\cdot}(a,1-a) - \overline{W}(a,1-a), \\
\overline{\epsilon}_{\cdot,i}(a, 1-a) &= \frac{1}{N-1} \sum_{j:j \neq i} \epsilon_{j,i}(a, 1-a) \\
&= \frac{1}{N-1} \sum_{j:j\neq i} \left\{ W_{j,i}(a,1-a) - \overline{W}(a,1-a) \right\} = \overline{W}_{\cdot,i}(a,1-a) - \overline{W}(a,1-a).
\end{aligned}$$

Also, for $\mathcal{E}_i(a, 1-a) \equiv (\mathcal{E}_{i,\cdot}(a,1-a), \mathcal{E}_{\cdot,i}(a,1-a))$ for $i = 1 \dots, N$, where $\sum_{i=1}^N \mathcal{E}_{i,\cdot} = 0$ and $\sum_{i=1}^N \mathcal{E}_{\cdot,i} = 0$, we have

$$\begin{aligned}
V_c\{\mathcal{E}_i(a,1-a)\} &= \frac{1}{\pi_a N} \sum_{i=1}^N \mathcal{E}_{i,\cdot}(a,1-a)^2 + \frac{1}{\pi_{1-a} N} \sum_{i=1}^N \mathcal{E}_{\cdot,i}(a,1-a)^2, \\
V\{\mathcal{E}_i(a,1-a)\} &= V_c\{\mathcal{E}_i(a,1-a)\} - \frac{1}{N} \sum_{i=1}^N \left\{ \mathcal{E}_{i,\cdot}(a,1-a) + \mathcal{E}_{\cdot,i}(a,1-a) \right\}^2,
\end{aligned}$$

with

$$\begin{aligned}
CV(\mathcal{E}_i) = & \frac{1}{\pi_a N} \sum_{i=1}^N \mathcal{E}_{i,\cdot}(a,1-a) \mathcal{E}_{\cdot,i}(1-a,a) + \frac{1}{\pi_{1-a} N} \sum_{i=1}^N \mathcal{E}_{i,\cdot}(1-a,a) \mathcal{E}_{\cdot,i}(a,1-a) \\
& - \frac{1}{N} \sum_{i=1}^N \left\{ \mathcal{E}_{i,\cdot}(a,1-a) + \mathcal{E}_{\cdot,i}(a,1-a) \right\} \left\{ \mathcal{E}_{i,\cdot}(1-a,a) + \mathcal{E}_{\cdot,i}(1-a,a) \right\}.
\end{aligned}$$

**Lemma S7.** *For* $a = 0, 1$, $\widehat{\lambda}_{\text{I}}(a, 1-a)$ *has expectation* $\mathbb{E}\{\widehat{\lambda}_{\text{I}}(a,1-a)\} = \lambda_{\text{I}}(a,1-a)$ *and variance* $\mathbb{V}\text{ar}\{\widehat{\lambda}_{\text{I}}(a,1-a)\} = N^{-1} V\{\overline{\epsilon}_i(a,1-a)\} + O(N^{-2})$, *with* $\mathbb{C}\text{ov}\{\widehat{\lambda}_{\text{I}}(a,1-a), \widehat{\lambda}_{\text{I}}(1-a,a)\} = N^{-1} CV(\overline{\epsilon}_i) + O(N^{-2})$.

**Condition S1.** $\{N(N-1)\}^{-1} \sum_{i \neq j} W_{i,j}(a,1-a)^4 = o(N)$ *for* $a = 0, 1$.

*Proof of Theorem 1.* We first prove the consistency. By Lemma S7 and Condition 1 in the main article and Condition S1,

$$
\begin{aligned}
&\mathbb{E}\left\{\widehat{\lambda}_{\mathrm{I}}(a,1-a)\right\} = \lambda(a,1-a),\\
&\mathbb{V}\mathrm{ar}\left\{\widehat{\lambda}_{\mathrm{I}}(a,1-a)\right\} = O\left(\frac{1}{N^2}\right)\sum_{i=1}^{N}\left\{\overline{W}_{i,\cdot}(a,1-a)-\overline{W}(a,1-a)\right\}^2 + O\left(\frac{1}{N^2}\right)\\
&\leq O\left(\frac{1}{N^2}\right)\sum_{i\neq j} W_{i,j}(a,1-a)^2 = o(1).
\end{aligned}
$$

Chebyshev's inequality yields $\widehat{\lambda}_{\mathrm{I}}(a,1-a)=\lambda(a,1-a)+o_{\mathbb{P}}(1)$. We then prove the asymptotic normality. From the proof of Lemma S7, we have

$$
\begin{pmatrix}\widehat{\lambda}_{\mathrm{I}}(a,1-a)-\lambda(a,1-a)\\ \widehat{\lambda}_{\mathrm{I}}(1-a,a)-\lambda(1-a,a)\end{pmatrix} = \frac{1}{N}\sum_{i=1}^{N}\begin{pmatrix}\frac{1}{\pi_a}\overline{\epsilon}_{i,\cdot}(a,1-a)\mathbb{1}_i(a)+\frac{1}{\pi_{1-a}}\overline{\epsilon}_{\cdot,i}(a,1-a)\mathbb{1}_i(1-a)\\ \frac{1}{\pi_{1-a}}\overline{\epsilon}_{i,\cdot}(1-a,a)\mathbb{1}_i(1-a)+\frac{1}{\pi_a}\overline{\epsilon}_{\cdot,i}(1-a,a)\mathbb{1}_i(a)\end{pmatrix} + \boldsymbol{O}_{\mathbb{P}}\left(\frac{1}{N}\right).
$$

Because,

$$
\begin{aligned}
|\overline{\epsilon}_{i,\cdot}(a,1-a)| &= |\overline{W}_{i,\cdot}(a,1-a)-\overline{W}(a,1-a)| \leq |\overline{W}_{i,\cdot}(a,1-a)| + |\overline{W}(a,1-a)|\\
&= |\overline{W}_{i,\cdot}(a,1-a)| + \left|\frac{1}{N}\sum_{i=1}^{N}\overline{W}_{i,\cdot}(a,1-a)\right| \leq 2\max_{1\leq i\leq N}|\overline{W}_{i,\cdot}(a,1-a)|,
\end{aligned}
$$

we have

$$
\begin{aligned}
\frac{1}{N}\max_{1\leq i\leq N}\overline{\epsilon}_{i,\cdot}(a,1-a)^2 &\leq O\left(\frac{1}{N}\right)\max_{1\leq i\leq N}\overline{W}_{i,\cdot}(a,1-a)^2\\
&= O\left(\frac{1}{N}\right)\left\{\max_{1\leq i\leq N}\frac{1}{N}\overline{W}_{i,\cdot}(a,1-a)^4\right\}^{1/2} N^{1/2}\\
&= O\left(\frac{1}{N}\right)\left[\max_{1\leq i\leq N}\frac{1}{N}\left\{\frac{1}{N-1}\sum_{j:j\neq i}W_{i,j}(a,1-a)\right\}^4\right]^{1/2} N^{1/2}\\
&\leq O\left(\frac{1}{N}\right)\left\{\max_{1\leq i\leq N}\frac{1}{N}\frac{(N-1)^3}{(N-1)^4}\sum_{j:j\neq i}W_{i,j}(a,1-a)^4\right\}^{1/2} N^{1/2} \qquad \text{(Hölder's inequality)}\\
&= O\left(\frac{1}{N}\right)\left\{\max_{1\leq i\leq N}\frac{1}{N(N-1)}\sum_{j:j\neq i}W_{i,j}(a,1-a)^4\right\}^{1/2} N^{1/2}\\
&\leq O\left(\frac{1}{N}\right)\left\{\frac{1}{N(N-1)}\sum_{i\neq j}W_{i,j}(a,1-a)^4\right\}^{1/2} N^{1/2} = o(1).
\end{aligned}
$$

Similar results can be obtained for $\overline{\epsilon}_{\cdot,i}(a,1-a)$ following the same arguments. Therefore, the asymptotic normality of $\widehat{\lambda}_{\mathrm{I}}(a,1-a)$ follows from Theorem 1 of Li and Ding (2017). □

We have the following lemma regarding the coefficient of covariates.

**Lemma S8.** *Under Conditions 1-3 in the main article,* $\widehat{\gamma}_{\mathrm{I}}^{\mathrm{adj}}(a,1-a)-\gamma_{\mathrm{I}}^{\mathrm{adj}}(a,1-a)=\boldsymbol{O}_{\mathbb{P}}(N^{-1/2})$ *for* $a=0,1$.

Recall that

$$\overline{r}^{\text{adj}}_{\text{I},i,\cdot}(a,1-a)=\frac{1}{N-1}\sum_{j:j\neq i} r^{\text{adj}}_{\text{I},i,j}(a,1-a)=\overline{W}_{i,\cdot}(a,1-a)-\overline{W}(a,1-a)-\overline{\boldsymbol{X}}_{i,\cdot}^{\top}\boldsymbol{\gamma}^{\text{adj}}_{\text{I}}(a,1-a),$$
$$\overline{r}^{\text{adj}}_{\text{I},\cdot,i}(a,1-a)=\frac{1}{N-1}\sum_{j:j\neq i} r^{\text{adj}}_{\text{I},j,i}(a,1-a)=\overline{W}_{\cdot,i}(a,1-a)-\overline{W}(a,1-a)-\overline{\boldsymbol{X}}_{\cdot,i}^{\top}\boldsymbol{\gamma}^{\text{adj}}_{\text{I}}(a,1-a).$$

**Lemma S9.** *For $a=0,1$,*

$$\mathbb{V}\text{ar}\left\{\widehat{\lambda}^{\text{adj}}_{\text{I}}(a,1-a)\right\}=\frac{1}{N}V\left\{\overline{r}^{\text{adj}}_{\text{I},i}(a,1-a)\right\}+O\left(\frac{1}{N^2}\right),$$
$$\mathbb{C}\text{ov}\left\{\widehat{\lambda}^{\text{adj}}_{\text{I}}(a,1-a),\widehat{\lambda}^{\text{adj}}_{\text{I}}(1-a,a)\right\}=\frac{1}{N}CV\left(\overline{r}^{\text{adj}}_{\text{I},i}\right)+O\left(\frac{1}{N^2}\right).$$

*Proof of Theorem 2.* We first prove the consistency. By the property of the OLS,

$$\widehat{\lambda}^{\text{adj}}_{\text{I}}(a,1-a)=\overline{W}_{\mathcal{S}(a,1-a)}-\overline{\boldsymbol{X}}_{\mathcal{S}(a,1-a)}^{\top}\widehat{\boldsymbol{\gamma}}^{\text{adj}}_{\text{I}}(a,1-a),$$

where

$$\overline{W}_{\mathcal{S}(a,1-a)}=\frac{1}{N_1N_0}\sum_{i\neq j}\mathbb{1}_i(a)\mathbb{1}_j(1-a)W_{i,j},\quad \overline{\boldsymbol{X}}_{\mathcal{S}(a,1-a)}=\frac{1}{N_1N_0}\sum_{i\neq j}\mathbb{1}_i(a)\mathbb{1}_j(1-a)\boldsymbol{X}_{i,j}.$$

By the proof of Lemma S8,

$$\overline{\boldsymbol{X}}_{\mathcal{S}(a,1-a)}=\boldsymbol{O}_{\mathbb{P}}\left(\frac{1}{N^{1/2}}\right),\quad \widehat{\boldsymbol{\gamma}}^{\text{adj}}_{\text{I}}(a,1-a)=\boldsymbol{O}_{\mathbb{P}}(1).$$

Thus, $\overline{\boldsymbol{X}}_{\mathcal{S}(a,1-a)}^{\top}\widehat{\boldsymbol{\gamma}}^{\text{adj}}_{\text{I}}(a,1-a)=O_{\mathbb{P}}(N^{-1/2})=o_{\mathbb{P}}(1)$. By Lemma S4, $\overline{W}_{\mathcal{S}(a,1-a)}=\lambda(a,1-a)+O_{\mathbb{P}}(N^{-1/2})=\lambda(a,1-a)+o_{\mathbb{P}}(1)$. Therefore, $\widehat{\lambda}^{\text{adj}}_{\text{I}}(a,1-a)=\lambda(a,1-a)+o_{\mathbb{P}}(1)$.

We then prove the asymptotic normality. By Lemmas S4 and S8,

$$N^{1/2}\overline{\boldsymbol{X}}_{\mathcal{S}(a,1-a)}^{\top}\left\{\widehat{\boldsymbol{\gamma}}^{\text{adj}}_{\text{I}}(a,1-a)-\boldsymbol{\gamma}^{\text{adj}}_{\text{I}}(a,1-a)\right\}=N^{1/2}\boldsymbol{O}_{\mathbb{P}}\left(\frac{1}{N^{1/2}}\right)\boldsymbol{O}_{\mathbb{P}}\left(\frac{1}{N^{1/2}}\right)=O_{\mathbb{P}}\left(\frac{1}{N^{1/2}}\right)=o_{\mathbb{P}}(1),$$

for $a=0,1$. Thus, since $V\{\overline{r}^{\text{adj}}_{\text{I},i}(a,1-a)\}\nrightarrow 0$,

$$\left[\mathbb{V}\text{ar}\left\{\widehat{\lambda}^{\text{adj}}_{\text{I}}(a,1-a)\right\}\right]^{-1/2}\left\{\widehat{\lambda}^{\text{adj}}_{\text{I}}(a,1-a)-\lambda(a,1-a)\right\}$$

has the same asymptotic distribution as

$$\left[\mathbb{V}\text{ar}\left\{\widehat{\lambda}^{\text{adj}}_{\text{I}}(a,1-a)\right\}\right]^{-1/2}\left[\left\{\overline{W}_{\mathcal{S}(a,1-a)}-\overline{\boldsymbol{X}}_{\mathcal{S}(a,1-a)}^{\top}\boldsymbol{\gamma}^{\text{adj}}_{\text{I}}(a,1-a)\right\}-\lambda(a,1-a)\right]\xrightarrow{d}\mathcal{N}(0,1),$$

by Theorem 1, because, under Conditions 2 and 3 in the main article,

$$\frac{1}{N}\sum_{i=1}^{N}\overline{r}^{\text{adj}}_{\text{I},i,\cdot}(a,1-a)^4=\frac{1}{N}\sum_{i=1}^{N}\left\{\frac{1}{N-1}\sum_{j:j\neq i}r^{\text{adj}}_{\text{I},i,j}(a,1-a)\right\}^4\leq\frac{1}{N}\sum_{i=1}^{N}\frac{(N-1)^3}{(N-1)^4}\sum_{j:j\neq i}r^{\text{adj}}_{\text{I},i,j}(a,1-a)^4$$
$$=\frac{1}{N(N-1)}\sum_{i\neq j}r^{\text{adj}}_{\text{I},i,j}(a,1-a)^4=o(N).$$

□

We then shift our focus to the ANCOVA estimator. The arguments for consistency and asymptotic normality follow the proofs of Theorems 1 and 2, and are thus omitted. We only derive the probability limit of $\widehat{\gamma}_{\mathrm{I}}^{\mathrm{acv}}$ and the asymptotic variances.

**Lemma S10.** *Under Conditions 1-3 in the main article, $\widehat{\gamma}_{\mathrm{I}}^{\mathrm{acv}} - \gamma_{\mathrm{I}}^{\mathrm{acv}} = \boldsymbol{O}_{\mathbb{P}}(N^{-1/2})$, where*

$$\gamma_{\mathrm{I}}^{\mathrm{acv}} = \left( \sum_{i \neq j} \boldsymbol{X}_{i,j} \boldsymbol{X}_{i,j}^{\top} \right)^{-1} \sum_{i \neq j} \boldsymbol{X}_{i,j} \mathbb{E}\{W_{i,j}(A_i, A_j)\}.$$

Recall that

$$\overline{r}_{\mathrm{I},i,\cdot}^{\mathrm{acv}}(a, 1-a) = \frac{1}{N-1} \sum_{j:j\neq i} r_{\mathrm{I},i,j}^{\mathrm{acv}}(a, 1-a) = \overline{W}_{i,\cdot}(a, 1-a) - \overline{W}(a, 1-a) - \overline{\boldsymbol{X}}_{i,\cdot}^{\top} \gamma_{\mathrm{I}}^{\mathrm{acv}},$$
$$\overline{r}_{\mathrm{I},\cdot,i}^{\mathrm{acv}}(a, 1-a) = \frac{1}{N-1} \sum_{j:j\neq i} r_{\mathrm{I},j,i}^{\mathrm{acv}}(a, 1-a) = \overline{W}_{\cdot,i}(a, 1-a) - \overline{W}(a, 1-a) - \overline{\boldsymbol{X}}_{\cdot,i}^{\top} \gamma_{\mathrm{I}}^{\mathrm{acv}}.$$

**Lemma S11.** *For $a = 0, 1$,*

$$\mathbb{V}\mathrm{ar}\left\{ \widehat{\lambda}_{\mathrm{I}}^{\mathrm{acv}}(a, 1-a) \right\} = \frac{1}{N} V\left\{ \overline{r}_{\mathrm{I},i}^{\mathrm{acv}}(a, 1-a) \right\} + O\left( \frac{1}{N^2} \right),$$
$$\mathbb{C}\mathrm{ov}\left\{ \widehat{\lambda}_{\mathrm{I}}^{\mathrm{acv}}(a, 1-a), \widehat{\lambda}_{\mathrm{I}}^{\mathrm{acv}}(1-a, a) \right\} = \frac{1}{N} CV\left( \overline{r}_{\mathrm{I},i}^{\mathrm{acv}} \right) + O\left( \frac{1}{N^2} \right).$$

# S3 Estimators using per unit averages of pairs

**Lemma S12.** *Under Conditions 1, 4, and 5 in the main article, $\widehat{\gamma}_{\mathrm{A},\mathfrak{o}}^{\mathrm{adj}}(a, 1-a) - \gamma_{\mathrm{A},\mathfrak{o}}^{\mathrm{adj}}(a, 1-a) = \boldsymbol{O}_{\mathbb{P}}(N^{-1/2})$ for $a = 0, 1$ and $\mathfrak{o} = 1, 2$.*

Recall that, for $\mathfrak{o} = 1, 2$,

$$\overline{r}_{\mathrm{A},\mathfrak{o},i,\cdot}^{\mathrm{adj}}(a, 1-a) = \frac{1}{N-1} \sum_{j:j\neq i} r_{\mathrm{A},\mathfrak{o},i,j}^{\mathrm{adj}}(a, 1-a) = \overline{W}_{i,\cdot}(a, 1-a) - \overline{W}(a, 1-a) - \overline{\boldsymbol{X}}_{i,\cdot}^{\top} \gamma_{\mathrm{A},\mathfrak{o}}^{\mathrm{adj}}(a, 1-a),$$
$$\overline{r}_{\mathrm{A},\mathfrak{o},\cdot,i}^{\mathrm{adj}}(a, 1-a) = \frac{1}{N-1} \sum_{j:j\neq i} r_{\mathrm{A},\mathfrak{o},j,i}^{\mathrm{adj}}(a, 1-a) = \overline{W}_{\cdot,i}(a, 1-a) - \overline{W}(a, 1-a) - \overline{\boldsymbol{X}}_{\cdot,i}^{\top} \gamma_{\mathrm{A},\mathfrak{o}}^{\mathrm{adj}}(a, 1-a).$$

**Lemma S13.** *For $a = 0, 1$ and $\mathfrak{o} = 1, 2$,*

$$\mathbb{V}\mathrm{ar}\left\{ \widehat{\lambda}_{\mathrm{A},\mathfrak{o}}^{\mathrm{adj}}(a, 1-a) \right\} = \frac{1}{N} V\left\{ \overline{r}_{\mathrm{A},\mathfrak{o},i}^{\mathrm{adj}}(a, 1-a) \right\} + O\left( \frac{1}{N^2} \right),$$
$$\mathbb{C}\mathrm{ov}\left\{ \widehat{\lambda}_{\mathrm{A},\mathfrak{o}}^{\mathrm{adj}}(a, 1-a), \widehat{\lambda}_{\mathrm{A},\mathfrak{o}}^{\mathrm{adj}}(1-a, a) \right\} = \frac{1}{N} CV\left( \overline{r}_{\mathrm{A},\mathfrak{o},i}^{\mathrm{adj}} \right) + O\left( \frac{1}{N^2} \right).$$

*Proof of Theorem 4.* We first prove the consistency. By the property of the OLS,

$$\widehat{\lambda}_{\mathrm{A},\mathfrak{o}}^{\mathrm{adj}}(a, 1-a) = \overline{W}_{\mathcal{S}(a,1-a)} - \overline{\boldsymbol{X}}_{\mathcal{S}(a,1-a)}^{\top} \widehat{\gamma}_{\mathrm{A},\mathfrak{o}}^{\mathrm{adj}}(a, 1-a).$$

By Lemma S12, $\widehat{\gamma}_{\mathrm{A},\mathfrak{o}}^{\mathrm{adj}}(a, 1-a) = \boldsymbol{O}_{\mathbb{P}}(1)$. Thus, $\overline{\boldsymbol{X}}_{\mathcal{S}(a,1-a)}^{\top} \widehat{\gamma}_{\mathrm{A},\mathfrak{o}}^{\mathrm{adj}}(a, 1-a) = O_{\mathbb{P}}(N^{-1/2}) = o_{\mathbb{P}}(1)$. By Lemma S4, $\overline{W}_{\mathcal{S}(a,1-a)} = \lambda(a, 1-a) + O_{\mathbb{P}}(N^{-1/2}) = \lambda(a, 1-a) + o_{\mathbb{P}}(1)$. Therefore, $\widehat{\lambda}_{\mathrm{A},\mathfrak{o}}^{\mathrm{adj}}(a, 1-a) = \lambda(a, 1-a) + o_{\mathbb{P}}(1)$.

We then prove the asymptotic normality. By Lemmas S4 and S12,

$$N^{1/2}\overline{\boldsymbol{X}}_{\mathcal{S}(a,1-a)}^{\top}\left\{\widehat{\boldsymbol{\gamma}}_{\mathrm{A},\mathfrak{o}}^{\mathrm{adj}}(a,1-a)-\boldsymbol{\gamma}_{\mathrm{A},\mathfrak{o}}^{\mathrm{adj}}(a,1-a)\right\}=N^{1/2}\boldsymbol{O}_{\mathbb{P}}\left(\frac{1}{N^{1/2}}\right)\boldsymbol{O}_{\mathbb{P}}\left(\frac{1}{N^{1/2}}\right)=O_{\mathbb{P}}\left(\frac{1}{N^{1/2}}\right)=o_{\mathbb{P}}(1).$$

Thus, since $V\{\overline{r}_{\mathrm{A},\mathfrak{o},i}^{\mathrm{adj}}(a,1-a)\}\nrightarrow 0$,

$$\left[\mathbb{V}\mathrm{ar}\left\{\widehat{\lambda}_{\mathrm{A},\mathfrak{o}}^{\mathrm{adj}}(a,1-a)\right\}\right]^{-1/2}\left\{\widehat{\lambda}_{\mathrm{A},\mathfrak{o}}^{\mathrm{adj}}(a,1-a)-\lambda(a,1-a)\right\}$$

has the same asymptotic distribution as

$$\left[\mathbb{V}\mathrm{ar}\left\{\widehat{\lambda}_{\mathrm{A},\mathfrak{o}}^{\mathrm{adj}}(a,1-a)\right\}\right]^{-1/2}\left[\left\{\overline{W}_{\mathcal{S}(a,1-a)}-\overline{\boldsymbol{X}}_{\mathcal{S}(a,1-a)}^{\top}\boldsymbol{\gamma}_{\mathrm{A},\mathfrak{o}}^{\mathrm{adj}}(a,1-a)\right\}-\lambda(a,1-a)\right]\xrightarrow{d}\mathcal{N}(0,1),$$

by Theorem 1, because, under Conditions 2 and 3 in the main article,

$$\begin{aligned}\frac{1}{N}\sum_{i=1}^{N}\overline{r}_{\mathrm{A},\mathfrak{o},i,\cdot}^{\mathrm{adj}}(a,1-a)^4&=\frac{1}{N}\sum_{i=1}^{N}\left\{\frac{1}{N-1}\sum_{j:j\neq i}r_{\mathrm{A},\mathfrak{o},i,j}^{\mathrm{adj}}(a,1-a)\right\}^4\leq\frac{1}{N}\sum_{i=1}^{N}\frac{(N-1)^3}{(N-1)^4}\sum_{j:j\neq i}r_{\mathrm{A},\mathfrak{o},i,j}^{\mathrm{adj}}(a,1-a)^4\\&=\frac{1}{N(N-1)}\sum_{i\neq j}r_{\mathrm{A},\mathfrak{o},i,j}^{\mathrm{adj}}(a,1-a)^4=o(N).\end{aligned}$$

□

For the ANCOVA estimator, the arguments for consistency and asymptotic normality follow the proofs of Theorem 4 and are thus omitted. We only derive the probability limit of $\widehat{\boldsymbol{\gamma}}_{\mathrm{A},\mathfrak{o}}^{\mathrm{acv}}$ and the asymptotic variances.

**Lemma S14.** *Under Conditions 1, 4, and 5 in the main article,* $\widehat{\boldsymbol{\gamma}}_{\mathrm{A},\mathfrak{o}}^{\mathrm{acv}}-\{\pi_a\boldsymbol{\gamma}_{\mathrm{A},\mathfrak{o}}^{\mathrm{adj}}(a,1-a)+\pi_{1-a}\boldsymbol{\gamma}_{\mathrm{A},\mathfrak{o}}^{\mathrm{adj}}(1-a,a)\}=\boldsymbol{O}_{\mathbb{P}}(N^{-1/2})$ *for* $a=0,1$ *and* $\mathfrak{o}=1,2$*.*

Recall that

$$\begin{aligned}\overline{r}_{\mathrm{A},\mathfrak{o},i,\cdot}^{\mathrm{acv}}(a,1-a)&=\frac{1}{N-1}\sum_{j:j\neq i}r_{\mathrm{A},\mathfrak{o},i,j}^{\mathrm{acv}}(a,1-a)=\overline{W}_{i,\cdot}(a,1-a)-\overline{W}(a,1-a)-\overline{\boldsymbol{X}}_{i,\cdot}^{\top}\boldsymbol{\gamma}_{\mathrm{A},\mathfrak{o}}^{\mathrm{acv}},\\\overline{r}_{\mathrm{A},\mathfrak{o},\cdot,i}^{\mathrm{acv}}(a,1-a)&=\frac{1}{N-1}\sum_{j:j\neq i}r_{\mathrm{A},\mathfrak{o},j,i}^{\mathrm{acv}}(a,1-a)=\overline{W}_{\cdot,i}(a,1-a)-\overline{W}(a,1-a)-\overline{\boldsymbol{X}}_{\cdot,i}^{\top}\boldsymbol{\gamma}_{\mathrm{A},\mathfrak{o}}^{\mathrm{acv}}.\end{aligned}$$

**Lemma S15.** *For* $a=0,1$ *and* $\mathfrak{o}=1,2$*,*

$$\begin{aligned}\mathbb{V}\mathrm{ar}\left\{\widehat{\lambda}_{\mathrm{A},\mathfrak{o}}^{\mathrm{acv}}(a,1-a)\right\}&=\frac{1}{N}V\left\{\overline{r}_{\mathrm{A},\mathfrak{o},i}^{\mathrm{acv}}(a,1-a)\right\}+O\left(\frac{1}{N^2}\right),\\\mathbb{C}\mathrm{ov}\left\{\widehat{\lambda}_{\mathrm{A},\mathfrak{o}}^{\mathrm{acv}}(a,1-a),\widehat{\lambda}_{\mathrm{A},\mathfrak{o}}^{\mathrm{acv}}(1-a,a)\right\}&=\frac{1}{N}CV\left(\overline{r}_{\mathrm{A},\mathfrak{o},i}^{\mathrm{acv}}\right)+O\left(\frac{1}{N^2}\right).\end{aligned}$$

The proof of Lemma S15 follows that of Lemma S11 and is thus omitted. We then prove Propositions 1-3 under contrast functions satisfying $W_{i,j}=C-W_{j,i}$ for some constant $C$.

*Proof of Proposition 1.* First, for $\boldsymbol{\gamma}_{\mathrm{I}}^{\mathrm{adj}}(a,1-a)$ and $\boldsymbol{\gamma}_{\mathrm{I}}^{\mathrm{adj}}(1-a,a)$, recall that

$$\boldsymbol{\gamma}_{\mathrm{I}}^{\mathrm{adj}}(a,1-a)=\left(\sum_{i\neq j}\boldsymbol{X}_{i,j}\boldsymbol{X}_{i,j}^{\top}\right)^{-1}\sum_{i\neq j}\boldsymbol{X}_{i,j}W_{i,j}(a,1-a),$$

$$\boldsymbol{\gamma}_{\mathrm{I}}^{\mathrm{adj}}(1-a,a)=\left(\sum_{i\neq j}\boldsymbol{X}_{i,j}\boldsymbol{X}_{i,j}^{\top}\right)^{-1}\sum_{i\neq j}\boldsymbol{X}_{i,j}W_{i,j}(1-a,a).$$

Since $W_{i,j}(a,1-a)=C-W_{j,i}(1-a,a)$, then

$$\sum_{i\neq j}\boldsymbol{X}_{i,j}W_{i,j}(a,1-a)=\sum_{i\neq j}\boldsymbol{X}_{i,j}\{C-W_{j,i}(1-a,a)\}=-\sum_{i\neq j}\boldsymbol{X}_{i,j}W_{j,i}(1-a,a).$$

Let $i'=j$ and $j'=i$. Then,

$$\sum_{i\neq j}X_{i,j}W_{j,i}(1-a,a)=\sum_{j'\neq i'}\boldsymbol{X}_{j',i'}W_{i',j'}(1-a,a)=-\sum_{i'\neq j'}\boldsymbol{X}_{i',j'}W_{i',j'}(1-a,a).$$

Thus,

$$\sum_{i\neq j}\boldsymbol{X}_{i,j}W_{j,i}(1-a,a)=-\sum_{i\neq j}\boldsymbol{X}_{i,j}W_{i,j}(1-a,a).$$

Therefore,

$$\sum_{i\neq j}\boldsymbol{X}_{i,j}W_{i,j}(a,1-a)=-\left\{-\sum_{i\neq j}\boldsymbol{X}_{i,j}W_{i,j}(1-a,a)\right\}=\sum_{i\neq j}\boldsymbol{X}_{i,j}W_{i,j}(1-a,a),$$

and

$$\boldsymbol{\gamma}_{\mathrm{I}}^{\mathrm{adj}}(a,1-a)=\boldsymbol{\gamma}_{\mathrm{I}}^{\mathrm{adj}}(1-a,a).$$

Then, for the leading terms of the Neyman variances,

$$\begin{aligned}\overline{r}_{\mathrm{I},i,\cdot}^{\mathrm{adj}}(a,1-a)&=\overline{W}_{i,\cdot}(a,1-a)-\overline{W}(a,1-a)-\overline{\boldsymbol{X}}_{i,\cdot}^{\top}\boldsymbol{\gamma}_{\mathrm{I}}^{\mathrm{adj}}(a,1-a)\\&=C-\overline{W}_{\cdot,i}(1-a,a)-\left\{C-\overline{W}(1-a,a)\right\}+\overline{\boldsymbol{X}}_{\cdot,i}^{\top}\boldsymbol{\gamma}_{\mathrm{I}}^{\mathrm{adj}}(1-a,a)\\&=-\overline{W}_{\cdot,i}(1-a,a)+\overline{W}(1-a,a)+\overline{\boldsymbol{X}}_{\cdot,i}^{\top}\boldsymbol{\gamma}_{\mathrm{I}}^{\mathrm{adj}}(1-a,a)\\&=-\overline{r}_{\mathrm{I},\cdot,i}^{\mathrm{adj}}(1-a,a).\end{aligned}$$

Similarly, $\overline{r}_{\mathrm{I},\cdot,i}^{\mathrm{adj}}(a,1-a)=-\overline{r}_{\mathrm{I},i,\cdot}^{\mathrm{adj}}(1-a,a)$. Thus, $V\{\overline{r}_{\mathrm{I},i}^{\mathrm{adj}}(a,1-a)\}=V\{\overline{r}_{\mathrm{I},i}^{\mathrm{adj}}(1-a,a)\}$. For the covariance,

$$\begin{aligned}CV(\overline{r}_{\mathrm{I},i}^{\mathrm{adj}})&=\frac{1}{\pi_aN}\sum_{i=1}^{N}\overline{r}_{\mathrm{I},i,\cdot}^{\mathrm{adj}}(a,1-a)\overline{r}_{\mathrm{I},\cdot,i}^{\mathrm{adj}}(1-a,a)+\frac{1}{\pi_{1-a}N}\sum_{i=1}^{N}\overline{r}_{\mathrm{I},i,\cdot}^{\mathrm{adj}}(1-a,a)\overline{r}_{\mathrm{I},\cdot,i}^{\mathrm{adj}}(a,1-a)\\&\quad-\frac{1}{N}\sum_{i=1}^{N}\left\{\overline{r}_{\mathrm{I},i,\cdot}^{\mathrm{adj}}(a,1-a)+\overline{r}_{\mathrm{I},\cdot,i}^{\mathrm{adj}}(a,1-a)\right\}\left\{\overline{r}_{\mathrm{I},i,\cdot}^{\mathrm{adj}}(1-a,a)+\overline{r}_{\mathrm{I},\cdot,i}^{\mathrm{adj}}(1-a,a)\right\}\\&=-\frac{1}{\pi_aN}\overline{r}_{\mathrm{I},i,\cdot}^{\mathrm{adj}}(a,1-a)^2-\frac{1}{\pi_{1-a}N}\sum_{i=1}^{N}\overline{r}_{\mathrm{I},i,\cdot}^{\mathrm{adj}}(1-a,a)^2\\&\quad-\frac{1}{N}\sum_{i=1}^{N}\left\{\overline{r}_{\mathrm{I},i,\cdot}^{\mathrm{adj}}(a,1-a)-\overline{r}_{\mathrm{I},i,\cdot}^{\mathrm{adj}}(1-a,a)\right\}\left\{\overline{r}_{\mathrm{I},i,\cdot}^{\mathrm{adj}}(1-a,a)-\overline{r}_{\mathrm{I},i,\cdot}^{\mathrm{adj}}(a,1-a)\right\}\\&=-\frac{1}{\pi_aN}\overline{r}_{\mathrm{I},i,\cdot}^{\mathrm{adj}}(a,1-a)^2-\frac{1}{\pi_{1-a}N}\sum_{i=1}^{N}\overline{r}_{\mathrm{I},i,\cdot}^{\mathrm{adj}}(1-a,a)^2+\frac{1}{N}\sum_{i=1}^{N}\left\{\overline{r}_{\mathrm{I},i,\cdot}^{\mathrm{adj}}(a,1-a)-\overline{r}_{\mathrm{I},i,\cdot}^{\mathrm{adj}}(1-a,a)\right\}^2\end{aligned}$$

$$= -\frac{1}{\pi_a N}\overline{r}^{\text{adj}}_{\text{I},i,\cdot}(a,1-a)^2 - \frac{1}{\pi_{1-a}N}\sum_{i=1}^{N}\overline{r}^{\text{adj}}_{\text{I},\cdot,i}(a,1-a)^2 + \frac{1}{N}\sum_{i=1}^{N}\left\{\overline{r}^{\text{adj}}_{\text{I},i,\cdot}(a,1-a) + \overline{r}^{\text{adj}}_{\text{I},\cdot,i}(a,1-a)\right\}^2$$

$$= -V\{\overline{r}^{\text{adj}}_{\text{I},i}(a,1-a)\} = -V\{\overline{r}^{\text{adj}}_{\text{I},i}(1-a,a)\}.$$

The results for $\widehat{\lambda}_{\text{I}}(a,1-a)$ and $\widehat{\lambda}^{\text{acv}}_{\text{I}}(a,1-a)$ are obtained following the same arguments. □

*Proof of Proposition 2.* First, we prove results for $\boldsymbol{\gamma}^{\text{adj}}_{\text{A},1}(a,1-a)$ and $\boldsymbol{\gamma}^{\text{adj}}_{\text{A},1}(1-a,a)$, recall that

$$\boldsymbol{\gamma}^{\text{adj}}_{\text{A},1}(a,1-a) = \left(\sum_{i=1}^{N}\overline{\boldsymbol{X}}_{i,\cdot}\overline{\boldsymbol{X}}_{i,\cdot}^{\top}\right)^{-1}\sum_{i=1}^{N}\overline{\boldsymbol{X}}_{i,\cdot}\overline{W}_{i,\cdot}(a,1-a),$$
$$\boldsymbol{\gamma}^{\text{adj}}_{\text{A},1}(1-a,a) = \left(\sum_{i=1}^{N}\overline{\boldsymbol{X}}_{i,\cdot}\overline{\boldsymbol{X}}_{i,\cdot}^{\top}\right)^{-1}\sum_{i=1}^{N}\overline{\boldsymbol{X}}_{i,\cdot}\overline{W}_{i,\cdot}(1-a,a).$$

Since $W_{i,j}(a,1-a) = C - W_{j,i}(1-a,a)$, then

$$\overline{W}_{i,\cdot}(a,1-a) = \frac{1}{N-1}\sum_{j:j\neq i}\{C - W_{j,i}(1-a,a)\} = C - \frac{1}{N-1}\sum_{j:j\neq i}W_{j,i}(1-a,a) = C - \overline{W}_{\cdot,i}(1-a,a).$$

Then,

$$\sum_{i=1}^{N}\overline{\boldsymbol{X}}_{i,\cdot}\overline{W}_{i,\cdot}(a,1-a) = \sum_{i=1}^{N}\overline{\boldsymbol{X}}_{i,\cdot}\{C - \overline{W}_{\cdot,i}(1-a,a)\} = -\sum_{i=1}^{N}\overline{\boldsymbol{X}}_{i,\cdot}\overline{W}_{\cdot,i}(1-a,a).$$

However,

$$\overline{W}_{\cdot,i}(1-a,a) = \frac{1}{N-1}\sum_{j:j\neq i}W_{j,i}(1-a,a) \neq -\frac{1}{N-1}\sum_{j:j\neq i}W_{i,j}(1-a,a) = -\overline{W}_{i,\cdot}(1-a,a).$$

Thus,

$$\sum_{i=1}^{N}\overline{\boldsymbol{X}}_{i,\cdot}\overline{W}_{i,\cdot}(a,1-a) \neq \sum_{i=1}^{N}\overline{\boldsymbol{X}}_{i,\cdot}\overline{W}_{i,\cdot}(1-a,a).$$

Therefore, in general,

$$\boldsymbol{\gamma}^{\text{adj}}_{\text{A},1}(a,1-a) \neq \boldsymbol{\gamma}^{\text{adj}}_{\text{A},1}(1-a,a).$$

The result of $\boldsymbol{\gamma}^{\text{adj}}_{\text{A},2}(a,1-a) \neq \boldsymbol{\gamma}^{\text{adj}}_{\text{A},2}(1-a,a)$ can be obtained following the same arguments. Then, for $\boldsymbol{\gamma}^{\text{adj}}_{\text{A},1}(a,1-a)$ and $\boldsymbol{\gamma}^{\text{adj}}_{\text{A},2}(1-a,a)$, recall that

$$\boldsymbol{\gamma}^{\text{adj}}_{\text{A},2}(1-a,a) = \left(\sum_{i=1}^{N}\overline{\boldsymbol{X}}_{\cdot,i}\overline{\boldsymbol{X}}_{\cdot,i}^{\top}\right)^{-1}\sum_{i=1}^{N}\overline{\boldsymbol{X}}_{\cdot,i}\overline{W}_{\cdot,i}(1-a,a).$$

Since $W_{i,j}(a,1-a) = C - W_{j,i}(1-a,a)$ and $\overline{\boldsymbol{X}}_{i,\cdot} = -\overline{\boldsymbol{X}}_{\cdot,i}$, then

$$\boldsymbol{\gamma}^{\text{adj}}_{\text{A},2}(1-a,a) = \left(\sum_{i=1}^{N}\overline{\boldsymbol{X}}_{\cdot,i}\overline{\boldsymbol{X}}_{\cdot,i}^{\top}\right)^{-1}\sum_{i=1}^{N}\overline{\boldsymbol{X}}_{\cdot,i}\overline{W}_{\cdot,i}(1-a,a)$$

$$
\begin{aligned}
&= -\left(\sum_{i=1}^{N} \overline{\boldsymbol{X}}_{i,\cdot}\overline{\boldsymbol{X}}_{i,\cdot}^{\top}\right)^{-1}\sum_{i=1}^{N}\overline{\boldsymbol{X}}_{i,\cdot}\left\{C-\overline{W}_{i,\cdot}(a,1-a)\right\}\\
&= C\left(\sum_{i=1}^{N} \overline{\boldsymbol{X}}_{i,\cdot}\overline{\boldsymbol{X}}_{i,\cdot}^{\top}\right)^{-1}\sum_{i=1}^{N}\overline{\boldsymbol{X}}_{i,\cdot}+\left(\sum_{i=1}^{N} \overline{\boldsymbol{X}}_{i,\cdot}\overline{\boldsymbol{X}}_{i,\cdot}^{\top}\right)^{-1}\sum_{i=1}^{N}\overline{\boldsymbol{X}}_{i,\cdot}\overline{W}_{i,\cdot}(a,1-a)\\
&= \left(\sum_{i=1}^{N} \overline{\boldsymbol{X}}_{i,\cdot}\overline{\boldsymbol{X}}_{i,\cdot}^{\top}\right)^{-1}\sum_{i=1}^{N}\overline{\boldsymbol{X}}_{i,\cdot}\overline{W}_{i,\cdot}(a,1-a)=\boldsymbol{\gamma}_{\mathrm{A},1}^{\mathrm{adj}}(a,1-a).
\end{aligned}
$$

Then, for the leading terms of the Neyman variances,

$$
\begin{aligned}
\overline{r}_{\mathrm{A},1,i,\cdot}^{\mathrm{adj}}(a,1-a) &= \overline{W}_{i,\cdot}(a,1-a)-\overline{W}(a,1-a)-\overline{\boldsymbol{X}}_{i,\cdot}^{\top}\boldsymbol{\gamma}_{\mathrm{A},1}^{\mathrm{adj}}(a,1-a)\\
&= C-\overline{W}_{\cdot,i}(1-a,a)-\left\{C-\overline{W}(1-a,a)\right\}+\overline{\boldsymbol{X}}_{\cdot,i}^{\top}\boldsymbol{\gamma}_{\mathrm{A},2}^{\mathrm{adj}}(1-a,a)\\
&= -\overline{W}_{\cdot,i}(1-a,a)+\overline{W}(1-a,a)+\overline{\boldsymbol{X}}_{\cdot,i}^{\top}\boldsymbol{\gamma}_{\mathrm{A},2}^{\mathrm{adj}}(1-a,a)\\
&= -\overline{r}_{\mathrm{A},2,\cdot,i}^{\mathrm{adj}}(1-a,a).
\end{aligned}
$$

Similarly, $\overline{r}_{\mathrm{A},1,\cdot,i}^{\mathrm{adj}}(a,1-a)=-\overline{r}_{\mathrm{A},2,i,\cdot}^{\mathrm{adj}}(1-a,a)$. Thus, $V\{\overline{r}_{\mathrm{A},1,i}^{\mathrm{adj}}(a,1-a)\}=V\{\overline{r}_{\mathrm{A},2,i}^{\mathrm{adj}}(1-a,a)\}$. For the covariance,

$$
\begin{aligned}
CV(\overline{r}_{\mathrm{A},1,i}^{\mathrm{adj}}) &= \frac{1}{\pi_a N}\sum_{i=1}^{N}\overline{r}_{\mathrm{A},1,i,\cdot}^{\mathrm{adj}}(a,1-a)\overline{r}_{\mathrm{A},1,\cdot,i}^{\mathrm{adj}}(1-a,a)+\frac{1}{\pi_{1-a}N}\sum_{i=1}^{N}\overline{r}_{\mathrm{A},1,i,\cdot}^{\mathrm{adj}}(1-a,a)\overline{r}_{\mathrm{A},1,\cdot,i}^{\mathrm{adj}}(a,1-a)\\
&\quad -\frac{1}{N}\sum_{i=1}^{N}\left\{\overline{r}_{\mathrm{A},1,i,\cdot}^{\mathrm{adj}}(a,1-a)+\overline{r}_{\mathrm{A},1,\cdot,i}^{\mathrm{adj}}(a,1-a)\right\}\left\{\overline{r}_{\mathrm{A},1,i,\cdot}^{\mathrm{adj}}(1-a,a)+\overline{r}_{\mathrm{A},1,\cdot,i}^{\mathrm{adj}}(1-a,a)\right\}\\
&= \frac{1}{\pi_a N}\sum_{i=1}^{N}\overline{r}_{\mathrm{A},2,\cdot,i}^{\mathrm{adj}}(1-a,a)\overline{r}_{\mathrm{A},2,i,\cdot}^{\mathrm{adj}}(a,1-a)+\frac{1}{\pi_{1-a}N}\sum_{i=1}^{N}\overline{r}_{\mathrm{A},2,\cdot,i}^{\mathrm{adj}}(a,1-a)\overline{r}_{\mathrm{A},2,i,\cdot}^{\mathrm{adj}}(1-a,a)\\
&\quad -\frac{1}{N}\sum_{i=1}^{N}\left\{\overline{r}_{\mathrm{A},2,\cdot,i}^{\mathrm{adj}}(1-a,a)+\overline{r}_{\mathrm{A},2,i,\cdot}^{\mathrm{adj}}(1-a,a)\right\}\left\{\overline{r}_{\mathrm{A},2,\cdot,i}^{\mathrm{adj}}(a,1-a)+\overline{r}_{\mathrm{A},2,i,\cdot}^{\mathrm{adj}}(a,1-a)\right\}\\
&= CV(\overline{r}_{\mathrm{A},2,i}^{\mathrm{adj}}).
\end{aligned}
$$

Results for the ANCOVA estimators are a direct implication of Lemmas S14 and S15, where

$$
\boldsymbol{\gamma}_{\mathrm{A},1}^{\mathrm{acv}}=\pi_a\boldsymbol{\gamma}_{\mathrm{A},1}^{\mathrm{adj}}(a,1-a)+\pi_{1-a}\boldsymbol{\gamma}_{\mathrm{A},1}^{\mathrm{adj}}(1-a,a)=\pi_a\boldsymbol{\gamma}_{\mathrm{A},2}^{\mathrm{adj}}(1-a,a)+\pi_{1-a}\boldsymbol{\gamma}_{\mathrm{A},2}^{\mathrm{adj}}(a,1-a)\neq\boldsymbol{\gamma}_{\mathrm{A},2}^{\mathrm{acv}},
$$

unless $\pi_0=\pi_1=1/2$. Therefore, $V\{\overline{r}_{\mathrm{A},1,i}^{\mathrm{acv}}(a,1-a)\}=V\{\overline{r}_{\mathrm{A},2,i}^{\mathrm{acv}}(1-a,a)\}$ and $CV(\overline{r}_{\mathrm{A},1,i}^{\mathrm{acv}})=CV(\overline{r}_{\mathrm{A},2,i}^{\mathrm{acv}})$ if $\pi_0=\pi_1=1/2$. □

*Proof of Proposition 3.* Following the proof of Lemma S7, for estimators using individual pairs, using $\widehat{\tau}_{\mathrm{I}}^{\mathrm{adj}}(a)$, we have

$$
\begin{aligned}
\Psi_{\mathrm{I}}^{\mathrm{adj},*}(a)=\frac{1}{N}\sum_{i=1}^{N}\bigg\{&\frac{1}{\pi_a}\overline{r}_{\mathrm{I},i,\cdot}^{\mathrm{adj}}(a,1-a)\mathbb{1}_i(a)-\frac{1}{\pi_a}\overline{r}_{\mathrm{I},\cdot,i}^{\mathrm{adj}}(1-a,a)\mathbb{1}_i(a)\\
&+\frac{1}{\pi_{1-a}}\overline{r}_{\mathrm{I},\cdot,i}^{\mathrm{adj}}(a,1-a)\mathbb{1}_i(1-a)-\frac{1}{\pi_{1-a}}\overline{r}_{\mathrm{I},i,\cdot}^{\mathrm{adj}}(1-a,a)\mathbb{1}_i(1-a)\bigg\}.
\end{aligned}
$$

From Proposition 1, we have $\overline{r}_{\mathrm{I},i,\cdot}^{\mathrm{adj}}(a,1-a)=-\overline{r}_{\mathrm{I},\cdot,i}^{\mathrm{adj}}(1-a,a)$. Then,

$$
\Psi_{\mathrm{I}}^{\mathrm{adj},*}(a)=\frac{1}{N}\sum_{i=1}^{N}\left\{\frac{2}{\pi_a}\overline{r}_{\mathrm{I},i,\cdot}^{\mathrm{adj}}(a,1-a)\mathbb{1}_i(a)-\frac{2}{\pi_{1-a}}\overline{r}_{\mathrm{I},i,\cdot}^{\mathrm{adj}}(1-a,a)\mathbb{1}_i(1-a)\right\}
$$

$$= \frac{1}{N}\sum_{i=1}^{N}\left\{\frac{2}{\pi_a}\overline{r}^{\text{adj}}_{\text{I},i,\cdot}(a,1-a)\mathbb{1}_i(a) + \frac{2}{\pi_{1-a}}\overline{r}^{\text{adj}}_{\text{I},\cdot,i}(a,1-a)\mathbb{1}_i(1-a)\right\}.$$

Therefore, we have $V(\overline{r}^{\text{adj}}_{\text{I},i}) = 4V\{\overline{r}^{\text{adj}}_{\text{I},i}(a,1-a)\} = 4V\{\overline{r}^{\text{adj}}_{\text{I},i}(1-a,a)\}$. Similar results can be obtained for other estimators using individual pairs following the same argument. For estimators using per-unit pair averages, using $\widehat{\tau}^{\text{adj}}_{\text{A},1}(a)$, we have

$$\Psi^{\text{adj},*}_{\text{A},1}(a) = \frac{1}{N}\sum_{i=1}^{N}\left\{\frac{1}{\pi_a}\overline{r}^{\text{adj}}_{\text{A},1,i,\cdot}(a,1-a)\mathbb{1}_i(a) - \frac{1}{\pi_a}\overline{r}^{\text{adj}}_{\text{A},1,\cdot,i}(1-a,a)\mathbb{1}_i(a)\right.$$
$$\left. + \frac{1}{\pi_{1-a}}\overline{r}^{\text{adj}}_{\text{A},1,\cdot,i}(a,1-a)\mathbb{1}_i(1-a) - \frac{1}{\pi_{1-a}}\overline{r}^{\text{adj}}_{\text{A},1,i,\cdot}(1-a,a)\mathbb{1}_i(1-a)\right\}.$$

From Proposition 2, we have $\overline{r}^{\text{adj}}_{\text{A},1,i,\cdot}(a,1-a) = -\overline{r}^{\text{adj}}_{\text{A},2,\cdot,i}(1-a,a)$. Then,

$$\Psi^{\text{adj},*}_{\text{A},1}(a) = \frac{1}{N}\sum_{i=1}^{N}\left\{\frac{1}{\pi_a}\overline{r}^{\text{adj}}_{\text{A},1,i,\cdot}(a,1-a)\mathbb{1}_i(a) + \frac{1}{\pi_a}\overline{r}^{\text{adj}}_{\text{A},2,i,\cdot}(a,1-a)\mathbb{1}_i(a)\right.$$
$$\left. + \frac{1}{\pi_{1-a}}\overline{r}^{\text{adj}}_{\text{A},1,\cdot,i}(a,1-a)\mathbb{1}_i(1-a) + \frac{1}{\pi_{1-a}}\overline{r}^{\text{adj}}_{\text{A},2,\cdot,i}(a,1-a)\mathbb{1}_i(1-a)\right\} = \Psi^{\text{adj},*}_{\text{A},2}(a).$$

Thus, $V(\overline{r}^{\text{adj}}_{\text{A},1,i}) = V(\overline{r}^{\text{adj}}_{\text{A},2,i})$. Similar results can be obtained for other estimators using per-unit pair averages following the same argument. □

# S4 PIM estimators for estimating the net benefit

## S4.1 Consistency and asymptotic normality of the PIM estimators

For $\widehat{\tau}_{\text{P}}(a)$, by the property of the OLS, we have

$$\widehat{\tau}_{\text{P}}(a) = \overline{W}_{\mathcal{S}(a,1-a)} - \overline{W}_{\mathcal{S}(1-a,a)} = \widehat{\lambda}_{\text{I}}(a,1-a) - \widehat{\lambda}_{\text{I}}(1-a,a)$$

Thus, its consistency and asymptotic normality are implied by those of $\widehat{\lambda}_{\text{I}}(a,1-a)$ and $\widehat{\lambda}_{\text{I}}(1-a,a)$. For $\widehat{\tau}^{\text{acv}}_{\text{P}}(a)$, let $\widehat{\gamma}^{\text{acv}}_{\text{P},W}$ and $\widehat{\gamma}^{\text{acv}}_{\text{P},D}$ denote the coefficients from the OLS fits of $W_{i,j}$ and $D_{i,j}$ on $\boldsymbol{X}_{i,j}$, respectively, with residuals $W_{i,j} - \boldsymbol{X}_{i,j}^\top\widehat{\gamma}^{\text{acv}}_{\text{P},W}$ and $D_{i,j} - \boldsymbol{X}_{i,j}^\top\widehat{\gamma}^{\text{acv}}_{\text{P},D}$. By the Frisch-Waugh-Lovell theorem (Angrist and Pischke, 2009), we have

$$\widehat{\tau}^{\text{acv}}_{\text{P}}(a) = 2\left(2N_1N_0 - \sum_{i\neq j} D_{i,j}\boldsymbol{X}_{i,j}^\top\widehat{\gamma}^{\text{acv}}_{\text{P},D}\right)^{-1}\left(\sum_{(i,j)\in\mathcal{S}(a,1-a)} W_{i,j} - \sum_{(i,j)\in\mathcal{S}(1-a,a)} W_{i,j} - \sum_{i\neq j} D_{i,j}\boldsymbol{X}_{i,j}^\top\widehat{\gamma}^{\text{acv}}_{\text{P},W}\right).$$

For $\widehat{\tau}^{\text{int}}_{\text{P}}(a)$, let $\widehat{\gamma}^{\text{int}}_{\text{P},W}$ and $\widehat{\gamma}^{\text{int}}_{\text{P},D}$ denote the coefficients from the OLS fits of $W_{i,j}$ and $D_{i,j}$ on $D_{i,j}\boldsymbol{X}_{i,j}$, respectively, with residuals $W_{i,j} - D_{i,j}\boldsymbol{X}_{i,j}^\top\widehat{\gamma}^{\text{int}}_{\text{P},W}$ and $D_{i,j} - D_{i,j}\boldsymbol{X}_{i,j}^\top\widehat{\gamma}^{\text{int}}_{\text{P},D}$. Then, again, by Frisch-Waugh-Lovell,

$$\widehat{\tau}^{\text{int}}_{\text{P}}(a) = 2\left(2N_1N_0 - \sum_{(i,j)\in\mathcal{S}} \boldsymbol{X}_{i,j}^\top\widehat{\gamma}^{\text{int}}_{\text{P},D}\right)^{-1}\left(\sum_{(i,j)\in\mathcal{S}(a,1-a)} W_{i,j} - \sum_{(i,j)\in\mathcal{S}(1-a,a)} W_{i,j} - \sum_{(i,j)\in\mathcal{S}} \boldsymbol{X}_{i,j}^\top\widehat{\gamma}^{\text{int}}_{\text{P},W}\right),$$

where $\mathcal{S} = \mathcal{S}(a,1-a)\cup\mathcal{S}(1-a,a)$. For $\widehat{\tau}^{\text{adj}}_{\text{P}}(a)$, let $\widehat{\gamma}^{\text{adj},W}_{\text{P},X}$ and $\widehat{\gamma}^{\text{adj},W}_{\text{P},DX}$ denote the respective coefficients of $\boldsymbol{X}_{i,j}$ and $D_{i,j}\boldsymbol{X}_{i,j}$ from the OLS fits of $W_{i,j}$ on $(\boldsymbol{X}_{i,j}^\top, D_{i,j}\boldsymbol{X}_{i,j}^\top)^\top$, with residual $W_{i,j} - \boldsymbol{X}_{i,j}^\top\widehat{\gamma}^{\text{adj},W}_{\text{P},X} - D_{i,j}\boldsymbol{X}_{i,j}^\top\widehat{\gamma}^{\text{adj},W}_{\text{P},DX}$. Similarly, let $\widehat{\gamma}^{\text{adj},D}_{\text{P},X}$ and $\widehat{\gamma}^{\text{adj},D}_{\text{P},DX}$ denote the respective coefficients of $\boldsymbol{X}_{i,j}$ and $D_{i,j}\boldsymbol{X}_{i,j}$ from the OLS fits of $D_{i,j}$ on $(\boldsymbol{X}_{i,j}^\top, D_{i,j}\boldsymbol{X}_{i,j}^\top)^\top$, with residual $D_{i,j} -$

$\boldsymbol{X}_{i,j}^{\top}\widehat{\boldsymbol{\gamma}}_{\mathrm{P},X}^{\mathrm{adj},D} - D_{i,j}\boldsymbol{X}_{i,j}^{\top}\widehat{\boldsymbol{\gamma}}_{\mathrm{P},DX}^{\mathrm{adj},D}$. Then, by Frisch-Waugh-Lovell,

$$\begin{aligned}\widehat{\tau}_{\mathrm{P}}^{\mathrm{adj}}(a) = 2 &\left\{\sum_{i\neq j}\left(D_{i,j} - \boldsymbol{X}_{i,j}^{\top}\widehat{\boldsymbol{\gamma}}_{\mathrm{P},X}^{\mathrm{adj},D} - D_{i,j}\boldsymbol{X}_{i,j}^{\top}\widehat{\boldsymbol{\gamma}}_{\mathrm{P},DX}^{\mathrm{adj},D}\right)^2\right\}^{-1} \\ &\times \sum_{i\neq j}\left(D_{i,j} - \boldsymbol{X}_{i,j}^{\top}\widehat{\boldsymbol{\gamma}}_{\mathrm{P},X}^{\mathrm{adj},D} - D_{i,j}\boldsymbol{X}_{i,j}^{\top}\widehat{\boldsymbol{\gamma}}_{\mathrm{P},DX}^{\mathrm{adj},D}\right)\left(W_{i,j} - \boldsymbol{X}_{i,j}^{\top}\widehat{\boldsymbol{\gamma}}_{\mathrm{P},X}^{\mathrm{adj},W} - D_{i,j}\boldsymbol{X}_{i,j}^{\top}\widehat{\boldsymbol{\gamma}}_{\mathrm{P},DX}^{\mathrm{adj},W}\right).\end{aligned}$$

Let $\boldsymbol{\gamma}_{\mathrm{P},W}^{\mathrm{acv}}$, $\boldsymbol{\gamma}_{\mathrm{P},D}^{\mathrm{acv}}$, $\boldsymbol{\gamma}_{\mathrm{P},W}^{\mathrm{int}}$, $\boldsymbol{\gamma}_{\mathrm{P},D}^{\mathrm{int}}$, $\boldsymbol{\gamma}_{\mathrm{P},X}^{\mathrm{adj},W}$, $\boldsymbol{\gamma}_{\mathrm{P},DX}^{\mathrm{adj},W}$, $\boldsymbol{\gamma}_{\mathrm{P},X}^{\mathrm{adj},D}$, and $\boldsymbol{\gamma}_{\mathrm{P},DX}^{\mathrm{adj},D}$ denote the finite-population probability limits of $\widehat{\boldsymbol{\gamma}}_{\mathrm{P},W}^{\mathrm{acv}}$, $\widehat{\boldsymbol{\gamma}}_{\mathrm{P},D}^{\mathrm{acv}}$, $\widehat{\boldsymbol{\gamma}}_{\mathrm{P},W}^{\mathrm{int}}$, $\widehat{\boldsymbol{\gamma}}_{\mathrm{P},D}^{\mathrm{int}}$, $\widehat{\boldsymbol{\gamma}}_{\mathrm{P},X}^{\mathrm{adj},W}$, $\widehat{\boldsymbol{\gamma}}_{\mathrm{P},DX}^{\mathrm{adj},W}$, $\widehat{\boldsymbol{\gamma}}_{\mathrm{P},X}^{\mathrm{adj},D}$, and $\widehat{\boldsymbol{\gamma}}_{\mathrm{P},DX}^{\mathrm{adj},D}$, respectively.

**Lemma S16.** *Under Conditions 1 and 2 in the main article, (i)* $\boldsymbol{\gamma}_{\mathrm{P},W}^{\mathrm{acv}} = \boldsymbol{O}(1)$, $\boldsymbol{\gamma}_{\mathrm{P},D}^{\mathrm{acv}} = \boldsymbol{o}(1)$, $\boldsymbol{\gamma}_{\mathrm{P},W}^{\mathrm{int}} = \boldsymbol{O}(1)$, $\boldsymbol{\gamma}_{\mathrm{P},D}^{\mathrm{int}} = \boldsymbol{o}(1)$, $\boldsymbol{\gamma}_{\mathrm{P},X}^{\mathrm{adj},W} = \boldsymbol{O}(1)$, $\boldsymbol{\gamma}_{\mathrm{P},DX}^{\mathrm{adj},W} = \boldsymbol{O}(1)$, $\boldsymbol{\gamma}_{\mathrm{P},X}^{\mathrm{adj},D} = \boldsymbol{o}(1)$, *and* $\boldsymbol{\gamma}_{\mathrm{P},DX}^{\mathrm{adj},D} = \boldsymbol{o}(1)$*; and (ii)* $\widehat{\boldsymbol{\gamma}}_{\mathrm{P},W}^{\mathrm{acv}} - \boldsymbol{\gamma}_{\mathrm{P},W}^{\mathrm{acv}} = \boldsymbol{O}_{\mathbb{P}}(N^{-1/2})$, $\widehat{\boldsymbol{\gamma}}_{\mathrm{P},D}^{\mathrm{acv}} = \boldsymbol{O}_{\mathbb{P}}(N^{-1/2})$, $\widehat{\boldsymbol{\gamma}}_{\mathrm{P},W}^{\mathrm{int}} - \boldsymbol{\gamma}_{\mathrm{P},W}^{\mathrm{int}} = \boldsymbol{O}_{\mathbb{P}}(N^{-1/2})$, $\widehat{\boldsymbol{\gamma}}_{\mathrm{P},D}^{\mathrm{int}} = \boldsymbol{O}_{\mathbb{P}}(N^{-1/2})$, $\widehat{\boldsymbol{\gamma}}_{\mathrm{P},X}^{\mathrm{adj},W} - \boldsymbol{\gamma}_{\mathrm{P},X}^{\mathrm{adj},W} = \boldsymbol{O}_{\mathbb{P}}(N^{-1/2})$, $\widehat{\boldsymbol{\gamma}}_{\mathrm{P},DX}^{\mathrm{adj},W} - \boldsymbol{\gamma}_{\mathrm{P},DX}^{\mathrm{adj},W} = \boldsymbol{O}_{\mathbb{P}}(N^{-1/2})$, $\widehat{\boldsymbol{\gamma}}_{\mathrm{P},X}^{\mathrm{adj},D} = \boldsymbol{O}_{\mathbb{P}}(N^{-1/2})$, $\widehat{\boldsymbol{\gamma}}_{\mathrm{P},DX}^{\mathrm{adj},D} = \boldsymbol{O}_{\mathbb{P}}(N^{-1/2})$.

Then, for $\widehat{\tau}_{\mathrm{P}}^{\mathrm{acv}}$, by Lemmas S2 and S16

$$\begin{aligned}\frac{1}{N(N-1)}\sum_{i\neq j} D_{i,j}\boldsymbol{X}_{i,j}^{\top}\widehat{\boldsymbol{\gamma}}_{\mathrm{P},W}^{\mathrm{acv}} &= \left\{\frac{1}{N(N-1)}\sum_{(i,j)\in\mathcal{S}(a,1-a)}\boldsymbol{X}_{i,j}^{\top} - \frac{1}{N(N-1)}\sum_{(i,j)\in\mathcal{S}(1-a,a)}\boldsymbol{X}_{i,j}^{\top}\right\}\widehat{\boldsymbol{\gamma}}_{\mathrm{P},W}^{\mathrm{acv}} \\ &= \left\{\frac{\pi_1\pi_0}{N(N-1)}\sum_{i\neq j}\boldsymbol{X}_{i,j}^{\top} - \frac{\pi_1\pi_0}{N(N-1)}\sum_{i\neq j}\boldsymbol{X}_{i,j}^{\top} + \boldsymbol{o}_{\mathbb{P}}\left(\frac{1}{N^{1/2}}\right)\right\}\widehat{\boldsymbol{\gamma}}_{\mathrm{P},W}^{\mathrm{acv}} \\ &= \left\{\boldsymbol{0} + \boldsymbol{o}_{\mathbb{P}}\left(\frac{1}{N^{1/2}}\right)\right\}\boldsymbol{O}_{\mathbb{P}}(1) = o_{\mathbb{P}}\left(\frac{1}{N^{1/2}}\right) = o_{\mathbb{P}}(1),\end{aligned}$$

and, similarly,

$$\frac{1}{N(N-1)}\sum_{i\neq j} D_{i,j}\boldsymbol{X}_{i,j}^{\top}\widehat{\boldsymbol{\gamma}}_{\mathrm{P},D}^{\mathrm{acv}} = \boldsymbol{o}_{\mathbb{P}}\left(\frac{1}{N^{1/2}}\right)\boldsymbol{o}_{\mathbb{P}}\left(\frac{1}{N^{1/2}}\right) = o_{\mathbb{P}}\left(\frac{1}{N}\right) = o_{\mathbb{P}}(1). \tag{S1}$$

By Lemma S3,

$$\begin{aligned}\widehat{\tau}_{\mathrm{P}}^{\mathrm{acv}}(a) &= 2\left\{2\pi_1\pi_0 + o_{\mathbb{P}}(1)\right\}^{-1}\left\{\pi_1\pi_0\overline{W}(a,1-a) - \pi_1\pi_0\overline{W}(1-a,a) + o_{\mathbb{P}}(1)\right\} \\ &= \overline{W}(a,1-a) - \overline{W}(1-a,a) + o_{\mathbb{P}}(1) = \tau + o_{\mathbb{P}}(1).\end{aligned}$$

The consistency of $\widehat{\tau}_{\mathrm{P}}^{\mathrm{int}}(a)$ and $\widehat{\tau}_{\mathrm{P}}^{\mathrm{adj}}(a)$ can be achieved by the same argument, and are thus omitted. For the asymptotic normality, by (S1), $\widehat{\tau}_{\mathrm{P}}^{\mathrm{acv}}(a)$ has the same asymptotic distribution as

$$\widehat{\tau}_{\mathrm{P}}^{\mathrm{acv},*}(a) = \overline{W}_{\mathcal{S}(a,1-a)} - \overline{W}_{\mathcal{S}(1-a,a)} - \{\overline{\boldsymbol{X}}_{\mathcal{S}(a,1-a)} - \overline{\boldsymbol{X}}_{\mathcal{S}(1-a,a)}\}^{\top}\widehat{\boldsymbol{\gamma}}_{\mathrm{P},W}^{\mathrm{acv}}.$$

Then, by Lemma S16, we have

$$\widehat{\tau}_{\mathrm{P}}^{\mathrm{acv},*}(a) = \overline{W}_{\mathcal{S}(a,1-a)} - \overline{W}_{\mathcal{S}(1-a,a)} - \{\overline{\boldsymbol{X}}_{\mathcal{S}(a,1-a)} - \overline{\boldsymbol{X}}_{\mathcal{S}(1-a,a)}\}^{\top}\boldsymbol{\gamma}_{\mathrm{P},W}^{\mathrm{acv}} + o_{\mathbb{P}}\left(\frac{1}{N^{1/2}}\right).$$

Similarly, $\widehat{\tau}_{\mathrm{P}}^{\mathrm{int}}(a)$ has the same asymptotic distribution as

$$\widehat{\tau}_{\mathrm{P}}^{\mathrm{int},*}(a) = \overline{W}_{\mathcal{S}(a,1-a)} - \overline{W}_{\mathcal{S}(1-a,a)} - \{\overline{\boldsymbol{X}}_{\mathcal{S}(a,1-a)} + \overline{\boldsymbol{X}}_{\mathcal{S}(1-a,a)}\}^{\top}\widehat{\boldsymbol{\gamma}}_{\mathrm{P},W}^{\mathrm{int}},$$

and

$$\widehat{\tau}_{\mathrm{P}}^{\mathrm{int},*}(a) = \overline{W}_{\mathcal{S}(a,1-a)} - \overline{W}_{\mathcal{S}(1-a,a)} - \{\overline{\boldsymbol{X}}_{\mathcal{S}(a,1-a)} + \overline{\boldsymbol{X}}_{\mathcal{S}(1-a,a)}\}^\top \boldsymbol{\gamma}_{\mathrm{P},W}^{\mathrm{int}} + o_{\mathbb{P}}\left(\frac{1}{N^{1/2}}\right).$$

For $\widehat{\tau}_{\mathrm{P}}^{\mathrm{adj}}(a)$, it has the same asymptotic distribution as

$$\widehat{\tau}_{\mathrm{P}}^{\mathrm{adj},*}(a) = \overline{W}_{\mathcal{S}(a,1-a)} - \overline{W}_{\mathcal{S}(1-a,a)} - \overline{\boldsymbol{X}}_{\mathcal{S}(a,1-a)}^\top\left(\widehat{\boldsymbol{\gamma}}_{\mathrm{P},DX}^{\mathrm{adj},W} + \widehat{\boldsymbol{\gamma}}_{\mathrm{P},X}^{\mathrm{adj},W}\right) - \overline{\boldsymbol{X}}_{\mathcal{S}(1-a,a)}^\top\left(\widehat{\boldsymbol{\gamma}}_{\mathrm{P},DX}^{\mathrm{adj},W} - \widehat{\boldsymbol{\gamma}}_{\mathrm{P},X}^{\mathrm{adj},W}\right),$$

and

$$\widehat{\tau}_{\mathrm{P}}^{\mathrm{adj},*}(a) = \overline{W}_{\mathcal{S}(a,1-a)} - \overline{W}_{\mathcal{S}(1-a,a)} - \overline{\boldsymbol{X}}_{\mathcal{S}(a,1-a)}^\top\left(\widehat{\boldsymbol{\gamma}}_{\mathrm{P},DX}^{\mathrm{adj},W} + \widehat{\boldsymbol{\gamma}}_{\mathrm{P},X}^{\mathrm{adj},W}\right) - \overline{\boldsymbol{X}}_{\mathcal{S}(1-a,a)}^\top\left(\widehat{\boldsymbol{\gamma}}_{\mathrm{P},DX}^{\mathrm{adj},W} - \widehat{\boldsymbol{\gamma}}_{\mathrm{P},X}^{\mathrm{adj},W}\right) + o_{\mathbb{P}}\left(\frac{1}{N^{1/2}}\right).$$

Thus, the asymptotic normality of $\widehat{\tau}_{\mathrm{P}}^{\mathrm{acv},*}(a)$ and $\widehat{\tau}_{\mathrm{P}}^{\mathrm{int},*}(a)$ is implied by that of $\widehat{\lambda}_{\mathrm{I}}^{\mathrm{acv}}(a,1-a)$, and the asymptotic normality of $\widehat{\tau}_{\mathrm{P}}^{\mathrm{adj},*}(a)$ is implied by that of $\widehat{\lambda}_{\mathrm{I}}^{\mathrm{adj}}(a,1-a)$.

## S4.2 Asymptotic variances

We derive the leading terms of $\mathbb{V}\mathrm{ar}\{\widehat{\tau}_{\mathrm{P}}^{\mathrm{adj}}(a)\}$, and $\mathbb{V}\mathrm{ar}\{\widehat{\tau}_{\mathrm{P}}(a)\}$. $\mathbb{V}\mathrm{ar}\{\widehat{\tau}_{\mathrm{P}}^{\mathrm{adj}}(a)\}$, and $\mathbb{V}\mathrm{ar}\{\widehat{\tau}_{\mathrm{P}}^{\mathrm{int}}(a)\}$ follow closely. Since $\widehat{\tau}_{\mathrm{P}}^{\mathrm{adj}}(a)$ has the same asymptotic distribution as $\widehat{\tau}_{\mathrm{P}}^{\mathrm{adj},*}(a)$, it suffices to derive the leading terms of $\mathbb{V}\mathrm{ar}\{\widehat{\tau}_{\mathrm{P}}^{\mathrm{adj},*}(a)\}$. Following our previous derivations of $\mathbb{V}\mathrm{ar}\{\widehat{\lambda}_{\mathrm{I}}(a,1-a)\}$, we have

$$\widehat{\tau}_{\mathrm{P}}^{\mathrm{adj},*}(a) - \tau(a) = \frac{1}{N_1N_0}\sum_{(i,j)\in\mathcal{S}(a,1-a)} r_{\mathrm{P},i,j}^{\mathrm{adj}}(a,1-a) - \frac{1}{N_1N_0}\sum_{(i,j)\in\mathcal{S}(1-a,a)} r_{\mathrm{P},i,j}^{\mathrm{adj}}(1-a,a) + O_{\mathbb{P}}\left(\frac{1}{N}\right),$$

where

$$\begin{aligned}
r_{\mathrm{P},i,j}^{\mathrm{adj}}(a,1-a) &= W_{i,j}(a,1-a) - \overline{W}(a,1-a) - \boldsymbol{X}_{i,j}^\top\left(\widehat{\boldsymbol{\gamma}}_{\mathrm{P},X}^{\mathrm{adj},W} + \widehat{\boldsymbol{\gamma}}_{\mathrm{P},DX}^{\mathrm{adj},W}\right),\\
r_{\mathrm{P},i,j}^{\mathrm{adj}}(1-a,a) &= W_{i,j}(1-a,a) - \overline{W}(1-a,a) - \boldsymbol{X}_{i,j}^\top\left(\widehat{\boldsymbol{\gamma}}_{\mathrm{P},X}^{\mathrm{adj},W} - \widehat{\boldsymbol{\gamma}}_{\mathrm{P},DX}^{\mathrm{adj},W}\right).
\end{aligned}$$

Then, applying the Hoeffding decomposition arguments in the proof of Lemma S7, we have

$$\widehat{\tau}_{\mathrm{P}}^{\mathrm{adj}}(a) - \tau(a) = \Psi_{\mathrm{P}}^{\mathrm{adj},*}(a) + O_{\mathbb{P}}\left(\frac{1}{N}\right),$$

where

$$\begin{aligned}
\Psi_{\mathrm{P}}^{\mathrm{adj},*}(a) = \frac{1}{N}\sum_{i=1}^{N}\Bigg\{&\frac{1}{\pi_a}\overline{r}_{\mathrm{P},i,\cdot}^{\mathrm{adj}}(a,1-a)\mathbb{1}_i(a) - \frac{1}{\pi_a}\overline{r}_{\mathrm{P},\cdot,i}^{\mathrm{adj}}(1-a,a)\mathbb{1}_i(a)\\
&+\frac{1}{\pi_{1-a}}\overline{r}_{\mathrm{P},\cdot,i}^{\mathrm{adj}}(a,1-a)\mathbb{1}_i(1-a) - \frac{1}{\pi_{1-a}}\overline{r}_{\mathrm{P},i,\cdot}^{\mathrm{adj}}(1-a,a)\mathbb{1}_i(1-a)\Bigg\},
\end{aligned}$$

with

$$\begin{aligned}
\overline{r}_{\mathrm{P},i,\cdot}^{\mathrm{adj}}(a,1-a) &= \frac{1}{N-1}\sum_{j:j\neq i} r_{\mathrm{P},i,j}^{\mathrm{adj}}(a,1-a), \quad \overline{r}_{\mathrm{P},\cdot,i}^{\mathrm{adj}}(a,1-a) = \frac{1}{N-1}\sum_{j:j\neq i} r_{\mathrm{P},j,i}^{\mathrm{adj}}(a,1-a),\\
\overline{r}_{\mathrm{P},i,\cdot}^{\mathrm{adj}}(1-a,a) &= \frac{1}{N-1}\sum_{j:j\neq i} r_{\mathrm{P},i,j}^{\mathrm{adj}}(1-a,a), \quad \overline{r}_{\mathrm{P},\cdot,i}^{\mathrm{adj}}(1-a,a) = \frac{1}{N-1}\sum_{j:j\neq i} r_{\mathrm{P},j,i}^{\mathrm{adj}}(1-a,a).
\end{aligned}$$

Thus, under complete randomization,

$$\begin{aligned}\mathbb{V}\text{ar}\left\{\Psi_{\mathrm{P}}^{\mathrm{adj},*}(a)\right\} &= \frac{1}{\pi_a N}\cdot\frac{1}{N-1}\sum_{i=1}^{N}\left\{\overline{r}_{\mathrm{P},i,\cdot}^{\mathrm{adj}}(a,1-a)-\overline{r}_{\mathrm{P},\cdot,i}^{\mathrm{adj}}(1-a,a)\right\}^2\\ &+\frac{1}{\pi_{1-a}N}\cdot\frac{1}{N-1}\sum_{i=1}^{N}\left\{\overline{r}_{\mathrm{P},i,\cdot}^{\mathrm{adj}}(1-a,a)-\overline{r}_{\mathrm{P},\cdot,i}^{\mathrm{adj}}(a,1-a)\right\}^2\\ &-\frac{1}{N}\cdot\frac{1}{N-1}\sum_{i=1}^{N}\left[\left\{\overline{r}_{\mathrm{P},i,\cdot}^{\mathrm{adj}}(a,1-a)-\overline{r}_{\mathrm{P},\cdot,i}^{\mathrm{adj}}(1-a,a)\right\}+\left\{\overline{r}_{\mathrm{P},i,\cdot}^{\mathrm{adj}}(1-a,a)-\overline{r}_{\mathrm{P},\cdot,i}^{\mathrm{adj}}(a,1-a)\right\}\right]^2.\end{aligned}$$

By the proof of Lemma S16, we have

$$\boldsymbol{\gamma}_{\mathrm{P},X}^{\mathrm{adj},W}=\boldsymbol{\gamma}_{\mathrm{P},W}^{\mathrm{acv}}=\boldsymbol{\gamma}_{\mathrm{I}}^{\mathrm{acv}},\quad \boldsymbol{\gamma}_{\mathrm{P},DX}^{\mathrm{adj},W}=\boldsymbol{\gamma}_{\mathrm{P},W}^{\mathrm{int}}.$$

Then, for $\widehat{\tau}_{\mathrm{P}}^{\mathrm{int}}(a)$,

$$\begin{aligned}&\overline{r}_{\mathrm{P},i,\cdot}^{\mathrm{int}}(a,1-a)-\overline{r}_{\mathrm{P},\cdot,i}^{\mathrm{int}}(1-a,a)\\ &=\left\{\overline{W}_{i,\cdot}(a,1-a)-\overline{W}(a,1-a)-\overline{X}_{i,\cdot}^{\top}\boldsymbol{\gamma}_{\mathrm{P},W}^{\mathrm{int}}\right\}-\left\{\overline{W}_{\cdot,i}(1-a,a)-\overline{W}(1-a,a)+\overline{X}_{\cdot,i}^{\top}\boldsymbol{\gamma}_{\mathrm{P},W}^{\mathrm{int}}\right\}\\ &=\overline{W}_{i,\cdot}(a,1-a)-\overline{W}(a,1-a)-\overline{X}_{i,\cdot}^{\top}\boldsymbol{\gamma}_{\mathrm{P},W}^{\mathrm{int}}-\overline{W}_{\cdot,i}(1-a,a)+\overline{W}(1-a,a)-\overline{X}_{\cdot,i}^{\top}\boldsymbol{\gamma}_{\mathrm{P},W}^{\mathrm{int}}\\ &=\overline{W}_{i,\cdot}(a,1-a)-\overline{W}(a,1-a)-\overline{X}_{i,\cdot}^{\top}\boldsymbol{\gamma}_{\mathrm{P},W}^{\mathrm{int}}-\overline{W}_{\cdot,i}(1-a,a)+\overline{W}(1-a,a)+\overline{X}_{i,\cdot}^{\top}\boldsymbol{\gamma}_{\mathrm{P},W}^{\mathrm{int}}\\ &=\overline{W}_{i,\cdot}(a,1-a)-\overline{W}(a,1-a)-\overline{W}_{\cdot,i}(1-a,a)+\overline{W}(1-a,a)\\ &=\overline{\epsilon}_{i,\cdot}(a,1-a)-\overline{\epsilon}_{\cdot,i}(1-a,a).\end{aligned}$$

Hence, $\widehat{\tau}_{\mathrm{P}}^{\mathrm{int}}(a)$ and $\widehat{\tau}_{\mathrm{I}}(a)=\widehat{\lambda}_{\mathrm{I}}(a,1-a)-\widehat{\lambda}_{\mathrm{I}}(1-a,a)$ are asymptotically equivalent. Similarly, for $\widehat{\tau}_{\mathrm{P}}^{\mathrm{adj}}(a)$, we have

$$\overline{r}_{\mathrm{P},i,\cdot}^{\mathrm{adj}}(a,1-a)-\overline{r}_{\mathrm{P},\cdot,i}^{\mathrm{adj}}(1-a,a)=\overline{r}_{\mathrm{P},i,\cdot}^{\mathrm{acv}}(a,1-a)-\overline{r}_{\mathrm{P},\cdot,i}^{\mathrm{acv}}(1-a,a).$$

Thus, $\widehat{\tau}_{\mathrm{P}}^{\mathrm{adj}}(a)$, $\widehat{\tau}_{\mathrm{P}}^{\mathrm{acv}}(a)$, and $\widehat{\tau}_{\mathrm{I}}^{\mathrm{acv}}(a)$ are asymptotically equivalent.

# S5 Variance results

## S5.1 Estimators using individual pairs

### S5.1.1 The heteroskedasticity-robust variance estimators

We first show that heteroskedasticity-robust (HR) variance estimators are not consistent for estimators using individual pairs. We focus on $\widehat{\lambda}_{\mathrm{I}}^{\mathrm{adj}}(a,1-a)$ estimators, and other estimators follow closely. Let $\boldsymbol{I}_{i,j}=(A_i(1-A_j),A_j(1-A_i))^{\top}$ and $\boldsymbol{J}_{i,j}=\boldsymbol{I}_{i,j}\otimes\boldsymbol{X}_{i,j}$, where '$\otimes$' is the Kronecker product. Then, $\boldsymbol{Z}_{\mathrm{I},i,j}^{\mathrm{adj}\top}=(\boldsymbol{I}_{i,j}^{\top},\boldsymbol{J}_{i,j}^{\top})$. Thus,

$$\boldsymbol{Z}_{\mathrm{I},i,j}^{\mathrm{adj}}\boldsymbol{Z}_{\mathrm{I},i,j}^{\mathrm{adj}\top}=\begin{pmatrix}\boldsymbol{I}_{i,j}\\ \boldsymbol{J}_{i,j}\end{pmatrix}\begin{pmatrix}\boldsymbol{I}_{i,j}^{\top} & \boldsymbol{J}_{i,j}^{\top}\end{pmatrix}=\begin{pmatrix}\boldsymbol{I}_{i,j}\boldsymbol{I}_{i,j}^{\top} & \boldsymbol{I}_{i,j}\boldsymbol{J}_{i,j}^{\top}\\ \boldsymbol{J}_{i,j}\boldsymbol{I}_{i,j}^{\top} & \boldsymbol{J}_{i,j}\boldsymbol{J}_{i,j}^{\top}\end{pmatrix}.$$

Then, define

$$\mathbf{G}_{\mathrm{I}}^{\mathrm{adj}}=\frac{1}{N(N-1)}\mathbf{Z}_{\mathrm{I}}^{\mathrm{adj}\top}\mathbf{Z}_{\mathrm{I}}^{\mathrm{adj}}=\frac{1}{N(N-1)}\sum_{i\neq j}\boldsymbol{Z}_{\mathrm{I},i,j}^{\mathrm{adj}}\boldsymbol{Z}_{\mathrm{I},i,j}^{\mathrm{adj}\top}=\begin{pmatrix}\mathbf{G}_{\mathrm{I},(1,1)}^{\mathrm{adj}} & \mathbf{G}_{\mathrm{I},(1,2)}^{\mathrm{adj}}\\ \mathbf{G}_{\mathrm{I},(1,2)}^{\mathrm{adj}\top} & \mathbf{G}_{\mathrm{I},(2,2)}^{\mathrm{adj}}\end{pmatrix},\tag{S2}$$

where

$$\mathbf{G}^{\text{adj}}_{\text{I},(1,1)} = \frac{1}{N(N-1)} \begin{pmatrix} N_1 N_0 & 0 \\ 0 & N_1 N_0 \end{pmatrix}, \quad \mathbf{G}^{\text{adj}}_{\text{I},(1,2)} = \frac{1}{N(N-1)} \begin{pmatrix} \sum_{(i,j)\in\mathcal{S}(1,0)} \boldsymbol{X}_{i,j}^\top & \mathbf{0} \\ \mathbf{0} & \sum_{(i,j)\in\mathcal{S}(0,1)} \boldsymbol{X}_{i,j}^\top \end{pmatrix},$$

and

$$\mathbf{G}^{\text{adj}}_{\text{I},(2,2)} = \frac{1}{N(N-1)} \begin{pmatrix} \sum_{(i,j)\in\mathcal{S}(1,0)} \boldsymbol{X}_{i,j}\boldsymbol{X}_{i,j}^\top & \mathbf{0} \\ \mathbf{0} & \sum_{(i,j)\in\mathcal{S}(0,1)} \boldsymbol{X}_{i,j}\boldsymbol{X}_{i,j}^\top \end{pmatrix}.$$

For the HR variance estimator, define

$$\overline{\mathbf{M}}^{\text{adj}}_{\text{I,HR}} = \frac{1}{N(N-1)} \sum_{i\neq j} \mathbf{M}^{\text{adj}}_{\text{I,HR},i,j} = \frac{1}{N(N-1)} \sum_{i\neq j} \boldsymbol{Z}^{\text{adj}}_{\text{I},i,j} \boldsymbol{Z}^{\text{adj}\top}_{\text{I},i,j} (\widehat{r}^{\text{adj}}_{\text{I},i,j})^2,$$

where

$$\mathbf{M}^{\text{adj}}_{\text{I,HR},i,j} = \begin{pmatrix} \boldsymbol{I}_{i,j}\boldsymbol{I}_{i,j}^\top & \boldsymbol{I}_{i,j}\boldsymbol{J}_{i,j}^\top \\ * & \boldsymbol{J}_{i,j}\boldsymbol{J}_{i,j}^\top \end{pmatrix} (\widehat{r}^{\text{adj}}_{\text{I},i,j})^2,$$

where $*$ indicates the symmetric components. Specifically,

$$\begin{aligned}
\boldsymbol{I}_{i,j}\boldsymbol{I}_{i,j}^\top (\widehat{r}^{\text{adj}}_{\text{I},i,j})^2 &= \begin{pmatrix} A_i(1-A_j)(\widehat{r}^{\text{adj}}_{\text{I},i,j})^2 & 0 \\ 0 & (1-A_i)A_j(\widehat{r}^{\text{adj}}_{\text{I},i,j})^2 \end{pmatrix}, \\
\boldsymbol{I}_{i,j}\boldsymbol{J}_{i,j}^\top (\widehat{r}^{\text{adj}}_{\text{I},i,j})^2 &= \begin{pmatrix} A_i(1-A_j)\boldsymbol{X}_{i,j}^\top(\widehat{r}^{\text{adj}}_{\text{I},i,j})^2 & \mathbf{0} \\ \mathbf{0} & (1-A_i)A_j\boldsymbol{X}_{i,j}^\top(\widehat{r}^{\text{adj}}_{\text{I},i,j})^2 \end{pmatrix}, \\
\boldsymbol{J}_{i,j}\boldsymbol{J}_{i,j}^\top (\widehat{r}^{\text{adj}}_{\text{I},i,j})^2 &= \begin{pmatrix} A_i(1-A_j)\boldsymbol{X}_{i,j}\boldsymbol{X}_{i,j}^\top(\widehat{r}^{\text{adj}}_{\text{I},i,j})^2 & \mathbf{0} \\ \mathbf{0} & (1-A_i)A_j\boldsymbol{X}_{i,j}\boldsymbol{X}_{i,j}^\top(\widehat{r}^{\text{adj}}_{\text{I},i,j})^2 \end{pmatrix}.
\end{aligned}$$

We have the following lemma regarding orders of the terms.

**Lemma S17.** *Under Conditions 1-3 in the main article, then*

$$\frac{1}{N(N-1)} \sum_{i\neq j} A_i(1-A_j)(\widehat{r}^{\text{adj}}_{\text{I},i,j})^2 - \frac{\pi_1\pi_0}{N(N-1)} \sum_{i\neq j} r^{\text{adj}}_{\text{I},i,j}(1,0)^2 = o_{\mathbb{P}}(1), \tag{S3}$$

$$\frac{1}{N(N-1)} \sum_{i\neq j} A_i(1-A_j)\boldsymbol{X}_{i,j}^\top(\widehat{r}^{\text{adj}}_{\text{I},i,j})^2 = \boldsymbol{O}_{\mathbb{P}}(1), \tag{S4}$$

$$\frac{1}{N(N-1)} \sum_{i\neq j} A_i(1-A_j)\boldsymbol{X}_{i,j}\boldsymbol{X}_{i,j}^\top(\widehat{r}^{\text{adj}}_{\text{I},i,j})^2 = \boldsymbol{O}_{\mathbb{P}}(1). \tag{S5}$$

*Similar results can be obtained for the* $(1-A_i)A_j$ *pairing.*

By Lemma S17, $\overline{\mathbf{M}}^{\text{adj}}_{\text{I,HR}} = \boldsymbol{O}_{\mathbb{P}}(1)$. We now analyze the HR variance estimators. Specifically, we have

$$N(N-1)\widehat{\text{se}}^2_{\text{HR}}\left\{\widehat{\lambda}^{\text{adj}}_{\text{I}}(1,0)\right\} = \left[(\boldsymbol{G}^{\text{adj}}_{\text{I}})^{-1}\overline{\mathbf{M}}^{\text{adj}}_{\text{I,HR}}(\boldsymbol{G}^{\text{adj}}_{\text{I}})^{-1}\right]_{(1,1)}.$$

Define

$$\boldsymbol{\Gamma}_{\mathrm{I}}^{\mathrm{adj}} = \begin{pmatrix} \boldsymbol{\Gamma}_{\mathrm{I},(1,1)}^{\mathrm{adj}} & \mathbf{0} \\ \mathbf{0} & \boldsymbol{\Gamma}_{\mathrm{I},(2,2)}^{\mathrm{adj}} \end{pmatrix}, \tag{S6}$$

where

$$\boldsymbol{\Gamma}_{\mathrm{I},(1,1)}^{\mathrm{adj}} = \begin{pmatrix} \pi_1\pi_0 & 0 \\ 0 & \pi_1\pi_0 \end{pmatrix}, \quad \boldsymbol{\Gamma}_{\mathrm{I},(2,2)}^{\mathrm{adj}} = \frac{\pi_1\pi_0}{N(N-1)} \sum_{i \neq j} \begin{pmatrix} \boldsymbol{X}_{i,j}\boldsymbol{X}_{i,j}^\top & \mathbf{0} \\ \mathbf{0} & \boldsymbol{X}_{i,j}\boldsymbol{X}_{i,j}^\top \end{pmatrix}.$$

as the expectation of $\mathbf{G}_{\mathrm{I}}^{\mathrm{adj}}$. Define $\boldsymbol{\Lambda}_{\mathrm{I}}^{\mathrm{adj}} = \mathbf{G}_{\mathrm{I}}^{\mathrm{adj}} - \boldsymbol{\Gamma}_{\mathrm{I}}^{\mathrm{adj}}$ and $\boldsymbol{\Omega}_{\mathrm{I}}^{\mathrm{adj}} = (\mathbf{G}_{\mathrm{I}}^{\mathrm{adj}})^{-1} - (\boldsymbol{\Gamma}_{\mathrm{I}}^{\mathrm{adj}})^{-1}$. By Lemma S2, $\boldsymbol{\Lambda}_{\mathrm{I}}^{\mathrm{adj}} = \boldsymbol{O}_{\mathbb{P}}(N^{-1/2})$, and by Lemma S3, $\boldsymbol{\Omega}_{\mathrm{I}}^{\mathrm{adj}} = \boldsymbol{O}_{\mathbb{P}}(N^{-1/2})$. Therefore,

$$\begin{aligned}
&(\mathbf{G}_{\mathrm{I}}^{\mathrm{adj}})^{-1}\overline{\mathbf{M}}_{\mathrm{I,HR}}^{\mathrm{adj}}(\mathbf{G}_{\mathrm{I}}^{\mathrm{adj}})^{-1} - (\boldsymbol{\Gamma}_{\mathrm{I}}^{\mathrm{adj}})^{-1}\overline{\mathbf{M}}_{\mathrm{I,HR}}^{\mathrm{adj}}(\boldsymbol{\Gamma}_{\mathrm{I}}^{\mathrm{adj}})^{-1} \\
&= \left\{(\boldsymbol{\Gamma}_{\mathrm{I}}^{\mathrm{adj}})^{-1} + \boldsymbol{\Omega}_{\mathrm{I}}^{\mathrm{adj}}\right\} \overline{\mathbf{M}}_{\mathrm{I,HR}}^{\mathrm{adj}} \left\{(\boldsymbol{\Gamma}_{\mathrm{I}}^{\mathrm{adj}})^{-1} + \boldsymbol{\Omega}_{\mathrm{I}}^{\mathrm{adj}}\right\} - (\boldsymbol{\Gamma}_{\mathrm{I}}^{\mathrm{adj}})^{-1}\overline{\mathbf{M}}_{\mathrm{I,HR}}^{\mathrm{adj}}(\boldsymbol{\Gamma}_{\mathrm{I}}^{\mathrm{adj}})^{-1} \\
&= \boldsymbol{\Omega}_{\mathrm{I}}^{\mathrm{adj}}\overline{\mathbf{M}}_{\mathrm{I,HR}}^{\mathrm{adj}}(\boldsymbol{\Gamma}_{\mathrm{I}}^{\mathrm{adj}})^{-1} + (\boldsymbol{\Gamma}_{\mathrm{I}}^{\mathrm{adj}})^{-1}\overline{\mathbf{M}}_{\mathrm{I,HR}}^{\mathrm{adj}}\boldsymbol{\Omega}_{\mathrm{I}}^{\mathrm{adj}} + \boldsymbol{\Omega}_{\mathrm{I}}^{\mathrm{adj}}\overline{\mathbf{M}}_{\mathrm{I,HR}}^{\mathrm{adj}}\boldsymbol{\Omega}_{\mathrm{I}}^{\mathrm{adj}} \\
&= \boldsymbol{O}_{\mathbb{P}}\left(\frac{1}{N^{1/2}}\right)\boldsymbol{O}_{\mathbb{P}}(1)\boldsymbol{O}_{\mathbb{P}}(1) + \boldsymbol{O}_{\mathbb{P}}(1)\boldsymbol{O}_{\mathbb{P}}(1)\boldsymbol{O}_{\mathbb{P}}\left(\frac{1}{N^{1/2}}\right) + \boldsymbol{O}_{\mathbb{P}}\left(\frac{1}{N^{1/2}}\right)\boldsymbol{O}_{\mathbb{P}}(1)\boldsymbol{O}_{\mathbb{P}}\left(\frac{1}{N^{1/2}}\right) = \boldsymbol{o}_{\mathbb{P}}(1).
\end{aligned}$$

Then, by Lemma S17,

$$\begin{aligned}
N(N-1)\widehat{\mathrm{se}}_{\mathrm{HR}}^2\left\{\widehat{\lambda}_{\mathrm{I}}^{\mathrm{adj}}(1,0)\right\} &= \left[(\boldsymbol{\Gamma}_{\mathrm{I}}^{\mathrm{adj}})^{-1}\overline{\mathbf{M}}_{\mathrm{I,HR}}^{\mathrm{adj}}(\boldsymbol{\Gamma}_{\mathrm{I}}^{\mathrm{adj}})^{-1}\right]_{(1,1)} + o_{\mathbb{P}}(1) \\
&= \frac{1}{N(N-1)} \cdot \frac{1}{\pi_1^2\pi_0^2}\sum_{i\neq j} A_i(1-A_j)(\widehat{r}_{\mathrm{I},i,j}^{\mathrm{adj}})^2 + o_{\mathbb{P}}(1) = \frac{1}{\pi_1\pi_0 N(N-1)}\sum_{i\neq j} r_{\mathrm{I},i,j}^{\mathrm{adj}}(1,0)^2 + o_{\mathbb{P}}(1).
\end{aligned}$$

The probability limit of $N(N-1)\widehat{\mathrm{se}}_{\mathrm{HR}}^2\{\widehat{\lambda}_{\mathrm{I}}^{\mathrm{adj}}(1,0)\}$ is not $V\{\overline{r}_{\mathrm{I},i}^{\mathrm{adj}}(1,0)\}$ or $V_c\{\overline{r}_{\mathrm{I},i}^{\mathrm{adj}}(1,0)\}$.

#### S5.1.2 The cluster-robust variance estimators

We then show that the cluster-robust (CR) variance estimators are not consistent for estimators using individual pairs. Similarly, we focus on $\widehat{\lambda}_{\mathrm{I}}^{\mathrm{adj}}(a,1-a)$. Stack $\boldsymbol{Z}_{\mathrm{I},i,j}^\top$ together to obtain matrix $\mathbf{Z}_{\mathrm{I},i}^{\mathrm{adj}}$, and stack $\mathbf{Z}_{\mathrm{I},i}^{\mathrm{adj}}$ together to obtain design matrix $\mathbf{Z}_{\mathrm{I}}^{\mathrm{adj}}$. For the CR variance estimator, define

$$\overline{\mathbf{M}}_{\mathrm{I,CR}}^{\mathrm{adj}} = \frac{1}{N(N-1)^2}\sum_{i=1}^N \mathbf{M}_{\mathrm{I,CR},i}^{\mathrm{adj}} = \frac{1}{N(N-1)^2}\sum_{i=1}^N \mathbf{Z}_{\mathrm{I},i}^{\mathrm{adj}\top}\widehat{\mathbf{R}}_{\mathrm{I},i}^{\mathrm{adj}}\mathbf{Z}_{\mathrm{I},i}^{\mathrm{adj}},$$

where $\widehat{\mathbf{R}}_{\mathrm{I},i}^{\mathrm{adj}}$ is an $(N-1)\times(N-1)$ matrix with $[\widehat{\mathbf{R}}_{\mathrm{I},i}^{\mathrm{adj}}]_{(j,k)} = \widehat{r}_{\mathrm{I},i,j}^{\mathrm{adj}}\widehat{r}_{\mathrm{I},i,k}^{\mathrm{adj}}$ for $j\neq i, k\neq i$.

**Lemma S18.** $\mathrm{M}_{\mathrm{I,CR},i}^{\mathrm{adj}}$ *is symmetric and*

$$\begin{aligned}
&\mathbf{M}_{\mathrm{I,CR},i}^{\mathrm{adj}} \\
&= \begin{pmatrix}
A_i U_{\mathrm{I,CR},i}^{\mathrm{adj}}(0)^2 & 0 & A_i U_{\mathrm{I,CR},i}^{\mathrm{adj}}(0)\boldsymbol{L}_{\mathrm{I,CR},i}^{\mathrm{adj}}(0)^\top & \mathbf{0} \\
0 & (1-A_i)U_{\mathrm{I,CR},i}^{\mathrm{adj}}(1)^2 & \mathbf{0} & (1-A_i)U_{\mathrm{I,CR},i}^{\mathrm{adj}}(1)\boldsymbol{L}_{\mathrm{I,CR},i}(1)^\top \\
A_i U_{\mathrm{I,CR},i}^{\mathrm{adj}}(0)\boldsymbol{L}_{\mathrm{I,CR},i}^{\mathrm{adj}}(0) & \mathbf{0} & A_i \boldsymbol{L}_{\mathrm{I,CR},i}^{\mathrm{adj}}(0)\boldsymbol{L}_{\mathrm{I,CR},i}^{\mathrm{adj}}(0)^\top & \mathbf{0} \\
\mathbf{0} & (1-A_i)U_{\mathrm{I,CR},i}^{\mathrm{adj}}(1)\boldsymbol{L}_{\mathrm{I,CR},i}^{\mathrm{adj}}(1) & \mathbf{0} & (1-A_i)\boldsymbol{L}_{\mathrm{I,CR},i}^{\mathrm{adj}}(1)\boldsymbol{L}_{\mathrm{I,CR},i}^{\mathrm{adj}}(1)^\top
\end{pmatrix},
\end{aligned}$$

*where*

$$U^{\text{adj}}_{\text{I,CR},i}(1) = \sum_{j:j\neq i} A_j \widehat{r}^{\text{adj}}_{\text{I},i,j}, \quad U^{\text{adj}}_{\text{I,CR},i}(0) = \sum_{j:j\neq i} (1-A_j)\widehat{r}^{\text{adj}}_{\text{I},i,j},$$
$$\boldsymbol{L}^{\text{adj}}_{\text{I,CR},i}(1) = \sum_{j:j\neq i} A_j \boldsymbol{X}_{i,j}\widehat{r}^{\text{adj}}_{\text{I},i,j}, \quad \boldsymbol{L}^{\text{adj}}_{\text{I,CR},i}(0) = \sum_{j:j\neq i} (1-A_j)\boldsymbol{X}_{i,j}\widehat{r}^{\text{adj}}_{\text{I},i,j}.$$

**Lemma S19.** *Under Conditions 1-3 in the main article, then*

$$\frac{1}{N(N-1)^2}\sum_{i=1}^N A_i \left\{\sum_{j:j\neq i}(1-A_j)\widehat{r}^{\text{adj}}_{\text{I},i,j}\right\}^2 - \frac{\pi_1\pi_0^2}{N}\sum_{i=1}^N r^{\text{adj}}_{\text{I},i,\cdot}(1,0)^2 = o_{\mathbb{P}}(1), \tag{S7}$$

$$\frac{1}{N(N-1)^2}\sum_{i=1}^N A_i \sum_{j:j\neq i}(1-A_j)\widehat{r}^{\text{adj}}_{\text{I},i,j}\sum_{j:j\neq i}(1-A_j)\boldsymbol{X}^\top_{i,j}\widehat{r}^{\text{adj}}_{\text{I},i,j} = \boldsymbol{O}_{\mathbb{P}}(1), \tag{S8}$$

$$\frac{1}{N(N-1)^2}\sum_{i=1}^N A_i \sum_{j:j\neq i}(1-A_j)\boldsymbol{X}_{i,j}\widehat{r}^{\text{adj}}_{\text{I},i,j}\sum_{j:j\neq i}(1-A_j)\boldsymbol{X}^\top_{i,j}\widehat{r}^{\text{adj}}_{\text{I},i,j} = \boldsymbol{O}_{\mathbb{P}}(1). \tag{S9}$$

*Similar results can be obtained for the* $(1-A_i)A_j$ *pairing.*

By Lemma S19, $\overline{\mathbf{M}}^{\text{adj}}_{\text{I,CR}} = \boldsymbol{O}_{\mathbb{P}}(1)$. We now analyze the CR variance estimators. Specifically, we have

$$N\widehat{\text{se}}^2_{\text{CR}}\left\{\widehat{\lambda}^{\text{adj}}_{\text{I}}(1,0)\right\} = \left[(\mathbf{G}^{\text{adj}}_{\text{I}})^{-1}\overline{\mathbf{M}}^{\text{adj}}_{\text{I,CR}}(\mathbf{G}^{\text{adj}}_{\text{I}})^{-1}\right]_{(1,1)},$$

where $\mathbf{G}^{\text{adj}}_{\text{I}}$ is given in (S2). Using similar arguments in the proof of the HR variance estimators, we have

$$(\mathbf{G}^{\text{adj}}_{\text{I}})^{-1}\overline{\mathbf{M}}^{\text{adj}}_{\text{I,CR}}(\mathbf{G}^{\text{adj}}_{\text{I}})^{-1} - (\boldsymbol{\Gamma}^{\text{adj}}_{\text{I}})^{-1}\overline{\mathbf{M}}^{\text{adj}}_{\text{I,CR}}(\boldsymbol{\Gamma}^{\text{adj}}_{\text{I}})^{-1} = \boldsymbol{o}_{\mathbb{P}}(1),$$

where $\boldsymbol{\Gamma}^{\text{adj}}_{\text{I}}$ is defined in (S6). Then, by Lemma S19,

$$\begin{aligned}N\widehat{\text{se}}^2_{\text{CR}}\left\{\widehat{\lambda}^{\text{adj}}_{\text{I}}(1,0)\right\} &= \left[(\boldsymbol{\Gamma}^{\text{adj}}_{\text{I}})^{-1}\overline{\mathbf{M}}^{\text{adj}}_{\text{I,CR}}(\boldsymbol{\Gamma}^{\text{adj}}_{\text{I}})^{-1}\right]_{(1,1)} + o_{\mathbb{P}}(1)\\ &= \frac{1}{N(N-1)^2}\cdot\frac{1}{\pi_1^2\pi_0^2}\sum_{i=1}^N A_i\left\{\sum_{j:j\neq i}(1-A_j)\widehat{r}^{\text{adj}}_{\text{I},i,j}\right\}^2 + o_{\mathbb{P}}(1) = \frac{1}{\pi_1 N}\sum_{i=1}^N \overline{r}^{\text{adj}}_{\text{I},i,\cdot}(1,0)^2 + o_{\mathbb{P}}(1).\end{aligned}$$

The probability limit of $N\widehat{\text{se}}^2_{\text{CR}}\{\widehat{\lambda}^{\text{adj}}_{\text{I}}(1,0)\}$ is not $V\{\overline{r}^{\text{adj}}_{\text{I},i}(1,0)\}$ or $V_c\{\overline{r}^{\text{adj}}_{\text{I},i}(1,0)\}$.

### S5.1.3 The standard two-way clustering variance estimators

We show that the standard two-way (TW) variance estimators are asymptotically conservative for the leading terms of the marginal variances but omit the covariances. We, again, focus on $\widehat{\lambda}^{\text{adj}}_{\text{I}}(a,1-a)$. We continue with the $\mathbf{Z}^{\text{adj}}_{\text{I}}$ design matrix for the CR variance estimators. For the TW variance estimator, the middle matrix

$$\begin{aligned}\mathbf{M}^{\text{adj}}_{\text{I,TW}} = &\sum_{i=1}^N\left(\sum_{j:j\neq i}\boldsymbol{Z}^{\text{adj}}_{\text{I},i,j}\widehat{r}^{\text{adj}}_{\text{I},i,j}\right)\left(\sum_{j:j\neq i}\boldsymbol{Z}^{\text{adj}}_{\text{I},i,j}\widehat{r}^{\text{adj}}_{\text{I},i,j}\right)^\top + \sum_{j=1}^N\left(\sum_{i:i\neq j}\boldsymbol{Z}^{\text{adj}}_{\text{I},i,j}\widehat{r}^{\text{adj}}_{\text{I},i,j}\right)\left(\sum_{i:i\neq j}\boldsymbol{Z}^{\text{adj}}_{\text{I},i,j}\widehat{r}^{\text{adj}}_{\text{I},i,j}\right)^\top\\ &-\sum_{i\neq j}\boldsymbol{Z}^{\text{adj}}_{\text{I},i,j}\boldsymbol{Z}^{\text{adj}\top}_{\text{I},i,j}(\widehat{r}^{\text{adj}}_{\text{I},i,j})^2.\end{aligned}$$

$\mathbf{M}^{\mathrm{adj}}_{\mathrm{I,TW}}$ is symmetric, with

$$\mathbf{M}^{\mathrm{adj}}_{\mathrm{I,TW}} = \begin{pmatrix} \mathrm{M}^{\mathrm{adj}}_{\mathrm{I,TW}}[1,1] & 0 & \mathbf{M}^{\mathrm{adj}}_{\mathrm{I,TW}}[1,3] & \mathbf{0} \\ * & \mathrm{M}^{\mathrm{adj}}_{\mathrm{I,TW}}[2,2] & \mathbf{0} & \mathbf{M}^{\mathrm{adj}}_{\mathrm{I,TW}}[2,4] \\ * & * & \mathbf{M}^{\mathrm{adj}}_{\mathrm{I,TW}}[3,3] & \mathbf{0} \\ * & * & * & \mathbf{M}^{\mathrm{adj}}_{\mathrm{I,TW}}[4,4] \end{pmatrix},$$

where $*$ denotes the symmetric components. Let

$$\begin{aligned}
U^{\mathrm{adj}}_{\mathrm{I,TW},i}(1,0) &= \sum_{j:j\neq i} A_i(1-A_j)\widehat{r}^{\mathrm{adj}}_{\mathrm{I},i,j}, \quad U^{\mathrm{adj}}_{\mathrm{I,TW},j}(1,0) = \sum_{i:i\neq j} A_i(1-A_j)\widehat{r}^{\mathrm{adj}}_{\mathrm{I},i,j}, \\
U^{\mathrm{adj}}_{\mathrm{I,TW},i}(0,1) &= \sum_{j:j\neq i} (1-A_i)A_j\widehat{r}^{\mathrm{adj}}_{\mathrm{I},i,j}, \quad U^{\mathrm{adj}}_{\mathrm{I,TW},j}(0,1) = \sum_{i:i\neq j} (1-A_i)A_j\widehat{r}^{\mathrm{adj}}_{\mathrm{I},i,j}, \\
\boldsymbol{L}^{\mathrm{adj}}_{\mathrm{I,TW},i}(1,0) &= \sum_{j:j\neq i} A_i(1-A_j)\boldsymbol{X}_{i,j}\widehat{r}^{\mathrm{adj}}_{\mathrm{I},i,j}, \quad \boldsymbol{L}^{\mathrm{adj}}_{\mathrm{I,TW},j}(1,0) = \sum_{i:i\neq j} A_i(1-A_j)\boldsymbol{X}_{i,j}\widehat{r}^{\mathrm{adj}}_{\mathrm{I},i,j}, \\
\boldsymbol{L}^{\mathrm{adj}}_{\mathrm{I,TW},i}(0,1) &= \sum_{j:j\neq i} (1-A_i)A_j\boldsymbol{X}_{i,j}\widehat{r}^{\mathrm{adj}}_{\mathrm{I},i,j}, \quad \boldsymbol{L}^{\mathrm{adj}}_{\mathrm{I,TW},j}(0,1) = \sum_{i:i\neq j} (1-A_i)A_j\boldsymbol{X}_{i,j}\widehat{r}^{\mathrm{adj}}_{\mathrm{I},i,j}.
\end{aligned}$$

Then,

$$\begin{aligned}
\mathrm{M}^{\mathrm{adj}}_{\mathrm{I,TW}}[1,1] &= \sum_{i=1}^N U^{\mathrm{adj}}_{\mathrm{I,TW},i}(1,0)^2 + \sum_{j=1}^N U^{\mathrm{adj}}_{\mathrm{I,TW},j}(1,0)^2 - \sum_{i\neq j} A_i(1-A_j)(\widehat{r}^{\mathrm{adj}}_{\mathrm{I},i,j})^2, \\
\mathbf{M}^{\mathrm{adj}}_{\mathrm{I,TW}}[1,3] &= \sum_{i=1}^N U^{\mathrm{adj}}_{\mathrm{I,TW},i}(1,0)\boldsymbol{L}^{\mathrm{adj}}_{\mathrm{I,TW},i}(1,0)^\top + \sum_{j=1}^N U^{\mathrm{adj}}_{\mathrm{I,TW},j}(1,0)\boldsymbol{L}_{\mathrm{I,TW},j}(1,0)^\top - \sum_{i\neq j} A_i(1-A_j)\boldsymbol{X}^\top_{i,j}(\widehat{r}^{\mathrm{adj}}_{\mathrm{I},i,j})^2, \\
\mathrm{M}^{\mathrm{adj}}_{\mathrm{I,TW}}[2,2] &= \sum_{i=1}^N U^{\mathrm{adj}}_{\mathrm{I,TW},i}(0,1)^2 + \sum_{j=1}^N U^{\mathrm{adj}}_{\mathrm{I,TW},j}(0,1)^2 - \sum_{i\neq j} (1-A_i)A_j(\widehat{r}^{\mathrm{adj}}_{\mathrm{I},i,j})^2, \\
\mathbf{M}^{\mathrm{adj}}_{\mathrm{I,TW}}[2,4] &= \sum_{i=1}^N U^{\mathrm{adj}}_{\mathrm{I,TW},i}(0,1)\boldsymbol{L}^{\mathrm{adj}}_{\mathrm{I,TW},i}(0,1)^\top + \sum_{j=1}^N U^{\mathrm{adj}}_{\mathrm{I,TW},j}(0,1)\boldsymbol{L}_{\mathrm{I,TW},j}(0,1)^\top - \sum_{i\neq j} (1-A_i)A_j\boldsymbol{X}^\top_{i,j}(\widehat{r}^{\mathrm{adj}}_{\mathrm{I},i,j})^2, \\
\mathbf{M}^{\mathrm{adj}}_{\mathrm{I,TW}}[3,3] &= \sum_{i=1}^N \boldsymbol{L}^{\mathrm{adj}}_{\mathrm{I,TW},i}(1,0)\boldsymbol{L}^{\mathrm{adj}}_{\mathrm{I,TW},i}(1,0)^\top + \sum_{j=1}^N \boldsymbol{L}_{\mathrm{I,TW},j}(1,0)\boldsymbol{L}_{\mathrm{I,TW},j}(1,0)^\top - \sum_{i\neq j} A_i(1-A_j)\boldsymbol{X}_{i,j}\boldsymbol{X}^\top_{i,j}(\widehat{r}^{\mathrm{adj}}_{\mathrm{I},i,j})^2, \\
\mathbf{M}^{\mathrm{adj}}_{\mathrm{I,TW}}[4,4] &= \sum_{i=1}^N \boldsymbol{L}^{\mathrm{adj}}_{\mathrm{I,TW},i}(0,1)\boldsymbol{L}^{\mathrm{adj}}_{\mathrm{I,TW},i}(0,1)^\top + \sum_{j=1}^N \boldsymbol{L}_{\mathrm{I,TW},j}(0,1)\boldsymbol{L}_{\mathrm{I,TW},j}(0,1)^\top - \sum_{i\neq j} (1-A_i)A_j\boldsymbol{X}_{i,j}\boldsymbol{X}^\top_{i,j}(\widehat{r}^{\mathrm{adj}}_{\mathrm{I},i,j})^2.
\end{aligned}$$

**Lemma S20.** *Under Conditions 1-3 in the main article, then*

$$\frac{1}{N(N-1)^2}\sum_{i=1}^N \left\{\sum_{j:j\neq i} A_i(1-A_j)\widehat{r}^{\mathrm{adj}}_{\mathrm{I},i,j}\right\}^2 - \frac{\pi_1\pi_0^2}{N}\sum_{i=1}^N \overline{r}^{\mathrm{adj}}_{\mathrm{I},i,\cdot}(1,0)^2 = o_{\mathbb{P}}(1), \tag{S10}$$

$$\frac{1}{N(N-1)^2}\sum_{i\neq j} A_i(1-A_j)(\widehat{r}^{\mathrm{adj}}_{\mathrm{I},i,j})^2 = o_{\mathbb{P}}(1), \tag{S11}$$

$$\frac{1}{N(N-1)^2}\sum_{i\neq j} A_i(1-A_j)\boldsymbol{X}^\top_{i,j}(\widehat{r}^{\mathrm{adj}}_{\mathrm{I},i,j})^2 = \boldsymbol{o}_{\mathbb{P}}(1), \tag{S12}$$

$$\frac{1}{N(N-1)^2}\sum_{i\neq j} A_i(1-A_j)\boldsymbol{X}_{i,j}\boldsymbol{X}^\top_{i,j}(\widehat{r}^{\mathrm{adj}}_{\mathrm{I},i,j})^2 = \boldsymbol{o}_{\mathbb{P}}(1), \tag{S13}$$

$$\frac{1}{N(N-1)^2}\sum_{i=1}^{N}\sum_{j:j\neq i}A_i(1-A_j)\widehat{r}^{\text{adj}}_{\text{I},i,j}\sum_{j:j\neq i}A_i(1-A_j)\boldsymbol{X}_{i,j}^{\top}\widehat{r}^{\text{adj}}_{\text{I},i,j}=\boldsymbol{O}_{\mathbb{P}}(1), \tag{S14}$$

$$\frac{1}{N(N-1)^2}\sum_{i=1}^{N}\sum_{j:j\neq i}A_i(1-A_j)\boldsymbol{X}_{i,j}\widehat{r}^{\text{adj}}_{\text{I},i,j}\sum_{j:j\neq i}A_i(1-A_j)\boldsymbol{X}_{i,j}^{\top}\widehat{r}^{\text{adj}}_{\text{I},i,j}=\boldsymbol{O}_{\mathbb{P}}(1). \tag{S15}$$

*Similar results can be obtained for the $(1-A_i)A_j$ pairing.*

The proof of Lemma S20 is similar to those of Lemmas S17 and S19. We omit the specific derivations but point out the connections with previous results. (S10) is implied by (S7); (S11) is implied by (S3); (S12) is implied by (S4); (S13) is implied by (S5); (S14) is implied by (S8); and (S15) is implied by (S9).

By Lemma S20,

$$\overline{\mathbf{M}}^{\text{adj}}_{\text{I,TW}}=\frac{1}{N(N-1)^2}\mathbf{M}^{\text{adj}}_{\text{I,TW}}=\boldsymbol{O}_{\mathbb{P}}(1).$$

We now analyze the TW variance estimators. Specifically, we have

$$N\widehat{\text{se}}^2_{\text{TW}}\left\{\widehat{\lambda}^{\text{adj}}_{\text{I}}(1,0)\right\}=\left[(\mathbf{G}^{\text{adj}}_{\text{I}})^{-1}\overline{\mathbf{M}}^{\text{adj}}_{\text{I,TW}}(\mathbf{G}^{\text{adj}}_{\text{I}})^{-1}\right]_{(1,1)},$$

where $\mathbf{G}^{\text{adj}}_{\text{I}}$ is given in (S2). Using similar arguments in the proof of the HR and CR variance estimators, we have

$$(\mathbf{G}^{\text{adj}}_{\text{I}})^{-1}\overline{\mathbf{M}}^{\text{adj}}_{\text{I,TW}}(\mathbf{G}^{\text{adj}}_{\text{I}})^{-1}-(\boldsymbol{\Gamma}^{\text{adj}}_{\text{I}})^{-1}\overline{\mathbf{M}}^{\text{adj}}_{\text{I,TW}}(\boldsymbol{\Gamma}^{\text{adj}}_{\text{I}})^{-1}=\boldsymbol{o}_{\mathbb{P}}(1),$$

where $\boldsymbol{\Gamma}^{\text{adj}}_{\text{I}}$ is defined in (S6). Then, by Lemma S20,

$$\begin{aligned}
&N\widehat{\text{se}}^2_{\text{TW}}\left\{\widehat{\lambda}^{\text{adj}}_{\text{I}}(1,0)\right\}=\left[(\boldsymbol{\Gamma}^{\text{adj}}_{\text{I}})^{-1}\overline{\mathbf{M}}^{\text{adj}}_{\text{I,TW}}(\boldsymbol{\Gamma}^{\text{adj}}_{\text{I}})^{-1}\right]_{(1,1)}+o_{\mathbb{P}}(1)\\
&=\frac{1}{N(N-1)^2}\cdot\frac{1}{\pi_1^2\pi_0^2}\sum_{i=1}^{N}A_i\left\{\sum_{j:j\neq i}(1-A_j)\widehat{r}^{\text{adj}}_{\text{I},i,j}\right\}^2+\frac{1}{N(N-1)^2}\cdot\frac{1}{\pi_1^2\pi_0^2}\sum_{i=1}^{N}(1-A_j)\left(\sum_{i:i\neq j}A_i\widehat{r}^{\text{adj}}_{\text{I},i,j}\right)^2+o_{\mathbb{P}}(1)\\
&=\frac{1}{\pi_1 N}\sum_{i=1}^{N}\overline{r}^{\text{adj}}_{\text{I},i,\cdot}(1,0)^2+\frac{1}{\pi_0 N}\sum_{j=1}^{N}\overline{r}^{\text{adj}}_{\text{I},\cdot,j}(1,0)^2+o_{\mathbb{P}}(1).
\end{aligned}$$

The probability limit of $N\widehat{\text{se}}^2_{\text{TW}}\{\widehat{\lambda}^{\text{adj}}_{\text{I}}(1,0)\}$ is $V_c\{\overline{r}^{\text{adj}}_{\text{I},i}(1,0)\}$. However,

$$\left[(\boldsymbol{\Gamma}^{\text{adj}}_{\text{I}})^{-1}\overline{\mathbf{M}}^{\text{adj}}_{\text{I,TW}}(\boldsymbol{\Gamma}^{\text{adj}}_{\text{I}})^{-1}\right]_{(1,2)}=\left[(\boldsymbol{\Gamma}^{\text{adj}}_{\text{I}})^{-1}\overline{\mathbf{M}}^{\text{adj}}_{\text{I,TW}}(\boldsymbol{\Gamma}^{\text{adj}}_{\text{I}})^{-1}\right]_{(2,1)}=o_{\mathbb{P}}(1),$$

implying that the TW estimator omits the covariance between $\widehat{\lambda}^{\text{adj}}_{\text{I}}(1,0)$ and $\widehat{\lambda}^{\text{adj}}_{\text{I}}(0,1)$.

#### S5.1.4 The complete two-way clustering variance estimators

We now show that the complete two-way (CTW) variance estimators are asymptotically conservative for the leading terms of the marginal variances and also consistent for sums of estimable components in the leading terms of the covariances. We focus on $\widehat{\lambda}^{\text{adj}}_{\text{I}}(a,1-a)$. We continue with the $\mathbf{Z}^{\text{adj}}_{\text{I}}$ design matrix for the TW variance estimators. For the CTW variance estimator, the middle matrix

$$\mathbf{M}^{\text{adj}}_{\text{I,CTW}}=\sum_{i=1}^{N}\left(\sum_{j:j\neq i}\boldsymbol{Z}^{\text{adj}}_{\text{I},i,j}\widehat{r}^{\text{adj}}_{\text{I},i,j}\right)\left(\sum_{j:j\neq i}\boldsymbol{Z}^{\text{adj}}_{\text{I},i,j}\widehat{r}^{\text{adj}}_{\text{I},i,j}\right)^{\top}+\sum_{j=1}^{N}\left(\sum_{i:i\neq j}\boldsymbol{Z}^{\text{adj}}_{\text{I},i,j}\widehat{r}^{\text{adj}}_{\text{I},i,j}\right)\left(\sum_{i:i\neq j}\boldsymbol{Z}^{\text{adj}}_{\text{I},i,j}\widehat{r}^{\text{adj}}_{\text{I},i,j}\right)^{\top}$$

$$+\sum_{i=1}^{N}\left(\sum_{j:j\neq i}\boldsymbol{Z}_{\mathrm{I},i,j}^{\mathrm{adj}}\widehat{r}_{\mathrm{I},i,j}^{\mathrm{adj}}\right)\left(\sum_{j:j\neq i}\boldsymbol{Z}_{\mathrm{I},j,i}^{\mathrm{adj}}\widehat{r}_{\mathrm{I},j,i}^{\mathrm{adj}}\right)^{\top}+\sum_{j=1}^{N}\left(\sum_{i:i\neq j}\boldsymbol{Z}_{\mathrm{I},i,j}^{\mathrm{adj}}\widehat{r}_{\mathrm{I},i,j}^{\mathrm{adj}}\right)\left(\sum_{i:i\neq j}\boldsymbol{Z}_{\mathrm{I},j,i}^{\mathrm{adj}}\widehat{r}_{\mathrm{I},j,i}^{\mathrm{adj}}\right)^{\top}$$
$$-\sum_{i\neq j}\boldsymbol{Z}_{\mathrm{I},i,j}^{\mathrm{adj}}\boldsymbol{Z}_{\mathrm{I},j,i}^{\mathrm{adj}\top}\widehat{r}_{\mathrm{I},i,j}^{\mathrm{adj}}\widehat{r}_{\mathrm{I},j,i}^{\mathrm{adj}}-\sum_{i\neq j}\boldsymbol{Z}_{\mathrm{I},i,j}^{\mathrm{adj}}\boldsymbol{Z}_{\mathrm{I},i,j}^{\mathrm{adj}\top}(\widehat{r}_{\mathrm{I},i,j}^{\mathrm{adj}})^{2}.$$

$\mathbf{M}_{\mathrm{I,CTW}}^{\mathrm{adj}}$ is symmetric, with

$$\mathbf{M}_{\mathrm{I,CTW}}^{\mathrm{adj}}=\begin{pmatrix}\mathrm{M}_{\mathrm{I,CTW}}^{\mathrm{adj}}[1,1] & \mathrm{M}_{\mathrm{I,CTW}}^{\mathrm{adj}}[1,2] & \mathbf{M}_{\mathrm{I,CTW}}^{\mathrm{adj}}[1,3] & \mathbf{M}_{\mathrm{I,CTW}}^{\mathrm{adj}}[1,4]\\ * & \mathrm{M}_{\mathrm{I,CTW}}^{\mathrm{adj}}[2,2] & \mathbf{M}_{\mathrm{I,CTW}}^{\mathrm{adj}}[2,3] & \mathbf{M}_{\mathrm{I,CTW}}^{\mathrm{adj}}[2,4]\\ * & * & \mathbf{M}_{\mathrm{I,CTW}}^{\mathrm{adj}}[3,3] & \mathbf{M}_{\mathrm{I,CTW}}^{\mathrm{adj}}[3,4]\\ * & * & * & \mathbf{M}_{\mathrm{I,CTW}}^{\mathrm{adj}}[4,4]\end{pmatrix},$$

where $*$ denotes the symmetric components. Note that the diagonal, and the $(1,3)$, $(2,4)$, $(3,1)$, and $(4,2)$ elements/blocks in the reverse effects and the correction are zero. We use entry $(1,1)$ in these matrices as an example, and other entries/blocks follow. Specifically,

$$\begin{aligned}&\sum_{j:j\neq i}A_i(1-A_j)\widehat{r}_{\mathrm{I},i,j}^{\mathrm{adj}}\sum_{j:j\neq i}A_j(1-A_i)\widehat{r}_{\mathrm{I},j,i}^{\mathrm{adj}}=(1-A_i)A_i\sum_{j:j\neq i}(1-A_j)\widehat{r}_{\mathrm{I},i,j}^{\mathrm{adj}}\sum_{j:j\neq i}A_j\widehat{r}_{\mathrm{I},j,i}^{\mathrm{adj}}=0,\\&\sum_{i:i\neq j}A_i(1-A_j)\widehat{r}_{\mathrm{I},i,j}^{\mathrm{adj}}\sum_{i:i\neq j}A_j(1-A_i)\widehat{r}_{\mathrm{I},j,i}^{\mathrm{adj}}=A_j(1-A_j)\sum_{j:j\neq i}A_i\widehat{r}_{\mathrm{I},i,j}^{\mathrm{adj}}\sum_{j:j\neq i}(1-A_i)\widehat{r}_{\mathrm{I},j,i}^{\mathrm{adj}}=0,\\&A_i(1-A_j)\widehat{r}_{\mathrm{I},i,j}^{\mathrm{adj}}A_j(1-A_i)\widehat{r}_{\mathrm{I},j,i}^{\mathrm{adj}}=A_i(1-A_j)A_j(1-A_i)\widehat{r}_{\mathrm{I},i,j}^{\mathrm{adj}}\widehat{r}_{\mathrm{I},j,i}^{\mathrm{adj}}=0.\end{aligned}$$

Then, we have

$$\begin{aligned}&\mathrm{M}_{\mathrm{I,CTW}}^{\mathrm{adj}}[1,1]=\mathrm{M}_{\mathrm{I,TW}}^{\mathrm{adj}}[1,1],\quad \mathrm{M}_{\mathrm{I,CTW}}^{\mathrm{adj}}[2,2]=\mathrm{M}_{\mathrm{I,TW}}^{\mathrm{adj}}[2,2],\quad \mathbf{M}_{\mathrm{I,CTW}}^{\mathrm{adj}}[3,3]=\mathbf{M}_{\mathrm{I,TW}}^{\mathrm{adj}}[3,3],\\&\mathbf{M}_{\mathrm{I,CTW}}^{\mathrm{adj}}[4,4]=\mathbf{M}_{\mathrm{I,TW}}^{\mathrm{adj}}[4,4],\quad \mathbf{M}_{\mathrm{I,CTW}}^{\mathrm{adj}}[1,3]=\mathbf{M}_{\mathrm{I,TW}}^{\mathrm{adj}}[1,3],\quad \mathbf{M}_{\mathrm{I,CTW}}^{\mathrm{adj}}[2,4]=\mathbf{M}_{\mathrm{I,TW}}^{\mathrm{adj}}[2,4],\end{aligned}$$

and also the symmetric entries/blocks. For non-zero entries/blocks,

$$\begin{aligned}\mathrm{M}_{\mathrm{I,CTW}}^{\mathrm{adj}}[1,2]=&\sum_{i=1}^{N}(1-A_i)\sum_{j:j\neq i}A_j\widehat{r}_{\mathrm{I},i,j}^{\mathrm{adj}}\sum_{j:j\neq i}A_j\widehat{r}_{\mathrm{I},j,i}^{\mathrm{adj}}+\sum_{j=1}^{N}A_j\sum_{j:j\neq i}(1-A_i)\widehat{r}_{\mathrm{I},i,j}^{\mathrm{adj}}\sum_{i:i\neq j}(1-A_i)\widehat{r}_{\mathrm{I},j,i}^{\mathrm{adj}}\\&-\sum_{i\neq j}A_i(1-A_j)\widehat{r}_{\mathrm{I},i,j}^{\mathrm{adj}}\widehat{r}_{\mathrm{I},j,i}^{\mathrm{adj}},\\ \mathbf{M}_{\mathrm{I,CTW}}^{\mathrm{adj}}[1,4]=&\sum_{i=1}^{N}(1-A_i)\sum_{j:j\neq i}A_j\widehat{r}_{\mathrm{I},i,j}^{\mathrm{adj}}\sum_{j:j\neq i}A_j\boldsymbol{X}_{j,i}^{\top}\widehat{r}_{\mathrm{I},j,i}^{\mathrm{adj}}+\sum_{j=1}^{N}A_j\sum_{j:j\neq i}(1-A_i)\widehat{r}_{\mathrm{I},i,j}^{\mathrm{adj}}\sum_{i:i\neq j}(1-A_i)\boldsymbol{X}_{j,i}^{\top}\widehat{r}_{\mathrm{I},j,i}^{\mathrm{adj}}\\&-\sum_{i\neq j}A_i(1-A_j)\widehat{r}_{\mathrm{I},i,j}^{\mathrm{adj}}\boldsymbol{X}_{j,i}^{\top}\widehat{r}_{\mathrm{I},j,i}^{\mathrm{adj}},\\ \mathbf{M}_{\mathrm{I,CTW}}^{\mathrm{adj}}[2,3]=&\sum_{i=1}^{N}A_i\sum_{j:j\neq i}(1-A_j)\widehat{r}_{\mathrm{I},i,j}^{\mathrm{adj}}\sum_{j:j\neq i}(1-A_j)\boldsymbol{X}_{j,i}^{\top}\widehat{r}_{\mathrm{I},j,i}^{\mathrm{adj}}+\sum_{j=1}^{N}(1-A_j)\sum_{j:j\neq i}A_i\widehat{r}_{\mathrm{I},i,j}^{\mathrm{adj}}\sum_{i:i\neq j}A_i\boldsymbol{X}_{j,i}^{\top}\widehat{r}_{\mathrm{I},j,i}^{\mathrm{adj}}\\&-\sum_{i\neq j}(1-A_i)A_j\widehat{r}_{\mathrm{I},i,j}^{\mathrm{adj}}\boldsymbol{X}_{j,i}^{\top}\widehat{r}_{\mathrm{I},j,i}^{\mathrm{adj}},\\ \mathbf{M}_{\mathrm{I,CTW}}^{\mathrm{adj}}[3,4]=&\sum_{i=1}^{N}(1-A_i)\sum_{j:j\neq i}A_j\boldsymbol{X}_{i,j}\widehat{r}_{\mathrm{I},i,j}^{\mathrm{adj}}\sum_{j:j\neq i}A_j\boldsymbol{X}_{j,i}^{\top}\widehat{r}_{\mathrm{I},j,i}^{\mathrm{adj}}+\sum_{j=1}^{N}A_j\sum_{j:j\neq i}(1-A_i)\boldsymbol{X}_{i,j}\widehat{r}_{\mathrm{I},i,j}^{\mathrm{adj}}\sum_{i:i\neq j}(1-A_i)\boldsymbol{X}_{j,i}^{\top}\widehat{r}_{\mathrm{I},j,i}^{\mathrm{adj}}\\&-\sum_{i\neq j}A_i(1-A_j)\boldsymbol{X}_{i,j}\boldsymbol{X}_{j,i}^{\top}\widehat{r}_{\mathrm{I},i,j}^{\mathrm{adj}}\widehat{r}_{\mathrm{I},j,i}^{\mathrm{adj}}.\end{aligned}$$

**Lemma S21.** *Under Conditions 1-3 in the main article, then*

$$\frac{1}{N(N-1)^2}\sum_{i=1}^{N}(1-A_i)\sum_{j:j\neq i}A_j\widehat{r}^{\text{adj}}_{\text{I},i,j}\sum_{j:j\neq i}A_j\widehat{r}^{\text{adj}}_{\text{I},j,i}-\frac{\pi_0\pi_1^2}{N}\sum_{i=1}^{N}\overline{r}^{\text{adj}}_{\text{I},\cdot,i}(1,0)\overline{r}^{\text{adj}}_{\text{I},i,\cdot}(0,1)=o_{\mathbb{P}}(1), \tag{S16}$$

$$\frac{1}{N(N-1)^2}\sum_{i\neq j}A_i(1-A_j)\widehat{r}^{\text{adj}}_{\text{I},i,j}\widehat{r}^{\text{adj}}_{\text{I},j,i}=o_{\mathbb{P}}(1), \tag{S17}$$

$$\frac{1}{N(N-1)^2}\sum_{i\neq j}A_i(1-A_j)\widehat{r}^{\text{adj}}_{\text{I},i,j}\boldsymbol{X}_{j,i}^{\top}\widehat{r}^{\text{adj}}_{\text{I},j,i}=\boldsymbol{o}_{\mathbb{P}}(1), \tag{S18}$$

$$\frac{1}{N(N-1)^2}\sum_{i\neq j}A_i(1-A_j)\boldsymbol{X}_{i,j}\boldsymbol{X}_{j,i}^{\top}\widehat{r}^{\text{adj}}_{\text{I},i,j}\widehat{r}^{\text{adj}}_{\text{I},j,i}=\boldsymbol{o}_{\mathbb{P}}(1), \tag{S19}$$

$$\frac{1}{N(N-1)^2}\sum_{i=1}^{N}(1-A_i)\sum_{j:j\neq i}A_j\widehat{r}^{\text{adj}}_{\text{I},i,j}\sum_{j:j\neq i}A_j\boldsymbol{X}_{j,i}^{\top}\widehat{r}^{\text{adj}}_{\text{I},j,i}=\boldsymbol{O}_{\mathbb{P}}(1), \tag{S20}$$

$$\frac{1}{N(N-1)^2}\sum_{i=1}^{N}(1-A_i)\sum_{j:j\neq i}A_j\boldsymbol{X}_{i,j}\widehat{r}^{\text{adj}}_{\text{I},i,j}\sum_{j:j\neq i}A_j\boldsymbol{X}_{j,i}^{\top}\widehat{r}^{\text{adj}}_{\text{I},j,i}=\boldsymbol{O}_{\mathbb{P}}(1). \tag{S21}$$

*Similar results can be obtained for other terms.*

Similar to Lemma S20, the proof of Lemma S21 follows that of Lemmas S17 and S19. We omit the specific derivations but point out the connections with previous results. (S16) is implied by (S7); (S17) is implied by (S3); (S18) is implied by (S4); (S19) is implied by (S5); (S20) is implied by (S8); and (S21) is implied by (S9).

By Lemmas S20 and S21,

$$\overline{\mathbf{M}}^{\text{adj}}_{\text{I,CTW}}=\frac{1}{N(N-1)^2}\mathbf{M}^{\text{adj}}_{\text{I,CTW}}=\boldsymbol{O}_{\mathbb{P}}(1).$$

We now analyze the CTW covariance estimators. The CTW variance estimators for marginal variances are identical to their respective TW counterparts. We thus focus on the covariances. Specifically, we have

$$N\widehat{\mathbb{C}\text{ov}}_{\text{CTW}}\left\{\widehat{\lambda}^{\text{adj}}_{\text{I}}(1,0),\widehat{\lambda}^{\text{adj}}_{\text{I}}(0,1)\right\}=\left[(\mathbf{G}^{\text{adj}}_{\text{I}})^{-1}\overline{\mathbf{M}}^{\text{adj}}_{\text{I,CTW}}(\mathbf{G}^{\text{adj}}_{\text{I}})^{-1}\right]_{(1,2)}.$$

Using similar arguments in the proof of the HR and CR variance estimators, we have

$$(\mathbf{G}^{\text{adj}}_{\text{I}})^{-1}\overline{\mathbf{M}}^{\text{adj}}_{\text{I,CTW}}(\mathbf{G}^{\text{adj}}_{\text{I}})^{-1}-(\boldsymbol{\Gamma}^{\text{adj}}_{\text{I}})^{-1}\overline{\mathbf{M}}^{\text{adj}}_{\text{I,CTW}}(\boldsymbol{\Gamma}^{\text{adj}}_{\text{I}})^{-1}=\boldsymbol{o}_{\mathbb{P}}(1).$$

By (S16) and (S17),

$$\begin{aligned}N\widehat{\mathbb{C}\text{ov}}_{\text{CTW}}\left\{\widehat{\lambda}^{\text{adj}}_{\text{I}}(1,0),\widehat{\lambda}^{\text{adj}}_{\text{I}}(0,1)\right\}&=\left[(\boldsymbol{\Gamma}^{\text{adj}}_{\text{I}})^{-1}\overline{\mathbf{M}}^{\text{adj}}_{\text{I,CTW}}(\boldsymbol{\Gamma}^{\text{adj}}_{\text{I}})^{-1}\right]_{(1,2)}+o_{\mathbb{P}}(1)\\&=\frac{1}{N(N-1)^2}\cdot\frac{1}{\pi_1^2\pi_0^2}\sum_{i=1}^{N}(1-A_i)\sum_{j:j\neq i}A_j\widehat{r}^{\text{adj}}_{\text{I},i,j}\sum_{j:j\neq i}A_j\widehat{r}^{\text{adj}}_{\text{I},j,i}\\&\quad+\frac{1}{N(N-1)^2}\cdot\frac{1}{\pi_1^2\pi_0^2}\sum_{j=1}^{N}A_j\sum_{j:j\neq i}(1-A_i)\widehat{r}^{\text{adj}}_{\text{I},i,j}\sum_{i:i\neq j}(1-A_i)\widehat{r}^{\text{adj}}_{\text{I},j,i}+o_{\mathbb{P}}(1)\\&=\frac{1}{\pi_0 N}\sum_{i=1}^{N}\overline{r}^{\text{adj}}_{\text{I},i,\cdot}(0,1)\overline{r}^{\text{adj}}_{\text{I},\cdot,i}(1,0)+\frac{1}{\pi_1 N}\sum_{j=1}^{N}\overline{r}^{\text{adj}}_{\text{I},\cdot,j}(0,1)\overline{r}^{\text{adj}}_{\text{I},j,\cdot}(1,0)+o_{\mathbb{P}}(1).\end{aligned}$$

The probability limit of $N\widehat{\mathbb{C}\text{ov}}_{\text{CTW}}\{\widehat{\lambda}^{\text{adj}}_{\text{I}}(1,0),\widehat{\lambda}^{\text{adj}}_{\text{I}}(0,1)\}$ is the sum of estimable components in $CV(\overline{r}^{\text{adj}}_{\text{I},i})$.

## S5.2 The PIM estimators

### S5.2.1 The CTW variance estimators

We prove that the CTW variance estimators are asymptotically conservative for the leading terms of the variances of the PIM estimators. We focus on $\widehat{\tau}_{\mathrm{P}}^{\mathrm{adj}}(1)$. Recall that the design vector $\boldsymbol{Z}_{\mathrm{P},i,j}^{\mathrm{adj}} = (D_{i,j}, \boldsymbol{X}_{i,j}^{\top}, D_{i,j}\boldsymbol{X}_{i,j}^{\top})^{\top}$, and $\widehat{r}_{\mathrm{P},i,j}^{\mathrm{adj}}$ is the residual from the OLS fit of $W_{i,j}$ on $(D_{i,j}, \boldsymbol{X}_{i,j}^{\top}, D_{i,j}\boldsymbol{X}_{i,j}^{\top})$. Stack $\boldsymbol{Z}_{\mathrm{P},i,j}^{\mathrm{adj}\top}$ to create design matrix $\mathbf{Z}_{\mathrm{P}}^{\mathrm{adj}}$. The CTW variance estimator is

$$\widehat{\mathrm{se}}_{\mathrm{CTW}}^{2}\left\{\widehat{\tau}_{\mathrm{P}}^{\mathrm{adj}}(1)\right\} = 4\left[\left(\mathbf{Z}_{\mathrm{P}}^{\mathrm{adj}\top}\mathbf{Z}_{\mathrm{P}}^{\mathrm{adj}}\right)^{-1}\mathbf{M}_{\mathrm{P,CTW}}^{\mathrm{adj}}\left(\mathbf{Z}_{\mathrm{P}}^{\mathrm{adj}\top}\mathbf{Z}_{\mathrm{P}}^{\mathrm{adj}}\right)^{-1}\right]_{(1,1)},$$

where,

$$\begin{aligned}
\mathbf{M}_{\mathrm{P,CTW}}^{\mathrm{adj}} =& \sum_{i=1}^{N}\left(\sum_{j:j\neq i}\boldsymbol{Z}_{\mathrm{P},i,j}^{\mathrm{adj}}\widehat{r}_{\mathrm{P},i,j}^{\mathrm{adj}}\right)\left(\sum_{j:j\neq i}\boldsymbol{Z}_{\mathrm{P},i,j}^{\mathrm{adj}}\widehat{r}_{\mathrm{P},i,j}^{\mathrm{adj}}\right)^{\top} + \sum_{j=1}^{N}\left(\sum_{i:i\neq j}\boldsymbol{Z}_{\mathrm{P},i,j}^{\mathrm{adj}}\widehat{r}_{\mathrm{P},i,j}^{\mathrm{adj}}\right)\left(\sum_{i:i\neq j}\boldsymbol{Z}_{\mathrm{P},i,j}^{\mathrm{adj}}\widehat{r}_{\mathrm{P},i,j}^{\mathrm{adj}}\right)^{\top} \\
&+ \sum_{i=1}^{N}\left(\sum_{j:j\neq i}\boldsymbol{Z}_{\mathrm{I},i,j}^{\mathrm{adj}}\widehat{r}_{\mathrm{P},i,j}^{\mathrm{adj}}\right)\left(\sum_{j:j\neq i}\boldsymbol{Z}_{\mathrm{P},j,i}^{\mathrm{adj}}\widehat{r}_{\mathrm{P},j,i}^{\mathrm{adj}}\right)^{\top} + \sum_{j=1}^{N}\left(\sum_{i:i\neq j}\boldsymbol{Z}_{\mathrm{P},i,j}^{\mathrm{adj}}\widehat{r}_{\mathrm{P},i,j}^{\mathrm{adj}}\right)\left(\sum_{i:i\neq j}\boldsymbol{Z}_{\mathrm{P},j,i}^{\mathrm{adj}}\widehat{r}_{\mathrm{P},j,i}^{\mathrm{adj}}\right)^{\top} \\
&- \sum_{i\neq j}\left\{\boldsymbol{Z}_{\mathrm{P},i,j}^{\mathrm{adj}}\boldsymbol{Z}_{\mathrm{P},j,i}^{\mathrm{adj}\top}\widehat{r}_{\mathrm{P},i,j}^{\mathrm{adj}}\widehat{r}_{\mathrm{P},j,i}^{\mathrm{adj}} + \boldsymbol{Z}_{\mathrm{P},i,j}^{\mathrm{adj}}\boldsymbol{Z}_{\mathrm{P},i,j}^{\mathrm{adj}\top}(\widehat{r}_{\mathrm{P},i,j}^{\mathrm{adj}})^{2}\right\}.
\end{aligned}$$

$\mathbf{M}_{\mathrm{P,CTW}}^{\mathrm{adj}}$ is symmetric, with

$$\mathbf{M}_{\mathrm{P,CTW}}^{\mathrm{adj}} = \begin{pmatrix} \mathrm{M}_{\mathrm{P,CTW}}^{\mathrm{adj}}[1,1] & \mathbf{M}_{\mathrm{P,CTW}}^{\mathrm{adj}}[1,2] & \mathbf{M}_{\mathrm{P,CTW}}^{\mathrm{adj}}[1,3] \\ * & \mathbf{M}_{\mathrm{P,CTW}}^{\mathrm{adj}}[2,2] & \mathbf{M}_{\mathrm{P,CTW}}^{\mathrm{adj}}[2,3] \\ * & * & \mathbf{M}_{\mathrm{P,CTW}}^{\mathrm{adj}}[3,3] \end{pmatrix},$$

where $*$ denotes the symmetric components. Then,

$$\begin{aligned}
\mathrm{M}_{\mathrm{P,CTW}}^{\mathrm{adj}}[1,1] =& \sum_{i=1}^{N}\left(\sum_{j:j\neq i}D_{i,j}\widehat{r}_{\mathrm{P},i,j}^{\mathrm{adj}}\right)^{2} + \sum_{j=1}^{N}\left(\sum_{i:i\neq j}D_{i,j}\widehat{r}_{\mathrm{P},i,j}^{\mathrm{adj}}\right)^{2} + \sum_{i=1}^{N}\sum_{j:j\neq i}D_{i,j}\widehat{r}_{\mathrm{P},i,j}^{\mathrm{adj}}\sum_{j:j\neq i}D_{j,i}\widehat{r}_{\mathrm{P},j,i}^{\mathrm{adj}} \\
&+ \sum_{j=1}^{N}\sum_{i:i\neq j}D_{i,j}\widehat{r}_{\mathrm{P},i,j}^{\mathrm{adj}}\sum_{i:i\neq j}D_{j,i}\widehat{r}_{\mathrm{P},j,i}^{\mathrm{adj}} - \sum_{i\neq j}D_{i,j}D_{j,i}\widehat{r}_{\mathrm{P},i,j}^{\mathrm{adj}}\widehat{r}_{\mathrm{P},j,i}^{\mathrm{adj}} - \sum_{i\neq j}D_{i,j}^{2}(\widehat{r}_{\mathrm{P},i,j}^{\mathrm{adj}})^{2}, \\
\mathbf{M}_{\mathrm{P,CTW}}^{\mathrm{adj}}[1,2] =& \sum_{i=1}^{N}\sum_{j:j\neq i}D_{i,j}\widehat{r}_{\mathrm{P},i,j}^{\mathrm{adj}}\sum_{j:j\neq i}\boldsymbol{X}_{i,j}^{\top}\widehat{r}_{\mathrm{P},i,j}^{\mathrm{adj}} + \sum_{j=1}^{N}\sum_{i:i\neq j}D_{i,j}\widehat{r}_{\mathrm{P},i,j}^{\mathrm{adj}}\sum_{i:i\neq j}\boldsymbol{X}_{i,j}^{\top}\widehat{r}_{\mathrm{P},i,j}^{\mathrm{adj}} \\
&+ \sum_{i=1}^{N}\sum_{j:j\neq i}D_{i,j}\widehat{r}_{\mathrm{P},i,j}^{\mathrm{adj}}\sum_{j:j\neq i}\boldsymbol{X}_{j,i}^{\top}\widehat{r}_{\mathrm{P},j,i}^{\mathrm{adj}} + \sum_{j=1}^{N}\sum_{i:i\neq j}D_{i,j}\widehat{r}_{\mathrm{P},i,j}^{\mathrm{adj}}\sum_{i:i\neq j}\boldsymbol{X}_{j,i}^{\top}\widehat{r}_{\mathrm{P},j,i}^{\mathrm{adj}} \\
&- \sum_{i\neq j}D_{i,j}\widehat{r}_{\mathrm{P},i,j}^{\mathrm{adj}}\boldsymbol{X}_{j,i}^{\top}\widehat{r}_{\mathrm{P},j,i}^{\mathrm{adj}} - \sum_{i\neq j}D_{i,j}\boldsymbol{X}_{i,j}^{\top}(\widehat{r}_{\mathrm{P},i,j}^{\mathrm{adj}})^{2}, \\
\mathbf{M}_{\mathrm{P,CTW}}^{\mathrm{adj}}[1,3] =& \sum_{i=1}^{N}\sum_{j:j\neq i}D_{i,j}\widehat{r}_{\mathrm{P},i,j}^{\mathrm{adj}}\sum_{j:j\neq i}D_{i,j}\boldsymbol{X}_{i,j}^{\top}\widehat{r}_{\mathrm{P},i,j}^{\mathrm{adj}} + \sum_{j=1}^{N}\sum_{i:i\neq j}D_{i,j}\widehat{r}_{\mathrm{P},i,j}^{\mathrm{adj}}\sum_{i:i\neq j}D_{i,j}\boldsymbol{X}_{i,j}^{\top}\widehat{r}_{\mathrm{P},i,j}^{\mathrm{adj}} \\
&+ \sum_{i=1}^{N}\sum_{j:j\neq i}D_{i,j}\widehat{r}_{\mathrm{P},i,j}^{\mathrm{adj}}\sum_{j:j\neq i}D_{j,i}\boldsymbol{X}_{j,i}^{\top}\widehat{r}_{\mathrm{P},j,i}^{\mathrm{adj}} + \sum_{j=1}^{N}\sum_{i:i\neq j}D_{i,j}\widehat{r}_{\mathrm{P},i,j}^{\mathrm{adj}}\sum_{i:i\neq j}D_{j,i}\boldsymbol{X}_{j,i}^{\top}\widehat{r}_{\mathrm{P},j,i}^{\mathrm{adj}} \\
&- \sum_{i\neq j}D_{i,j}D_{j,i}\widehat{r}_{\mathrm{P},i,j}^{\mathrm{adj}}\boldsymbol{X}_{j,i}^{\top}\widehat{r}_{\mathrm{P},j,i}^{\mathrm{adj}} - \sum_{i\neq j}D_{i,j}^{2}\boldsymbol{X}_{i,j}^{\top}(\widehat{r}_{\mathrm{P},i,j}^{\mathrm{adj}})^{2},
\end{aligned}$$

$$\mathbf{M}^{\mathrm{adj}}_{\mathrm{P,CTW}}[2,2] = \sum_{i=1}^{N}\sum_{j:j\neq i}\boldsymbol{X}_{i,j}\widehat{r}^{\mathrm{adj}}_{\mathrm{P},i,j}\sum_{j:j\neq i}\boldsymbol{X}_{i,j}^{\top}\widehat{r}^{\mathrm{adj}}_{\mathrm{P},i,j} + \sum_{j=1}^{N}\sum_{i:i\neq j}\boldsymbol{X}_{i,j}\widehat{r}^{\mathrm{adj}}_{\mathrm{P},i,j}\sum_{i:i\neq j}\boldsymbol{X}_{i,j}^{\top}\widehat{r}^{\mathrm{adj}}_{\mathrm{P},i,j}$$
$$+ \sum_{i=1}^{N}\sum_{j:j\neq i}\boldsymbol{X}_{i,j}\widehat{r}^{\mathrm{adj}}_{\mathrm{P},i,j}\sum_{j:j\neq i}\boldsymbol{X}_{j,i}^{\top}\widehat{r}^{\mathrm{adj}}_{\mathrm{P},j,i} + \sum_{j=1}^{N}\sum_{i:i\neq j}\boldsymbol{X}_{i,j}\widehat{r}^{\mathrm{adj}}_{\mathrm{P},i,j}\sum_{i:i\neq j}\boldsymbol{X}_{j,i}^{\top}\widehat{r}^{\mathrm{adj}}_{\mathrm{P},j,i}$$
$$- \sum_{i\neq j}\boldsymbol{X}_{i,j}\boldsymbol{X}_{j,i}^{\top}\widehat{r}^{\mathrm{adj}}_{\mathrm{P},i,j}\widehat{r}^{\mathrm{adj}}_{\mathrm{P},j,i} - \sum_{i\neq j}\boldsymbol{X}_{i,j}\boldsymbol{X}_{i,j}^{\top}(\widehat{r}^{\mathrm{adj}}_{\mathrm{P},i,j})^2,$$

$$\mathbf{M}^{\mathrm{adj}}_{\mathrm{P,CTW}}[2,3] = \sum_{i=1}^{N}\sum_{j:j\neq i}\boldsymbol{X}_{i,j}\widehat{r}^{\mathrm{adj}}_{\mathrm{P},i,j}\sum_{j:j\neq i}D_{i,j}\boldsymbol{X}_{i,j}^{\top}\widehat{r}^{\mathrm{adj}}_{\mathrm{P},i,j} + \sum_{j=1}^{N}\sum_{i:i\neq j}\boldsymbol{X}_{i,j}\widehat{r}^{\mathrm{adj}}_{\mathrm{P},i,j}\sum_{i:i\neq j}D_{i,j}\boldsymbol{X}_{i,j}^{\top}\widehat{r}^{\mathrm{adj}}_{\mathrm{P},i,j}$$
$$+ \sum_{i=1}^{N}\sum_{j:j\neq i}\boldsymbol{X}_{i,j}\widehat{r}^{\mathrm{adj}}_{\mathrm{P},i,j}\sum_{j:j\neq i}D_{j,i}\boldsymbol{X}_{j,i}^{\top}\widehat{r}^{\mathrm{adj}}_{\mathrm{P},j,i} + \sum_{j=1}^{N}\sum_{i:i\neq j}\boldsymbol{X}_{i,j}\widehat{r}^{\mathrm{adj}}_{\mathrm{P},i,j}\sum_{i:i\neq j}D_{j,i}\boldsymbol{X}_{j,i}^{\top}\widehat{r}^{\mathrm{adj}}_{\mathrm{P},j,i}$$
$$- \sum_{i\neq j}D_{j,i}\boldsymbol{X}_{i,j}\boldsymbol{X}_{j,i}^{\top}\widehat{r}^{\mathrm{adj}}_{\mathrm{P},i,j}\widehat{r}^{\mathrm{adj}}_{\mathrm{P},j,i} - \sum_{i\neq j}D_{i,j}\boldsymbol{X}_{i,j}\boldsymbol{X}_{i,j}^{\top}(\widehat{r}^{\mathrm{adj}}_{\mathrm{P},i,j})^2,$$

$$\mathbf{M}^{\mathrm{adj}}_{\mathrm{P,CTW}}[3,3] = \sum_{i=1}^{N}\sum_{j:j\neq i}D_{i,j}\boldsymbol{X}_{i,j}\widehat{r}^{\mathrm{adj}}_{\mathrm{P},i,j}\sum_{j:j\neq i}D_{i,j}\boldsymbol{X}_{i,j}^{\top}\widehat{r}^{\mathrm{adj}}_{\mathrm{P},i,j} + \sum_{j=1}^{N}\sum_{i:i\neq j}D_{i,j}\boldsymbol{X}_{i,j}\widehat{r}^{\mathrm{adj}}_{\mathrm{P},i,j}\sum_{i:i\neq j}D_{i,j}\boldsymbol{X}_{i,j}^{\top}\widehat{r}^{\mathrm{adj}}_{\mathrm{P},i,j}$$
$$+ \sum_{i=1}^{N}\sum_{j:j\neq i}D_{i,j}\boldsymbol{X}_{i,j}\widehat{r}^{\mathrm{adj}}_{\mathrm{P},i,j}\sum_{j:j\neq i}D_{j,i}\boldsymbol{X}_{j,i}^{\top}\widehat{r}^{\mathrm{adj}}_{\mathrm{P},j,i} + \sum_{j=1}^{N}\sum_{i:i\neq j}D_{i,j}\boldsymbol{X}_{i,j}\widehat{r}^{\mathrm{adj}}_{\mathrm{P},i,j}\sum_{i:i\neq j}D_{j,i}\boldsymbol{X}_{j,i}^{\top}\widehat{r}^{\mathrm{adj}}_{\mathrm{P},j,i}$$
$$- \sum_{i\neq j}D_{i,j}D_{j,i}\boldsymbol{X}_{i,j}\boldsymbol{X}_{j,i}^{\top}\widehat{r}^{\mathrm{adj}}_{\mathrm{P},i,j}\widehat{r}^{\mathrm{adj}}_{\mathrm{P},j,i} - \sum_{i\neq j}D_{i,j}^2\boldsymbol{X}_{i,j}\boldsymbol{X}_{i,j}^{\top}(\widehat{r}^{\mathrm{adj}}_{\mathrm{P},i,j})^2.$$

Also, recall that $\mathcal{S} = \mathcal{S}(1,0)\cup\mathcal{S}(0,1)$, and then define

$$\mathbf{G}^{\mathrm{adj}}_{\mathrm{P}} = \frac{1}{N(N-1)}\mathbf{Z}^{\mathrm{adj}\top}_{\mathrm{P}}\mathbf{Z}^{\mathrm{adj}}_{\mathrm{P}} = \frac{1}{N(N-1)}\sum_{i\neq j}\boldsymbol{Z}^{\mathrm{adj}}_{\mathrm{P},i,j}\boldsymbol{Z}^{\mathrm{adj}\top}_{\mathrm{P},i,j}$$
$$= \frac{1}{N(N-1)}\begin{pmatrix} 2N_1N_0 & \sum_{(i,j)\in\mathcal{S}(1,0)}\boldsymbol{X}_{i,j}^{\top} - \sum_{(i,j)\in\mathcal{S}(0,1)}\boldsymbol{X}_{i,j}^{\top} & \sum_{(i,j)\in\mathcal{S}}\boldsymbol{X}_{i,j}^{\top} \\ * & \sum_{i\neq j}\boldsymbol{X}_{i,j}\boldsymbol{X}_{i,j}^{\top} & \sum_{(i,j)\in\mathcal{S}(1,0)}\boldsymbol{X}_{i,j}\boldsymbol{X}_{i,j}^{\top} - \sum_{(i,j)\in\mathcal{S}(0,1)}\boldsymbol{X}_{i,j}\boldsymbol{X}_{i,j}^{\top} \\ * & * & \sum_{(i,j)\in\mathcal{S}}\boldsymbol{X}_{i,j}\boldsymbol{X}_{i,j}^{\top} \end{pmatrix}, \tag{S22}$$

with its expectation

$$\boldsymbol{\Gamma}^{\mathrm{adj}}_{\mathrm{P}} = \begin{pmatrix} 2\pi_1\pi_0 & \mathbf{0} & \mathbf{0} \\ * & \frac{1}{N(N-1)}\sum_{i\neq j}\boldsymbol{X}_{i,j}\boldsymbol{X}_{i,j}^{\top} & \mathbf{0} \\ * & * & \frac{2\pi_1\pi_0}{N(N-1)}\sum_{i\neq j}\boldsymbol{X}_{i,j}\boldsymbol{X}_{i,j}^{\top} \end{pmatrix}. \tag{S23}$$

We have the following lemma.

**Lemma S22.** *Under Conditions 1-3 in the main article, then*

$$\frac{1}{N(N-1)^2}\sum_{i=1}^{N}\left(\sum_{j:j\neq i}D_{i,j}\widehat{r}^{\mathrm{adj}}_{\mathrm{P},i,j}\right)^2 - \frac{\pi_1\pi_0^2}{N}\sum_{i=1}^{N}\overline{r}^{\mathrm{adj}}_{\mathrm{P},i,\cdot}(1,0)^2 - \frac{\pi_1^2\pi_0}{N}\sum_{i=1}^{N}\overline{r}^{\mathrm{adj}}_{\mathrm{P},i,\cdot}(0,1)^2 = o_{\mathbb{P}}(1), \tag{S24}$$

$$\frac{1}{N(N-1)^2}\sum_{i=1}^{N}\sum_{j:j\neq i}D_{i,j}\widehat{r}^{\mathrm{adj}}_{\mathrm{P},i,j}\sum_{j:j\neq i}D_{j,i}\widehat{r}^{\mathrm{adj}}_{\mathrm{P},j,i} + \frac{\pi_0\pi_1^2}{N}\sum_{i=1}^{N}\overline{r}^{\mathrm{adj}}_{\mathrm{P},\cdot,i}(1,0)\overline{r}^{\mathrm{adj}}_{\mathrm{P},i,\cdot}(0,1)$$

$$+\frac{\pi_1\pi_0^2}{N}\sum_{i=1}^{N}\overline{r}^{\mathrm{adj}}_{\mathrm{P},i,\cdot}(1,0)\overline{r}^{\mathrm{adj}}_{\mathrm{P},\cdot,i}(0,1)=o_{\mathbb{P}}(1), \tag{S25}$$

$$\frac{1}{N(N-1)^2}\sum_{i\neq j}\left\{D_{i,j}D_{j,i}\widehat{r}^{\mathrm{adj}}_{\mathrm{P},i,j}\widehat{r}^{\mathrm{adj}}_{\mathrm{P},j,i}+D_{i,j}^2(\widehat{r}^{\mathrm{adj}}_{\mathrm{P},i,j})^2\right\}=o_{\mathbb{P}}(1), \tag{S26}$$

$$\frac{1}{N(N-1)^2}\sum_{i\neq j}\left\{D_{i,j}\widehat{r}^{\mathrm{adj}}_{\mathrm{P},i,j}\boldsymbol{X}_{j,i}^\top\widehat{r}^{\mathrm{adj}}_{\mathrm{P},j,i}+D_{i,j}\boldsymbol{X}_{i,j}^\top(\widehat{r}^{\mathrm{adj}}_{\mathrm{P},i,j})^2\right\}=\boldsymbol{o}_{\mathbb{P}}(1), \tag{S27}$$

$$\frac{1}{N(N-1)^2}\sum_{i\neq j}\left\{D_{i,j}D_{j,i}\widehat{r}^{\mathrm{adj}}_{\mathrm{P},i,j}\boldsymbol{X}_{j,i}^\top\widehat{r}^{\mathrm{adj}}_{\mathrm{P},j,i}+D_{i,j}^2\boldsymbol{X}_{i,j}^\top(\widehat{r}^{\mathrm{adj}}_{\mathrm{P},i,j})^2\right\}=\boldsymbol{o}_{\mathbb{P}}(1), \tag{S28}$$

$$\frac{1}{N(N-1)^2}\sum_{i\neq j}\left\{\boldsymbol{X}_{i,j}\boldsymbol{X}_{j,i}^\top\widehat{r}^{\mathrm{adj}}_{\mathrm{P},i,j}\widehat{r}^{\mathrm{adj}}_{\mathrm{P},j,i}+\boldsymbol{X}_{i,j}\boldsymbol{X}_{i,j}^\top(\widehat{r}^{\mathrm{adj}}_{\mathrm{P},i,j})^2\right\}=\boldsymbol{o}_{\mathbb{P}}(1), \tag{S29}$$

$$\frac{1}{N(N-1)^2}\sum_{i\neq j}\left\{D_{j,i}\boldsymbol{X}_{i,j}\boldsymbol{X}_{j,i}^\top\widehat{r}^{\mathrm{adj}}_{\mathrm{P},i,j}\widehat{r}^{\mathrm{adj}}_{\mathrm{P},j,i}+D_{i,j}\boldsymbol{X}_{i,j}\boldsymbol{X}_{i,j}^\top(\widehat{r}^{\mathrm{adj}}_{\mathrm{P},i,j})^2\right\}=\boldsymbol{o}_{\mathbb{P}}(1), \tag{S30}$$

$$\frac{1}{N(N-1)^2}\sum_{i\neq j}\left\{D_{i,j}D_{j,i}\boldsymbol{X}_{i,j}\boldsymbol{X}_{j,i}^\top\widehat{r}^{\mathrm{adj}}_{\mathrm{P},i,j}\widehat{r}^{\mathrm{adj}}_{\mathrm{P},j,i}+D_{i,j}^2\boldsymbol{X}_{i,j}\boldsymbol{X}_{i,j}^\top(\widehat{r}^{\mathrm{adj}}_{\mathrm{P},i,j})^2\right\}=\boldsymbol{o}_{\mathbb{P}}(1), \tag{S31}$$

$$\frac{1}{N(N-1)^2}\sum_{i=1}^{N}\sum_{j:j\neq i}D_{i,j}\widehat{r}^{\mathrm{adj}}_{\mathrm{P},i,j}\sum_{j:j\neq i}\boldsymbol{X}_{i,j}^\top\widehat{r}^{\mathrm{adj}}_{\mathrm{P},i,j}=\boldsymbol{O}_{\mathbb{P}}(1), \tag{S32}$$

$$\frac{1}{N(N-1)^2}\sum_{i=1}^{N}\sum_{j:j\neq i}D_{i,j}\widehat{r}^{\mathrm{adj}}_{\mathrm{P},i,j}\sum_{j:j\neq i}D_{i,j}\boldsymbol{X}_{i,j}^\top\widehat{r}^{\mathrm{adj}}_{\mathrm{P},i,j}=\boldsymbol{O}_{\mathbb{P}}(1), \tag{S33}$$

$$\frac{1}{N(N-1)^2}\sum_{i=1}^{N}\sum_{j:j\neq i}D_{i,j}\widehat{r}^{\mathrm{adj}}_{\mathrm{P},i,j}\sum_{j:j\neq i}\boldsymbol{X}_{j,i}^\top\widehat{r}^{\mathrm{adj}}_{\mathrm{P},j,i}=\boldsymbol{O}_{\mathbb{P}}(1), \tag{S34}$$

$$\frac{1}{N(N-1)^2}\sum_{i=1}^{N}\sum_{j:j\neq i}D_{i,j}\widehat{r}^{\mathrm{adj}}_{\mathrm{P},i,j}\sum_{j:j\neq i}D_{j,i}\boldsymbol{X}_{j,i}^\top\widehat{r}^{\mathrm{adj}}_{\mathrm{P},j,i}=\boldsymbol{O}_{\mathbb{P}}(1), \tag{S35}$$

$$\frac{1}{N(N-1)^2}\sum_{i=1}^{N}\sum_{j:j\neq i}\boldsymbol{X}_{i,j}\widehat{r}^{\mathrm{adj}}_{\mathrm{P},i,j}\sum_{j:j\neq i}\boldsymbol{X}_{i,j}^\top\widehat{r}^{\mathrm{adj}}_{\mathrm{P},i,j}=\boldsymbol{O}_{\mathbb{P}}(1), \tag{S36}$$

$$\frac{1}{N(N-1)^2}\sum_{i=1}^{N}\sum_{j:j\neq i}\boldsymbol{X}_{i,j}\widehat{r}^{\mathrm{adj}}_{\mathrm{P},i,j}\sum_{j:j\neq i}D_{i,j}\boldsymbol{X}_{i,j}^\top\widehat{r}^{\mathrm{adj}}_{\mathrm{P},i,j}=\boldsymbol{O}_{\mathbb{P}}(1), \tag{S37}$$

$$\frac{1}{N(N-1)^2}\sum_{i=1}^{N}\sum_{j:j\neq i}D_{i,j}\boldsymbol{X}_{i,j}\widehat{r}^{\mathrm{adj}}_{\mathrm{P},i,j}\sum_{j:j\neq i}D_{i,j}\boldsymbol{X}_{i,j}^\top\widehat{r}^{\mathrm{adj}}_{\mathrm{P},i,j}=\boldsymbol{O}_{\mathbb{P}}(1), \tag{S38}$$

$$\frac{1}{N(N-1)^2}\sum_{i=1}^{N}\sum_{j:j\neq i}\boldsymbol{X}_{i,j}\widehat{r}^{\mathrm{adj}}_{\mathrm{P},i,j}\sum_{j:j\neq i}\boldsymbol{X}_{j,i}^\top\widehat{r}^{\mathrm{adj}}_{\mathrm{P},j,i}=\boldsymbol{O}_{\mathbb{P}}(1), \tag{S39}$$

$$\frac{1}{N(N-1)^2}\sum_{i=1}^{N}\sum_{j:j\neq i}\boldsymbol{X}_{i,j}\widehat{r}^{\mathrm{adj}}_{\mathrm{P},i,j}\sum_{j:j\neq i}D_{j,i}\boldsymbol{X}_{j,i}^\top\widehat{r}^{\mathrm{adj}}_{\mathrm{P},j,i}=\boldsymbol{O}_{\mathbb{P}}(1), \tag{S40}$$

$$\frac{1}{N(N-1)^2}\sum_{i=1}^{N}\sum_{j:j\neq i}D_{i,j}\boldsymbol{X}_{i,j}\widehat{r}^{\mathrm{adj}}_{\mathrm{P},i,j}\sum_{j:j\neq i}D_{j,i}\boldsymbol{X}_{j,i}^\top\widehat{r}^{\mathrm{adj}}_{\mathrm{P},j,i}=\boldsymbol{O}_{\mathbb{P}}(1). \tag{S41}$$

*Similar results can be obtained for terms with summations over $i: i\neq j$ and $j=1,\ldots,N$.*

Since $D_{i,j}=A_i-A_j=A_i(1-A_j)-A_j(1-A_i)$ and $D_{i,j}^2=A_i(1-A_j)+A_j(1-A_i)$, we have (S24) and (S25) implied by (S7), (S26) implied by (S3), (S27) and (S28) implied by (S4), (S29) - (S31) implied by (S5), (S32) - (S35) implied by (S8), and (S36)

- (S41) implied by (S9). By Lemma S22,

$$\overline{\mathbf{M}}^{\text{adj}}_{\text{P,CTW}} = \frac{1}{N(N-1)^2}\mathbf{M}^{\text{adj}}_{\text{P,CTW}} = \boldsymbol{O}_{\mathbb{P}}(1).$$

We now analyze the CTW variance estimators. Using similar arguments in the proof of the HR variance estimator for $\widehat{\lambda}^{\text{adj}}_{\text{I}}(a, 1-a)$, we have

$$(\mathbf{G}^{\text{adj}}_{\text{P}})^{-1}\overline{\mathbf{M}}^{\text{adj}}_{\text{P,CTW}}(\mathbf{G}^{\text{adj}}_{\text{P}})^{-1} - (\boldsymbol{\Gamma}^{\text{adj}}_{\text{P}})^{-1}\overline{\mathbf{M}}^{\text{adj}}_{\text{P,CTW}}(\boldsymbol{\Gamma}^{\text{adj}}_{\text{P}})^{-1} = \boldsymbol{o}_{\mathbb{P}}(1).$$

Then, by Lemma S22,

$$\begin{aligned}
&N\widehat{\text{se}}^2_{\text{CTW}}\left\{\widehat{\tau}^{\text{adj}}_{\text{P}}(1)\right\} = 4\left[(\boldsymbol{\Gamma}^{\text{adj}}_{\text{P}})^{-1}\overline{\mathbf{M}}^{\text{adj}}_{\text{P,CTW}}(\boldsymbol{\Gamma}^{\text{adj}}_{\text{P}})^{-1}\right]_{(1,1)} + o_{\mathbb{P}}(1)\\
&= \frac{1}{N(N-1)^2}\cdot\frac{1}{\pi_1^2\pi_0^2}\sum_{i=1}^{N}\left(\sum_{j:j\neq i} D_{i,j}\widehat{r}^{\text{adj}}_{\text{P},i,j}\right)^2 + \frac{1}{N(N-1)^2}\cdot\frac{1}{\pi_1^2\pi_0^2}\sum_{j=1}^{N}\left(\sum_{i:i\neq j} D_{i,j}\widehat{r}^{\text{adj}}_{\text{P},i,j}\right)^2\\
&\quad + \frac{1}{N(N-1)^2}\cdot\frac{1}{\pi_1^2\pi_0^2}\sum_{i=1}^{N}\sum_{j:j\neq i} D_{i,j}\widehat{r}^{\text{adj}}_{\text{P},i,j}\sum_{j:j\neq i} D_{j,i}\widehat{r}^{\text{adj}}_{\text{P},j,i} + \frac{1}{N(N-1)^2}\cdot\frac{1}{\pi_1^2\pi_0^2}\sum_{j=1}^{N}\sum_{i:i\neq j} D_{i,j}\widehat{r}^{\text{adj}}_{\text{P},i,j}\sum_{i:i\neq j} D_{j,i}\widehat{r}^{\text{adj}}_{\text{P},j,i} + o_{\mathbb{P}}(1)\\
&= \frac{1}{\pi_1 N}\sum_{i=1}^{N}\overline{r}^{\text{adj}}_{\text{P},i,\cdot}(1,0)^2 + \frac{1}{\pi_0 N}\sum_{i=1}^{N}\overline{r}^{\text{adj}}_{\text{P},i,\cdot}(0,1)^2 + \frac{1}{\pi_0 N}\sum_{j=1}^{N}\overline{r}^{\text{adj}}_{\text{P},\cdot,j}(1,0)^2 + \frac{1}{\pi_1 N}\sum_{j=1}^{N}\overline{r}^{\text{adj}}_{\text{P},\cdot,j}(0,1)^2\\
&\quad - \frac{1}{\pi_0 N}\sum_{i=1}^{N}\overline{r}^{\text{adj}}_{\text{P},\cdot,i}(1,0)\overline{r}^{\text{adj}}_{\text{P},i,\cdot}(0,1) - \frac{1}{\pi_1 N}\sum_{i=1}^{N}\overline{r}^{\text{adj}}_{\text{P},i,\cdot}(1,0)\overline{r}^{\text{adj}}_{\text{P},\cdot,i}(0,1)\\
&\quad - \frac{1}{\pi_1 N}\sum_{j=1}^{N}\overline{r}^{\text{adj}}_{\text{P},j,\cdot}(1,0)\overline{r}^{\text{adj}}_{\text{P},\cdot,j}(0,1) - \frac{1}{\pi_0 N}\sum_{j=1}^{N}\overline{r}^{\text{adj}}_{\text{P},\cdot,j}(1,0)\overline{r}^{\text{adj}}_{\text{P},j,\cdot}(0,1) + o_{\mathbb{P}}(1),
\end{aligned}$$

which, after relabeling, is

$$\frac{1}{\pi_1 N}\sum_{i=1}^{N}\{\overline{r}_{\text{P},i,\cdot}(1,0) - \overline{r}_{\text{P},\cdot,i}(0,1)\}^2 + \frac{1}{\pi_0 N}\sum_{i=1}^{N}\{\overline{r}_{\text{P},i,\cdot}(0,1) - \overline{r}_{\text{P},\cdot,i}(1,0)\}^2 + o_{\mathbb{P}}(1).$$

The probability limit of $N\widehat{\text{se}}^2_{\text{CTW}}\{\widehat{\tau}^{\text{adj}}_{\text{P}}(1)\}$ is $V_c(\overline{r}^{\text{adj}}_{\text{P},i})$.

### S5.2.2 The HR variance estimators

We prove that the HR variance estimators are not consistent for the variances of the PIM estimators. We focus on $\widehat{\tau}^{\text{adj}}_{\text{P}}(1)$. We continue with the design matrix $\mathbf{Z}^{\text{adj}}_{\text{P}}$. The HR variance estimator is

$$\widehat{\text{se}}^2_{\text{HR}}\left\{\widehat{\tau}^{\text{adj}}_{\text{P}}(1)\right\} = 4\left[\left(\mathbf{Z}^{\text{adj}\top}_{\text{P}}\mathbf{Z}^{\text{adj}}_{\text{P}}\right)^{-1}\mathbf{M}^{\text{adj}}_{\text{P,HR}}\left(\mathbf{Z}^{\text{adj}\top}_{\text{P}}\mathbf{Z}^{\text{adj}}_{\text{P}}\right)^{-1}\right]_{(1,1)},$$

where,

$$\mathbf{M}^{\text{adj}}_{\text{P,HR}} = \sum_{i\neq j}\boldsymbol{Z}^{\text{adj}}_{\text{P},i,j}\boldsymbol{Z}^{\text{adj}\top}_{\text{P},i,j}(\widehat{r}^{\text{adj}}_{\text{P},i,j})^2.$$

$\mathbf{M}^{\text{adj}}_{\text{P,HR}}$ is symmetric, with

$$\mathbf{M}^{\text{adj}}_{\text{P,HR}} = \begin{pmatrix} \mathbf{M}^{\text{adj}}_{\text{P,HR}}[1,1] & \mathbf{M}^{\text{adj}}_{\text{P,HR}}[1,2] & \mathbf{M}^{\text{adj}}_{\text{P,HR}}[1,3] \\ * & \mathbf{M}^{\text{adj}}_{\text{P,HR}}[2,2] & \mathbf{M}^{\text{adj}}_{\text{P,HR}}[2,3] \\ * & * & \mathbf{M}^{\text{adj}}_{\text{P,HR}}[3,3] \end{pmatrix},$$

where $*$ denotes the symmetric components. Then,

$$\mathbf{M}^{\text{adj}}_{\text{P,HR}}[1,1] = \sum_{i\neq j} D^2_{i,j}(\widehat{r}^{\text{adj}}_{\text{P},i,j})^2, \quad \mathbf{M}^{\text{adj}}_{\text{P,HR}}[1,2] = \sum_{i\neq j} D_{i,j}\boldsymbol{X}^\top_{i,j}(\widehat{r}^{\text{adj}}_{\text{P},i,j})^2,$$
$$\mathbf{M}^{\text{adj}}_{\text{P,HR}}[1,3] = \sum_{i\neq j} D^2_{i,j}\boldsymbol{X}^\top_{i,j}(\widehat{r}^{\text{adj}}_{\text{P},i,j})^2, \quad \mathbf{M}^{\text{adj}}_{\text{P,HR}}[2,2] = \sum_{i\neq j} \boldsymbol{X}_{i,j}\boldsymbol{X}^\top_{i,j}(\widehat{r}^{\text{adj}}_{\text{P},i,j})^2,$$
$$\mathbf{M}^{\text{adj}}_{\text{P,HR}}[2,3] = \sum_{i\neq j} D_{i,j}\boldsymbol{X}_{i,j}\boldsymbol{X}^\top_{i,j}(\widehat{r}^{\text{adj}}_{\text{P},i,j})^2, \quad \mathbf{M}^{\text{adj}}_{\text{P,HR}}[3,3] = \sum_{i\neq j} D^2_{i,j}\boldsymbol{X}_{i,j}\boldsymbol{X}^\top_{i,j}(\widehat{r}^{\text{adj}}_{\text{P},i,j})^2.$$

We have the following lemma.

**Lemma S23.** *Under Conditions 1-3 in the main article, then*

$$\frac{1}{N(N-1)}\sum_{i\neq j} D^2_{i,j}(\widehat{r}^{\text{adj}}_{\text{P},i,j})^2 - \frac{\pi_1\pi_0}{N(N-1)}\sum_{i\neq j} r^{\text{adj}}_{\text{P},i,j}(1,0)^2 - \frac{\pi_1\pi_0}{N(N-1)}\sum_{i\neq j} r^{\text{adj}}_{\text{P},i,j}(0,1)^2 = o_{\mathbb{P}}(1), \tag{S42}$$

$$\frac{1}{N(N-1)}\sum_{i\neq j} D_{i,j}\boldsymbol{X}^\top_{i,j}(\widehat{r}^{\text{adj}}_{\text{P},i,j})^2 = \boldsymbol{O}_{\mathbb{P}}(1), \tag{S43}$$

$$\frac{1}{N(N-1)}\sum_{i\neq j} D^2_{i,j}\boldsymbol{X}^\top_{i,j}(\widehat{r}^{\text{adj}}_{\text{P},i,j})^2 = \boldsymbol{O}_{\mathbb{P}}(1), \tag{S44}$$

$$\frac{1}{N(N-1)}\sum_{i\neq j} \boldsymbol{X}_{i,j}\boldsymbol{X}^\top_{i,j}(\widehat{r}^{\text{adj}}_{\text{P},i,j})^2 = \boldsymbol{O}_{\mathbb{P}}(1), \tag{S45}$$

$$\frac{1}{N(N-1)}\sum_{i\neq j} D_{i,j}\boldsymbol{X}_{i,j}\boldsymbol{X}^\top_{i,j}(\widehat{r}^{\text{adj}}_{\text{P},i,j})^2 = \boldsymbol{O}_{\mathbb{P}}(1), \tag{S46}$$

$$\frac{1}{N(N-1)}\sum_{i\neq j} D^2_{i,j}\boldsymbol{X}_{i,j}\boldsymbol{X}^\top_{i,j}(\widehat{r}^{\text{adj}}_{\text{P},i,j})^2 = \boldsymbol{O}_{\mathbb{P}}(1). \tag{S47}$$

We have (S42) implied by (S3), (S43) and (S44) implied by (S4), and (S45) - (S47) implied by (S5). By Lemma S23,

$$\overline{\mathbf{M}}^{\text{adj}}_{\text{P,HR}} = \frac{1}{N(N-1)}\mathbf{M}^{\text{adj}}_{\text{P,HR}} = \boldsymbol{O}_{\mathbb{P}}(1).$$

We now analyze the HR variance estimators. Using similar arguments in the proof of the HR variance estimators for $\widehat{\lambda}^{\text{adj}}_{\text{I}}(a, 1-a)$, we have

$$(\mathbf{G}^{\text{adj}}_{\text{P}})^{-1}\overline{\mathbf{M}}^{\text{adj}}_{\text{P,HR}}(\mathbf{G}^{\text{adj}}_{\text{P}})^{-1} - (\boldsymbol{\Gamma}^{\text{adj}}_{\text{P}})^{-1}\overline{\mathbf{M}}^{\text{adj}}_{\text{P,HR}}(\boldsymbol{\Gamma}^{\text{adj}}_{\text{P}})^{-1} = \boldsymbol{o}_{\mathbb{P}}(1),$$

where $\mathbf{G}^{\text{adj}}_{\text{P}}$ is defined in (S22) and $\boldsymbol{\Gamma}^{\text{adj}}_{\text{P}}$ is defined in (S23). Then, by Lemma S23,

$$\begin{aligned} N(N-1)\widehat{\text{se}}^2_{\text{HR}}\left\{\widehat{\tau}^{\text{adj}}_{\text{P}}(1)\right\} &= 4\left[(\boldsymbol{\Gamma}^{\text{adj}}_{\text{P}})^{-1}\overline{\mathbf{M}}^{\text{adj}}_{\text{P,HR}}(\boldsymbol{\Gamma}^{\text{adj}}_{\text{P}})^{-1}\right]_{(1,1)} + o_{\mathbb{P}}(1) \\ &= \frac{1}{N(N-1)}\cdot\frac{1}{\pi_1^2\pi_0^2}\sum_{i\neq j} D^2_{i,j}(\widehat{r}^{\text{adj}}_{\text{P},i,j})^2 + o_{\mathbb{P}}(1) \end{aligned}$$

$$= \frac{1}{\pi_1\pi_0 N(N-1)} \sum_{i\neq j} r^{\mathrm{adj}}_{\mathrm{P},i,j}(1,0)^2 + \frac{1}{\pi_1\pi_0 N(N-1)} \sum_{i\neq j} r^{\mathrm{adj}}_{\mathrm{P},i,j}(0,1)^2 + o_{\mathbb{P}}(1).$$

Thus, the probability limit of $N(N-1)\widehat{\mathrm{se}}^2_{\mathrm{HR}}\{\widehat{\tau}^{\mathrm{adj}}_{\mathrm{P}}(1)\}$ is not $V(\overline{r}^{\mathrm{adj}}_{\mathrm{P},i})$ or $V_c(\overline{r}^{\mathrm{adj}}_{\mathrm{P},i})$.

### S5.2.3 The CR variance estimators

We prove that the CR variance estimators are not consistent for the leading terms of the variances of the PIM estimators. We focus on $\widehat{\tau}^{\mathrm{adj}}_{\mathrm{P}}(1)$ and continue with design matrix $\mathbf{Z}^{\mathrm{adj}}_{\mathrm{P}}$. Stack $\boldsymbol{Z}^{\mathrm{adj}\top}_{\mathrm{P},i,j}$ to create $\mathbf{Z}^{\mathrm{adj}}_{\mathrm{P},i}$. The CR variance estimator is

$$\widehat{\mathrm{se}}^2_{\mathrm{CR}}\left\{\widehat{\tau}^{\mathrm{adj}}_{\mathrm{P}}(1)\right\} = 4\left[\left(\mathbf{Z}^{\mathrm{adj}\top}_{\mathrm{P}}\mathbf{Z}^{\mathrm{adj}}_{\mathrm{P}}\right)^{-1}\mathbf{M}^{\mathrm{adj}}_{\mathrm{P,CR}}\left(\mathbf{Z}^{\mathrm{adj}\top}_{\mathrm{P}}\mathbf{Z}^{\mathrm{adj}}_{\mathrm{P}}\right)^{-1}\right]_{(1,1)},$$

where,

$$\mathbf{M}^{\mathrm{adj}}_{\mathrm{P,CR}} = \sum_{i=1}^{N} \mathbf{Z}^{\mathrm{adj}\top}_{\mathrm{P},i}\widehat{\mathbf{R}}^{\mathrm{adj}}_{\mathrm{P},i}\mathbf{Z}^{\mathrm{adj}}_{\mathrm{P},i},$$

where $\widehat{\mathbf{R}}^{\mathrm{adj}}_{\mathrm{P},i}$ is an $(N-1)\times(N-1)$ matrix with $[\widehat{\mathbf{R}}^{\mathrm{adj}}_{\mathrm{P},i}]_{(j,k)} = \widehat{r}^{\mathrm{adj}}_{\mathrm{P},i,j}\widehat{r}^{\mathrm{adj}}_{\mathrm{P},i,k}$ for $j\neq i, k\neq i$. $\mathbf{M}^{\mathrm{adj}}_{\mathrm{P,CR}}$ is symmetric, with

$$\mathbf{M}^{\mathrm{adj}}_{\mathrm{P,CR}} = \begin{pmatrix} \mathrm{M}^{\mathrm{adj}}_{\mathrm{P,CR}}[1,1] & \mathbf{M}^{\mathrm{adj}}_{\mathrm{P,CR}}[1,2] & \mathbf{M}^{\mathrm{adj}}_{\mathrm{P,CR}}[1,3] \\ * & \mathbf{M}^{\mathrm{adj}}_{\mathrm{P,CR}}[2,2] & \mathbf{M}^{\mathrm{adj}}_{\mathrm{P,CR}}[2,3] \\ * & * & \mathbf{M}^{\mathrm{adj}}_{\mathrm{P,CR}}[3,3] \end{pmatrix},$$

where $*$ denotes the symmetric components. Then,

$$\mathrm{M}^{\mathrm{adj}}_{\mathrm{P,CR}}[1,1] = \sum_{i=1}^{N}\left(\sum_{j:j\neq i} D_{i,j}\widehat{r}^{\mathrm{adj}}_{\mathrm{P},i,j}\right)^2,$$

$$\mathbf{M}^{\mathrm{adj}}_{\mathrm{P,CR}}[1,2] = \sum_{i=1}^{N}\sum_{j:j\neq i} D_{i,j}\widehat{r}^{\mathrm{adj}}_{\mathrm{P},i,j}\sum_{j:j\neq i}\boldsymbol{X}^{\top}_{i,j}\widehat{r}^{\mathrm{adj}}_{\mathrm{P},i,j},$$

$$\mathbf{M}^{\mathrm{adj}}_{\mathrm{P,CR}}[1,3] = \sum_{i=1}^{N}\sum_{j:j\neq i} D_{i,j}\widehat{r}^{\mathrm{adj}}_{\mathrm{P},i,j}\sum_{j:j\neq i} D_{i,j}\boldsymbol{X}^{\top}_{i,j}\widehat{r}^{\mathrm{adj}}_{\mathrm{P},i,j},$$

$$\mathbf{M}^{\mathrm{adj}}_{\mathrm{P,CR}}[2,2] = \sum_{i=1}^{N}\sum_{j:j\neq i}\boldsymbol{X}_{i,j}\widehat{r}^{\mathrm{adj}}_{\mathrm{P},i,j}\sum_{j:j\neq i}\boldsymbol{X}^{\top}_{i,j}\widehat{r}^{\mathrm{adj}}_{\mathrm{P},i,j},$$

$$\mathbf{M}^{\mathrm{adj}}_{\mathrm{P,CR}}[2,3] = \sum_{i=1}^{N}\sum_{j:j\neq i}\boldsymbol{X}_{i,j}\widehat{r}^{\mathrm{adj}}_{\mathrm{P},i,j}\sum_{j:j\neq i} D_{i,j}\boldsymbol{X}^{\top}_{i,j}\widehat{r}^{\mathrm{adj}}_{\mathrm{P},i,j},$$

$$\mathbf{M}^{\mathrm{adj}}_{\mathrm{P,CR}}[3,3] = \sum_{i=1}^{N}\sum_{j:j\neq i} D_{i,j}\boldsymbol{X}_{i,j}\widehat{r}^{\mathrm{adj}}_{\mathrm{P},i,j}\sum_{j:j\neq i} D_{i,j}\boldsymbol{X}^{\top}_{i,j}\widehat{r}^{\mathrm{adj}}_{\mathrm{P},i,j}.$$

By Lemma S22, under Conditions 1-3 in the main article,

$$\frac{1}{N(N-1)^2}\sum_{i=1}^{N}\left(\sum_{j:j\neq i} D_{i,j}\widehat{r}^{\mathrm{adj}}_{\mathrm{P},i,j}\right)^2 - \frac{\pi_1\pi_0^2}{N}\sum_{i=1}^{N}\overline{r}^{\mathrm{adj}}_{\mathrm{P},i,\cdot}(1,0)^2 - \frac{\pi_1^2\pi_0}{N}\sum_{i=1}^{N}\overline{r}^{\mathrm{adj}}_{\mathrm{P},i,\cdot}(0,1)^2 = o_{\mathbb{P}}(1),$$

$$\frac{1}{N(N-1)^2}\sum_{i=1}^{N}\sum_{j:j\neq i} D_{i,j}\widehat{r}^{\mathrm{adj}}_{\mathrm{P},i,j}\sum_{j:j\neq i}\boldsymbol{X}^{\top}_{i,j}\widehat{r}^{\mathrm{adj}}_{\mathrm{P},i,j} = \boldsymbol{O}_{\mathbb{P}}(1),$$

$$\frac{1}{N(N-1)^2}\sum_{i=1}^{N}\sum_{j:j\neq i} D_{i,j}\widehat{r}^{\text{adj}}_{\text{P},i,j}\sum_{j:j\neq i} D_{i,j}\boldsymbol{X}^{\top}_{i,j}\widehat{r}^{\text{adj}}_{\text{P},i,j} = \boldsymbol{O}_{\mathbb{P}}(1),$$
$$\frac{1}{N(N-1)^2}\sum_{i=1}^{N}\sum_{j:j\neq i} \boldsymbol{X}_{i,j}\widehat{r}^{\text{adj}}_{\text{P},i,j}\sum_{j:j\neq i} \boldsymbol{X}^{\top}_{i,j}\widehat{r}^{\text{adj}}_{\text{P},i,j} = \boldsymbol{O}_{\mathbb{P}}(1),$$
$$\frac{1}{N(N-1)^2}\sum_{i=1}^{N}\sum_{j:j\neq i} \boldsymbol{X}_{i,j}\widehat{r}^{\text{adj}}_{\text{P},i,j}\sum_{j:j\neq i} D_{i,j}\boldsymbol{X}^{\top}_{i,j}\widehat{r}^{\text{adj}}_{\text{P},i,j} = \boldsymbol{O}_{\mathbb{P}}(1),$$
$$\frac{1}{N(N-1)^2}\sum_{i=1}^{N}\sum_{j:j\neq i} D_{i,j}\boldsymbol{X}_{i,j}\widehat{r}^{\text{adj}}_{\text{P},i,j}\sum_{j:j\neq i} D_{i,j}\boldsymbol{X}^{\top}_{i,j}\widehat{r}^{\text{adj}}_{\text{P},i,j} = \boldsymbol{O}_{\mathbb{P}}(1).$$

Then,

$$\overline{\mathbf{M}}^{\text{adj}}_{\text{P,CR}} = \frac{1}{N(N-1)^2}\mathbf{M}^{\text{adj}}_{\text{P,CR}} = \boldsymbol{O}_{\mathbb{P}}(1).$$

We now analyze the CR variance estimators. Using similar arguments in the proof of the HR variance estimator for $\widehat{\lambda}^{\text{adj}}_{\text{I}}(a, 1-a)$, we have

$$(\mathbf{G}^{\text{adj}}_{\text{P}})^{-1}\overline{\mathbf{M}}^{\text{adj}}_{\text{P,CR}}(\mathbf{G}^{\text{adj}}_{\text{P}})^{-1} - (\boldsymbol{\Gamma}^{\text{adj}}_{\text{P}})^{-1}\overline{\mathbf{M}}^{\text{adj}}_{\text{P,CR}}(\boldsymbol{\Gamma}^{\text{adj}}_{\text{P}})^{-1} = \boldsymbol{o}_{\mathbb{P}}(1),$$

where $\mathbf{G}^{\text{adj}}_{\text{P}}$ is defined in (S22) and $\boldsymbol{\Gamma}^{\text{adj}}_{\text{P}}$ is defined in (S23). Then, by Lemma S22,

$$\begin{aligned}
N\widehat{\text{se}}^2_{\text{CR}}\left\{\widehat{\tau}^{\text{adj}}_{\text{P}}(1)\right\} &= 4\left[(\boldsymbol{\Gamma}^{\text{adj}}_{\text{P}})^{-1}\overline{\mathbf{M}}^{\text{adj}}_{\text{P,CR}}(\boldsymbol{\Gamma}^{\text{adj}}_{\text{P}})^{-1}\right]_{(1,1)} + o_{\mathbb{P}}(1)\\
&= \frac{1}{N(N-1)^2}\cdot\frac{1}{\pi_1^2\pi_0^2}\sum_{i=1}^{N}\left(\sum_{j:j\neq i} D_{i,j}\widehat{r}^{\text{adj}}_{\text{P},i,j}\right)^2 + \frac{1}{N(N-1)^2}\cdot\frac{1}{\pi_1^2\pi_0^2}\sum_{j=1}^{N}\left(\sum_{i:i\neq j} D_{i,j}\widehat{r}^{\text{adj}}_{\text{P},i,j}\right)^2 + o_{\mathbb{P}}(1)\\
&= \frac{1}{\pi_1 N}\sum_{i=1}^{N}\overline{r}^{\text{adj}}_{\text{P},i,\cdot}(1,0)^2 + \frac{1}{\pi_0 N}\sum_{i=1}^{N}\overline{r}^{\text{adj}}_{\text{P},i,\cdot}(0,1)^2 + o_{\mathbb{P}}(1).
\end{aligned}$$

Thus, the probability limit of $N\widehat{\text{se}}^2_{\text{CR}}\{\widehat{\tau}^{\text{adj}}_{\text{P}}(1)\}$ is not $V(\overline{r}^{\text{adj}}_{\text{P},i})$ or $V_c(\overline{r}^{\text{adj}}_{\text{P},i})$.

#### S5.2.4 The TW variance estimators

We prove that the TW variance estimators are not consistent for the leading terms of the variances of the PIM estimators. We focus on $\widehat{\tau}^{\text{adj}}_{\text{P}}(1)$ and continue with the design matrix $\mathbf{Z}^{\text{adj}}_{\text{P}}$. The TW variance estimator is

$$\widehat{\text{se}}^2_{\text{TW}}\left\{\widehat{\tau}^{\text{adj}}_{\text{P}}(1)\right\} = 4\left[\left(\mathbf{Z}^{\text{adj}\top}_{\text{P}}\mathbf{Z}^{\text{adj}}_{\text{P}}\right)^{-1}\mathbf{M}^{\text{adj}}_{\text{P,TW}}\left(\mathbf{Z}^{\text{adj}\top}_{\text{P}}\mathbf{Z}^{\text{adj}}_{\text{P}}\right)^{-1}\right]_{(1,1)},$$

where,

$$\begin{aligned}
\mathbf{M}^{\text{adj}}_{\text{P,TW}} = &\sum_{i=1}^{N}\left(\sum_{j:j\neq i}\boldsymbol{Z}^{\text{adj}}_{\text{P},i,j}\widehat{r}^{\text{adj}}_{\text{P},i,j}\right)\left(\sum_{j:j\neq i}\boldsymbol{Z}^{\text{adj}}_{\text{P},i,j}\widehat{r}^{\text{adj}}_{\text{P},i,j}\right)^{\top} + \sum_{j=1}^{N}\left(\sum_{i:i\neq j}\boldsymbol{Z}^{\text{adj}}_{\text{P},i,j}\widehat{r}^{\text{adj}}_{\text{P},i,j}\right)\left(\sum_{i:i\neq j}\boldsymbol{Z}^{\text{adj}}_{\text{P},i,j}\widehat{r}^{\text{adj}}_{\text{P},i,j}\right)^{\top}\\
&-\sum_{i\neq j}\boldsymbol{Z}^{\text{adj}}_{\text{P},i,j}\boldsymbol{Z}^{\text{adj}\top}_{\text{P},i,j}(\widehat{r}^{\text{adj}}_{\text{P},i,j})^2.
\end{aligned}$$

$\mathbf{M}^{\text{adj}}_{\text{P,TW}}$ is symmetric, with

$$\mathbf{M}^{\text{adj}}_{\text{P,TW}} = \begin{pmatrix} \mathrm{M}^{\text{adj}}_{\text{P,TW}}[1,1] & \mathbf{M}^{\text{adj}}_{\text{P,TW}}[1,2] & \mathbf{M}^{\text{adj}}_{\text{P,TW}}[1,3] \\ * & \mathbf{M}^{\text{adj}}_{\text{P,TW}}[2,2] & \mathbf{M}^{\text{adj}}_{\text{P,TW}}[2,3] \\ * & * & \mathbf{M}^{\text{adj}}_{\text{P,TW}}[3,3] \end{pmatrix},$$

where $*$ denotes the symmetric components. Then,

$$\mathrm{M}^{\text{adj}}_{\text{P,TW}}[1,1] = \sum_{i=1}^{N}\left(\sum_{j:j\neq i} D_{i,j}\widehat{r}^{\text{adj}}_{\text{P},i,j}\right)^2 + \sum_{j=1}^{N}\left(\sum_{i:i\neq j} D_{i,j}\widehat{r}^{\text{adj}}_{\text{P},i,j}\right)^2 - \sum_{i\neq j} D^2_{i,j}(\widehat{r}^{\text{adj}}_{\text{P},i,j})^2,$$

$$\mathbf{M}^{\text{adj}}_{\text{P,TW}}[1,2] = \sum_{i=1}^{N}\sum_{j:j\neq i} D_{i,j}\widehat{r}^{\text{adj}}_{\text{P},i,j}\sum_{j:j\neq i}\boldsymbol{X}^{\top}_{i,j}\widehat{r}^{\text{adj}}_{\text{P},i,j} + \sum_{j=1}^{N}\sum_{i:i\neq j} D_{i,j}\widehat{r}^{\text{adj}}_{\text{P},i,j}\sum_{i:i\neq j}\boldsymbol{X}^{\top}_{i,j}\widehat{r}^{\text{adj}}_{\text{P},i,j} - \sum_{i\neq j} D_{i,j}\boldsymbol{X}^{\top}_{i,j}(\widehat{r}^{\text{adj}}_{\text{P},i,j})^2,$$

$$\begin{aligned}\mathbf{M}^{\text{adj}}_{\text{P,TW}}[1,3] = {} & \sum_{i=1}^{N}\sum_{j:j\neq i} D_{i,j}\widehat{r}^{\text{adj}}_{\text{P},i,j}\sum_{j:j\neq i} D_{i,j}\boldsymbol{X}^{\top}_{i,j}\widehat{r}^{\text{adj}}_{\text{P},i,j} + \sum_{j=1}^{N}\sum_{i:i\neq j} D_{i,j}\widehat{r}^{\text{adj}}_{\text{P},i,j}\sum_{i:i\neq j} D_{i,j}\boldsymbol{X}^{\top}_{i,j}\widehat{r}^{\text{adj}}_{\text{P},i,j} \\ & - \sum_{i\neq j} D^2_{i,j}\boldsymbol{X}^{\top}_{i,j}(\widehat{r}^{\text{adj}}_{\text{P},i,j})^2,\end{aligned}$$

$$\begin{aligned}\mathbf{M}^{\text{adj}}_{\text{P,TW}}[2,2] = {} & \sum_{i=1}^{N}\sum_{j:j\neq i} \boldsymbol{X}_{i,j}\widehat{r}^{\text{adj}}_{\text{P},i,j}\sum_{j:j\neq i} \boldsymbol{X}^{\top}_{i,j}\widehat{r}^{\text{adj}}_{\text{P},i,j} + \sum_{j=1}^{N}\sum_{i:i\neq j} \boldsymbol{X}_{i,j}\widehat{r}^{\text{adj}}_{\text{P},i,j}\sum_{i:i\neq j} \boldsymbol{X}^{\top}_{i,j}\widehat{r}^{\text{adj}}_{\text{P},i,j} \\ & - \sum_{i\neq j} \boldsymbol{X}_{i,j}\boldsymbol{X}^{\top}_{i,j}(\widehat{r}^{\text{adj}}_{\text{P},i,j})^2,\end{aligned}$$

$$\begin{aligned}\mathbf{M}^{\text{adj}}_{\text{P,TW}}[2,3] = {} & \sum_{i=1}^{N}\sum_{j:j\neq i} \boldsymbol{X}_{i,j}\widehat{r}^{\text{adj}}_{\text{P},i,j}\sum_{j:j\neq i} D_{i,j}\boldsymbol{X}^{\top}_{i,j}\widehat{r}^{\text{adj}}_{\text{P},i,j} + \sum_{j=1}^{N}\sum_{i:i\neq j} \boldsymbol{X}_{i,j}\widehat{r}^{\text{adj}}_{\text{P},i,j}\sum_{i:i\neq j} D_{i,j}\boldsymbol{X}^{\top}_{i,j}\widehat{r}^{\text{adj}}_{\text{P},i,j} \\ & - \sum_{i\neq j} D_{i,j}\boldsymbol{X}_{i,j}\boldsymbol{X}^{\top}_{i,j}(\widehat{r}^{\text{adj}}_{\text{P},i,j})^2,\end{aligned}$$

$$\begin{aligned}\mathbf{M}^{\text{adj}}_{\text{P,TW}}[3,3] = {} & \sum_{i=1}^{N}\sum_{j:j\neq i} D_{i,j}\boldsymbol{X}_{i,j}\widehat{r}^{\text{adj}}_{\text{P},i,j}\sum_{j:j\neq i} D_{i,j}\boldsymbol{X}^{\top}_{i,j}\widehat{r}^{\text{adj}}_{\text{P},i,j} + \sum_{j=1}^{N}\sum_{i:i\neq j} D_{i,j}\boldsymbol{X}_{i,j}\widehat{r}^{\text{adj}}_{\text{P},i,j}\sum_{i:i\neq j} D_{i,j}\boldsymbol{X}^{\top}_{i,j}\widehat{r}^{\text{adj}}_{\text{P},i,j} \\ & - \sum_{i\neq j} D^2_{i,j}\boldsymbol{X}_{i,j}\boldsymbol{X}^{\top}_{i,j}(\widehat{r}^{\text{adj}}_{\text{P},i,j})^2.\end{aligned}$$

By Lemmas S22 and S23, under Conditions 1-3 in the main article,

$$\frac{1}{N(N-1)^2}\sum_{i=1}^{N}\left(\sum_{j:j\neq i} D_{i,j}\widehat{r}^{\text{adj}}_{\text{P},i,j}\right)^2 - \frac{\pi_1\pi_0^2}{N}\sum_{i=1}^{N}\overline{r}^{\text{adj}}_{\text{P},i,\cdot}(1,0)^2 - \frac{\pi_1^2\pi_0}{N}\sum_{i=1}^{N}\overline{r}^{\text{adj}}_{\text{P},i,\cdot}(0,1)^2 = o_{\mathbb{P}}(1),$$

$$\frac{1}{N(N-1)^2}\sum_{i\neq j} D^2_{i,j}(\widehat{r}^{\text{adj}}_{\text{P},i,j})^2 = o_{\mathbb{P}}(1), \quad \frac{1}{N(N-1)^2}\sum_{i\neq j} D_{i,j}\boldsymbol{X}^{\top}_{i,j}(\widehat{r}^{\text{adj}}_{\text{P},i,j})^2 = \boldsymbol{o}_{\mathbb{P}}(1),$$

$$\frac{1}{N(N-1)^2}\sum_{i\neq j} D^2_{i,j}\boldsymbol{X}^{\top}_{i,j}(\widehat{r}^{\text{adj}}_{\text{P},i,j})^2 = \boldsymbol{o}_{\mathbb{P}}(1), \quad \frac{1}{N(N-1)^2}\sum_{i\neq j} \boldsymbol{X}_{i,j}\boldsymbol{X}^{\top}_{i,j}(\widehat{r}^{\text{adj}}_{\text{P},i,j})^2 = \boldsymbol{o}_{\mathbb{P}}(1),$$

$$\frac{1}{N(N-1)^2}\sum_{i\neq j} D_{i,j}\boldsymbol{X}_{i,j}\boldsymbol{X}^{\top}_{i,j}(\widehat{r}^{\text{adj}}_{\text{P},i,j})^2 = \boldsymbol{o}_{\mathbb{P}}(1), \quad \frac{1}{N(N-1)^2}\sum_{i\neq j} D^2_{i,j}\boldsymbol{X}_{i,j}\boldsymbol{X}^{\top}_{i,j}(\widehat{r}^{\text{adj}}_{\text{P},i,j})^2 = \boldsymbol{o}_{\mathbb{P}}(1),$$

$$\frac{1}{N(N-1)^2}\sum_{i=1}^{N}\sum_{j:j\neq i} D_{i,j}\widehat{r}^{\text{adj}}_{\text{P},i,j}\sum_{j:j\neq i}\boldsymbol{X}^{\top}_{i,j}\widehat{r}^{\text{adj}}_{\text{P},i,j} = \boldsymbol{O}_{\mathbb{P}}(1),$$

$$\frac{1}{N(N-1)^2}\sum_{i=1}^{N}\sum_{j:j\neq i} D_{i,j}\widehat{r}^{\text{adj}}_{\text{P},i,j}\sum_{j:j\neq i} D_{i,j}\boldsymbol{X}^{\top}_{i,j}\widehat{r}^{\text{adj}}_{\text{P},i,j} = \boldsymbol{O}_{\mathbb{P}}(1),$$
$$\frac{1}{N(N-1)^2}\sum_{i=1}^{N}\sum_{j:j\neq i} \boldsymbol{X}_{i,j}\widehat{r}^{\text{adj}}_{\text{P},i,j}\sum_{j:j\neq i} \boldsymbol{X}^{\top}_{i,j}\widehat{r}^{\text{adj}}_{\text{P},i,j} = \boldsymbol{O}_{\mathbb{P}}(1),$$
$$\frac{1}{N(N-1)^2}\sum_{i=1}^{N}\sum_{j:j\neq i} \boldsymbol{X}_{i,j}\widehat{r}^{\text{adj}}_{\text{P},i,j}\sum_{j:j\neq i} D_{i,j}\boldsymbol{X}^{\top}_{i,j}\widehat{r}^{\text{adj}}_{\text{P},i,j} = \boldsymbol{O}_{\mathbb{P}}(1),$$
$$\frac{1}{N(N-1)^2}\sum_{i=1}^{N}\sum_{j:j\neq i} D_{i,j}\boldsymbol{X}_{i,j}\widehat{r}^{\text{adj}}_{\text{P},i,j}\sum_{j:j\neq i} D_{i,j}\boldsymbol{X}^{\top}_{i,j}\widehat{r}^{\text{adj}}_{\text{P},i,j} = \boldsymbol{O}_{\mathbb{P}}(1).$$

Then,

$$\overline{\mathbf{M}}^{\text{adj}}_{\text{P,TW}} = \frac{1}{N(N-1)^2}\mathbf{M}^{\text{adj}}_{\text{P,TW}} = \boldsymbol{O}_{\mathbb{P}}(1).$$

We now analyze the TW variance estimators. Using similar arguments in the proof of the HR variance estimator for $\widehat{\lambda}^{\text{adj}}_{\text{I}}(a, 1-a)$, we have

$$(\mathbf{G}^{\text{adj}}_{\text{P}})^{-1}\overline{\mathbf{M}}^{\text{adj}}_{\text{P,TW}}(\mathbf{G}^{\text{adj}}_{\text{P}})^{-1} - (\mathbf{\Gamma}^{\text{adj}}_{\text{P}})^{-1}\overline{\mathbf{M}}^{\text{adj}}_{\text{P,TW}}(\mathbf{\Gamma}^{\text{adj}}_{\text{P}})^{-1} = \boldsymbol{o}_{\mathbb{P}}(1),$$

where $\mathbf{G}^{\text{adj}}_{\text{P}}$ is defined in (S22) and $\mathbf{\Gamma}^{\text{adj}}_{\text{P}}$ is defined in (S23). Then, by Lemma S22,

$$\begin{aligned}
N\widehat{\text{se}}^2_{\text{TW}}\left\{\widehat{\tau}^{\text{adj}}_{\text{P}}(1)\right\} &= 4\left[(\mathbf{\Gamma}^{\text{adj}}_{\text{P}})^{-1}\overline{\mathbf{M}}^{\text{adj}}_{\text{P,TW}}(\mathbf{\Gamma}^{\text{adj}}_{\text{P}})^{-1}\right]_{(1,1)} + o_{\mathbb{P}}(1)\\
&= \frac{1}{N(N-1)^2}\cdot\frac{1}{\pi_1^2\pi_0^2}\sum_{i=1}^{N}\left(\sum_{j:j\neq i} D_{i,j}\widehat{r}^{\text{adj}}_{\text{P},i,j}\right)^2 + \frac{1}{N(N-1)^2}\cdot\frac{1}{\pi_1^2\pi_0^2}\sum_{j=1}^{N}\left(\sum_{i:i\neq j} D_{i,j}\widehat{r}^{\text{adj}}_{\text{P},i,j}\right)^2 + o_{\mathbb{P}}(1)\\
&= \frac{1}{\pi_1 N}\sum_{i=1}^{N}\overline{r}^{\text{adj}}_{\text{P},i,\cdot}(1,0)^2 + \frac{1}{\pi_0 N}\sum_{i=1}^{N}\overline{r}^{\text{adj}}_{\text{P},i,\cdot}(0,1)^2 + \frac{1}{\pi_0 N}\sum_{j=1}^{N}\overline{r}^{\text{adj}}_{\text{P},\cdot,j}(1,0)^2 + \frac{1}{\pi_1 N}\sum_{j=1}^{N}\overline{r}^{\text{adj}}_{\text{P},\cdot,j}(0,1)^2 + o_{\mathbb{P}}(1).
\end{aligned}$$

Thus, the probability limit of $N\widehat{\text{se}}^2_{\text{TW}}\{\widehat{\tau}^{\text{adj}}_{\text{P}}(1)\}$ is not $V(\overline{r}^{\text{adj}}_{\text{P},i})$ or $V_c(\overline{r}^{\text{adj}}_{\text{P},i})$.

## S5.3 Estimators using per-unit pair averages

### S5.3.1 The HR variance estimators

We prove that the HR variance estimator is not consistent for the variances of estimators using per-unit pair averages. We focus on $\widehat{\lambda}^{\text{adj}}_{\text{A},1}(a, 1-a)$. Recall that the design vector is $\boldsymbol{Z}^{\text{adj}}_{\text{A},i,\cdot} = (A_i, 1-A_i, A_i\overline{\boldsymbol{X}}^{A\top}_{i,\cdot}, (1-A_i)\overline{\boldsymbol{X}}^{A\top}_{i,\cdot})^{\top}$. Stack $\boldsymbol{Z}^{\text{adj}\top}_{\text{A},i,\cdot}$ to create design matrix $\mathbf{Z}^{\text{adj}}_{\text{A},1}$. The HR variance estimator for $\widehat{\lambda}^{\text{adj}}_{\text{A},1}(1,0)$ is

$$\widehat{\text{se}}^2_{\text{HR}}\left\{\widehat{\lambda}^{\text{adj}}_{\text{A},1}(1,0)\right\} = \left[\left(\mathbf{Z}^{\text{adj}\top}_{\text{A},1}\mathbf{Z}^{\text{adj}}_{\text{A},1}\right)^{-1}\mathbf{M}^{\text{adj}}_{\text{A},1,\text{HR}}\left(\mathbf{Z}^{\text{adj}\top}_{\text{A},1}\mathbf{Z}^{\text{adj}}_{\text{A},1}\right)^{-1}\right]_{(1,1)},$$

where the middle matrix

$$\mathbf{M}^{\text{adj}}_{\text{A},1,\text{HR}} = \sum_{i=1}^{N}\boldsymbol{Z}^{\text{adj}}_{\text{A},i,\cdot}\boldsymbol{Z}^{\text{adj}\top}_{\text{A},i,\cdot}(\widehat{r}^{\text{adj}}_{\text{A},1,i,\cdot})^2$$

$$= \begin{pmatrix} \mathrm{M}^{\mathrm{adj}}_{\mathrm{A},1,\mathrm{HR}}[1,1] & 0 & \mathbf{M}^{\mathrm{adj}}_{\mathrm{A},1,\mathrm{HR}}[1,3] & \mathbf{0} \\ * & \mathrm{M}^{\mathrm{adj}}_{\mathrm{A},1,\mathrm{HR}}[2,2] & \mathbf{0} & \mathbf{M}^{\mathrm{adj}}_{\mathrm{A},1,\mathrm{HR}}[2,4] \\ * & * & \mathbf{M}^{\mathrm{adj}}_{\mathrm{A},1,\mathrm{HR}}[3,3] & \mathbf{0} \\ * & * & * & \mathbf{M}^{\mathrm{adj}}_{\mathrm{A},1,\mathrm{HR}}[4,4] \end{pmatrix}.$$

Specifically,

$$\mathrm{M}^{\mathrm{adj}}_{\mathrm{A},1,\mathrm{HR}}[1,1] = \sum_{i=1}^{N} A_i (\widehat{r}^{\mathrm{adj}}_{\mathrm{A},1,i,\cdot})^2, \quad \mathrm{M}^{\mathrm{adj}}_{\mathrm{A},1,\mathrm{HR}}[2,2] = \sum_{i=1}^{N} (1-A_i)(\widehat{r}^{\mathrm{adj}}_{\mathrm{A},1,i,\cdot})^2,$$
$$\mathbf{M}^{\mathrm{adj}}_{\mathrm{A},1,\mathrm{HR}}[1,3] = \sum_{i=1}^{N} A_i \overline{\boldsymbol{X}}^{A\top}_{i,\cdot} (\widehat{r}^{\mathrm{adj}}_{\mathrm{A},1,i,\cdot})^2, \quad \mathbf{M}^{\mathrm{adj}}_{\mathrm{A},1,\mathrm{HR}}[2,4] = \sum_{i=1}^{N} (1-A_i) \overline{\boldsymbol{X}}^{A\top}_{i,\cdot} (\widehat{r}^{\mathrm{adj}}_{\mathrm{A},1,i,\cdot})^2,$$
$$\mathbf{M}^{\mathrm{adj}}_{\mathrm{A},1,\mathrm{HR}}[3,3] = \sum_{i=1}^{N} A_i \overline{\boldsymbol{X}}^{A}_{i,\cdot} \overline{\boldsymbol{X}}^{A\top}_{i,\cdot} (\widehat{r}^{\mathrm{adj}}_{\mathrm{A},1,i,\cdot})^2, \quad \mathbf{M}^{\mathrm{adj}}_{\mathrm{A},1,\mathrm{HR}}[2,4] = \sum_{i=1}^{N} (1-A_i) \overline{\boldsymbol{X}}^{A}_{i,\cdot} \overline{\boldsymbol{X}}^{A\top}_{i,\cdot} (\widehat{r}^{\mathrm{adj}}_{\mathrm{A},1,i,\cdot})^2.$$

**Lemma S24.** *Under Conditions 1, 4, and 5 in the main article, then*

$$\frac{1}{N}\sum_{i=1}^{N} A_i (\widehat{r}^{\mathrm{adj}}_{\mathrm{A},1,i,\cdot})^2 - \frac{\pi_1}{N}\sum_{i=1}^{N} r^{\mathrm{adj}}_{\mathrm{A},1,i,\cdot}(1,0)^2 = o_{\mathbb{P}}(1), \tag{S48}$$
$$\frac{1}{N}\sum_{i=1}^{N} A_i \overline{\boldsymbol{X}}^{A\top}_{i,\cdot} (\widehat{r}^{\mathrm{adj}}_{\mathrm{A},1,i,\cdot})^2 = \boldsymbol{O}_{\mathbb{P}}(1), \tag{S49}$$
$$\frac{1}{N}\sum_{i=1}^{N} A_i \overline{\boldsymbol{X}}^{A}_{i,\cdot} \overline{\boldsymbol{X}}^{A\top}_{i,\cdot} (\widehat{r}^{\mathrm{adj}}_{\mathrm{A},1,i,\cdot})^2 = \boldsymbol{O}_{\mathbb{P}}(1). \tag{S50}$$

*Similar results can be obtained for the* $1 - A_i$ *terms.*

By Lemma S24,

$$\overline{\mathbf{M}}^{\mathrm{adj}}_{\mathrm{A},1,\mathrm{HR}} = \frac{1}{N}\mathbf{M}^{\mathrm{adj}}_{\mathrm{A},1,\mathrm{HR}} = \boldsymbol{O}_{\mathbb{P}}(1).$$

Define

$$\mathbf{G}^{\mathrm{adj}}_{\mathrm{A},1} = \frac{1}{N}\mathbf{Z}^{\mathrm{adj}\top}_{\mathrm{A},1}\mathbf{Z}^{\mathrm{adj}}_{\mathrm{A},1} = \frac{1}{N}\sum_{i=1}^{N} \boldsymbol{Z}^{\mathrm{adj}}_{\mathrm{A},i,\cdot}\boldsymbol{Z}^{\mathrm{adj}\top}_{\mathrm{A},i,\cdot} = \frac{1}{N}\begin{pmatrix} N_1 & 0 & \sum_{i:A_i=1} \overline{\boldsymbol{X}}^{A\top}_{i,\cdot} & \mathbf{0} \\ * & N_0 & \mathbf{0} & \sum_{i:A_i=0} \overline{\boldsymbol{X}}^{A\top}_{i,\cdot} \\ * & * & \sum_{i:A_i=1} \overline{\boldsymbol{X}}^{A}_{i,\cdot}\overline{\boldsymbol{X}}^{A\top}_{i,\cdot} & \mathbf{0} \\ * & * & * & \sum_{i:A_i=0} \overline{\boldsymbol{X}}^{A}_{i,\cdot}\overline{\boldsymbol{X}}^{A\top}_{i,\cdot} \end{pmatrix}, \tag{S51}$$

with its expectation

$$\boldsymbol{\Gamma}^{\mathrm{adj}}_{\mathrm{A},1} = \begin{pmatrix} \pi_1 & 0 & \mathbf{0} & \mathbf{0} \\ * & \pi_0 & \mathbf{0} & \mathbf{0} \\ * & * & \frac{\pi_1}{N}\sum_{i\neq j} \overline{\boldsymbol{X}}_{i,\cdot}\overline{\boldsymbol{X}}^{\top}_{i,\cdot} & \mathbf{0} \\ * & * & * & \frac{\pi_0}{N}\sum_{i\neq j} \overline{\boldsymbol{X}}_{i,\cdot}\overline{\boldsymbol{X}}^{\top}_{i,\cdot} \end{pmatrix}. \tag{S52}$$

We now analyze the HR variance estimators. Using similar arguments in previous proofs, we have

$$(\mathbf{G}^{\text{adj}}_{\text{A},1})^{-1}\overline{\mathbf{M}}^{\text{adj}}_{\text{A},1,\text{HR}}(\mathbf{G}^{\text{adj}}_{\text{A},1})^{-1} - (\mathbf{\Gamma}^{\text{adj}}_{\text{A},1})^{-1}\overline{\mathbf{M}}^{\text{adj}}_{\text{A},1,\text{HR}}(\mathbf{\Gamma}^{\text{adj}}_{\text{A},1})^{-1} = \boldsymbol{o}_{\mathbb{P}}(1).$$

Then, by Lemma S24,

$$\begin{aligned} N\widehat{\text{se}}^2_{\text{HR}}\left\{\widehat{\lambda}^{\text{adj}}_{\text{A},1}(1,0)\right\} &= \left[(\mathbf{\Gamma}^{\text{adj}}_{\text{A},1})^{-1}\overline{\mathbf{M}}^{\text{adj}}_{\text{A},1,\text{HR}}(\mathbf{\Gamma}^{\text{adj}}_{\text{A},1})^{-1}\right]_{(1,1)} + o_{\mathbb{P}}(1) \\ &= \frac{1}{N}\cdot\frac{1}{\pi_1^2}\sum_{i=1}^{N} A_i(\widehat{r}^{\text{adj}}_{\text{A},1,i,\cdot})^2 + o_{\mathbb{P}}(1) = \frac{1}{\pi_1 N}\sum_{i=1}^{N}\overline{r}^{\text{adj}}_{\text{A},1,i,\cdot}(1,0)^2 + o_{\mathbb{P}}(1). \end{aligned}$$

The probability limit of $N\widehat{\text{se}}^2_{\text{HR}}\{\widehat{\lambda}^{\text{adj}}_{\text{A},1}(1,0)\}$ not $V\{\overline{r}^{\text{adj}}_{\text{A},1,i}(1,0)\}$ or $V_c\{\overline{r}^{\text{adj}}_{\text{A},1,i}(1,0)\}$.

### S5.3.2 The TW variance estimators

We show that the TW variance estimators are asymptotically conservative for the leading terms of the marginal variances but omit the covariances. We focus on $\widehat{\lambda}^{\text{adj}}_{\text{A},1}(a,1-a)$. Recall that the other design vector is $\boldsymbol{Z}^{\text{adj}}_{\text{A},\cdot,i} = (1-A_i, A_i, (1-A_i)\overline{\boldsymbol{X}}^{A\top}_{i,\cdot}, A_i\overline{\boldsymbol{X}}^{A\top}_{i,\cdot})^\top$. Stack $\boldsymbol{Z}^{\text{adj}\top}_{\text{A},\cdot,i}$ to create design matrix $\mathbf{Z}^{\text{adj}}_{\text{A},2}$. The TW variance estimator for $\widehat{\lambda}^{\text{adj}}_{\text{A},1}(1,0)$ is

$$\widehat{\text{se}}^2_{\text{TW}}\left\{\widehat{\lambda}^{\text{adj}}_{\text{A},1}(1,0)\right\} = \left[\left(\mathbf{Z}^{\text{adj}\top}_{\text{A},1}\mathbf{Z}^{\text{adj}}_{\text{A},1}\right)^{-1}\mathbf{M}^{\text{adj}}_{\text{A},1,\text{HR}}\left(\mathbf{Z}^{\text{adj}\top}_{\text{A},1}\mathbf{Z}^{\text{adj}}_{\text{A},1}\right)^{-1}\right]_{(1,1)} + \left[\left(\mathbf{Z}^{\text{adj}\top}_{\text{A},2}\mathbf{Z}^{\text{adj}}_{\text{A},2}\right)^{-1}\mathbf{M}^{\text{adj},(1)}_{\text{A},2,\text{HR}}\left(\mathbf{Z}^{\text{adj}\top}_{\text{A},2}\mathbf{Z}^{\text{adj}}_{\text{A},2}\right)^{-1}\right]_{(1,1)},$$

where the middle matrix

$$\begin{aligned} \mathbf{M}^{\text{adj},(1)}_{\text{A},2,\text{HR}} &= \sum_{i=1}^{N}\boldsymbol{Z}^{\text{adj}}_{\text{A},\cdot,i}\boldsymbol{Z}^{\text{adj}\top}_{\text{A},\cdot,i}(\widehat{r}^{\text{adj}}_{\text{A},1,\cdot,i})^2 \\ &= \begin{pmatrix} \text{M}^{\text{adj},(1)}_{\text{A},2,\text{HR}}[1,1] & 0 & \mathbf{M}^{\text{adj},(1)}_{\text{A},2,\text{HR}}[1,3] & \mathbf{0} \\ * & \text{M}^{\text{adj},(1)}_{\text{A},2,\text{HR}}[2,2] & \mathbf{0} & \mathbf{M}^{\text{adj},(1)}_{\text{A},2,\text{HR}}[2,4] \\ * & * & \mathbf{M}^{\text{adj},(1)}_{\text{A},2,\text{HR}}[3,3] & \mathbf{0} \\ * & * & * & \mathbf{M}^{\text{adj},(1)}_{\text{A},2,\text{HR}}[4,4] \end{pmatrix}. \end{aligned}$$

Specifically,

$$\begin{aligned} &\text{M}^{\text{adj},(1)}_{\text{A},2,\text{HR}}[1,1] = \sum_{i=1}^{N}(1-A_i)(\widehat{r}^{\text{adj}}_{\text{A},1,\cdot,i})^2, \quad \text{M}^{\text{adj},(1)}_{\text{A},2,\text{HR}}[2,2] = \sum_{i=1}^{N}A_i(\widehat{r}^{\text{adj}}_{\text{A},1,\cdot,i})^2, \\ &\mathbf{M}^{\text{adj},(1)}_{\text{A},2,\text{HR}}[1,3] = \sum_{i=1}^{N}(1-A_i)\overline{\boldsymbol{X}}^{A\top}_{\cdot,i}(\widehat{r}^{\text{adj}}_{\text{A},1,\cdot,i})^2, \quad \mathbf{M}^{\text{adj},(1)}_{\text{A},2,\text{HR}}[2,4] = \sum_{i=1}^{N}A_i\overline{\boldsymbol{X}}^{A\top}_{\cdot,i}(\widehat{r}^{\text{adj}}_{\text{A},1,\cdot,i})^2, \\ &\mathbf{M}^{\text{adj},(1)}_{\text{A},2,\text{HR}}[3,3] = \sum_{i=1}^{N}(1-A_i)\overline{\boldsymbol{X}}^{A}_{\cdot,i}\overline{\boldsymbol{X}}^{A\top}_{\cdot,i}(\widehat{r}^{\text{adj}}_{\text{A},1,\cdot,i})^2, \quad \mathbf{M}^{\text{adj},(1)}_{\text{A},2,\text{HR}}[2,4] = \sum_{i=1}^{N}A_i\overline{\boldsymbol{X}}^{A}_{\cdot,i}\overline{\boldsymbol{X}}^{A\top}_{\cdot,i}(\widehat{r}^{\text{adj}}_{\text{A},1,\cdot,i})^2. \end{aligned}$$

**Lemma S25.** *Under Conditions 1, 4, and 5 in the main article, then*

$$\frac{1}{N}\sum_{i=1}^{N}(1-A_i)(\widehat{r}^{\text{adj}}_{\text{A},1,\cdot,i})^2 - \frac{\pi_0}{N}\sum_{i=1}^{N}r^{\text{adj}}_{\text{A},1,\cdot,i}(1,0)^2 = o_{\mathbb{P}}(1), \tag{S53}$$

$$\frac{1}{N}\sum_{i=1}^{N}(1-A_i)\overline{\boldsymbol{X}}^{A\top}_{\cdot,i}(\widehat{r}^{\text{adj}}_{\text{A},1,\cdot,i})^2 = \boldsymbol{O}_{\mathbb{P}}(1), \tag{S54}$$

$$\frac{1}{N}\sum_{i=1}^{N}(1-A_i)\overline{\boldsymbol{X}}^{A}_{\cdot,i}\overline{\boldsymbol{X}}^{A\top}_{\cdot,i}(\widehat{r}^{\text{adj}}_{\text{A},1,\cdot,i})^2 = \boldsymbol{O}_{\mathbb{P}}(1). \tag{S55}$$

*Similar results can be obtained for the $A_i$ terms.*

(S53) is implied by (S48). (S54) is implied by (S49). (S55) is implied by (S50). Detailed proofs are omitted. By Lemma S25,

$$\overline{\mathbf{M}}^{\text{adj},(1)}_{\text{A},2,\text{HR}} = \frac{1}{N}\mathbf{M}^{\text{adj},(1)}_{\text{A},2,\text{HR}} = \boldsymbol{O}_{\mathbb{P}}(1).$$

Define

$$\mathbf{G}^{\text{adj}}_{\text{A},2} = \frac{1}{N}\mathbf{Z}^{\text{adj}\top}_{\text{A},2}\mathbf{Z}^{\text{adj}}_{\text{A},2} = \frac{1}{N}\sum_{i=1}^{N}\boldsymbol{Z}^{\text{adj}}_{\text{A},\cdot,i}\boldsymbol{Z}^{\text{adj}\top}_{\text{A},\cdot,i} = \frac{1}{N}\begin{pmatrix} N_0 & 0 & \sum_{i:A_i=0}\overline{\boldsymbol{X}}^{A\top}_{\cdot,i} & \mathbf{0} \\ * & N_1 & \mathbf{0} & \sum_{i:A_i=1}\overline{\boldsymbol{X}}^{A\top}_{\cdot,i} \\ * & * & \sum_{i:A_i=0}\overline{\boldsymbol{X}}^{A}_{\cdot,i}\overline{\boldsymbol{X}}^{A\top}_{\cdot,i} & \mathbf{0} \\ * & * & * & \sum_{i:A_i=1}\overline{\boldsymbol{X}}^{A}_{\cdot,i}\overline{\boldsymbol{X}}^{A\top}_{\cdot,i} \end{pmatrix}, \tag{S56}$$

with its expectation

$$\boldsymbol{\Gamma}^{\text{adj}}_{\text{A},2} = \begin{pmatrix} \pi_0 & 0 & \mathbf{0} & \mathbf{0} \\ * & \pi_1 & \mathbf{0} & \mathbf{0} \\ * & * & \frac{\pi_0}{N}\sum_{i\neq j}\overline{\boldsymbol{X}}_{\cdot,i}\overline{\boldsymbol{X}}^{\top}_{\cdot,i} & \mathbf{0} \\ * & * & * & \frac{\pi_1}{N}\sum_{i\neq j}\overline{\boldsymbol{X}}_{\cdot,i}\overline{\boldsymbol{X}}^{\top}_{\cdot,i} \end{pmatrix}. \tag{S57}$$

We now analyze the TW variance estimators. Using similar arguments in previous proofs, we have

$$(\mathbf{G}^{\text{adj}}_{\text{A},2})^{-1}\overline{\mathbf{M}}^{\text{adj},(1)}_{\text{A},2,\text{HR}}(\mathbf{G}^{\text{adj}}_{\text{A},2})^{-1} - (\boldsymbol{\Gamma}^{\text{adj}}_{\text{A},2})^{-1}\overline{\mathbf{M}}^{\text{adj},(1)}_{\text{A},2,\text{HR}}(\boldsymbol{\Gamma}^{\text{adj}}_{\text{A},2})^{-1} = \boldsymbol{o}_{\mathbb{P}}(1).$$

Then, by Lemma S25,

$$\begin{aligned} N\widehat{\text{se}}^2_{\text{TW}}\left\{\widehat{\lambda}^{\text{adj}}_{\text{A},1}(1,0)\right\} &= \left[(\boldsymbol{\Gamma}^{\text{adj}}_{\text{A},1})^{-1}\overline{\mathbf{M}}^{\text{adj}}_{\text{A},1,\text{HR}}(\boldsymbol{\Gamma}^{\text{adj}}_{\text{A},1})^{-1}\right]_{(1,1)} + \left[(\boldsymbol{\Gamma}^{\text{adj}}_{\text{A},2})^{-1}\overline{\mathbf{M}}^{\text{adj},(1)}_{\text{A},2,\text{HR}}(\boldsymbol{\Gamma}^{\text{adj}}_{\text{A},2})^{-1}\right]_{(1,1)} + o_{\mathbb{P}}(1) \\ &= \frac{1}{N}\cdot\frac{1}{\pi_1^2}\sum_{i=1}^{N}A_i(\widehat{r}^{\text{adj}}_{\text{A},1,i,\cdot})^2 + \frac{1}{N}\cdot\frac{1}{\pi_0^2}\sum_{i=1}^{N}(1-A_i)(\widehat{r}^{\text{adj}}_{\text{A},1,\cdot,i})^2 + o_{\mathbb{P}}(1) \\ &= \frac{1}{\pi_1 N}\sum_{i=1}^{N}\overline{r}^{\text{adj}}_{\text{A},1,i,\cdot}(1,0)^2 + \frac{1}{\pi_0 N}\sum_{i=1}^{N}\overline{r}^{\text{adj}}_{\text{A},1,\cdot,i}(1,0)^2 + o_{\mathbb{P}}(1). \end{aligned}$$

The probability limit of $N\widehat{\text{se}}^2_{\text{TW}}\{\widehat{\lambda}^{\text{adj}}_{\text{A},1}(1,0)\}$ is $V_c\{\overline{r}^{\text{adj}}_{\text{A},1,i}(1,0)\}$. However,

$$\begin{aligned} \left[(\boldsymbol{\Gamma}^{\text{adj}}_{\text{A},1})^{-1}\overline{\mathbf{M}}^{\text{adj}}_{\text{A},1,\text{HR}}(\boldsymbol{\Gamma}^{\text{adj}}_{\text{A},1})^{-1}\right]_{(1,2)} &= \left[(\boldsymbol{\Gamma}^{\text{adj}}_{\text{A},1})^{-1}\overline{\mathbf{M}}^{\text{adj}}_{\text{A},1,\text{HR}}(\boldsymbol{\Gamma}^{\text{adj}}_{\text{A},1})^{-1}\right]_{(2,1)} = o_{\mathbb{P}}(1), \\ \left[(\boldsymbol{\Gamma}^{\text{adj}}_{\text{A},2})^{-1}\overline{\mathbf{M}}^{\text{adj},(1)}_{\text{A},2,\text{HR}}(\boldsymbol{\Gamma}^{\text{adj}}_{\text{A},2})^{-1}\right]_{(1,2)} &= \left[(\boldsymbol{\Gamma}^{\text{adj}}_{\text{A},2})^{-1}\overline{\mathbf{M}}^{\text{adj},(1)}_{\text{A},2,\text{HR}}(\boldsymbol{\Gamma}^{\text{adj}}_{\text{A},2})^{-1}\right]_{(2,1)} = o_{\mathbb{P}}(1), \end{aligned}$$

implying that the TW estimator omits the covariance between $\widehat{\lambda}^{\text{adj}}_{\text{A},1}(1,0)$ and $\widehat{\lambda}^{\text{adj}}_{\text{A},1}(0,1)$.

#### S5.3.3 The CTW variance estimators

We now prove that the CTW variance estimators are asymptotically conservative for the leading terms of the marginal variances and consistent for sums of estimable components in the leading terms of the covariances. The CTW variance estimator for $\widehat{\lambda}_{\mathrm{A},1}^{\mathrm{adj}}(1,0)$ is

$$
\begin{aligned}
\widehat{\mathrm{se}}^2_{\mathrm{CTW}}\left\{\widehat{\lambda}_{\mathrm{A},1}^{\mathrm{adj}}(1,0)\right\} = {} & \left[\left(\mathbf{Z}_{\mathrm{A},1}^{\mathrm{adj}\top}\mathbf{Z}_{\mathrm{A},1}^{\mathrm{adj}}\right)^{-1}\mathbf{M}_{\mathrm{A},1,\mathrm{HR}}^{\mathrm{adj}}\left(\mathbf{Z}_{\mathrm{A},1}^{\mathrm{adj}\top}\mathbf{Z}_{\mathrm{A},1}^{\mathrm{adj}}\right)^{-1}\right]_{(1,1)} + \left[\left(\mathbf{Z}_{\mathrm{A},2}^{\mathrm{adj}\top}\mathbf{Z}_{\mathrm{A},2}^{\mathrm{adj}}\right)^{-1}\mathbf{M}_{\mathrm{A},2,\mathrm{HR}}^{\mathrm{adj},(1)}\left(\mathbf{Z}_{\mathrm{A},2}^{\mathrm{adj}\top}\mathbf{Z}_{\mathrm{A},2}^{\mathrm{adj}}\right)^{-1}\right]_{(1,1)} \\
& + \left[\left(\mathbf{Z}_{\mathrm{A},1}^{\mathrm{adj}\top}\mathbf{Z}_{\mathrm{A},1}^{\mathrm{adj}}\right)^{-1}\left(\sum_{i=1}^N \boldsymbol{Z}_{\mathrm{A},i,\cdot}^{\mathrm{adj}}\boldsymbol{Z}_{\mathrm{A},\cdot,i}^{\mathrm{adj}\top}\widehat{r}_{\mathrm{A},1,i,\cdot}^{\mathrm{adj}}\widehat{r}_{\mathrm{A},1,\cdot,i}^{\mathrm{adj}}\right)\left(\mathbf{Z}_{\mathrm{A},2}^{\mathrm{adj}\top}\mathbf{Z}_{\mathrm{A},2}^{\mathrm{adj}}\right)^{-1}\right]_{(1,1)} \\
& + \left[\left(\mathbf{Z}_{\mathrm{A},2}^{\mathrm{adj}\top}\mathbf{Z}_{\mathrm{A},2}^{\mathrm{adj}}\right)^{-1}\left(\sum_{i=1}^N \boldsymbol{Z}_{\mathrm{A},\cdot,i}^{\mathrm{adj}}\boldsymbol{Z}_{\mathrm{A},i,\cdot}^{\mathrm{adj}\top}\widehat{r}_{\mathrm{A},1,\cdot,i}^{\mathrm{adj}}\widehat{r}_{\mathrm{A},1,i,\cdot}^{\mathrm{adj}}\right)\left(\mathbf{Z}_{\mathrm{A},1}^{\mathrm{adj}\top}\mathbf{Z}_{\mathrm{A},1}^{\mathrm{adj}}\right)^{-1}\right]_{(1,1)}.
\end{aligned}
$$

Specifically,

$$
\begin{aligned}
&\sum_{i=1}^N \boldsymbol{Z}_{\mathrm{A},i,\cdot}^{\mathrm{adj}}\boldsymbol{Z}_{\mathrm{A},\cdot,i}^{\mathrm{adj}\top}\widehat{r}_{\mathrm{A},1,i,\cdot}^{\mathrm{adj}}\widehat{r}_{\mathrm{A},1,\cdot,i}^{\mathrm{adj}} \\
&= \sum_{i=1}^N \begin{pmatrix}
0 & A_i\widehat{r}_{\mathrm{A},1,i,\cdot}^{\mathrm{adj}}\widehat{r}_{\mathrm{A},1,\cdot,i}^{\mathrm{adj}} & \mathbf{0} & A_i\widehat{r}_{\mathrm{A},1,i,\cdot}^{\mathrm{adj}}\overline{\boldsymbol{X}}_{\cdot,i}^{A\top}\widehat{r}_{\mathrm{A},1,\cdot,i}^{\mathrm{adj}} \\
(1-A_i)\widehat{r}_{\mathrm{A},1,i,\cdot}^{\mathrm{adj}}\widehat{r}_{\mathrm{A},1,\cdot,i}^{\mathrm{adj}} & 0 & (1-A_i)\widehat{r}_{\mathrm{A},1,i,\cdot}^{\mathrm{adj}}\overline{\boldsymbol{X}}_{\cdot,i}^{A\top}\widehat{r}_{\mathrm{A},1,\cdot,i}^{\mathrm{adj}} & \mathbf{0} \\
\mathbf{0} & A_i\overline{\boldsymbol{X}}_{\cdot,i}^{A}\widehat{r}_{\mathrm{A},1,i,\cdot}^{\mathrm{adj}}\widehat{r}_{\mathrm{A},1,\cdot,i}^{\mathrm{adj}} & \mathbf{0} & A_i\overline{\boldsymbol{X}}_{i,\cdot}^{A}\overline{\boldsymbol{X}}_{\cdot,i}^{A\top}\widehat{r}_{\mathrm{A},1,i,\cdot}^{\mathrm{adj}}\widehat{r}_{\mathrm{A},1,\cdot,i}^{\mathrm{adj}} \\
(1-A_i)\overline{\boldsymbol{X}}_{\cdot,i}^{A}\widehat{r}_{\mathrm{A},1,i,\cdot}^{\mathrm{adj}}\widehat{r}_{\mathrm{A},1,\cdot,i}^{\mathrm{adj}} & \mathbf{0} & (1-A_i)\overline{\boldsymbol{X}}_{i,\cdot}^{A}\overline{\boldsymbol{X}}_{\cdot,i}^{A\top}\widehat{r}_{\mathrm{A},1,i,\cdot}^{\mathrm{adj}}\widehat{r}_{\mathrm{A},1,\cdot,i}^{\mathrm{adj}} & \mathbf{0}
\end{pmatrix},
\end{aligned}
$$

and

$$
\sum_{i=1}^N \boldsymbol{Z}_{\mathrm{A},\cdot,i}^{\mathrm{adj}}\boldsymbol{Z}_{\mathrm{A},i,\cdot}^{\mathrm{adj}\top}\widehat{r}_{\mathrm{A},1,\cdot,i}^{\mathrm{adj}}\widehat{r}_{\mathrm{A},1,i,\cdot}^{\mathrm{adj}} = \left(\sum_{i=1}^N \boldsymbol{Z}_{\mathrm{A},i,\cdot}^{\mathrm{adj}}\boldsymbol{Z}_{\mathrm{A},\cdot,i}^{\mathrm{adj}\top}\widehat{r}_{\mathrm{A},1,i,\cdot}^{\mathrm{adj}}\widehat{r}_{\mathrm{A},1,\cdot,i}^{\mathrm{adj}}\right)^\top.
$$

Thus, we have

$$
\widehat{\mathrm{se}}^2_{\mathrm{CTW}}\left\{\widehat{\lambda}_{\mathrm{A},1}^{\mathrm{adj}}(1,0)\right\} = \widehat{\mathrm{se}}^2_{\mathrm{TW}}\left\{\widehat{\lambda}_{\mathrm{A},1}^{\mathrm{adj}}(1,0)\right\} = V_c\{\overline{r}_{\mathrm{A},1,i}(1,0)\}.
$$

For the covariances, we have the following lemma.

**Lemma S26.** *Under Conditions 1, 4, and 5 in the main article, then*

$$
\frac{1}{N}\sum_{i=1}^N A_i\widehat{r}_{\mathrm{A},1,i,\cdot}\widehat{r}_{\mathrm{A},1,\cdot,i}^{\mathrm{adj}} - \frac{\pi_1}{N}\sum_{i=1}^N r_{\mathrm{A},1,i,\cdot}^{\mathrm{adj}}(1,0)r_{\mathrm{A},1,\cdot,i}^{\mathrm{adj}}(0,1) = o_{\mathbb{P}}(1), \tag{S58}
$$

$$
\frac{1}{N}\sum_{i=1}^N A_i\widehat{r}_{\mathrm{A},1,i,\cdot}^{\mathrm{adj}}\overline{\boldsymbol{X}}_{\cdot,i}^{A\top}\widehat{r}_{\mathrm{A},1,\cdot,i}^{\mathrm{adj}} = \boldsymbol{O}_{\mathbb{P}}(1), \tag{S59}
$$

$$
\frac{1}{N}\sum_{i=1}^N A_i\overline{\boldsymbol{X}}_{i,\cdot}^{A}\overline{\boldsymbol{X}}_{\cdot,i}^{A\top}\widehat{r}_{\mathrm{A},1,i,\cdot}^{\mathrm{adj}}\widehat{r}_{\mathrm{A},1,\cdot,i}^{\mathrm{adj}} = \boldsymbol{O}_{\mathbb{P}}(1). \tag{S60}
$$

*Similar results can be obtained for the $1-A_i$ terms.*

(S58) is implied by (S53). (S59) is implied by (S54). (S60) is implied by (S55). Detailed proofs are omitted. By Lemma S26,

$$
\frac{1}{N}\sum_{i=1}^N \boldsymbol{Z}_{\mathrm{A},i,\cdot}^{\mathrm{adj}}\boldsymbol{Z}_{\mathrm{A},\cdot,i}^{\mathrm{adj}\top}\widehat{r}_{\mathrm{A},1,i,\cdot}^{\mathrm{adj}}\widehat{r}_{\mathrm{A},1,\cdot,i}^{\mathrm{adj}} = \boldsymbol{O}_{\mathbb{P}}(1).
$$

Using similar arguments in previous proofs, we have

$$(\mathbf{G}^{\mathrm{adj}}_{\mathrm{A},1})^{-1}\left(\frac{1}{N}\sum_{i=1}^{N}\boldsymbol{Z}^{\mathrm{adj}}_{\mathrm{A},i,\cdot}\boldsymbol{Z}^{\mathrm{adj}\top}_{\mathrm{A},\cdot,i}\widehat{r}^{\mathrm{adj}}_{\mathrm{A},1,i,\cdot}\widehat{r}^{\mathrm{adj}}_{\mathrm{A},1,\cdot,i}\right)(\mathbf{G}^{\mathrm{adj}}_{\mathrm{A},2})^{-1}$$
$$-(\mathbf{\Gamma}^{\mathrm{adj}}_{\mathrm{A},1})^{-1}\left(\frac{1}{N}\sum_{i=1}^{N}\boldsymbol{Z}^{\mathrm{adj}}_{\mathrm{A},i,\cdot}\boldsymbol{Z}^{\mathrm{adj}\top}_{\mathrm{A},\cdot,i}\widehat{r}^{\mathrm{adj}}_{\mathrm{A},1,i,\cdot}\widehat{r}^{\mathrm{adj}}_{\mathrm{A},1,\cdot,i}\right)(\mathbf{\Gamma}^{\mathrm{adj}}_{\mathrm{A},2})^{-1}=\boldsymbol{o}_{\mathbb{P}}(1),$$
$$(\mathbf{G}^{\mathrm{adj}}_{\mathrm{A},2})^{-1}\left(\frac{1}{N}\sum_{i=1}^{N}\boldsymbol{Z}^{\mathrm{adj}}_{\mathrm{A},\cdot,i}\boldsymbol{Z}^{\mathrm{adj}\top}_{\mathrm{A},i,\cdot}\widehat{r}^{\mathrm{adj}}_{\mathrm{A},1,\cdot,i}\widehat{r}^{\mathrm{adj}}_{\mathrm{A},1,i,\cdot}\right)(\mathbf{G}^{\mathrm{adj}}_{\mathrm{A},1})^{-1}$$
$$-(\mathbf{\Gamma}^{\mathrm{adj}}_{\mathrm{A},2})^{-1}\left(\frac{1}{N}\sum_{i=1}^{N}\boldsymbol{Z}^{\mathrm{adj}}_{\mathrm{A},\cdot,i}\boldsymbol{Z}^{\mathrm{adj}\top}_{\mathrm{A},i,\cdot}\widehat{r}^{\mathrm{adj}}_{\mathrm{A},1,\cdot,i}\widehat{r}^{\mathrm{adj}}_{\mathrm{A},1,i,\cdot}\right)(\mathbf{\Gamma}^{\mathrm{adj}}_{\mathrm{A},1})^{-1}=\boldsymbol{o}_{\mathbb{P}}(1).$$

where $\mathbf{G}^{\mathrm{adj}}_{\mathrm{A},1}$ is defined in (S51), $\mathbf{\Gamma}^{\mathrm{adj}}_{\mathrm{A},1}$ is defined in (S52), $\mathbf{G}^{\mathrm{adj}}_{\mathrm{A},2}$ is defined in (S56), and $\mathbf{\Gamma}^{\mathrm{adj}}_{\mathrm{A},2}$ is defined in (S57). Then, by Lemma S26,

$$N\widehat{\mathbb{C}\mathrm{ov}}_{\mathrm{CTW}}\left\{\widehat{\lambda}^{\mathrm{adj}}_{\mathrm{A},1}(1,0),\widehat{\lambda}^{\mathrm{adj}}_{\mathrm{A},1}(0,1)\right\}=\left[(\mathbf{\Gamma}^{\mathrm{adj}}_{\mathrm{A},1})^{-1}\left(\frac{1}{N}\sum_{i=1}^{N}\boldsymbol{Z}^{\mathrm{adj}}_{\mathrm{A},i,\cdot}\boldsymbol{Z}^{\mathrm{adj}\top}_{\mathrm{A},\cdot,i}\widehat{r}^{\mathrm{adj}}_{\mathrm{A},1,i,\cdot}\widehat{r}^{\mathrm{adj}}_{\mathrm{A},1,\cdot,i}\right)(\mathbf{\Gamma}^{\mathrm{adj}}_{\mathrm{A},2})^{-1}\right]_{(1,2)}$$
$$+\left[(\mathbf{\Gamma}^{\mathrm{adj}}_{\mathrm{A},2})^{-1}\left(\frac{1}{N}\sum_{i=1}^{N}\boldsymbol{Z}^{\mathrm{adj}}_{\mathrm{A},\cdot,i}\boldsymbol{Z}^{\mathrm{adj}\top}_{\mathrm{A},i,\cdot}\widehat{r}^{\mathrm{adj}}_{\mathrm{A},1,\cdot,i}\widehat{r}^{\mathrm{adj}}_{\mathrm{A},1,i,\cdot}\right)(\mathbf{\Gamma}^{\mathrm{adj}}_{\mathrm{A},1})^{-1}\right]_{(1,2)}+o_{\mathbb{P}}(1)$$
$$=\frac{1}{N}\cdot\frac{1}{\pi_1^2}\sum_{i=1}^{N}A_i\widehat{r}^{\mathrm{adj}}_{\mathrm{A},1,i,\cdot}\widehat{r}^{\mathrm{adj}}_{\mathrm{A},1,\cdot,i}+\frac{1}{N}\cdot\frac{1}{\pi_0^2}\sum_{i=1}^{N}(1-A_i)\widehat{r}^{\mathrm{adj}}_{\mathrm{A},1,\cdot,i}\widehat{r}^{\mathrm{adj}}_{\mathrm{A},1,i,\cdot}+o_{\mathbb{P}}(1)$$
$$=\frac{1}{\pi_1 N}\sum_{i=1}^{N}\overline{r}^{\mathrm{adj}}_{\mathrm{A},1,i,\cdot}(1,0)\overline{r}^{\mathrm{adj}}_{\mathrm{A},1,\cdot,i}(0,1)+\frac{1}{\pi_0 N}\sum_{i=1}^{N}\overline{r}^{\mathrm{adj}}_{\mathrm{A},1,i,\cdot}(0,1)\overline{r}^{\mathrm{adj}}_{\mathrm{A},1,\cdot,i}(1,0)+o_{\mathbb{P}}(1).$$

The probability limit of $N\widehat{\mathbb{C}\mathrm{ov}}_{\mathrm{CTW}}\{\widehat{\lambda}^{\mathrm{adj}}_{\mathrm{A},1}(1,0),\widehat{\lambda}^{\mathrm{adj}}_{\mathrm{A},1}(0,1)\}$ is the sum of estimable components in $CV(\overline{r}^{\mathrm{adj}}_{\mathrm{A},1,i})$.

# S6 Proof of the Lemmas

## S6.1 Lemma S1

Let $H_{i,j}=A_i(1-A_j)$ and

$$\mu_{H,N}=\mathbb{E}(H_{i,j})=\frac{N_1(N-N_1)}{N(N-1)}.$$

Note that $\mu_{H,N}=\pi_1\pi_0+O(N^{-1})$, so $\mu_{H,N}=O(1)$. Let $\widetilde{H}_{i,j}=H_{i,j}-\mu_{H,N}$. Then

$$\overline{b}-\mathbb{E}(\overline{b})=\frac{1}{N(N-1)}\sum_{i\neq j}b_{i,j}\widetilde{H}_{i,j}.$$

Thus

$$\mathbb{V}\mathrm{ar}(\overline{b})=\frac{1}{N^2(N-1)^2}\sum_{i\neq j}\sum_{k\neq l}b_{i,j}b_{k,l}\mathbb{C}\mathrm{ov}(H_{i,j},H_{k,l}).$$

For $|\{i,j\}\cap\{k,l\}|=2$, if $(i,j)=(k,l)$,

$$\mathbb{C}\mathrm{ov}(H_{i,j},H_{i,j})=\mathbb{V}\mathrm{ar}(H_{i,j})=\mu_{H,N}(1-\mu_{H,N})=O(1),$$

and the number of such terms is $N(N-1)$, with the contribution to variance as

$$V_{2a}=\frac{1}{N^2(N-1)^2}\sum_{i\neq j}b_{i,j}^2\cdot O(1).$$

Given $\sum_{i\neq j}b_{i,j}^2=O(N^2)$, we have

$$|V_{2a}|\leq O\left(\frac{1}{N^4}\right)\cdot O(N^2)=O\left(\frac{1}{N^2}\right).$$

If $(i,j)=(l,k)$, then $H_{i,j}H_{j,i}=0$. Therefore,

$$\mathbb{C}\mathrm{ov}(H_{i,j},H_{j,i})=\mathbb{E}(H_{i,j}H_{j,i})-\mu_{H,N}^2=-\mu_{H,N}^2=O(1),$$

and the number of such terms is $N(N-1)$, with the contribution to variance as

$$V_{2b}=\frac{1}{N^4}\sum_{i\neq j}b_{i,j}b_{j,i}\cdot(-\mu_{H,N}^2).$$

By the Cauchy-Schwarz inequality,

$$\left|\sum_{i\neq j}b_{i,j}b_{j,i}\right|\leq\sum_{i\neq j}\frac{b_{i,j}^2+b_{j,i}^2}{2}=O(N^2).$$

Therefore, $|V_{2b}|=O(N^{-2})$. Thus

$$V_2=V_{2a}+V_{2b}=O\left(\frac{1}{N^2}\right).$$

For $|\{i,j\}\cap\{k,l\}|=1$, there are four subcases up to symmetry: (i) $i=k,j\neq l,j\neq i,l\neq i$, (ii) $i=l,j\neq k,j\neq i,k\neq i$, (iii) $j=k,i\neq l,i\neq j,l\neq j$, and (iv) $j=l,i\neq k,i\neq j,k\neq j$. We show that, for each, the variance contribution is $O(N^{-1})$. If $i=k,j\neq l$, all distinct,

$$\begin{aligned}\mathbb{E}(H_{i,j}H_{i,l})&=\mathbb{E}\{A_i(1-A_j)(1-A_l)\}=\mathbb{P}(A_i=1,A_j=0,A_l=0)\\&=\frac{\binom{N-3}{N_1-1}}{\binom{N}{N_1}}=\frac{N_1(N-N_1)(N-N_1-1)}{N(N-1)(N-2)},\end{aligned}$$

under fixed $N_1$. Then

$$\mathbb{E}(H_{i,j}H_{i,l})=\frac{\pi_1\pi_0^2N^3+O(N^2)}{N^3+O(N^2)}=\pi_1\pi_0^2+O\left(\frac{1}{N}\right).$$

Also, since $\mathbb{E}(H_{i,j}) = \pi_1\pi_0 + O(N^{-1})$, we have

$$\mathbb{C}\text{ov}(H_{i,j}, H_{i,l}) = \pi_1\pi_0^2 - (\pi_1\pi_0)^2 + O\left(\frac{1}{N}\right) = \pi_1\pi_0^2\pi_0 + O\left(\frac{1}{N}\right) = pq^3 + O\left(\frac{1}{N}\right) = O(1).$$

The number of such index tuples $(i, j, l)$ is $N(N-1)(N-2)$, with the contribution to variance

$$\frac{1}{N^4}\sum_{i,j,l \text{ distinct}} b_{i,j}b_{i,l}\mathbb{C}\text{ov}(H_{i,j}, H_{i,l}).$$

Then,

$$\left|\sum_{i,j,l \text{ distinct}} b_{i,j}b_{i,l}\mathbb{C}\text{ov}(H_{i,j}, H_{i,l})\right| \le O(1)\sum_i \sum_{j:j\neq i}\sum_{l:l\neq i, l\neq j}|b_{i,j}b_{i,l}|,$$

where, for fixed $i$,

$$\sum_{j:j\neq i}\sum_{l:l\neq i,l\neq j}|b_{i,j}b_{i,l}| \le \left(\sum_{j:j\neq i}|b_{i,j}|\right)^2.$$

By Cauchy–Schwarz inequality,

$$\sum_{j:j\neq i}|b_{i,j}| \le \left\{(N-1)\sum_{j:j\neq i} b_{i,j}^2\right\}^{1/2}.$$

Since $\sum_i \sum_{j:j\neq i} b_{ij}^2 = \sum_{i\neq j} b_{i,j}^2 = O(N^2)$, we have

$$\sum_i \left(\sum_{j:j\neq i}|b_{i,j}|\right)^2 \le \sum_i \left(N\sum_{j:j\neq i} b_{i,j}^2\right) = N\sum_{i\neq j} b_{i,j}^2 = N\cdot O(N^2) = O(N^3).$$

Therefore,

$$\left|\sum_{i,j,l \text{ distinct}} b_{i,j}b_{i,l}\mathbb{C}\text{ov}(H_{i,j}, H_{i,l})\right| = O(N^3).$$

The other three subcases are similar: each yields covariance $O(1)$ and the sum over indices is bounded by $O(N^3)$ via the same Cauchy–Schwarz argument (possibly with roles of $i, j$ swapped, but the bound is symmetric). Thus, the total contribution from this case is:

$$V_1 = O\left(\frac{1}{N^4}\right)O(N^3) = O\left(\frac{1}{N}\right).$$

For $|\{i,j\}\cap\{k,l\}| = 0$, i.e., $i, j, k, l$ all distinct, we have

$$\mathbb{E}(H_{i,j}H_{k,l}) = \frac{\binom{N-4}{N_1-2}}{\binom{N}{N_1}} = \frac{N_1(N_1-1)(N-N_1)(N-N_1-1)}{N(N-1)(N-2)(N-3)} = (\pi_1\pi_0)^2 + O\left(\frac{1}{N}\right).$$

Therefore,

$$\mathbb{C}\text{ov}(H_{i,j}, H_{k,l}) = O\left(\frac{1}{N}\right),$$

and the number of such terms is $O(N^4)$. Then,

$$\left|\sum_{i\neq j\neq k\neq l} b_{i,j}b_{k,l}\mathbb{C}\text{ov}(H_{i,j}, H_{k,l})\right| \leq O\left(\frac{1}{N}\right) \sum_{i\neq j\neq k\neq l} |b_{i,j}b_{k,l}|,$$

where

$$\sum_{i\neq j\neq k\neq l} |b_{i,j}b_{k,l}| \leq \left(\sum_{i\neq j} |b_{i,j}|\right)^2,$$

with

$$\sum_{i\neq j} |b_{i,j}| \leq \left\{N(N-1)\sum_{i\neq j} b_{i,j}^2\right\}^{1/2} = \left\{O(N^2)\cdot O(N^2)\right\}^{1/2} = O(N^2).$$

Therefore, the variance contribution from this case is

$$V_0 = O\left(\frac{1}{N^4}\right)\cdot O(N^4)\cdot O\left(\frac{1}{N}\right) = O\left(\frac{1}{N}\right).$$

For the final bound, we have

$$\mathbb{V}\text{ar}(\bar{b}) = V_2 + V_1 + V_0 = O\left(\frac{1}{N^2}\right) + O\left(\frac{1}{N}\right) + O\left(\frac{1}{N}\right) = O\left(\frac{1}{N}\right).$$

This bound is tight in the worst case, over $b_{i,j}$ satisfying the given condition.

## S6.2 Lemma S5

By the Cauchy-Schwarz inequality,

$$\sum_{i\neq j} b_{i,j}^2 \leq \left\{N(N-1)\sum_{i\neq j} b_{i,j}^4\right\}^{1/2} \leq \left\{\sum_{i\neq j} b_{i,j}^4\right\}^{1/2} O(N) = o(N^{3/2})O(N) = o(N^{5/2}).$$

Similar to the proof of Lemma S1, the variance can be analyzed by the size of the overlap between $\{i,j\}$ and $\{k,l\}$. Following the same arguments, if $|\{i,j\}\cap\{k,l\}| = 2$ and $(i,j) = (k,l)$, the variance contribution is

$$V_{2a} = \frac{1}{N^2(N-1)^2}\sum_{i\neq j} b_{i,j}^4 \cdot O(1) = o\left(\frac{N^3}{N^4}\right) = o\left(\frac{1}{N}\right).$$

If $(i,j) = (l,k)$, the contribution is

$$V_{2b} = \frac{1}{N^2(N-1)^2}\sum_{i\neq j} b_{i,j}^2 b_{j,i}^2 O(1) \leq \frac{1}{N^2(N-1)^2}\sum_{i\neq j} \frac{b_{i,j}^4 + b_{j,i}^4}{2} O(1) = o\left(\frac{N^3}{N^4}\right) = o\left(\frac{1}{N}\right).$$

For $|\{i,j\}\cap\{k,l\}|=1$, if $i=k, j\neq l$, all distinct. We have the contribution magnitude as

$$\frac{1}{N^4}\sum_{i,j,l \text{ distinct}} b_{i,j}^2 b_{i,l}^2 O(1) = \frac{1}{N^4}\sum_{i}\sum_{j\neq i}\sum_{l\neq i, l\neq j} b_{i,j}^2 b_{i,l}^2 O(1) \leq \frac{1}{N^4}\sum_{i}\left(\sum_{j\neq i} b_{i,j}^2\right)^2 O(1)$$
$$\leq \frac{1}{N^4}\sum_{i}(N-1)\sum_{j\neq i} b_{i,j}^4 O(1) \leq \frac{1}{N}\cdot\frac{1}{N(N-1)}\sum_{i\neq j} b_{i,j}^4 O(1) = O\left(\frac{1}{N}\right)o(N)O(1) = o(1).$$

The other three $|\{i,j\}\cap\{k,l\}|=1$ subcases are symmetric. Thus, the total contribution is $V_1 = o(1)$. For $|\{i,j\}\cap\{k,l\}|=0$. We have the contribution

$$V_0 \leq \frac{1}{N^5}\sum_{i\neq j\neq k\neq l} b_{i,j}^2 b_{k,l}^2 O(1) \leq \frac{1}{N^5}\left(\sum_{i\neq j} b_{i,j}^2\right)^2 O(1) \leq O\left(\frac{1}{N^5}\right)o(N^5)O(1) = o(1).$$

The statement is proved.

## S6.3 Lemma S6

By Jensen's inequality,

$$\overline{b}_{i,\cdot}^4 \leq \frac{1}{N-1}\sum_{k:k\neq i} b_{i,k}^4,$$

so

$$\frac{1}{N}\sum_{i=1}^N \frac{1}{N-1}\sum_{k:k\neq i} b_{i,k}^4 \geq \frac{1}{N}\sum_{i=1}^N \overline{b}_{i,\cdot}^4 = O(1),$$

Similarly,

$$\frac{1}{N}\sum_{i=1}^N \frac{1}{N-1}\sum_{k:k\neq i} c_{i,k}^4 \geq \frac{1}{N}\sum_{i=1}^N \overline{c}_{i,\cdot}^4 = O(1).$$

Let $\delta_i^b = \overline{b}_{i,\cdot}^A - \overline{b}_{i,\cdot}$ and $\delta_i^c = \overline{c}_{i,\cdot}^A - \overline{c}_{i,\cdot}$. By Rosenthal's inequality for sampling without replacement,

$$\mathbb{E}\left\{(\delta_i^b)^4\right\} \leq \frac{C}{N_{1-a}^2}\cdot\frac{1}{N-1}\sum_{k:k\neq i}(b_{i,k}-\overline{b}_{i,\cdot})^4 = O\left(\frac{1}{N^2}\right).$$

Thus, similarly, $\mathbb{E}\{(\delta_i^c)^4\} = O(N^{-2})$. Write

$$\overline{b}_{i,\cdot}^A\overline{c}_{i,\cdot}^A = (\overline{b}_{i,\cdot}+\delta_i^b)(\overline{c}_{i,\cdot}+\delta_i^c) = \overline{b}_{i,\cdot}\overline{c}_{i,\cdot} + \overline{b}_{i,\cdot}\delta_i^c + \overline{c}_{i,\cdot}\delta_i^b + \delta_i^b\delta_i^c.$$

Then,

$$\frac{1}{N}\sum_{i=1}^N(\overline{b}_{i,\cdot}\overline{c}_{i,\cdot})^2 \leq \left(\frac{1}{N}\sum_{i=1}^N\overline{b}_{i,\cdot}^4\right)^{1/2}\left(\frac{1}{N}\sum_{i=1}^N\overline{c}_{i,\cdot}^4\right)^{1/2} = O(1),$$
$$\frac{1}{N}\sum_{i=1}^N(\overline{b}_{i,\cdot}\delta_i^c)^2 \leq \left(\frac{1}{N}\sum_{i=1}^N\overline{b}_{i,\cdot}^4\right)^{1/2}\left\{\frac{1}{N}\sum_{i=1}^N(\delta_i^c)^4\right\}^{1/2} = O(1)O\left(\frac{1}{N}\right) = O\left(\frac{1}{N}\right),$$

$$\frac{1}{N}\sum_{i=1}^{N}(\overline{c}_{i,\cdot}\delta_i^b)^2 \leq \left(\frac{1}{N}\sum_{i=1}^{N}\overline{c}_{i,\cdot}^4\right)^{1/2}\left\{\frac{1}{N}\sum_{i=1}^{N}(\delta_i^b)^4\right\}^{1/2} = O(1)O\left(\frac{1}{N}\right) = O\left(\frac{1}{N}\right),$$
$$\frac{1}{N}\sum_{i=1}^{N}(\delta_i^b\delta_i^c)^2 \leq \left\{\frac{1}{N}\sum_{i=1}^{N}(\delta_i^b)^4\right\}^{1/2}\left\{\frac{1}{N}\sum_{i=1}^{N}(\delta_i^c)^4\right\}^{1/2} = O\left(\frac{1}{N}\right)O\left(\frac{1}{N}\right) = O\left(\frac{1}{N^2}\right),$$

Let $S_i = \overline{b}_{i,\cdot}^A\overline{c}_{i,\cdot}^A$ and $S_j = \overline{b}_{j,\cdot}^A\overline{c}_{j,\cdot}^A$. Thus, $\mathbb{E}(S_i^2|A_i = a) = O(1)$. For $i \neq j$, we have

$$\mathbb{C}\mathrm{ov}\left\{\mathbb{1}_i(a)S_i, \mathbb{1}_j(a)S_j\right\} = \mathbb{E}\left\{\mathbb{1}_i(a)S_i\mathbb{1}_j(a)S_j\right\} - \mathbb{E}\left\{\mathbb{1}_i(a)S_i\right\}\mathbb{E}\left\{\mathbb{1}_j(a)S_j\right\}.$$

Define

$$\pi_{aa} = \mathbb{P}(A_i = a, A_j = a) = \frac{N_a(N_a-1)}{N(N-1)} = \pi_a^2 + O\left(\frac{1}{N}\right).$$

Then,

$$\mathbb{E}\left\{\mathbb{1}_i(a)S_i\mathbb{1}_j(a)S_j\right\} = \pi_{aa}\mathbb{E}\left(S_iS_j|A_i = a, A_j = a\right).$$

Given $A_i = a, A_j = a$, the set $\mathcal{B} = \{i : A_i = 1-a\}$ is a simple random sample of size $N_{1-a}$ from $\mathcal{U} = \{1,\ldots,N\} \setminus \{i,j\}$, with $|\mathcal{U}| = m = N-2$. Let $\mathbb{E}_{\mathcal{B}}(\cdot)$ denote expectation over $\mathcal{B}$. We have

$$\mathbb{E}\left(S_iS_j|A_i = a, A_j = a\right) = \mathbb{E}_{\mathcal{B}}\left(S_iS_j\right) = \mathbb{C}\mathrm{ov}_{\mathcal{B}}\left(S_i, S_j\right) + \mathbb{E}_{\mathcal{B}}\left(S_i\right)\mathbb{E}_{\mathcal{B}}\left(S_j\right). \tag{S61}$$

by the covariance formula for sampling without replacement, for any deterministic sequences $x_u, y_u$ for $u \in \mathcal{U}$,

$$\mathbb{C}\mathrm{ov}_{\mathcal{B}}\left(\frac{1}{n}\sum_{u\in\mathcal{B}}x_u, \frac{1}{n}\sum_{u\in\mathcal{B}}y_u\right) = \frac{m-n}{mn(m-1)}\sum_{u\in\mathcal{U}}(x_u-\overline{x})(y_u-\overline{y}),$$

where $\overline{x} = m^{-1}\sum_{u\in\mathcal{U}}x_u$, $n = N_{1-a}$, and $m - n = N_a - 2$. Here, $m \asymp N$, $n \asymp N$, so

$$\frac{m-n}{mn(m-1)} \asymp \frac{1}{N^2}.$$

The sum $\sum_{u\in\mathcal{U}}(x_u-\overline{x})(y_u-\overline{y}) = O(N)$ if $x_u, y_u$ are bounded. Thus,

$$\mathbb{C}\mathrm{ov}_{\mathcal{B}}\left(\frac{1}{n}\sum_{u\in\mathcal{B}}x_u, \frac{1}{n}\sum_{u\in\mathcal{B}}y_u\right) = O\left(\frac{1}{N}\right). \tag{S62}$$

Now, rewrite

$$S_i = \frac{1}{N_{1-a}}\sum_{u\in\mathcal{B}}b_{i,u}\frac{1}{N_{1-a}}\sum_{u\in\mathcal{B}}c_{i,u} = M_i^bM_i^c, \quad S_j = \frac{1}{N_{1-a}}\sum_{u\in\mathcal{B}}b_{j,u}\frac{1}{N_{1-a}}\sum_{u\in\mathcal{B}}c_{j,u} = M_j^bM_j^c,$$

with

$$\mu_i^b = \mathbb{E}_{\mathcal{B}}(M_i^b) = \frac{1}{N-2}\sum_{u\in\mathcal{U}}b_{i,u}, \quad \mu_i^c = \mathbb{E}_{\mathcal{B}}\left(M_i^c\right) = \frac{1}{N-2}\sum_{u\in\mathcal{U}}c_{i,u},$$

$$\mu_j^b = \mathbb{E}_{\mathcal{B}}(M_j^b) = \frac{1}{N-2}\sum_{u\in\mathcal{U}} b_{j,u}, \quad \mu_j^c = \mathbb{E}_{\mathcal{B}}\left(M_j^c\right) = \frac{1}{N-2}\sum_{u\in\mathcal{U}} c_{j,u}.$$

and

$$\Delta_i^b = M_i^b - \mu_i^b, \quad \Delta_i^c = M_i^c - \mu_i^c, \quad \Delta_j^b = M_j^b - \mu_j^b, \quad \Delta_j^c = M_j^c - \mu_j^c.$$

Then,

$$\begin{aligned} S_i &= (\mu_i^b + \Delta_i^b)(\mu_i^c + \Delta_i^c) = \mu_i^b\mu_i^c + \mu_i^b\Delta_i^c + \mu_i^c\Delta_i^b + \Delta_i^c\Delta_i^b, \\ S_j &= \mu_j^b\mu_j^c + \mu_j^b\Delta_j^c + \mu_j^c\Delta_j^b + \Delta_j^b\Delta_j^c. \end{aligned}$$

Write $S_i = P_i + Q_i$, where

$$P_i = \mu_i^b\mu_i^c, \quad Q_i = \mu_i^b\Delta_i^c + \mu_i^c\Delta_i^b + \Delta_i^b\Delta_i^c.$$

Similarly, for $S_j$. Then

$$S_iS_j = P_iP_j + P_iQ_j + Q_iP_j + Q_iQ_j.$$

So,

$$\mathbb{E}_{\mathcal{B}}(S_iS_j) = P_iP_j + P_i\mathbb{E}(Q_j) + P_j\mathbb{E}(Q_i) + \mathbb{E}(Q_iQ_j) = P_iP_j + \mathbb{E}(Q_iQ_j).$$

Since $\mathbb{E}_{\mathcal{B}}(S_i) = P_i$ and $\mathbb{E}_{\mathcal{B}}(S_j) = P_j$, then $\mathbb{C}\text{ov}_{\mathcal{B}}(S_i, S_j) = \mathbb{E}(Q_iQ_j)$. Specifically,

$$\begin{aligned} Q_iQ_j = &(\mu_i^b\Delta_i^c)(\mu_j^b\Delta_j^c) + (\mu_i^b\Delta_i^c)(\mu_j^c\Delta_j^b) + (\mu_i^b\Delta_i^c)(\Delta_j^b\Delta_j^c) + (\mu_i^c\Delta_i^b)(\mu_j^b\Delta_j^c) \\ &+ (\mu_i^c\Delta_i^b)(\mu_j^c\Delta_j^b) + (\mu_i^c\Delta_i^b)(\Delta_j^b\Delta_j^c) + (\Delta_i^b\Delta_i^c)(\mu_j^b\Delta_j^c) + (\Delta_i^b\Delta_i^c)(\mu_j^c\Delta_j^b) \\ &+ (\Delta_i^b\Delta_i^c)(\Delta_j^b\Delta_j^c). \end{aligned}$$

By (S62), we have

$$\mathbb{E}(\Delta_i^b\Delta_j^b) = O\left(\frac{1}{N}\right), \quad \mathbb{E}(\Delta_i^c\Delta_j^c) = O\left(\frac{1}{N}\right), \quad \mathbb{E}(\Delta_i^b\Delta_j^c) = O\left(\frac{1}{N}\right), \quad \mathbb{E}(\Delta_i^c\Delta_j^b) = O\left(\frac{1}{N}\right).$$

Also, by the Cauchy-Schwarz inequality,

$$\mathbb{E}(|\Delta_i^b\Delta_i^c|) \le \left[\mathbb{E}\{(\Delta_i^b)^2\}\mathbb{E}\{(\Delta_i^c)^2\}\right]^{1/2} = O\left(\frac{1}{N}\right),$$

since variances are $O(N^{-1})$. Similarly,

$$\begin{aligned} \mathbb{E}(|\Delta_i^b\Delta_j^b\Delta_j^c|) &\le \left[\mathbb{E}\{(\Delta_i^b)^2\}\mathbb{E}\{(\Delta_j^b\Delta_j^c)^2\}\right]^{1/2} \le \left[\mathbb{E}\{(\Delta_i^b)^2\}\mathbb{E}\{(\Delta_j^b)^4\}^{1/2}\mathbb{E}\{(\Delta_j^c)^4\}^{1/2}\right]^{1/2} \\ &= \left\{O\left(\frac{1}{N}\right)O\left(\frac{1}{N}\right)O\left(\frac{1}{N}\right)\right\}^{1/2} = O\left(\frac{1}{N^{3/2}}\right). \end{aligned}$$

Similarly, any term with three $\Delta$'s is $O(N^{-3/2})$, and four $\Delta$'s $O(N^{-2})$. Therefore,

$$\mathbb{E}\left\{(\mu_i^b\Delta_i^c)(\mu_j^b\Delta_j^c)\right\} = \mu_i^b\mu_j^b\mathbb{E}(\Delta_i^c\Delta_j^c) = O(1)O\left(\frac{1}{N}\right) = O\left(\frac{1}{N}\right),$$

$$
\begin{aligned}
&\mathbb{E}\left\{(\mu_i^b\Delta_i^c)(\mu_j^c\Delta_j^b)\right\} = \mu_i^b\mu_j^c\mathbb{E}(\Delta_i^c\Delta_j^b) = O\left(\frac{1}{N}\right), \\
&\mathbb{E}\left\{(\mu_i^b\Delta_i^c)(\Delta_j^b\Delta_j^c)\right\} = \mu_i^b\mathbb{E}(\Delta_i^c\Delta_j^b\Delta_j^c) = O(1)O\left(\frac{1}{N^{3/2}}\right) = O\left(\frac{1}{N^{3/2}}\right), \\
&\mathbb{E}\left\{(\mu_i^c\Delta_i^b)(\mu_j^b\Delta_j^c)\right\} = O\left(\frac{1}{N}\right), \quad \mathbb{E}\left\{(\mu_i^c\Delta_i^b)(\mu_j^c\Delta_j^b)\right\} = O\left(\frac{1}{N}\right), \\
&\mathbb{E}\left\{(\mu_i^c\Delta_i^b)(\Delta_j^b\Delta_j^c)\right\} = O\left(\frac{1}{N^{3/2}}\right), \quad \mathbb{E}\left\{(\Delta_i^b\Delta_i^c)(\mu_j^b\Delta_j^c)\right\} = O\left(\frac{1}{N^{3/2}}\right), \\
&\mathbb{E}\left\{(\Delta_i^b\Delta_i^c)(\mu_j^c\Delta_j^b)\right\} = O\left(\frac{1}{N^{3/2}}\right), \quad \mathbb{E}\left\{(\Delta_i^b\Delta_i^c)(\Delta_j^b\Delta_j^c)\right\} = O\left(\frac{1}{N^2}\right).
\end{aligned}
$$

Thus,

$$
\mathbb{E}(Q_iQ_j) = \mathbb{C}\text{ov}_{\mathcal{B}}(S_i, S_j) = O\left(\frac{1}{N}\right).
$$

Hence

$$
\mathbb{E}(S_iS_j|A_i = a, A_j = a) = \mathbb{E}_{\mathcal{B}}\left(S_i\right)\mathbb{E}_{\mathcal{B}}\left(S_j\right) + O\left(\frac{1}{N}\right).
$$

Since excluding one unit changes the finite-sample expectation by $O(N^{-1})$, we have

$$
\mathbb{E}_{\mathcal{B}}\left(S_i\right) = \mathbb{E}(S_i|A_i = a) + O\left(\frac{1}{N}\right),
$$

which, by (S61), leads to

$$
\mathbb{E}(S_iS_j|A_i = a, A_j = a) = \mathbb{E}(S_i|A_i = a)^2 + O\left(\frac{1}{N}\right).
$$

Putting everything together, we have

$$
\begin{aligned}
&\mathbb{E}\left\{\mathbb{1}_i(a)S_i\mathbb{1}_j(a)S_j\right\} = \pi_{aa}\left\{\mathbb{E}(S_i|A_i = a)^2 + O\left(\frac{1}{N}\right)\right\}, \\
&\mathbb{E}\{\mathbb{1}_i(a)S_i\}\mathbb{E}\{\mathbb{1}_j(a)S_j\} = \pi_a^2\mathbb{E}(S_i|A_i = a)^2.
\end{aligned}
$$

Thus,

$$
\mathbb{C}\text{ov}\left\{\mathbb{1}_i(a)S_i, \mathbb{1}_j(a)S_j\right\} = \left\{\pi_a^2 + O\left(\frac{1}{N}\right)\right\}\left\{\mathbb{E}(S_i|A_i = a)^2 + O\left(\frac{1}{N}\right)\right\} - \pi_a^2\mathbb{E}(S_i|A_i = a)^2 = O\left(\frac{1}{N}\right).
$$

Lastly,

$$
\begin{aligned}
\mathbb{V}\text{ar}\left\{\frac{1}{N_a}\sum_{i=1}^N \mathbb{1}_i(a)S_i\right\} &= \frac{1}{N_a^2}\left[\sum_{i=1}^N \mathbb{V}\text{ar}\left\{\mathbb{1}_i(a)S_i\right\} + \sum_{i\neq j}\mathbb{C}\text{ov}\left\{\mathbb{1}_i(a)S_i, \mathbb{1}_j(a)S_j\right\}\right] \\
&= O\left(\frac{1}{N^2}\right)\left\{N\cdot O(1) + N(N-1)\cdot O\left(\frac{1}{N}\right)\right\} \\
&= O\left(\frac{1}{N^2}\right)O(N) = O\left(\frac{1}{N}\right).
\end{aligned}
$$

## S6.4 Lemma S7

### S6.4.1 Expectation

For $\widehat{\lambda}_{\mathrm{I}}(a, 1-a)$, we have

$$\mathbb{E}\left\{\widehat{\lambda}_{\mathrm{I}}(a,1-a)\right\} = \mathbb{E}\left\{\frac{\sum_{i\neq j} \mathbb{1}_i(a)\mathbb{1}_j(1-a)W_{i,j}}{|\mathcal{S}(a,1-a)|}\right\} = \frac{1}{N_1N_0}\sum_{i\neq j}\mathbb{E}\left\{\mathbb{1}_i(a)\mathbb{1}_j(1-a)\right\}W_{i,j}(a,1-a)$$
$$= \frac{1}{N_1N_0}\sum_{i\neq j}\frac{N_1N_0}{N(N-1)}W_{i,j}(a,1-a) = \overline{W}(a,1-a) = \lambda(a,1-a).$$

### S6.4.2 Variance

By the property of the OLS fit,

$$\begin{pmatrix}\widehat{\lambda}_{\mathrm{I}}(a,1-a)-\lambda(a,1-a)\\ \widehat{\lambda}_{\mathrm{I}}(1-a,a)-\lambda(1-a,a)\end{pmatrix} = \begin{pmatrix}\overline{W}_{\mathcal{S}(a,1-a)}-\overline{W}(a,1-a)\\ \overline{W}_{\mathcal{S}(1-a,a)}-\overline{W}(1-a,a)\end{pmatrix}.$$

Then,

$$\widehat{\lambda}_{\mathrm{I}}(a,1-a)-\lambda(a,1-a) = \frac{1}{N_1N_0}\sum_{(i,j)\in\mathcal{S}(a,1-a)}\left\{W_{i,j}-\overline{W}(a,1-a)\right\} = \frac{1}{N_1N_0}\sum_{(i,j)\in\mathcal{S}(a,1-a)}\epsilon_{i,j}(a,1-a).$$

Let

$$\mathbf{\Psi}_{\mathrm{I}} = \begin{pmatrix}\widehat{\lambda}_{\mathrm{I}}(a,1-a)-\lambda(a,1-a)\\ \widehat{\lambda}_{\mathrm{I}}(1-a,a)-\lambda(1-a,a)\end{pmatrix} = \frac{1}{N(N-1)}\sum_{i\neq j}\frac{N(N-1)}{N_1N_0}\begin{pmatrix}\mathbb{1}_i(a)\mathbb{1}_j(1-a)\epsilon_{i,j}(a,1-a)\\ \mathbb{1}_i(1-a)\mathbb{1}_j(a)\epsilon_{i,j}(1-a,a)\end{pmatrix}$$
$$\equiv \frac{1}{N(N-1)}\sum_{i\neq j}\boldsymbol{\psi}_{\mathrm{I},i,j}.$$

By the Hoeffding decomposition (van der Vaart, 1998, §11.4 & §12.3),

$$\mathbf{\Psi}_{\mathrm{I}} = \mathbb{E}(\mathbf{\Psi}_{\mathrm{I}}) + \frac{1}{N}\sum_{i=1}^{N}\boldsymbol{\psi}_{\mathrm{I},i}^{(1)} + \frac{1}{N}\sum_{j=1}^{N}\boldsymbol{\psi}_{\mathrm{I},j}^{(2)} + \frac{1}{N(N-1)}\sum_{i\neq j}\widetilde{\boldsymbol{\psi}}_{\mathrm{I},i,j},$$

where

$$\boldsymbol{\psi}_{\mathrm{I},i}^{(1)} = \frac{1}{N-1}\sum_{j:j\neq i}\left\{\mathbb{E}(\boldsymbol{\psi}_{\mathrm{I},i,j}|A_i)-\mathbb{E}(\mathbf{\Psi}_{\mathrm{I}})\right\}, \quad \boldsymbol{\psi}_{\mathrm{I},j}^{(2)} = \frac{1}{N-1}\sum_{i:i\neq j}\left\{\mathbb{E}(\boldsymbol{\psi}_{\mathrm{I},i,j}|A_j)-\mathbb{E}(\mathbf{\Psi}_{\mathrm{I}})\right\},$$
$$\widetilde{\boldsymbol{\psi}}_{\mathrm{I},i,j} = \boldsymbol{\psi}_{\mathrm{I},i,j} - \boldsymbol{\psi}_{\mathrm{I},i}^{(1)} - \boldsymbol{\psi}_{\mathrm{I},j}^{(2)} + \mathbb{E}(\mathbf{\Psi}_{\mathrm{I}})$$

with $\mathbb{E}(\mathbf{\Psi}_{\mathrm{I}}) = \mathbf{0}$, $\mathbb{E}(\boldsymbol{\psi}_{\mathrm{I},i}^{(1)}) = \mathbf{0}$, $\mathbb{E}(\boldsymbol{\psi}_{\mathrm{I},j}^{(2)}) = \mathbf{0}$, and $\mathbb{E}(\widetilde{\boldsymbol{\psi}}_{\mathrm{I},i,j}) = \mathbf{0}$. Specifically,

$$\boldsymbol{\psi}_{\mathrm{I},i}^{(1)} = \begin{pmatrix}\frac{1}{\pi_a}\bar{\epsilon}_{i,\cdot}(a,1-a)\mathbb{1}_i(a)\\ \frac{1}{\pi_{1-a}}\bar{\epsilon}_{i,\cdot}(1-a,a)\mathbb{1}_i(1-a)\end{pmatrix}, \quad \boldsymbol{\psi}_{\mathrm{I},j}^{(2)} = \begin{pmatrix}\frac{1}{\pi_{1-a}}\bar{\epsilon}_{\cdot,j}(a,1-a)\mathbb{1}_j(1-a)\\ \frac{1}{\pi_a}\bar{\epsilon}_{\cdot,j}(1-a,a)\mathbb{1}_j(1-a)\end{pmatrix}.$$

After relabeling, we have

$$\boldsymbol{\Psi}_{\mathrm{I}} = \frac{1}{N}\sum_{i=1}^{N}\left(\boldsymbol{\psi}_{\mathrm{I},i}^{(1)} + \boldsymbol{\psi}_{\mathrm{I},i}^{(2)}\right) + \frac{1}{N(N-1)}\sum_{i\neq j}\widetilde{\boldsymbol{\psi}}_{\mathrm{I},i,j} = \boldsymbol{\Psi}_{\mathrm{I}}^{*} + \frac{1}{N(N-1)}\sum_{i\neq j}\widetilde{\boldsymbol{\psi}}_{\mathrm{I},i,j}.$$

Since, under Condition S1, $\boldsymbol{\psi}_{\mathrm{I},i,j} = \boldsymbol{O}_{\mathbb{P}}(1)$, then

$$\mathbb{V}\mathrm{ar}\left\{\frac{1}{N(N-1)}\sum_{i\neq j}\widetilde{\boldsymbol{\psi}}_{\mathrm{I},i,j}\right\} = \boldsymbol{O}\left(\frac{1}{N^2}\right).$$

We then calculate the $\mathbb{V}\mathrm{ar}(\boldsymbol{\Psi}_{\mathrm{I}}^{*})$. Specifically, $\boldsymbol{\Psi}_{\mathrm{I}}^{*} = (\Psi_{\mathrm{I}}^{*}(a,1-a), \Psi_{\mathrm{I}}^{*}(1-a,a))^{\top}$, where

$$\Psi_{\mathrm{I}}^{*}(a,1-a) = \frac{1}{N_a}\sum_{i=1}^{N}\bar{\epsilon}_{i,\cdot}(a,1-a)\mathbb{1}_i(a) + \frac{1}{N_{1-a}}\sum_{i=1}^{N}\bar{\epsilon}_{\cdot,i}(a,1-a)\mathbb{1}_i(1-a).$$

Under complete randomization with fixed $N_a$, we have

$$\begin{aligned}
\mathbb{V}\mathrm{ar}\{\Psi_{\mathrm{I}}^{*}(a,1-a)\} &= \left(\frac{1}{N_a} - \frac{1}{N}\right)\frac{1}{N-1}\sum_{i=1}^{N}\bar{\epsilon}_{i,\cdot}(a,1-a)^2 + \left(\frac{1}{N_{1-a}} - \frac{1}{N}\right)\frac{1}{N-1}\sum_{i=1}^{N}\bar{\epsilon}_{\cdot,i}(a,1-a)^2 \\
&\quad - \frac{2}{N}\cdot\frac{1}{N-1}\sum_{i=1}^{N}\bar{\epsilon}_{i,\cdot}(a,1-a)\bar{\epsilon}_{\cdot,i}(a,1-a) \\
&= \frac{1}{N-1}V\{\bar{\epsilon}_i(a,1-a)\}.
\end{aligned}$$

For $\mathbb{C}\mathrm{ov}\{\Psi_{\mathrm{I}}^{*}(a,1-a), \Psi_{\mathrm{I}}^{*}(1-a,a)\}$, we have

$$\begin{aligned}
\Psi_{\mathrm{I}}^{*}(a,1-a) &= \frac{1}{\pi_a N}\sum_{i=1}^{N}\bar{\epsilon}_{i,\cdot}(a,1-a)\mathbb{1}_i(a) + \frac{1}{\pi_{1-a}N}\sum_{i=1}^{N}\bar{\epsilon}_{\cdot,i}(a,1-a)\mathbb{1}_i(1-a), \\
\Psi_{\mathrm{I}}^{*}(1-a,a) &= \frac{1}{\pi_{1-a}N}\sum_{i=1}^{N}\bar{\epsilon}_{i,\cdot}(1-a,a)\mathbb{1}_i(1-a) + \frac{1}{\pi_a N}\sum_{i=1}^{N}\bar{\epsilon}_{\cdot,i}(1-a,a)\mathbb{1}_i(a).
\end{aligned}$$

Let

$$\begin{aligned}
J_1 &= \frac{1}{\pi_a N}\sum_{i=1}^{N}\bar{\epsilon}_{i,\cdot}(a,1-a)\mathbb{1}_i(a), \quad \frac{1}{\pi_{1-a}N}\sum_{i=1}^{N}\bar{\epsilon}_{\cdot,i}(a,1-a)\mathbb{1}_i(1-a), \\
J_3 &= \frac{1}{\pi_{1-a}N}\sum_{i=1}^{N}\bar{\epsilon}_{i,\cdot}(1-a,a)\mathbb{1}_i(1-a), \quad J_4 = \frac{1}{\pi_a N}\sum_{i=1}^{N}\bar{\epsilon}_{\cdot,i}(1-a,a)\mathbb{1}_i(a).
\end{aligned}$$

Then,

$$\mathbb{C}\mathrm{ov}\{\Psi_{\mathrm{I}}^{*}(a,1-a), \Psi_{\mathrm{I}}^{*}(1-a,a)\} = \mathbb{C}\mathrm{ov}(J_1,J_3) + \mathbb{C}\mathrm{ov}(J_1,J_4) + \mathbb{C}\mathrm{ov}(J_2,J_3) + \mathbb{C}\mathrm{ov}(J_2,J_4).$$

For simple random sampling of size $N_a$ from $N$,

$$\mathbb{C}\mathrm{ov}\left(\frac{1}{N_a}\sum_{i:A_i=a}x_i, \frac{1}{N_{1-a}}\sum_{i:A_i=1-a}y_i\right) = -\frac{1}{N}s_{xy} = -\frac{1}{N}\cdot\frac{1}{N-1}\sum_{i=1}^{N}x_iy_i,$$

$$\mathbb{C}\text{ov}\left(\frac{1}{N_a}\sum_{i:A_i=a} x_i, \frac{1}{N_a}\sum_{i:A_i=a} y_i\right) = \left(\frac{1}{N_a} - \frac{1}{N}\right) s_{xy} = \left(\frac{1}{N_a} - \frac{1}{N}\right) \frac{1}{N-1}\sum_{i=1}^{N} x_i y_i.$$

Thus,

$$\begin{aligned}
\mathbb{C}\text{ov}(J_1, J_3) &= -\frac{1}{N} \cdot \frac{1}{N-1}\sum_{i=1}^{N} \overline{\epsilon}_{i,\cdot}(a, 1-a)\overline{\epsilon}_{i,\cdot}(1-a, a), \\
\mathbb{C}\text{ov}(J_1, J_4) &= \left(\frac{1}{N_1} - \frac{1}{N}\right) \cdot \frac{1}{N-1}\sum_{i=1}^{N} \overline{\epsilon}_{i,\cdot}(a, 1-a)\overline{\epsilon}_{\cdot,i}(1-a, a), \\
\mathbb{C}\text{ov}(J_2, J_3) &= \left(\frac{1}{N_{1-a}} - \frac{1}{N}\right) \cdot \frac{1}{N-1}\sum_{i=1}^{N} \overline{\epsilon}_{\cdot,i}(a, 1-a)\overline{\epsilon}_{i,\cdot}(1-a, a), \\
\mathbb{C}\text{ov}(J_2, J_4) &= -\frac{1}{N} \cdot \frac{1}{N-1}\sum_{i=1}^{N} \overline{\epsilon}_{\cdot,i}(a, 1-a)\overline{\epsilon}_{\cdot,i}(1-a, a).
\end{aligned}$$

Summing up these terms, we have

$$\begin{aligned}
&\mathbb{C}\text{ov}\{\Psi_{\mathrm{I}}^*(a, 1-a), \Psi_{\mathrm{I}}^*(1-a, a)\} \\
&= -\frac{1}{N(N-1)}\sum_{i=1}^{N} \overline{\epsilon}_{i,\cdot}(a, 1-a)\overline{\epsilon}_{i,\cdot}(1-a, a) + \left(\frac{1}{N_a} - \frac{1}{N}\right)\frac{1}{N-1}\sum_{i=1}^{N} \overline{\epsilon}_{i,\cdot}(a, 1-a)\overline{\epsilon}_{\cdot,i}(1-a, a) \\
&\quad + \left(\frac{1}{N_{1-a}} - \frac{1}{N}\right)\frac{1}{N-1}\sum_{i=1}^{N} \overline{\epsilon}_{\cdot,i}(a, 1-a)\overline{\epsilon}_{i,\cdot}(1-a, a) - \frac{1}{N(N-1)}\sum_{i=1}^{N} \overline{\epsilon}_{\cdot,i}(a, 1-a)\overline{\epsilon}_{\cdot,i}(1-a, a) \\
&= \frac{1}{N-1} CV(\overline{\epsilon}_i).
\end{aligned}$$

## S6.5 Lemma S8

We have

$$\begin{aligned}
\widehat{\gamma}_{\mathrm{I}}^{\mathrm{adj}}(a, 1-a) = &\left\{\sum_{(i,j)\in\mathcal{S}(a,1-a)} \left(\boldsymbol{X}_{i,j} - \overline{\boldsymbol{X}}_{\mathcal{S}(a,1-a)}\right)\left(\boldsymbol{X}_{i,j} - \overline{\boldsymbol{X}}_{\mathcal{S}(a,1-a)}\right)^{\top}\right\}^{-1} \\
&\times \sum_{(i,j)\in\mathcal{S}(a,1-a)} \left(\boldsymbol{X}_{i,j} - \overline{\boldsymbol{X}}_{\mathcal{S}(a,1-a)}\right)\left(W_{i,j} - \overline{W}_{\mathcal{S}(a,1-a)}\right).
\end{aligned}$$

First, consider the numerator of $\widehat{\gamma}_{\mathrm{I}}^{\mathrm{adj}}(a, 1-a)$. By Condition 3 in the main article,

$$\mathbb{E}\left\{\frac{1}{N(N-1)}\sum_{(i,j)\in\mathcal{S}(a,1-a)} \boldsymbol{X}_{i,j}W_{i,j}\right\} = \frac{\pi_1\pi_0}{N(N-1)}\sum_{i\neq j} \boldsymbol{X}_{i,j}W_{i,j}(a, 1-a) = \boldsymbol{O}(1).$$

Lemma S2 and Condition 2 in the main article imply that

$$\mathbb{V}\text{ar}\left\{\frac{1}{N(N-1)}\sum_{(i,j)\in\mathcal{S}(a,1-a)} \boldsymbol{X}_{i,j}W_{i,j}\right\} = \boldsymbol{O}\left(\frac{1}{N}\right).$$

Therefore,

$$\frac{1}{N(N-1)} \sum_{(i,j)\in\mathcal{S}(a,1-a)} \boldsymbol{X}_{i,j} W_{i,j} = \frac{\pi_1\pi_0}{N(N-1)} \sum_{i\neq j} \boldsymbol{X}_{i,j} W_{i,j}(a,1-a) + \boldsymbol{O}_{\mathbb{P}}\left(\frac{1}{N^{1/2}}\right).$$

Similarly, Lemma S4 implies

$$\overline{\boldsymbol{X}}_{\mathcal{S}(a,1-a)} = \frac{1}{N(N-1)} \sum_{i\neq j} \boldsymbol{X}_{i,j} + \boldsymbol{O}_{\mathbb{P}}\left(\frac{1}{N^{1/2}}\right) = \boldsymbol{O}_{\mathbb{P}}\left(\frac{1}{N^{1/2}}\right),$$
$$\overline{W}_{\mathcal{S}(a,1-a)} = \frac{1}{N(N-1)} \sum_{i\neq j} W_{i,j}(a,1-a) + O_{\mathbb{P}}\left(\frac{1}{N^{1/2}}\right) = \overline{W}(a,1-a) + O_{\mathbb{P}}\left(\frac{1}{N^{1/2}}\right).$$

Therefore, the numerator and the denominator of $\widehat{\boldsymbol{\gamma}}_{\mathrm{I}}^{\mathrm{adj}}(a,1-a)$ satisfy

$$\begin{aligned}&\frac{1}{N(N-1)} \sum_{(i,j)\in\mathcal{S}(a,1-a)} \left(\boldsymbol{X}_{i,j} - \overline{\boldsymbol{X}}_{\mathcal{S}(a,1-a)}\right)\left(W_{i,j} - \overline{W}_{\mathcal{S}(a,1-a)}\right)\\ &= \frac{\pi_1\pi_0}{N(N-1)} \sum_{i\neq j} \boldsymbol{X}_{i,j} W_{i,j}(a,1-a) + \boldsymbol{O}_{\mathbb{P}}\left(\frac{1}{N^{1/2}}\right)\end{aligned}$$

and

$$\begin{aligned}&\frac{1}{N(N-1)} \sum_{(i,j)\in\mathcal{S}(a,1-a)} \left(\boldsymbol{X}_{i,j} - \overline{\boldsymbol{X}}_{\mathcal{S}(a,1-a)}\right)\left(\boldsymbol{X}_{i,j} - \overline{\boldsymbol{X}}_{\mathcal{S}(a,1-a)}\right)^\top\\ &= \frac{\pi_1\pi_0}{N(N-1)} \sum_{i\neq j} \boldsymbol{X}_{i,j}\boldsymbol{X}_{i,j}^\top + \boldsymbol{O}_{\mathbb{P}}\left(\frac{1}{N^{1/2}}\right).\end{aligned}$$

By Lemma S3, we have $\widehat{\boldsymbol{\gamma}}_{\mathrm{I}}^{\mathrm{adj}}(a,1-a) - \boldsymbol{\gamma}_{\mathrm{I}}^{\mathrm{adj}}(a,1-a) = \boldsymbol{O}_{\mathbb{P}}(N^{-1/2})$.

## S6.6 Lemma S9

By the property of the OLS,

$$\widehat{\lambda}_{\mathrm{I}}^{\mathrm{adj}}(a,1-a) = \overline{W}_{\mathcal{S}(a,1-a)} - \overline{\boldsymbol{X}}_{\mathcal{S}(a,1-a)}^\top \widehat{\boldsymbol{\gamma}}_{\mathrm{I}}^{\mathrm{adj}}(a,1-a).$$

Thus,

$$\begin{aligned}&\widehat{\lambda}_{\mathrm{I}}^{\mathrm{adj}}(a,1-a) - \lambda(a,1-a)\\ &= \left\{\overline{W}_{\mathcal{S}(a,1-a)} - \lambda(a,1-a)\right\} - \overline{\boldsymbol{X}}_{\mathcal{S}(a,1-a)}^\top \widehat{\boldsymbol{\gamma}}_{\mathrm{I}}^{\mathrm{adj}}(a,1-a)\\ &= \frac{1}{N_1N_0} \sum_{(i,j)\in\mathcal{S}(a,1-a)} \left\{W_{i,j} - \overline{W}(a,1-a) - \boldsymbol{X}_{i,j}^\top \boldsymbol{\gamma}_{\mathrm{I}}^{\mathrm{adj}}(a,1-a)\right\} + \overline{\boldsymbol{X}}_{\mathcal{S}(a,1-a)}^\top \left\{\boldsymbol{\gamma}_{\mathrm{I}}^{\mathrm{adj}}(a,1-a) - \widehat{\boldsymbol{\gamma}}_{\mathrm{I}}^{\mathrm{adj}}(a,1-a)\right\}\\ &= \frac{1}{N_1N_0} \sum_{(i,j)\in\mathcal{S}(a,1-a)} r_{\mathrm{I},i,j}^{\mathrm{adj}}(a,1-a) + \overline{\boldsymbol{X}}_{\mathcal{S}(a,1-a)}^\top \left\{\boldsymbol{\gamma}_{\mathrm{I}}^{\mathrm{adj}}(a,1-a) - \widehat{\boldsymbol{\gamma}}_{\mathrm{I}}^{\mathrm{adj}}(a,1-a)\right\}.\end{aligned}$$

By Lemma S8, $\widehat{\boldsymbol{\gamma}}_{\mathrm{I}}^{\mathrm{adj}}(a,1-a) - \boldsymbol{\gamma}_{\mathrm{I}}^{\mathrm{adj}}(a,1-a) = \boldsymbol{O}_{\mathbb{P}}(N^{-1/2})$ and $\overline{\boldsymbol{X}}_{\mathcal{S}(a,1-a)} = \boldsymbol{O}_{\mathbb{P}}(N^{-1/2})$. Therefore,

$$\widehat{\lambda}_{\mathrm{I}}^{\mathrm{adj}}(a,1-a) - \lambda(a,1-a) = \frac{1}{N_1N_0} \sum_{(i,j)\in\mathcal{S}(a,1-a)} r_{\mathrm{I},i,j}^{\mathrm{adj}}(a,1-a) + O_{\mathbb{P}}\left(\frac{1}{N}\right).$$

Hence, applying the same arguments (the Hoeffding decomposition) in the proof of Lemma S7, we have $\mathbb{V}\mathrm{ar}\{\widehat{\lambda}_{\mathrm{I}}^{\mathrm{adj}}(a, 1-a)\}$, and similarly, the covariance $\mathbb{C}\mathrm{ov}\{\widehat{\lambda}_{\mathrm{I}}^{\mathrm{adj}}(a, 1-a), \widehat{\lambda}_{\mathrm{I}}^{\mathrm{adj}}(1-a, a)\}$.

## S6.7 Lemma S10

We derive the probability limit of $\widehat{\gamma}_{\mathrm{I}}^{\mathrm{acv}}$. The convergence proof follows that of Lemma S8 and is thus omitted. We can obtain $\widehat{\gamma}_{\mathrm{I}}^{\mathrm{acv}}$ by Frisch-Waugh-Lovell. The residual from the OLS of $W_{i,j}$ on $(A_i(1-A_j), (1-A_i)A_j)$ is

$$W_{i,j}^{\mathrm{acv}} = W_{i,j} - A_i(1-A_j)\overline{W}_{\mathcal{S}(1,0)} - (1-A_i)A_j\overline{W}_{\mathcal{S}(0,1)},$$

and the residual from the OLS fit of $\boldsymbol{X}_{i,j}$ on $(A_i(1-A_j), (1-A_i)A_j)$ is

$$\boldsymbol{X}_{i,j}^{\mathrm{acv}} = \boldsymbol{X}_{i,j} - A_i(1-A_j)\overline{\boldsymbol{X}}_{\mathcal{S}(1,0)} - (1-A_i)A_j\overline{\boldsymbol{X}}_{\mathcal{S}(0,1)}.$$

Therefore,

$$\widehat{\gamma}_{\mathrm{I}}^{\mathrm{acv}} = \left(\sum_{i\neq j}\boldsymbol{X}_{i,j}^{\mathrm{acv}}\boldsymbol{X}_{i,j}^{\mathrm{acv}\top}\right)^{-1}\sum_{i\neq j}\boldsymbol{X}_{i,j}^{\mathrm{acv}}W_{i,j}^{\mathrm{acv}}.$$

By Lemma S2, the numerator of $\widehat{\gamma}_{\mathrm{I}}^{\mathrm{acv}}$ satisfies

$$\begin{aligned}
&\frac{1}{N(N-1)}\sum_{i\neq j}\boldsymbol{X}_{i,j}^{\mathrm{acv}}W_{i,j}^{\mathrm{acv}} \\
&= \frac{1}{N(N-1)}\sum_{(i,j)\in\mathcal{S}(1,0)}\left(\boldsymbol{X}_{i,j}-\overline{\boldsymbol{X}}_{\mathcal{S}(1,0)}\right)\left(W_{i,j}-\overline{W}_{\mathcal{S}(1,0)}\right) \\
&\quad + \frac{1}{N(N-1)}\sum_{(i,j)\in\mathcal{S}(0,1)}\left(\boldsymbol{X}_{i,j}-\overline{\boldsymbol{X}}_{\mathcal{S}(0,1)}\right)\left(W_{i,j}-\overline{W}_{\mathcal{S}(0,1)}\right) + \frac{1}{N(N-1)}\sum_{(i,j)\notin\mathcal{S}}\boldsymbol{X}_{i,j}W_{i,j} \\
&= \frac{1}{N(N-1)}\sum_{(i,j)\in\mathcal{S}(1,0)}\boldsymbol{X}_{i,j}W_{i,j} - \frac{N_1N_0}{N(N-1)}\overline{\boldsymbol{X}}_{\mathcal{S}(1,0)}\overline{W}_{\mathcal{S}(1,0)} \\
&\quad + \frac{1}{N(N-1)}\sum_{(i,j)\in\mathcal{S}(0,1)}\boldsymbol{X}_{i,j}W_{i,j} - \frac{N_1N_0}{N(N-1)}\overline{\boldsymbol{X}}_{\mathcal{S}(0,1)}\overline{W}_{\mathcal{S}(0,1)} + \frac{1}{N(N-1)}\sum_{(i,j)\notin\mathcal{S}}\boldsymbol{X}_{i,j}W_{i,j} \\
&= \frac{\pi_1\pi_0}{N(N-1)}\sum_{i\neq j}\boldsymbol{X}_{i,j}W_{i,j}(1,0) + \frac{\pi_1\pi_0}{N(N-1)}\sum_{i\neq j}\boldsymbol{X}_{i,j}W_{i,j}(0,1) \\
&\quad + \frac{\pi_1^2}{N(N-1)}\sum_{i\neq j}\boldsymbol{X}_{i,j}W_{i,j}(1,1) + \frac{\pi_0^2}{N(N-1)}\sum_{i\neq j}\boldsymbol{X}_{i,j}W_{i,j}(0,0) + \boldsymbol{O}_{\mathbb{P}}\left(\frac{1}{N^{1/2}}\right) \\
&= \frac{1}{N(N-1)}\sum_{i\neq j}\boldsymbol{X}_{i,j}\mathbb{E}\{W_{i,j}(A_i,A_j)\} + \boldsymbol{O}_{\mathbb{P}}\left(\frac{1}{N^{1/2}}\right).
\end{aligned}$$

Similarly, its denominator satisfies

$$\frac{1}{N(N-1)}\sum_{i\neq j}\boldsymbol{X}_{i,j}^{\mathrm{acv}}\boldsymbol{X}_{i,j}^{\mathrm{acv}\top} = \frac{1}{N(N-1)}\sum_{i\neq j}\boldsymbol{X}_{i,j}\boldsymbol{X}_{i,j}^{\top} + \boldsymbol{O}_{\mathbb{P}}\left(\frac{1}{N^{1/2}}\right).$$

By Lemma S3,

$$\widehat{\gamma}_{\mathrm{I}}^{\mathrm{acv}} = \left( \sum_{i \neq j} \boldsymbol{X}_{i,j} \boldsymbol{X}_{i,j}^{\top} \right)^{-1} \sum_{i \neq j} \boldsymbol{X}_{i,j} \mathbb{E}\{W_{i,j}(A_i, A_j)\} + \boldsymbol{O}_{\mathbb{P}} \left( \frac{1}{N^{1/2}} \right).$$

## S6.8 Lemma S11

By the property of the OLS,

$$\widehat{\lambda}_{\mathrm{I}}^{\mathrm{acv}}(a, 1-a) = \overline{W}_{\mathcal{S}(a,1-a)} - \overline{\boldsymbol{X}}_{\mathcal{S}(a,1-a)}^{\top} \widehat{\gamma}_{\mathrm{I}}^{\mathrm{acv}}.$$

Following the proof of Lemma S9,

$$\widehat{\lambda}_{\mathrm{F}}(a, 1-a) - \lambda(a, 1-a) = \frac{1}{N_1 N_0} \sum_{(i,j) \in \mathcal{S}(a,1-a)} r_{\mathrm{I},i,j}^{\mathrm{acv}}(a, 1-a) + O_{\mathbb{P}} \left( \frac{1}{N} \right),$$

where

$$r_{\mathrm{I},i,j}^{\mathrm{acv}}(a, 1-a) = W_{i,j}(a, 1-a) - \overline{W}(a, 1-a) - \boldsymbol{X}_{i,j}^{\top} \boldsymbol{\gamma}_{\mathrm{I}}^{\mathrm{acv}}.$$

Hence, applying the same technique via the Hoeffding decomposition, we have $\mathbb{V}\mathrm{ar}\{\widehat{\lambda}_{\mathrm{I}}^{\mathrm{acv}}(a, 1-a)\}$, and similarly, the covariance $\mathbb{C}\mathrm{ov}\{\widehat{\lambda}_{\mathrm{I}}^{\mathrm{acv}}(a, 1-a), \widehat{\lambda}_{\mathrm{I}}^{\mathrm{acv}}(a, 1-a)\}$.

## S6.9 Lemma S12

We have

$$\widehat{\boldsymbol{\gamma}}_{\mathrm{A},1}^{\mathrm{adj}}(a, 1-a) = \left\{ \sum_{i: A_i = a} \left( \overline{\boldsymbol{X}}_{i,\cdot}^{A} - \overline{\boldsymbol{X}}_{\mathcal{S}(a,1-a)} \right) \left( \overline{\boldsymbol{X}}_{i,\cdot}^{A} - \overline{\boldsymbol{X}}_{\mathcal{S}(a,1-a)} \right)^{\top} \right\}^{-1} \times \sum_{i: A_i = a} \left( \overline{\boldsymbol{X}}_{i,\cdot}^{A} - \overline{\boldsymbol{X}}_{\mathcal{S}(a,1-a)} \right) \left( \overline{W}_{i,\cdot}^{A} - \overline{W}_{\mathcal{S}(a,1-a)} \right).$$

First, consider the numerator of $\widehat{\boldsymbol{\gamma}}_{\mathrm{A},1}^{\mathrm{adj}}(a, 1-a)$. By Condition 5 in the main article,

$$\mathbb{E} \left( \frac{1}{N} \sum_{i: A_i = a} \overline{\boldsymbol{X}}_{i,\cdot}^{A} \overline{W}_{i,\cdot}^{A} \right) = \frac{\pi_a}{N} \sum_{i=1}^{N} \overline{\boldsymbol{X}}_{i,\cdot} \overline{W}_{i,\cdot}(a, 1-a) = \boldsymbol{O}(1).$$

By Condition 4 in the main article and Lemma S6,

$$\mathbb{V}\mathrm{ar} \left( \frac{1}{N} \sum_{i: A_i = a} \overline{\boldsymbol{X}}_{i,\cdot}^{A} \overline{W}_{i,\cdot}^{A} \right) = \boldsymbol{O} \left( \frac{1}{N} \right).$$

Therefore,

$$\frac{1}{N} \sum_{i: A_i = a} \overline{\boldsymbol{X}}_{i,\cdot}^{A} \overline{W}_{i,\cdot}^{A} = \frac{\pi_a}{N} \sum_{i=1}^{N} \overline{\boldsymbol{X}}_{i,\cdot} \overline{W}_{i,\cdot}(a, 1-a) + \boldsymbol{O}_{\mathbb{P}} \left( \frac{1}{N^{1/2}} \right).$$

By the proof of Lemma S8

$$\overline{\boldsymbol{X}}_{\mathcal{S}(a,1-a)} = \frac{1}{N(N-1)}\sum_{i\neq j}\boldsymbol{X}_{i,j} + \boldsymbol{O}_{\mathbb{P}}\left(\frac{1}{N^{1/2}}\right) = \boldsymbol{O}_{\mathbb{P}}\left(\frac{1}{N^{1/2}}\right)$$

$$\overline{W}_{\mathcal{S}(a,1-a)} = \frac{1}{N(N-1)}\sum_{i\neq j}W_{i,j}(a,1-a) + O_{\mathbb{P}}\left(\frac{1}{N^{1/2}}\right) = \overline{W}(a,1-a) + O_{\mathbb{P}}\left(\frac{1}{N^{1/2}}\right).$$

Therefore, the numerator and the denominator of $\widehat{\gamma}^{\text{adj}}_{\text{A},1}(a,1-a)$ satisfy

$$\frac{1}{N}\sum_{i:A_i=a}\left(\overline{\boldsymbol{X}}^{A}_{i,\cdot} - \overline{\boldsymbol{X}}_{\mathcal{S}(a,1-a)}\right)\left(\overline{W}^{A}_{i,\cdot} - \overline{W}_{\mathcal{S}(a,1-a)}\right) = \frac{\pi_a}{N}\sum_{i=1}^{N}\overline{\boldsymbol{X}}_{i,\cdot}\overline{W}_{i,\cdot}(a,1-a) + \boldsymbol{O}_{\mathbb{P}}\left(\frac{1}{N^{1/2}}\right)$$

and

$$\frac{1}{N}\sum_{i:A_i=a}\left(\overline{\boldsymbol{X}}^{A}_{i,\cdot} - \overline{\boldsymbol{X}}_{\mathcal{S}(a,1-a)}\right)\left(\overline{\boldsymbol{X}}^{A}_{i,\cdot} - \overline{\boldsymbol{X}}_{\mathcal{S}(a,1-a)}\right)^{\top} = \frac{\pi_a}{N}\sum_{i=1}^{N}\overline{\boldsymbol{X}}_{i,\cdot}\overline{\boldsymbol{X}}^{\top}_{i,\cdot} + \boldsymbol{O}_{\mathbb{P}}\left(\frac{1}{N^{1/2}}\right).$$

By Lemma S3, we have $\widehat{\gamma}^{\text{adj}}_{\text{A},1}(a,1-a) - \gamma^{\text{adj}}_{\text{A},1}(a,1-a) = \boldsymbol{O}_{\mathbb{P}}(N^{-1/2})$. The result for $\widehat{\gamma}^{\text{adj}}_{\text{A},2}(a,1-a)$ is obtained following the same argument.

## S6.10 Lemma S13

By the property of the OLS,

$$\widehat{\lambda}^{\text{adj}}_{\text{A},\mathfrak{o}}(a,1-a) = \overline{W}_{\mathcal{S}(a,1-a)} - \overline{\boldsymbol{X}}^{\top}_{\mathcal{S}(a,1-a)}\widehat{\gamma}^{\text{adj}}_{\text{A},\mathfrak{o}}(a,1-a).$$

Thus,

$$\begin{aligned}&\widehat{\lambda}^{\text{adj}}_{\text{A},\mathfrak{o}}(a,1-a) - \lambda(a,1-a)\\ &= \left\{\overline{W}_{\mathcal{S}(a,1-a)} - \lambda(a,1-a)\right\} - \overline{\boldsymbol{X}}^{\top}_{\mathcal{S}(a,1-a)}\gamma^{\text{adj}}_{\text{A},\mathfrak{o}}(a,1-a) + \overline{\boldsymbol{X}}^{\top}_{\mathcal{S}(a,1-a)}\left\{\gamma^{\text{adj}}_{\text{A},\mathfrak{o}}(a,1-a) - \widehat{\gamma}^{\text{adj}}_{\text{A},\mathfrak{o}}(a,1-a)\right\}.\end{aligned}$$

By Lemma S12, $\widehat{\gamma}^{\text{adj}}_{\text{A},\mathfrak{o}}(a,1-a) - \gamma^{\text{adj}}_{\text{A},\mathfrak{o}}(a,1-a) = \boldsymbol{O}_{\mathbb{P}}(N^{-1/2})$ and $\overline{\boldsymbol{X}}_{\mathcal{S}(a,1-a)} = \boldsymbol{O}_{\mathbb{P}}(N^{-1/2})$. Therefore,

$$\begin{aligned}\widehat{\lambda}^{\text{adj}}_{\text{A},\mathfrak{o}}(a,1-a) - \lambda(a,1-a) &= \left\{\overline{W}_{\mathcal{S}(a,1-a)} - \lambda(a,1-a)\right\} - \overline{\boldsymbol{X}}^{\top}_{\mathcal{S}(a,1-a)}\gamma^{\text{adj}}_{\text{A},\mathfrak{o}}(a,1-a) + O_{\mathbb{P}}\left(\frac{1}{N}\right)\\ &= \frac{1}{N_1N_0}\sum_{(i,j)\in\mathcal{S}(a,1-a)} r^{\text{adj}}_{\text{A},\mathfrak{o},i,j}(a,1-a) + O_{\mathbb{P}}\left(\frac{1}{N}\right)\end{aligned}$$

where

$$r^{\text{adj}}_{\text{A},\mathfrak{o},i,j}(a,1-a) = W_{i,j}(a,1-a) - \overline{W}(a,1-a) - \boldsymbol{X}^{\top}_{i,j}\gamma^{\text{adj}}_{\text{A},\mathfrak{o}}(a,1-a).$$

Hence, applying the same arguments (the Hoeffding decomposition) in the proof of Lemma S7, we have $\mathbb{V}\text{ar}\{\widehat{\lambda}^{\text{adj}}_{\text{A},\mathfrak{o}}(a,1-a)\}$, and similarly, the covariance $\mathbb{C}\text{ov}\{\widehat{\lambda}^{\text{adj}}_{\text{A},\mathfrak{o}}(a,1-a), \widehat{\lambda}^{\text{adj}}_{\text{A},\mathfrak{o}}(1-a,a)\}$. For $\mathbb{C}\text{ov}\{\widehat{\lambda}^{\text{adj}}_{\text{A},1}(a,1-a), \widehat{\lambda}^{\text{adj}}_{\text{A},2}(a,1-a)\}$, the covariance between $\widehat{\lambda}^{\text{adj}}_{\text{A},1}(a,1-a)$ and $\widehat{\lambda}^{\text{adj}}_{\text{A},2}(a,1-a)$, we have

$$\Psi^{\text{adj},*}_{\text{A},1}(a,1-a) = \frac{1}{\pi_a N}\sum_{i=1}^{N}\overline{r}^{\text{adj}}_{\text{A},1,i,\cdot}(a,1-a)\mathbb{1}_i(a) + \frac{1}{\pi_{1-a}N}\sum_{i=1}^{N}\overline{r}^{\text{adj}}_{\text{A},1,\cdot,i}(a,1-a)\mathbb{1}_i(1-a),$$

$$\Psi^{\mathrm{adj},*}_{\mathrm{A},2}(a,1-a)=\frac{1}{\pi_a N}\sum_{i=1}^{N}\overline{r}^{\mathrm{adj}}_{\mathrm{A},2,i,\cdot}(a,1-a)\mathbb{1}_i(a)+\frac{1}{\pi_{1-a}N}\sum_{i=1}^{N}\overline{r}^{\mathrm{adj}}_{\mathrm{A},2,\cdot,i}(a,1-a)\mathbb{1}_i(1-a).$$

Thus, the leading term of $N\mathbb{C}\mathrm{ov}\{\widehat{\lambda}^{\mathrm{adj}}_{\mathrm{A},1}(a,1-a),\widehat{\lambda}^{\mathrm{adj}}_{\mathrm{A},2}(a,1-a)\}$ is

$$\begin{aligned}
&\left(\frac{1}{N_a}-\frac{1}{N}\right)\sum_{i=1}^{N}\overline{r}^{\mathrm{adj}}_{\mathrm{A},1,i,\cdot}(a,1-a)\overline{r}^{\mathrm{adj}}_{\mathrm{A},2,i,\cdot}(a,1-a)+\left(\frac{1}{N_{1-a}}-\frac{1}{N}\right)\sum_{i=1}^{N}\overline{r}^{\mathrm{adj}}_{\mathrm{A},1,\cdot,i}(a,1-a)\overline{r}^{\mathrm{adj}}_{\mathrm{A},2,\cdot,i}(a,1-a)\\
&\quad-\frac{1}{N}\sum_{i=1}^{N}\overline{r}^{\mathrm{adj}}_{\mathrm{A},1,i,\cdot}(a,1-a)\overline{r}^{\mathrm{adj}}_{\mathrm{A},2,\cdot,i}(a,1-a)-\frac{1}{N}\sum_{i=1}^{N}\overline{r}^{\mathrm{adj}}_{\mathrm{A},2,i,\cdot}(a,1-a)\overline{r}^{\mathrm{adj}}_{\mathrm{A},1,\cdot,i}(a,1-a)\\
&=\frac{1}{\pi_a N}\sum_{i=1}^{N}\overline{r}^{\mathrm{adj}}_{\mathrm{A},1,i,\cdot}(a,1-a)\overline{r}^{\mathrm{adj}}_{\mathrm{A},2,i,\cdot}(a,1-a)+\frac{1}{\pi_{1-a}N}\sum_{i=1}^{N}\overline{r}^{\mathrm{adj}}_{\mathrm{A},1,\cdot,i}(a,1-a)\overline{r}^{\mathrm{adj}}_{\mathrm{A},2,\cdot,i}(a,1-a)\\
&\quad-\frac{1}{N}\sum_{i=1}^{N}\left\{\overline{r}^{\mathrm{adj}}_{\mathrm{A},1,i,\cdot}(a,1-a)+\overline{r}^{\mathrm{adj}}_{\mathrm{A},1,\cdot,i}(a,1-a)\right\}\left\{\overline{r}^{\mathrm{adj}}_{\mathrm{A},2,i,\cdot}(a,1-a)+\overline{r}^{\mathrm{adj}}_{\mathrm{A},2,\cdot,i}(a,1-a)\right\}.
\end{aligned}$$

## S6.11 Lemma S14

We derive the probability limit of $\widehat{\gamma}^{\mathrm{acv}}_{\mathrm{A},1}$. The convergence proof follows that of Lemma S12 and is thus omitted. Same as $\widehat{\gamma}^{\mathrm{acv}}_{\mathrm{I}}$, we can obtain $\widehat{\gamma}^{\mathrm{acv}}_{\mathrm{A},1}$ by Frisch-Waugh-Lovell. The residual from the OLS fit of $\overline{W}^{A}_{i,\cdot}$ on $(A_i,1-A_i)$ is

$$\overline{W}^{A,\mathrm{acv}}_{i,\cdot}=\overline{W}^{A}_{i,\cdot}-A_i\overline{W}_{\mathcal{S}(1,0)}-(1-A_i)\overline{W}_{\mathcal{S}(0,1)},$$

and the residual from the OLS fit of $\overline{\boldsymbol{X}}^{A}_{i,\cdot}$ on $(A_i,1-A_i)$ is

$$\overline{\boldsymbol{X}}^{A,\mathrm{acv}}_{i,\cdot}=\overline{\boldsymbol{X}}^{A}_{i,\cdot}-A_i\overline{\boldsymbol{X}}_{\mathcal{S}(1,0)}-(1-A_i)\overline{\boldsymbol{X}}_{\mathcal{S}(0,1)}.$$

Therefore,

$$\widehat{\gamma}^{\mathrm{acv}}_{\mathrm{A},1}=\left(\sum_{i=1}^{N}\overline{\boldsymbol{X}}^{A,\mathrm{acv}}_{i,\cdot}\overline{\boldsymbol{X}}^{A,\mathrm{acv}\top}_{i,\cdot}\right)^{-1}\sum_{i=1}^{N}\overline{\boldsymbol{X}}^{A,\mathrm{acv}}_{i,\cdot}\overline{W}^{A,\mathrm{acv}}_{i,\cdot}.$$

By Lemma S6, the numerator of $\widehat{\gamma}^{\mathrm{acv}}_{\mathrm{A},1}$ satisfies

$$\begin{aligned}
&\frac{1}{N}\sum_{i=1}^{N}\overline{\boldsymbol{X}}^{A,\mathrm{acv}}_{i,\cdot}\overline{W}^{A,\mathrm{acv}}_{i,\cdot}\\
&=\frac{1}{N}\sum_{i:A_i=1}\left(\overline{\boldsymbol{X}}^{A}_{i,\cdot}-\overline{\boldsymbol{X}}_{\mathcal{S}(1,0)}\right)\left(\overline{W}^{A}_{i,\cdot}-\overline{W}_{\mathcal{S}(1,0)}\right)+\frac{1}{N}\sum_{i:A_i=0}\left(\overline{\boldsymbol{X}}^{A}_{i,\cdot}-\overline{\boldsymbol{X}}_{\mathcal{S}(0,1)}\right)\left(\overline{W}^{A}_{i,\cdot}-\overline{W}_{\mathcal{S}(0,1)}\right)\\
&=\frac{1}{N}\sum_{i:A_i=1}\overline{\boldsymbol{X}}^{A}_{i,\cdot}\overline{W}^{A}_{i,\cdot}-\frac{N_1}{N}\overline{\boldsymbol{X}}_{\mathcal{S}(1,0)}\overline{W}_{\mathcal{S}(1,0)}+\frac{1}{N}\sum_{i:A_i=0}\overline{\boldsymbol{X}}^{A}_{i,\cdot}\overline{W}^{A}_{i,\cdot}-\frac{N_0}{N}\overline{\boldsymbol{X}}_{\mathcal{S}(0,1)}\overline{W}_{\mathcal{S}(0,1)}\\
&=\frac{\pi_1}{N}\sum_{i=1}^{N}\overline{\boldsymbol{X}}_{i,\cdot}\overline{W}_{i,\cdot}(1,0)+\frac{\pi_0}{N}\sum_{i=1}^{N}\overline{\boldsymbol{X}}_{i,\cdot}\overline{W}_{i,\cdot}(0,1)+\boldsymbol{O}_{\mathbb{P}}\left(\frac{1}{N^{1/2}}\right).
\end{aligned}$$

Its denominator satisfies

$$\frac{1}{N}\sum_{i=1}^{N}\overline{\boldsymbol{X}}^{A,\mathrm{acv}}_{i,\cdot}\overline{\boldsymbol{X}}^{A,\mathrm{acv}\top}_{i,\cdot}=\frac{1}{N}\sum_{i=1}^{N}\overline{\boldsymbol{X}}_{i,\cdot}\overline{\boldsymbol{X}}^{\top}_{i,\cdot}+\boldsymbol{O}_{\mathbb{P}}\left(\frac{1}{N^{1/2}}\right).$$

By Lemma S3,

$$\widehat{\gamma}^{\text{acv}}_{\text{A},1} = \pi_1 \boldsymbol{\gamma}^{\text{adj}}_{\text{A},1}(1,0) + \pi_0 \boldsymbol{\gamma}^{\text{adj}}_{\text{A},1}(0,1) + \boldsymbol{O}_{\mathbb{P}}\left(\frac{1}{N^{1/2}}\right).$$

Results for $\widehat{\gamma}^{\text{acv}}_{\text{A},2}$ can be obtained following the same arguments.

## S6.12 Lemma S16

We derive the finite-population probability limits. The convergence proof follows that of Lemma S8 and is thus omitted. For $\widehat{\gamma}^{\text{acv}}_{\text{P},W}$, we have

$$\widehat{\gamma}^{\text{acv}}_{\text{P},W} = \left(\sum_{i\neq j} \boldsymbol{X}_{i,j}\boldsymbol{X}_{i,j}^\top\right)^{-1} \sum_{i\neq j} \boldsymbol{X}_{i,j} W_{i,j}.$$

Then,

$$\begin{aligned}
\gamma^{\text{acv}}_{\text{P},W} &= \mathbb{E}(\widehat{\gamma}^{\text{acv}}_{\text{P},W}) = \left(\sum_{i\neq j} \boldsymbol{X}_{i,j}\boldsymbol{X}_{i,j}^\top\right)^{-1} \sum_{i\neq j} \boldsymbol{X}_{i,j}\mathbb{E}\{W_{i,j}(A_i,A_j)\} \\
&= \left\{\frac{1}{N(N-1)}\sum_{i\neq j} \boldsymbol{X}_{i,j}\boldsymbol{X}_{i,j}^\top\right\}^{-1} \frac{1}{N(N-1)}\sum_{i\neq j} \boldsymbol{X}_{i,j}\mathbb{E}\{W_{i,j}(A_i,A_j)\} = \boldsymbol{O}(1)\boldsymbol{O}(1) = \boldsymbol{O}(1).
\end{aligned}$$

For $\widehat{\gamma}^{\text{acv}}_{\text{P},D}$, we have

$$\widehat{\gamma}^{\text{acv}}_{\text{P},D} = \left(\sum_{i\neq j} \boldsymbol{X}_{i,j}\boldsymbol{X}_{i,j}^\top\right)^{-1} \sum_{i\neq j} \boldsymbol{X}_{i,j} D_{i,j}.$$

Then,

$$\gamma^{\text{acv}}_{\text{P},D} = \mathbb{E}(\widehat{\gamma}^{\text{acv}}_{\text{P},D}) = \left(\sum_{i\neq j} \boldsymbol{X}_{i,j}\boldsymbol{X}_{i,j}^\top\right)^{-1} \sum_{i\neq j} \boldsymbol{X}_{i,j}\mathbb{E}(D_{i,j}) = \boldsymbol{O}(1)\cdot 0 = \boldsymbol{0} = \boldsymbol{o}(1).$$

For $\widehat{\gamma}^{\text{int}}_{\text{P},W}$, we have

$$\begin{aligned}
\widehat{\gamma}^{\text{int}}_{\text{P},W} &= \left\{\sum_{(i,j)\in\mathcal{S}} \boldsymbol{X}_{i,j}\boldsymbol{X}_{i,j}^\top\right\}^{-1} \left\{\sum_{(i,j)\in\mathcal{S}(a,1-a)} \boldsymbol{X}_{i,j}W_{i,j}(a,1-a) - \sum_{(i,j)\in\mathcal{S}(1-a,a)} \boldsymbol{X}_{i,j}W_{i,j}(1-a)\right\} \\
&= \left\{\frac{1}{2N_1N_0}\sum_{(i,j)\in\mathcal{S}} \boldsymbol{X}_{i,j}\boldsymbol{X}_{i,j}^\top\right\}^{-1} \\
&\quad \times \left\{\frac{1}{2N_1N_0}\sum_{(i,j)\in\mathcal{S}(a,1-a)} \boldsymbol{X}_{i,j}W_{i,j}(a,1-a) - \frac{1}{2N_1N_0}\sum_{(i,j)\in\mathcal{S}(1-a,a)} \boldsymbol{X}_{i,j}W_{i,j}(1-a)\right\} \\
&= \left\{\frac{1}{N(N-1)}\sum_{i\neq j} \boldsymbol{X}_{i,j}\boldsymbol{X}_{i,j}^\top\right\}^{-1}
\end{aligned}$$

$$\times \left\{ \frac{1}{2N(N-1)} \sum_{i \neq j} \boldsymbol{X}_{i,j} W_{i,j}(a, 1-a) - \frac{1}{2N(N-1)} \sum_{i \neq j} \boldsymbol{X}_{i,j} W_{i,j}(1-a) \right\} + \boldsymbol{o}_{\mathbb{P}}(1)$$

$$= \boldsymbol{O}(1)\boldsymbol{O}(1) + \boldsymbol{o}_{\mathbb{P}}(1) = \boldsymbol{O}(1) + \boldsymbol{o}_{\mathbb{P}}(1).$$

Then, $\boldsymbol{\gamma}^{\text{int}}_{\text{P},W} = \boldsymbol{O}(1)$. For $\widehat{\boldsymbol{\gamma}}^{\text{int}}_{\text{P},D}$, we have

$$\begin{aligned}
\widehat{\boldsymbol{\gamma}}^{\text{int}}_{\text{P},D} &= \left\{ \sum_{(i,j)\in\mathcal{S}} \boldsymbol{X}_{i,j}\boldsymbol{X}_{i,j}^\top \right\}^{-1} \sum_{(i,j)\in\mathcal{S}} \boldsymbol{X}_{i,j} \\
&= \left\{ \frac{1}{2N_1N_0} \sum_{(i,j)\in\mathcal{S}} \boldsymbol{X}_{i,j}\boldsymbol{X}_{i,j}^\top \right\}^{-1} \left\{ \frac{1}{2N_1N_0} \sum_{(i,j)\in\mathcal{S}} \boldsymbol{X}_{i,j} \right\} \\
&= \left\{ \frac{1}{N(N-1)} \sum_{i\neq j} \boldsymbol{X}_{i,j}\boldsymbol{X}_{i,j}^\top \right\}^{-1} \left\{ \frac{1}{N(N-1)} \sum_{i\neq j} \boldsymbol{X}_{i,j} \right\} + \boldsymbol{o}_{\mathbb{P}}(1) \\
&= \boldsymbol{O}(1)\cdot\boldsymbol{0} + \boldsymbol{o}_{\mathbb{P}}(1) = \boldsymbol{0} + \boldsymbol{o}_{\mathbb{P}}(1) = \boldsymbol{o}_{\mathbb{P}}(1).
\end{aligned}$$

Then, $\boldsymbol{\gamma}^{\text{int}}_{\text{P},D} = \boldsymbol{o}(1)$. Let

$$\begin{aligned}
&\boldsymbol{\Delta} \\
&= \frac{1}{N(N-1)} \begin{pmatrix} \sum_{i\neq j} \boldsymbol{X}_{i,j}\boldsymbol{X}_{i,j}^\top & \sum_{(i,j)\in\mathcal{S}(a,1-a)} \boldsymbol{X}_{i,j}\boldsymbol{X}_{i,j}^\top - \sum_{(i,j)\in\mathcal{S}(1-a,a)} \boldsymbol{X}_{i,j}\boldsymbol{X}_{i,j}^\top \\ \sum_{(i,j)\in\mathcal{S}(a,1-a)} \boldsymbol{X}_{i,j}\boldsymbol{X}_{i,j}^\top - \sum_{(i,j)\in\mathcal{S}(1-a,a)} \boldsymbol{X}_{i,j}\boldsymbol{X}_{i,j}^\top & \sum_{(i,j)\in\mathcal{S}(a,1-a)} \boldsymbol{X}_{i,j}\boldsymbol{X}_{i,j}^\top + \sum_{(i,j)\in\mathcal{S}(1-a,a)} \boldsymbol{X}_{i,j}\boldsymbol{X}_{i,j}^\top \end{pmatrix} \\
&= \frac{1}{N(N-1)} \begin{pmatrix} \sum_{i\neq j} \boldsymbol{X}_{i,j}\boldsymbol{X}_{i,j}^\top & \boldsymbol{0} \\ \boldsymbol{0} & 2\pi_1\pi_0 \sum_{i\neq j} \boldsymbol{X}_{i,j}\boldsymbol{X}_{i,j}^\top \end{pmatrix} + \boldsymbol{o}_{\mathbb{P}}(1) = \boldsymbol{O}(1) + \boldsymbol{o}_{\mathbb{P}}(1).
\end{aligned}$$

Then, by Lemma S3,

$$\begin{aligned}
\begin{pmatrix} \widehat{\boldsymbol{\gamma}}^{\text{adj},W}_{\text{P},X} \\ \widehat{\boldsymbol{\gamma}}^{\text{adj},W}_{\text{P},DX} \end{pmatrix} &= \boldsymbol{\Delta}^{-1} \frac{1}{N(N-1)} \begin{pmatrix} \sum_{i\neq j} \boldsymbol{X}_{i,j} W_{i,j} \\ \sum_{(i,j)\in\mathcal{S}(a,1-a)} \boldsymbol{X}_{i,j} W_{i,j} - \sum_{(i,j)\in\mathcal{S}(1-a,a)} \boldsymbol{X}_{i,j} W_{i,j} \end{pmatrix} \\
&= \boldsymbol{\Delta}^{-1} \frac{1}{N(N-1)} \begin{pmatrix} \sum_{i\neq j} \boldsymbol{X}_{i,j} \mathbb{E}\{W_{i,j}(A_i, A_j)\} \\ \pi_1\pi_0 \sum_{i\neq j} \boldsymbol{X}_{i,j}\{W_{i,j}(a,1-a) - W_{i,j}(1-a,a)\} \end{pmatrix} + \boldsymbol{o}_{\mathbb{P}}(1) \\
&= \{\boldsymbol{O}(1) + \boldsymbol{o}_{\mathbb{P}}(1)\}\boldsymbol{O}(1) + \boldsymbol{o}_{\mathbb{P}}(1) = \boldsymbol{O}_{\mathbb{P}}(1).
\end{aligned}$$

Also, by Lemma S3,

$$\begin{pmatrix} \widehat{\boldsymbol{\gamma}}^{\text{adj},D}_{\text{P},X} \\ \widehat{\boldsymbol{\gamma}}^{\text{adj},D}_{\text{P},DX} \end{pmatrix} = \boldsymbol{\Delta}^{-1} \frac{1}{N(N-1)} \begin{pmatrix} \sum_{(i,j)\in\mathcal{S}(a,1-a)} \boldsymbol{X}_{i,j} - \sum_{(i,j)\in\mathcal{S}(1-a,a)} \boldsymbol{X}_{i,j} \\ \sum_{(i,j)\in\mathcal{S}(a,1-a)} \boldsymbol{X}_{i,j} + \sum_{(i,j)\in\mathcal{S}(1-a,a)} \boldsymbol{X}_{i,j} \end{pmatrix}$$

$$
= \boldsymbol{\Delta}^{-1} \frac{1}{N(N-1)} \begin{pmatrix} \pi_1\pi_0 \sum_{i\neq j} \boldsymbol{X}_{i,j} - \pi_1\pi_0 \sum_{i\neq j} \boldsymbol{X}_{i,j} \\ \pi_1\pi_0 \sum_{i\neq j} \boldsymbol{X}_{i,j} + \pi_1\pi_0 \sum_{i\neq j} \boldsymbol{X}_{i,j} \end{pmatrix} + \boldsymbol{o}_{\mathbb{P}}(1)
$$

$$
= \{\boldsymbol{O}(1) + \boldsymbol{o}_{\mathbb{P}}(1)\} \cdot \boldsymbol{0} + \boldsymbol{o}_{\mathbb{P}}(1) = \boldsymbol{o}_{\mathbb{P}}(1).
$$

It can be easily observed that $\boldsymbol{\gamma}_{\mathrm{P},X}^{\mathrm{adj},W} = \boldsymbol{\gamma}_{\mathrm{P},W}^{\mathrm{acv}} = \boldsymbol{\gamma}_{\mathrm{I}}^{\mathrm{acv}}$ and $\boldsymbol{\gamma}_{\mathrm{P},DX}^{\mathrm{adj},W} = \boldsymbol{\gamma}_{\mathrm{P},W}^{\mathrm{int}}$.

## S6.13 Lemma S17

First, we prove (S3). By the definition of $\widehat{r}_{\mathrm{I},i,j}^{\mathrm{adj}}$,

$$
\frac{1}{N(N-1)} \sum_{i\neq j} A_i(1-A_j)(\widehat{r}_{\mathrm{I},i,j}^{\mathrm{adj}})^2
$$

$$
= \frac{1}{N(N-1)} \sum_{i\neq j} A_i(1-A_j) \left\{ W_{i,j}(1,0) - \overline{W}_{\mathcal{S}(1,0)} - \left(\boldsymbol{X}_{i,j} - \overline{\boldsymbol{X}}_{\mathcal{S}(1,0)}\right)^\top \widehat{\boldsymbol{\gamma}}_{\mathrm{I}}^{\mathrm{adj}}(1,0) \right\}^2
$$

$$
= \frac{1}{N(N-1)} \sum_{i\neq j} A_i(1-A_j) \left\{ r_{\mathrm{I},i,j}^{\mathrm{adj}}(1,0) + \boldsymbol{X}_{i,j}^\top \boldsymbol{\gamma}_{\mathrm{I}}^{\mathrm{adj}}(1,0) - \bar{\epsilon}_{\mathcal{S}(1,0)} - \left(\boldsymbol{X}_{i,j} - \overline{\boldsymbol{X}}_{\mathcal{S}(1,0)}\right)^\top \widehat{\boldsymbol{\gamma}}_{\mathrm{I}}^{\mathrm{adj}}(1,0) \right\}^2
$$

$$
= \frac{1}{N(N-1)} \sum_{i\neq j} A_i(1-A_j) \left[ r_{\mathrm{I},i,j}^{\mathrm{adj}}(1,0) + \boldsymbol{X}_{i,j}^\top \left\{ \boldsymbol{\gamma}_{\mathrm{I}}^{\mathrm{adj}}(1,0) - \widehat{\boldsymbol{\gamma}}_{\mathrm{I}}^{\mathrm{adj}}(1,0) \right\} - \left\{ \bar{\epsilon}_{\mathcal{S}(1,0)} - \overline{\boldsymbol{X}}_{\mathcal{S}(1,0)}^\top \widehat{\boldsymbol{\gamma}}_{\mathrm{I}}^{\mathrm{adj}}(1,0) \right\} \right]^2
$$

$$
= T_{\mathrm{HR},1} + T_{\mathrm{HR},2} + T_{\mathrm{HR},3} + T_{\mathrm{HR},4} - T_{\mathrm{HR},5} - T_{\mathrm{HR},6},
$$

where

$$
T_{\mathrm{HR},1} = \frac{1}{N(N-1)} \sum_{i\neq j} A_i(1-A_j) r_{\mathrm{I},i,j}^{\mathrm{adj}}(1,0)^2,
$$

$$
T_{\mathrm{HR},2} = \frac{1}{N(N-1)} \sum_{i\neq j} A_i(1-A_j) \left[ \boldsymbol{X}_{i,j}^\top \left\{ \boldsymbol{\gamma}_{\mathrm{I}}^{\mathrm{adj}}(1,0) - \widehat{\boldsymbol{\gamma}}_{\mathrm{I}}^{\mathrm{adj}}(1,0) \right\} \right]^2,
$$

$$
T_{\mathrm{HR},3} = \frac{1}{N(N-1)} \sum_{i\neq j} A_i(1-A_j) \left\{ \bar{\epsilon}_{\mathcal{S}(1,0)} - \overline{\boldsymbol{X}}_{\mathcal{S}(1,0)}^\top \widehat{\boldsymbol{\gamma}}_{\mathrm{I}}^{\mathrm{adj}}(1,0) \right\}^2
$$

$$
T_{\mathrm{HR},4} = \frac{2}{N(N-1)} \sum_{i\neq j} A_i(1-A_j) r_{\mathrm{I},i,j}^{\mathrm{adj}}(1,0) \boldsymbol{X}_{i,j}^\top \left\{ \boldsymbol{\gamma}_{\mathrm{I}}^{\mathrm{adj}}(1,0) - \widehat{\boldsymbol{\gamma}}_{\mathrm{I}}^{\mathrm{adj}}(1,0) \right\},
$$

$$
T_{\mathrm{HR},5} = \frac{2}{N(N-1)} \sum_{i\neq j} A_i(1-A_j) r_{\mathrm{I},i,j}^{\mathrm{adj}}(1,0) \left\{ \bar{\epsilon}_{\mathcal{S}(1,0)} - \overline{\boldsymbol{X}}_{\mathcal{S}(1,0)}^\top \widehat{\boldsymbol{\gamma}}_{\mathrm{I}}^{\mathrm{adj}}(1,0) \right\},
$$

$$
T_{\mathrm{HR},6} = \frac{2}{N(N-1)} \sum_{i\neq j} A_i(1-A_j) \boldsymbol{X}_{i,j}^\top \left\{ \boldsymbol{\gamma}_{\mathrm{I}}^{\mathrm{adj}}(1,0) - \widehat{\boldsymbol{\gamma}}_{\mathrm{I}}^{\mathrm{adj}}(1,0) \right\} \left\{ \bar{\epsilon}_{\mathcal{S}(1,0)} - \overline{\boldsymbol{X}}_{\mathcal{S}(1,0)}^\top \widehat{\boldsymbol{\gamma}}_{\mathrm{I}}^{\mathrm{adj}}(1,0) \right\}.
$$

Except for $T_{\mathrm{HR},1}$, all other terms are $o_{\mathbb{P}}(1)$. We show that $T_{\mathrm{HR},4} = o_{\mathbb{P}}(1)$ and omit the proofs for other terms. Specifically,

$$
|T_{\mathrm{HR},4}| \leq \frac{2}{N(N-1)} \sum_{i\neq j} \left\| r_{\mathrm{I},i,j}^{\mathrm{adj}}(1,0) \boldsymbol{X}_{i,j} \right\| \left\| \boldsymbol{\gamma}_{\mathrm{I}}^{\mathrm{adj}}(1,0) - \widehat{\boldsymbol{\gamma}}_{\mathrm{I}}^{\mathrm{adj}}(1,0) \right\|
$$

$$
\leq \frac{2}{N(N-1)} \sum_{i\neq j} \left\{ r_{\mathrm{I},i,j}^{\mathrm{adj}}(1,0)^2 + \|\boldsymbol{X}_{i,j}\|^2 \right\} \left\| \boldsymbol{\gamma}_{\mathrm{I}}^{\mathrm{adj}}(1,0) - \widehat{\boldsymbol{\gamma}}_{\mathrm{I}}^{\mathrm{adj}}(1,0) \right\|
$$

By Lemma S8, $\|\gamma_{\mathrm{I}}^{\mathrm{adj}}(1,0)-\widehat{\gamma}_{\mathrm{I}}^{\mathrm{adj}}(1,0)\| = O_{\mathbb{P}}(N^{-1/2})$, and under Conditions 2 and 3 in the main article,

$$\frac{1}{N(N-1)}\sum_{i\neq j} r_{\mathrm{I},i,j}^{\mathrm{adj}}(1,0)^2 = O(1), \quad \frac{1}{N(N-1)}\sum_{i\neq j}\|\boldsymbol{X}_{i,j}\|^2 = O(1).$$

Therefore, $|T_{\mathrm{HR},4}| \le O(1)O_{\mathbb{P}}(N^{-1/2}) = o_{\mathbb{P}}(1)$. To finish the proof of (S3), we only need to verify that $T_{\mathrm{HR},1}$ differs from its mean by a term of $o_{\mathbb{P}}(1)$. By Lemma S5, $\mathbb{V}\mathrm{ar}(T_{\mathrm{HR},1}) = o(1)$, and the result follows from Chebyshev's inequality.

Second, we prove (S4). By the definition of $\widehat{r}_{\mathrm{I},i,j}^{\mathrm{adj}}$,

$$\begin{aligned}
&\frac{1}{N(N-1)}\sum_{i\neq j} A_i(1-A_j)\boldsymbol{X}_{i,j}^{\top}(\widehat{r}_{\mathrm{I},i,j}^{\mathrm{adj}})^2\\
&= \frac{1}{N(N-1)}\sum_{i\neq j} A_i(1-A_j)\boldsymbol{X}_{i,j}^{\top}\left[\epsilon_{i,j}(1,0) - \boldsymbol{X}_{i,j}^{\top}\widehat{\gamma}_{\mathrm{I}}^{\mathrm{adj}}(1,0) - \left\{\overline{\epsilon}_{\mathcal{S}(1,0)} - \overline{\boldsymbol{X}}_{\mathcal{S}(1,0)}^{\top}\widehat{\gamma}_{\mathrm{I}}^{\mathrm{adj}}(1,0)\right\}\right]^2\\
&= \boldsymbol{T}_{\mathrm{HR},7} + \boldsymbol{T}_{\mathrm{HR},8} + \boldsymbol{T}_{\mathrm{HR},9} - \boldsymbol{T}_{\mathrm{HR},10} - \boldsymbol{T}_{\mathrm{HR},11} + \boldsymbol{T}_{\mathrm{HR},12},
\end{aligned}$$

where

$$\begin{aligned}
\boldsymbol{T}_{\mathrm{HR},7} &= \frac{1}{N(N-1)}\sum_{i\neq j} A_i(1-A_j)\boldsymbol{X}_{i,j}^{\top}\epsilon_{i,j}(1,0)^2,\\
\boldsymbol{T}_{\mathrm{HR},8} &= \frac{1}{N(N-1)}\sum_{i\neq j} A_i(1-A_j)\boldsymbol{X}_{i,j}^{\top}\left\{\boldsymbol{X}_{i,j}^{\top}\widehat{\gamma}_{\mathrm{I}}^{\mathrm{adj}}(1,0)\right\}^2,\\
\boldsymbol{T}_{\mathrm{HR},9} &= \frac{1}{N(N-1)}\sum_{i\neq j} A_i(1-A_j)\boldsymbol{X}_{i,j}^{\top}\left\{\overline{\epsilon}_{\mathcal{S}(1,0)} - \overline{\boldsymbol{X}}_{\mathcal{S}(1,0)}^{\top}\widehat{\gamma}_{\mathrm{I}}^{\mathrm{adj}}(1,0)\right\}^2,\\
\boldsymbol{T}_{\mathrm{HR},10} &= \frac{2}{N(N-1)}\sum_{i\neq j} A_i(1-A_j)\boldsymbol{X}_{i,j}^{\top}\epsilon_{i,j}(1,0),\\
\boldsymbol{T}_{\mathrm{HR},11} &= \frac{2}{N(N-1)}\sum_{i\neq j} A_i(1-A_j)\boldsymbol{X}_{i,j}^{\top}\epsilon_{i,j}(1,0)\left\{\overline{\epsilon}_{\mathrm{N},\mathcal{S}(1,0)} - \overline{\boldsymbol{X}}_{\mathcal{S}(1,0)}^{\top}\widehat{\gamma}_{\mathrm{I}}^{\mathrm{adj}}(1,0)\right\},\\
\boldsymbol{T}_{\mathrm{HR},12} &= \frac{2}{N(N-1)}\sum_{i\neq j} A_i(1-A_j)\boldsymbol{X}_{i,j}^{\top}\left\{\boldsymbol{X}_{i,j}^{\top}\widehat{\gamma}_{\mathrm{I}}^{\mathrm{adj}}(1,0)\right\}\left\{\overline{\epsilon}_{\mathcal{S}(1,0)} - \overline{\boldsymbol{X}}_{\mathcal{S}(1,0)}^{\top}\widehat{\gamma}_{\mathrm{I}}^{\mathrm{adj}}(1,0)\right\}.
\end{aligned}$$

All terms $\boldsymbol{T}_{\mathrm{HR},7}$ to $\boldsymbol{T}_{\mathrm{HR},12}$ are $\boldsymbol{O}_{\mathbb{P}}(1)$. We prove that $\boldsymbol{T}_{\mathrm{HR},7} = \boldsymbol{O}_{\mathbb{P}}(1)$ and omit the proofs for other terms. Specifically, under Condition 2 in the main article,

$$\|\boldsymbol{T}_{\mathrm{HR},7}\| \le \frac{1}{N(N-1)}\sum_{i\neq j}\|\boldsymbol{X}_{i,j}\|\,\epsilon_{i,j}(1,0)^2 \le \frac{1}{N(N-1)}\sum_{i\neq j}\left\{\|\boldsymbol{X}_{i,j}\|^2 + \epsilon_{i,j}(1,0)^4\right\} \le O(1) + O(1).$$

Therefore, (S4) holds. The proof of (S5) is similar to that of (S4), and is thus omitted.

## S6.14 Lemma S18

By definition,

$$\mathbf{Z}_{\mathrm{I},i}^{\mathrm{adj}} = \begin{pmatrix} A_i(1-A_j)\mathbf{1}_{N-1} & (1-A_i)A_j\mathbf{1}_{N-1} & A_i(1-A_j)\mathbf{X}_i & (1-A_i)A_j\mathbf{X}_i \end{pmatrix},$$

where $\mathbf{1}_{N-1}$ is an $(N-1)$ vector of ones, and $\mathbf{X}_i$ is a matrix formed by stacking $\boldsymbol{X}_{i,j}^{\top}$ for $j \neq i$. Let

$$\boldsymbol{v}_i = \sum_{j:j\neq i} \boldsymbol{Z}_{\mathrm{I},i,j}^{\mathrm{adj}\top}\widehat{r}_{\mathrm{I},i,j}^{\mathrm{adj}} = \begin{pmatrix} v_{1,i} & v_{2,i} & \boldsymbol{v}_{3,i}^{\top} & \boldsymbol{v}_{4,i}^{\top}\end{pmatrix}^{\top},$$

where

$$v_{1,i} = \sum_{j:j\neq i} A_i(1-A_j)\widehat{r}^{\text{adj}}_{\text{I},i,j} = A_i U^{\text{adj}}_{\text{I,CR},i}(0), \quad v_{2,i} = \sum_{j:j\neq i}(1-A_i)A_j\widehat{r}^{\text{adj}}_{\text{I},i,j} = (1-A_i)U^{\text{adj}}_{\text{I,CR},i}(1),$$
$$\boldsymbol{v}_{3,i} = \sum_{j:j\neq i} A_i(1-A_j)\boldsymbol{X}_{i,j}\widehat{r}^{\text{adj}}_{\text{I},i,j} = A_i \boldsymbol{L}^{\text{adj}}_{\text{I,CR},i}(0), \quad \boldsymbol{v}_{4,i} = \sum_{j:j\neq i}(1-A_i)A_j\boldsymbol{X}_{i,j}\widehat{r}^{\text{adj}}_{\text{I},i,j} = (1-A_i)\boldsymbol{L}^{\text{adj}}_{\text{I,CR},i}(1).$$

Then,

$$\mathbf{M}^{\text{adj}}_{\text{I,CR},i} = \mathbf{Z}^{\text{adj}\top}_{\text{I},i}\widehat{\mathbf{R}}^{\text{adj}}_i\mathbf{Z}^{\text{adj}}_{\text{I},i} = \boldsymbol{v}_i\boldsymbol{v}_i^\top = \begin{pmatrix} v_{1,i}^2 & v_{1,i}v_{2,i} & v_{1,i}\boldsymbol{v}_{3,i}^\top & v_{1,i}\boldsymbol{v}_{4,i}^\top \\ v_{2,i}v_{1,i} & v_{2,i}^2 & v_{2,i}\boldsymbol{v}_{3,i}^\top & v_{2,i}\boldsymbol{v}_{4,i}^\top \\ \boldsymbol{v}_{3,i}v_{1,i} & \boldsymbol{v}_{3,i}v_{2,i} & \boldsymbol{v}_{3,i}\boldsymbol{v}_{3,i}^\top & \boldsymbol{v}_{3,i}\boldsymbol{v}_{4,i}^\top \\ \boldsymbol{v}_{4,i}v_{1,i} & \boldsymbol{v}_{4,i}v_{2,i} & \boldsymbol{v}_{4,i}\boldsymbol{v}_{3,i}^\top & \boldsymbol{v}_{4,i}\boldsymbol{v}_{4,i}^\top \end{pmatrix}.$$

Plugging in the expressions, we have

$$\begin{aligned}
&\mathbf{M}^{\text{adj}}_{\text{I,CR},i} = \mathbf{Z}^{\text{adj}\top}_{\text{I},i}\widehat{\mathbf{R}}^{\text{adj}}_i\mathbf{Z}^{\text{adj}}_{\text{I},i} \\
&= \begin{pmatrix} A_iU^{\text{adj}}_{\text{I,CR},i}(0)^2 & 0 & A_iU^{\text{adj}}_{\text{I,CR},i}(0)\boldsymbol{L}^{\text{adj}}_{\text{I,CR},i}(0)^\top & \mathbf{0} \\ 0 & (1-A_i)U^{\text{adj}}_{\text{I,CR},i}(1)^2 & \mathbf{0} & (1-A_i)U^{\text{adj}}_{\text{I,CR},i}(1)\boldsymbol{L}^{\text{adj}}_{\text{I,CR},i}(1)^\top \\ A_iU^{\text{adj}}_{\text{I,CR},i}(0)\boldsymbol{L}^{\text{adj}}_{\text{I,CR},i}(0) & \mathbf{0} & A_i\boldsymbol{L}^{\text{adj}}_{\text{I,CR},i}(0)\boldsymbol{L}^{\text{adj}}_{\text{I,CR},i}(0)^\top & \mathbf{0} \\ \mathbf{0} & (1-A_i)U^{\text{adj}}_{\text{I,CR},i}(1)\boldsymbol{L}^{\text{adj}}_{\text{I,CR},i}(1) & \mathbf{0} & (1-A_i)\boldsymbol{L}^{\text{adj}}_{\text{I,CR},i}(1)\boldsymbol{L}^{\text{adj}}_{\text{I,CR},i}(1)^\top \end{pmatrix}.
\end{aligned}$$

## S6.15 Lemma S19

First, we prove (S7). By the definition of $\widehat{r}^{\text{adj}}_{\text{I},i,j}$,

$$\begin{aligned}
&\frac{1}{N(N-1)^2}\sum_{i=1}^N A_i\left\{\sum_{j:j\neq i}(1-A_j)\widehat{r}^{\text{adj}}_{\text{I},i,j}\right\}^2 \\
&= \frac{1}{N(N-1)^2}\sum_{i=1}^N A_i\left[\sum_{j:j\neq i}(1-A_j)\left\{W_{i,j}(1,0) - \overline{W}_{\mathcal{S}(1,0)} - \left(\boldsymbol{X}_{i,j} - \overline{\boldsymbol{X}}_{\mathcal{S}(1,0)}\right)^\top\widehat{\boldsymbol{\gamma}}^{\text{adj}}_{\text{I}}(1,0)\right\}\right]^2 \\
&= \frac{1}{N(N-1)^2}\sum_{i=1}^N A_i\left[\sum_{j:j\neq i}(1-A_j)\left\{r^{\text{adj}}_{\text{I},i,j}(1,0) + \boldsymbol{X}_{i,j}^\top\boldsymbol{\gamma}^{\text{adj}}_{\text{I}}(1,0) - \overline{\epsilon}_{\mathcal{S}(1,0)} - \left(\boldsymbol{X}_{i,j} - \overline{\boldsymbol{X}}_{\mathcal{S}(1,0)}\right)^\top\widehat{\boldsymbol{\gamma}}^{\text{adj}}_{\text{I}}(1,0)\right\}\right]^2 \\
&= \frac{1}{N(N-1)^2}\sum_{i=1}^N A_i\left(\sum_{j:j\neq i}(1-A_j)\left[r^{\text{adj}}_{\text{I},i,j}(1,0) + \boldsymbol{X}_{i,j}^\top\left\{\boldsymbol{\gamma}^{\text{adj}}_{\text{I}}(1,0) - \widehat{\boldsymbol{\gamma}}^{\text{adj}}_{\text{I}}(1,0)\right\} - \left\{\overline{\epsilon}_{\mathcal{S}(1,0)} - \overline{\boldsymbol{X}}^\top_{\mathcal{S}(1,0)}\widehat{\boldsymbol{\gamma}}^{\text{adj}}_{\text{I}}(1,0)\right\}\right]\right)^2 \\
&= T_{\text{CR},1} + T_{\text{CR},2} + T_{\text{CR},3} + T_{\text{CR},4} - T_{\text{CR},5} - T_{\text{CR},6},
\end{aligned}$$

where

$$T_{\text{CR},1} = \frac{1}{N(N-1)^2}\sum_{i=1}^N A_i\left\{\sum_{j:j\neq i}(1-A_j)r^{\text{adj}}_{\text{I},i,j}(1,0)\right\}^2,$$
$$T_{\text{CR},2} = \frac{1}{N(N-1)^2}\sum_{i=1}^N A_i\left[\sum_{j:j\neq i}(1-A_j)\boldsymbol{X}_{i,j}^\top\left\{\boldsymbol{\gamma}^{\text{adj}}_{\text{I}}(1,0) - \widehat{\boldsymbol{\gamma}}^{\text{adj}}_{\text{I}}(1,0)\right\}\right]^2,$$

$$T_{\mathrm{CR},3}=\frac{1}{N(N-1)^2}\sum_{i=1}^{N}A_i\left[\sum_{j:j\neq i}(1-A_j)\left\{\bar{\epsilon}_{\mathcal{S}(1,0)}-\overline{\boldsymbol{X}}_{\mathcal{S}(a,1-a)}^{\top}\widehat{\boldsymbol{\gamma}}_{\mathrm{I}}^{\mathrm{adj}}(1,0)\right\}\right]^2$$

$$T_{\mathrm{CR},4}=\frac{2}{N(N-1)^2}\sum_{i=1}^{N}A_i\sum_{j:j\neq i}(1-A_j)r_{\mathrm{I},i,j}^{\mathrm{adj}}(1,0)\sum_{j:j\neq i}(1-A_j)\boldsymbol{X}_{i,j}^{\top}\left\{\boldsymbol{\gamma}_{\mathrm{I}}^{\mathrm{adj}}(1,0)-\widehat{\boldsymbol{\gamma}}_{\mathrm{I}}^{\mathrm{adj}}(1,0)\right\},$$

$$T_{\mathrm{CR},5}=\frac{2}{N(N-1)^2}\sum_{i=1}^{N}A_i\sum_{j:j\neq i}(1-A_j)r_{\mathrm{I},i,j}^{\mathrm{adj}}(1,0)\sum_{j:j\neq i}(1-A_j)\left\{\bar{\epsilon}_{\mathcal{S}(1,0)}-\overline{\boldsymbol{X}}_{\mathcal{S}(a,1-a)}^{\top}\widehat{\boldsymbol{\gamma}}_{\mathrm{I}}^{\mathrm{adj}}(1,0)\right\},$$

$$T_{\mathrm{CR},6}=\frac{2}{N(N-1)^2}\sum_{i=1}^{N}A_i\sum_{j:j\neq i}(1-A_j)\boldsymbol{X}_{i,j}^{\top}\left\{\boldsymbol{\gamma}_{\mathrm{I}}^{\mathrm{adj}}(1,0)-\widehat{\boldsymbol{\gamma}}_{\mathrm{I}}^{\mathrm{adj}}(1,0)\right\}\sum_{j:j\neq i}(1-A_j)\left\{\bar{\epsilon}_{\mathcal{S}(1,0)}-\overline{\boldsymbol{X}}_{\mathcal{S}(a,1-a)}^{\top}\widehat{\boldsymbol{\gamma}}_{\mathrm{I}}^{\mathrm{adj}}(1,0)\right\}.$$

Except for $T_{\mathrm{CR},1}$, all other terms are $o_{\mathbb{P}}(1)$. We show that $T_{\mathrm{CR},4}=o_{\mathbb{P}}(1)$ and omit the proofs for other terms. Specifically,

$$\begin{aligned}
|T_{\mathrm{CR},4}| &\leq \frac{2}{N(N-1)^2}\sum_{i=1}^{N}\left\|\sum_{j:j\neq i}r_{\mathrm{I},i,j}^{\mathrm{adj}}(1,0)\sum_{j:j\neq i}\boldsymbol{X}_{i,j}\right\|\left\|\boldsymbol{\gamma}_{\mathrm{I}}^{\mathrm{adj}}(1,0)-\widehat{\boldsymbol{\gamma}}_{\mathrm{I}}^{\mathrm{adj}}(1,0)\right\| \\
&\leq \frac{2}{N(N-1)^2}\sum_{i=1}^{N}\left[\left\{\sum_{j:j\neq i}r_{\mathrm{I},i,j}^{\mathrm{adj}}(1,0)\right\}^2+\left\|\sum_{j:j\neq i}\boldsymbol{X}_{i,j}\right\|^2\right]\left\|\boldsymbol{\gamma}_{\mathrm{I}}^{\mathrm{adj}}(1,0)-\widehat{\boldsymbol{\gamma}}_{\mathrm{I}}^{\mathrm{adj}}(1,0)\right\| \\
&\leq \frac{2}{N(N-1)}\sum_{i=1}^{N}\left\{\sum_{j:j\neq i}r_{\mathrm{I},i,j}^{\mathrm{adj}}(1,0)^2+\sum_{j:j\neq i}\|\boldsymbol{X}_{i,j}\|^2\right\}\left\|\boldsymbol{\gamma}_{\mathrm{I}}^{\mathrm{adj}}(1,0)-\widehat{\boldsymbol{\gamma}}_{\mathrm{I}}^{\mathrm{adj}}(1,0)\right\|. \qquad \text{(Hölder's inequality)}
\end{aligned}$$

By Lemma S8, $\|\boldsymbol{\gamma}_{\mathrm{I}}^{\mathrm{adj}}(1,0)-\widehat{\boldsymbol{\gamma}}_{\mathrm{I}}^{\mathrm{adj}}(1,0)\|=O_{\mathbb{P}}(N^{-1/2})$, and under Conditions 2 and 3 in the main article,

$$\frac{1}{N(N-1)}\sum_{i\neq j}r_{\mathrm{I},i,j}^{\mathrm{adj}}(1,0)^2=O(1),\quad \frac{1}{N(N-1)}\sum_{i\neq j}\|\boldsymbol{X}_{i,j}\|^2=O(1).$$

Therefore, $|T_{\mathrm{CR},4}|\leq O(1)O_{\mathbb{P}}(N^{-1/2})=o_{\mathbb{P}}(1)$. To finish the proof of (S7), we only need to verify that $T_{\mathrm{CR},1}$ differs from its mean by a term of $o_{\mathbb{P}}(1)$. Specifically, by Hölder's inequality

$$\begin{aligned}
\mathbb{V}\mathrm{ar}(T_{\mathrm{CR},1}) &\leq \frac{1}{N^2(N-1)^4}\sum_{i=1}^{N}\left\{\sum_{j:j\neq i}r_{\mathrm{I},i,j}^{\mathrm{adj}}(1,0)\right\}^2\leq\frac{1}{N^2(N-1)^4}\sum_{i=1}^{N}(N-1)^3\sum_{j:j\neq i}r_{\mathrm{I},i,j}^{\mathrm{adj}}(1,0)^4 \\
&\leq O\left(\frac{1}{N}\right)\cdot\frac{1}{N(N-1)}\sum_{i\neq j}r_{\mathrm{I},i,j}^{\mathrm{adj}}(1,0)^4=O\left(\frac{1}{N}\right)o(N)=o(1).
\end{aligned}$$

Then, the result follows from Chebyshev's inequality. Second, we prove (S8). By the definition of $\widehat{r}_{\mathrm{I},i,j}^{\mathrm{adj}}$,

$$\begin{aligned}
&\frac{1}{N(N-1)^2}\sum_{i=1}^{N}A_i(1-A_j)\sum_{j:j\neq i}\widehat{r}_{\mathrm{I},i,j}^{\mathrm{adj}}\sum_{j:j\neq i}\boldsymbol{X}_{i,j}^{\top}\widehat{r}_{\mathrm{I},i,j}^{\mathrm{adj}} \\
&=\frac{1}{N(N-1)^2}\sum_{i=1}^{N}A_i(1-A_j)\sum_{j:j\neq i}\left[\epsilon_{i,j}(1,0)-\boldsymbol{X}_{i,j}^{\top}\widehat{\boldsymbol{\gamma}}_{\mathrm{I}}^{\mathrm{adj}}(1,0)-\left\{\bar{\epsilon}_{\mathcal{S}(1,0)}-\overline{\boldsymbol{X}}_{\mathcal{S}(a,1-a)}^{\top}\widehat{\boldsymbol{\gamma}}_{\mathrm{I}}^{\mathrm{adj}}(1,0)\right\}\right] \\
&\quad\times\sum_{j:j\neq i}\boldsymbol{X}_{i,j}^{\top}\left[\epsilon_{i,j}(1,0)-\boldsymbol{X}_{i,j}^{\top}\widehat{\boldsymbol{\gamma}}_{\mathrm{I}}^{\mathrm{adj}}(1,0)-\left\{\bar{\epsilon}_{\mathcal{S}(1,0)}-\overline{\boldsymbol{X}}_{\mathcal{S}(a,1-a)}^{\top}\widehat{\boldsymbol{\gamma}}_{\mathrm{I}}^{\mathrm{adj}}(1,0)\right\}\right] \\
&=\boldsymbol{T}_{\mathrm{CR},7}-\boldsymbol{T}_{\mathrm{CR},8}-\boldsymbol{T}_{\mathrm{CR},9}-\boldsymbol{T}_{\mathrm{CR},10}+\boldsymbol{T}_{\mathrm{CR},11}+\boldsymbol{T}_{\mathrm{CR},12}-\boldsymbol{T}_{\mathrm{CR},13}+\boldsymbol{T}_{\mathrm{CR},14}+\boldsymbol{T}_{\mathrm{CR},15},
\end{aligned}$$

where

$$\boldsymbol{T}_{\mathrm{CR},7} = \frac{1}{N(N-1)^2}\sum_{i=1}^{N} A_i(1-A_j)\sum_{j:j\neq i}\epsilon_{i,j}(1,0)\sum_{j:j\neq i}\boldsymbol{X}_{i,j}^{\top}\epsilon_{i,j}(1,0),$$

$$\boldsymbol{T}_{\mathrm{CR},8} = \frac{1}{N(N-1)^2}\sum_{i=1}^{N} A_i(1-A_j)\sum_{j:j\neq i}\epsilon_{i,j}(1,0)\sum_{j:j\neq i}\boldsymbol{X}_{i,j}^{\top}\left\{\boldsymbol{X}_{i,j}^{\top}\widehat{\gamma}_{\mathrm{I}}^{\mathrm{adj}}(1,0)\right\},$$

$$\boldsymbol{T}_{\mathrm{CR},9} = \frac{1}{N(N-1)^2}\sum_{i=1}^{N} A_i(1-A_j)\sum_{j:j\neq i}\epsilon_{i,j}(1,0)\sum_{j:j\neq i}\boldsymbol{X}_{i,j}^{\top}\left\{\bar{\epsilon}_{\mathcal{S}(1,0)}-\overline{\boldsymbol{X}}_{\mathcal{S}(a,1-a)}^{\top}\widehat{\gamma}_{\mathrm{I}}^{\mathrm{adj}}(1,0)\right\},$$

$$\boldsymbol{T}_{\mathrm{CR},10} = \frac{1}{N(N-1)^2}\sum_{i=1}^{N} A_i(1-A_j)\sum_{j:j\neq i}\boldsymbol{X}_{i,j}^{\top}\widehat{\gamma}_{\mathrm{I}}^{\mathrm{adj}}(1,0)\sum_{j:j\neq i}\boldsymbol{X}_{i,j}^{\top}\epsilon_{i,j}(1,0),$$

$$\boldsymbol{T}_{\mathrm{CR},11} = \frac{1}{N(N-1)^2}\sum_{i=1}^{N} A_i(1-A_j)\sum_{j:j\neq i}\boldsymbol{X}_{i,j}^{\top}\widehat{\gamma}_{\mathrm{I}}^{\mathrm{adj}}(1,0)\sum_{j:j\neq i}\boldsymbol{X}_{i,j}^{\top}\left\{\boldsymbol{X}_{i,j}^{\top}\widehat{\gamma}_{\mathrm{I}}^{\mathrm{adj}}(1,0)\right\},$$

$$\boldsymbol{T}_{\mathrm{CR},12} = \frac{1}{N(N-1)^2}\sum_{i=1}^{N} A_i(1-A_j)\sum_{j:j\neq i}\boldsymbol{X}_{i,j}^{\top}\widehat{\gamma}_{\mathrm{I}}^{\mathrm{adj}}(1,0)\sum_{j:j\neq i}\boldsymbol{X}_{i,j}^{\top}\left\{\bar{\epsilon}_{\mathcal{S}(1,0)}-\overline{\boldsymbol{X}}_{\mathcal{S}(a,1-a)}^{\top}\widehat{\gamma}_{\mathrm{I}}^{\mathrm{adj}}(1,0)\right\},$$

$$\boldsymbol{T}_{\mathrm{CR},13} = \frac{1}{N(N-1)^2}\sum_{i=1}^{N} A_i(1-A_j)\sum_{j:j\neq i}\left\{\bar{\epsilon}_{\mathcal{S}(1,0)}-\overline{\boldsymbol{X}}_{\mathcal{S}(a,1-a)}^{\top}\widehat{\gamma}_{\mathrm{I}}^{\mathrm{adj}}(1,0)\right\}\sum_{j:j\neq i}\boldsymbol{X}_{i,j}^{\top}\epsilon_{i,j}(1,0),$$

$$\boldsymbol{T}_{\mathrm{CR},14} = \frac{1}{N(N-1)^2}\sum_{i=1}^{N} A_i(1-A_j)\sum_{j:j\neq i}\left\{\bar{\epsilon}_{\mathcal{S}(1,0)}-\overline{\boldsymbol{X}}_{\mathcal{S}(a,1-a)}^{\top}\widehat{\gamma}_{\mathrm{I}}^{\mathrm{adj}}(1,0)\right\}\sum_{j:j\neq i}\boldsymbol{X}_{i,j}^{\top}\left\{\boldsymbol{X}_{i,j}^{\top}\widehat{\gamma}_{\mathrm{I}}^{\mathrm{adj}}(1,0)\right\},$$

$$\boldsymbol{T}_{\mathrm{CR},15} = \frac{1}{N(N-1)^2}\sum_{i=1}^{N} A_i(1-A_j)\sum_{j:j\neq i}\left\{\bar{\epsilon}_{\mathcal{S}(1,0)}-\overline{\boldsymbol{X}}_{\mathcal{S}(a,1-a)}^{\top}\widehat{\gamma}_{\mathrm{I}}^{\mathrm{adj}}(1,0)\right\}\sum_{j:j\neq i}\boldsymbol{X}_{i,j}^{\top}\left\{\bar{\epsilon}_{\mathcal{S}(1,0)}-\overline{\boldsymbol{X}}_{\mathcal{S}(a,1-a)}^{\top}\widehat{\gamma}_{\mathrm{I}}^{\mathrm{adj}}(1,0)\right\}.$$

All terms $\boldsymbol{T}_{\mathrm{CR},7}$ to $\boldsymbol{T}_{\mathrm{CR},15}$ are $\boldsymbol{O}_{\mathbb{P}}(1)$. We prove that $\boldsymbol{T}_{\mathrm{CR},7} = \boldsymbol{O}_{\mathbb{P}}(1)$ and omit the proofs for other terms. Specifically, under Condition 3 in the main article,

$$\begin{aligned}
\|\boldsymbol{T}_{\mathrm{CR},7}\| &\leq \frac{1}{N(N-1)^2}\sum_{i=1}^{N}\left\|\sum_{j:j\neq i}\epsilon_{i,j}(1,0)\sum_{j:j\neq i}\boldsymbol{X}_{i,j}^{\top}\epsilon_{i,j}(1,0)\right\| \\
&\leq O\left(\frac{1}{N^3}\right)\sum_{i=1}^{N}\left[\left\{\sum_{j:j\neq i}\epsilon_{i,j}(1,0)\right\}^2+\left\|\sum_{j:j\neq i}\boldsymbol{X}_{i,j}^{\top}\epsilon_{i,j}(1,0)\right\|^2\right] \\
&\leq O\left(\frac{1}{N^3}\right)\sum_{i=1}^{N}\left\{(N-1)\sum_{j:j\neq i}\epsilon_{i,j}(1,0)^2+(N-1)\sum_{j:j\neq i}\|\boldsymbol{X}_{i,j}\|^2\epsilon_{i,j}(1,0)^2\right\} \qquad \text{(Hölder's inequality)} \\
&\leq O\left(\frac{1}{N^2}\right)\sum_{i=1}^{N}\sum_{j:j\neq i}\left\{\epsilon_{i,j}(1,0)^2+\|\boldsymbol{X}_{i,j}\|^4+\epsilon_{i,j}(1,0)^4\right\}\leq O(1).
\end{aligned}$$

Therefore, (S8) holds. The proof of (S9) is similar to that of (S8), and is thus omitted.

## S6.16 Lemma S24

For (S48), by the definition of $\widehat{r}_{\mathrm{A},1,i,\cdot}^{\mathrm{adj}}$,

$$\frac{1}{N}\sum_{i=1}^{N}A_i(\widehat{r}_{\mathrm{A},1,i,\cdot}^{\mathrm{adj}})^2$$

$$
\begin{aligned}
&= \frac{1}{NN_0^2}\sum_{i=1}^N A_i\left(\sum_{j:j\neq i}\widehat{r}^{\text{adj}}_{\text{A},1,i,j}\right)^2 \\
&= \frac{1}{NN_0^2}\sum_{i=1}^N A_i\left[\sum_{j:j\neq i}(1-A_j)\left\{W_{i,j}(1,0)-\overline{W}_{\mathcal{S}(1,0)}-\left(\boldsymbol{X}_{i,j}-\overline{\boldsymbol{X}}_{\mathcal{S}(1,0)}\right)^\top\widehat{\boldsymbol{\gamma}}^{\text{adj}}_{\text{A},1}(1,0)\right\}\right]^2 \\
&= \frac{1}{NN_0^2}\sum_{i=1}^N A_i\left[\sum_{j:j\neq i}(1-A_j)\left\{r^{\text{adj}}_{\text{A},1,i,j}(1,0)+\boldsymbol{X}_{i,j}^\top\boldsymbol{\gamma}^{\text{adj}}_{\text{A},1}(1,0)-\overline{\epsilon}_{\mathcal{S}(1,0)}-\left(\boldsymbol{X}_{i,j}-\overline{\boldsymbol{X}}_{\mathcal{S}(1,0)}\right)^\top\widehat{\boldsymbol{\gamma}}^{\text{adj}}_{\text{A},1}(1,0)\right\}\right]^2 \\
&= \frac{1}{NN_0^2}\sum_{i=1}^N A_i\left(\sum_{j:j\neq i}(1-A_j)\left[r^{\text{adj}}_{\text{A},1,i,j}(1,0)+\boldsymbol{X}_{i,j}^\top\left\{\boldsymbol{\gamma}^{\text{adj}}_{\text{A},1}(1,0)-\widehat{\boldsymbol{\gamma}}^{\text{adj}}_{\text{A},1}(1,0)\right\}-\left\{\overline{\epsilon}_{\mathcal{S}(1,0)}-\overline{\boldsymbol{X}}_{\mathcal{S}(1,0)}^\top\widehat{\boldsymbol{\gamma}}^{\text{adj}}_{\text{A},1}(1,0)\right\}\right]\right)^2 .
\end{aligned}
$$

Then, the proof follows that of (S7) and thus is omitted. For (S49),

$$
\begin{aligned}
&\frac{1}{N}\sum_{i=1}^N A_i\overline{\boldsymbol{X}}^{A\top}_{i,\cdot}(\widehat{r}^{\text{adj}}_{\text{A},1,i,\cdot})^2 \\
&= \frac{1}{NN_0^2}\sum_{i=1}^N A_i\overline{\boldsymbol{X}}^{A\top}_{i,\cdot}\left(\sum_{j:j\neq i}(1-A_j)\left[\epsilon_{i,j}(1,0)-\boldsymbol{X}_{i,j}^\top\widehat{\boldsymbol{\gamma}}^{\text{adj}}_{\text{A},1}(1,0)-\left\{\overline{\epsilon}_{\mathcal{S}(1,0)}-\overline{\boldsymbol{X}}_{\mathcal{S}(1,0)}^\top\widehat{\boldsymbol{\gamma}}^{\text{adj}}_{\text{A},1}(1,0)\right\}\right]\right)^2 \\
&= \frac{1}{NN_0^2}\sum_{i=1}^N A_i(1-A_j)\overline{\boldsymbol{X}}^{A\top}_{i,\cdot}\sum_{j:j\neq i}\left[\epsilon_{i,j}(1,0)-\boldsymbol{X}_{i,j}^\top\widehat{\boldsymbol{\gamma}}^{\text{adj}}_{\text{A},1}(1,0)-\left\{\overline{\epsilon}_{\mathcal{S}(1,0)}-\overline{\boldsymbol{X}}_{\mathcal{S}(a,1-a)}^\top\widehat{\boldsymbol{\gamma}}^{\text{adj}}_{\text{A},1}(1,0)\right\}\right] \\
&\quad\times\sum_{j:j\neq i}\left[\epsilon_{i,j}(1,0)-\boldsymbol{X}_{i,j}^\top\widehat{\boldsymbol{\gamma}}^{\text{adj}}_{\text{A},1}(1,0)-\left\{\overline{\epsilon}_{\mathcal{S}(1,0)}-\overline{\boldsymbol{X}}_{\mathcal{S}(a,1-a)}^\top\widehat{\boldsymbol{\gamma}}^{\text{adj}}_{\text{A},1}(1,0)\right\}\right] \\
&= \boldsymbol{T}_{\text{A,HR},7}-\boldsymbol{T}_{\text{A,HR},8}-\boldsymbol{T}_{\text{A,HR},9}-\boldsymbol{T}_{\text{A,HR},10}+\boldsymbol{T}_{\text{A,HR},11}+T_{\text{A,HR},12}-T_{\text{A,HR},13}+T_{\text{A,HR},14}+\boldsymbol{T}_{\text{A,HR},15},
\end{aligned}
$$

where

$$
\begin{aligned}
\boldsymbol{T}_{\text{A,HR},7} &= \frac{1}{NN_0^2}\sum_{i=1}^N A_i(1-A_j)\overline{\boldsymbol{X}}^{A\top}_{i,\cdot}\sum_{j:j\neq i}\epsilon_{i,j}(1,0)\sum_{j:j\neq i}\boldsymbol{X}_{i,j}^\top\epsilon_{i,j}(1,0), \\
\boldsymbol{T}_{\text{A,HR},8} &= \frac{1}{NN_0^2}\sum_{i=1}^N A_i(1-A_j)\overline{\boldsymbol{X}}^{A\top}_{i,\cdot}\sum_{j:j\neq i}\epsilon_{i,j}(1,0)\sum_{j:j\neq i}\boldsymbol{X}_{i,j}^\top\left\{\boldsymbol{X}_{i,j}^\top\widehat{\boldsymbol{\gamma}}^{\text{adj}}_{\text{A},1}(1,0)\right\}, \\
\boldsymbol{T}_{\text{A,HR},9} &= \frac{1}{NN_0^2}\sum_{i=1}^N A_i(1-A_j)\overline{\boldsymbol{X}}^{A\top}_{i,\cdot}\sum_{j:j\neq i}\epsilon_{i,j}(1,0)\sum_{j:j\neq i}\boldsymbol{X}_{i,j}^\top\left\{\overline{\epsilon}_{\mathcal{S}(1,0)}-\overline{\boldsymbol{X}}_{\mathcal{S}(a,1-a)}^\top\widehat{\boldsymbol{\gamma}}^{\text{adj}}_{\text{A},1}(1,0)\right\}, \\
\boldsymbol{T}_{\text{A,HR},10} &= \frac{1}{NN_0^2}\sum_{i=1}^N A_i(1-A_j)\overline{\boldsymbol{X}}^{A\top}_{i,\cdot}\sum_{j:j\neq i}\boldsymbol{X}_{i,j}^\top\widehat{\boldsymbol{\gamma}}^{\text{adj}}_{\text{A},1}(1,0)\sum_{j:j\neq i}\boldsymbol{X}_{i,j}^\top\epsilon_{i,j}(1,0), \\
\boldsymbol{T}_{\text{A,HR},11} &= \frac{1}{NN_0^2}\sum_{i=1}^N A_i(1-A_j)\overline{\boldsymbol{X}}^{A\top}_{i,\cdot}\sum_{j:j\neq i}\boldsymbol{X}_{i,j}^\top\widehat{\boldsymbol{\gamma}}^{\text{adj}}_{\text{A},1}(1,0)\sum_{j:j\neq i}\boldsymbol{X}_{i,j}^\top\left\{\boldsymbol{X}_{i,j}^\top\widehat{\boldsymbol{\gamma}}^{\text{adj}}_{\text{A},1}(1,0)\right\}, \\
\boldsymbol{T}_{\text{A,HR},12} &= \frac{1}{NN_0^2}\sum_{i=1}^N A_i(1-A_j)\overline{\boldsymbol{X}}^{A\top}_{i,\cdot}\sum_{j:j\neq i}\boldsymbol{X}_{i,j}^\top\widehat{\boldsymbol{\gamma}}^{\text{adj}}_{\text{A},1}(1,0)\sum_{j:j\neq i}\boldsymbol{X}_{i,j}^\top\left\{\overline{\epsilon}_{\mathcal{S}(1,0)}-\overline{\boldsymbol{X}}_{\mathcal{S}(a,1-a)}^\top\widehat{\boldsymbol{\gamma}}^{\text{adj}}_{\text{A},1}(1,0)\right\}, \\
\boldsymbol{T}_{\text{A,HR},13} &= \frac{1}{NN_0^2}\sum_{i=1}^N A_i(1-A_j)\overline{\boldsymbol{X}}^{A\top}_{i,\cdot}\sum_{j:j\neq i}\left\{\overline{\epsilon}_{\mathcal{S}(1,0)}-\overline{\boldsymbol{X}}_{\mathcal{S}(a,1-a)}^\top\widehat{\boldsymbol{\gamma}}^{\text{adj}}_{\text{A},1}(1,0)\right\}\sum_{j:j\neq i}\boldsymbol{X}_{i,j}^\top\epsilon_{i,j}(1,0), \\
\boldsymbol{T}_{\text{A,HR},14} &= \frac{1}{NN_0^2}\sum_{i=1}^N A_i(1-A_j)\overline{\boldsymbol{X}}^{A\top}_{i,\cdot}\sum_{j:j\neq i}\left\{\overline{\epsilon}_{\mathcal{S}(1,0)}-\overline{\boldsymbol{X}}_{\mathcal{S}(a,1-a)}^\top\widehat{\boldsymbol{\gamma}}^{\text{adj}}_{\text{A},1}(1,0)\right\}\sum_{j:j\neq i}\boldsymbol{X}_{i,j}^\top\left\{\boldsymbol{X}_{i,j}^\top\widehat{\boldsymbol{\gamma}}^{\text{adj}}_{\text{A},1}(1,0)\right\},
\end{aligned}
$$

$$\boldsymbol{T}_{\text{A,HR},15} = \frac{1}{NN_0^2}\sum_{i=1}^{N} A_i(1-A_j)\overline{\boldsymbol{X}}_{i,\cdot}^{A\top} \sum_{j:j\neq i} \left\{\bar{\epsilon}_{\mathcal{S}(1,0)} - \overline{\boldsymbol{X}}_{\mathcal{S}(a,1-a)}^{\top}\widehat{\gamma}_{\text{A},1}^{\text{adj}}(1,0)\right\} \sum_{j:j\neq i} \boldsymbol{X}_{i,j}^{\top}\left\{\bar{\epsilon}_{\mathcal{S}(1,0)} - \overline{\boldsymbol{X}}_{\mathcal{S}(a,1-a)}^{\top}\widehat{\gamma}_{\text{A},1}^{\text{adj}}(1,0)\right\}.$$

All terms $\boldsymbol{T}_{\text{A,HR},7}$ to $\boldsymbol{T}_{\text{A,HR},15}$ are $\boldsymbol{O}_{\mathbb{P}}(1)$. We prove that $\boldsymbol{T}_{\text{A,HR},7} = \boldsymbol{O}_{\mathbb{P}}(1)$ and omit the proofs for other terms. Specifically, under Condition 4 in the main article,

$$\begin{aligned}
\|\boldsymbol{T}_{\text{A,HR},7}\| &\leq \frac{1}{N(N-1)^2}\sum_{i=1}^{N}\|\overline{\boldsymbol{X}}_{i,\cdot}\| \left\| \sum_{j:j\neq i}\epsilon_{i,j}(1,0)\sum_{j:j\neq i}\boldsymbol{X}_{i,j}^{\top}\epsilon_{i,j}(1,0)\right\| \\
&\leq O\left(\frac{1}{N^3}\right)\sum_{i=1}^{N} O(1)\left[\left\{\sum_{j:j\neq i}\epsilon_{i,j}(1,0)\right\}^2 + \left\|\sum_{j:j\neq i}\boldsymbol{X}_{i,j}^{\top}\epsilon_{i,j}(1,0)\right\|^2\right] \\
&\leq O\left(\frac{1}{N^3}\right)\sum_{i=1}^{N}\left\{(N-1)\sum_{j:j\neq i}\epsilon_{i,j}(1,0)^2 + (N-1)\sum_{j:j\neq i}\|\boldsymbol{X}_{i,j}\|^2\epsilon_{i,j}(1,0)^2\right\} \qquad \text{(Hölder's inequality)} \\
&\leq O\left(\frac{1}{N^2}\right)\sum_{i=1}^{N}\sum_{j:j\neq i}\left\{\epsilon_{i,j}(1,0)^2 + \|\boldsymbol{X}_{i,j}\|^4 + \epsilon_{i,j}(1,0)^4\right\} \leq O(1).
\end{aligned}$$

Therefore, (S49) holds. The proof of (S50) is similar to that of (S49), and is thus omitted.

# References


Angrist, J. D. and Pischke, J.-S. (2009), *Mostly Harmless Econometrics: An Empiricist's Companion*, Princeton University Press.

Li, X. and Ding, P. (2017), "General forms of finite population central limit theorems with applications to causal inference," *Journal of the American Statistical Association*, 112, 1759–1769.

Su, F. and Ding, P. (2021), "Model-assisted analyses of cluster-randomized experiments," *Journal of the Royal Statistical Society: Series B (Statistical Methodology)*, 83, 994–1015.

van der Vaart, A. (1998), *Asymptotic Statistics*, Cambridge University Press.

# S7 Additional simulation results

Web Table S1: Results from simulation study I. ESE: empirical standard error; ASE: average standard error; ECP: empirical coverage percentage of the 95% confidence interval. ASEs are from the complete two-way (CTW) variance estimator.

| $\lambda(1,0)$ | | | | | | | | |
|---|---|---|---|---|---|---|---|---|
| | $N=200$ | | | | $N=500$ | | | |
| Estimator | Bias | ESE | ASE | ECP | Bias | ESE | ASE | ECP |
| $\widehat{\lambda}_{\mathrm{I}}$ | −.0001 | .0411 | .0401 | .950 | −.0001 | .0256 | .0256 | .951 |
| $\widehat{\lambda}_{\mathrm{I}}^{\mathrm{adj}}$ | −.0002 | .0353 | .0342 | .952 | −.0005 | .0221 | .0218 | .948 |
| $\widehat{\lambda}_{\mathrm{I}}^{\mathrm{acv}}$ | −.0002 | .0352 | .0342 | .953 | −.0005 | .0221 | .0218 | .947 |
| $\widehat{\lambda}_{\mathrm{A},1}^{\mathrm{adj}}$ | .0005 | .0375 | .0358 | .948 | −.0002 | .0237 | .0221 | .935 |
| $\widehat{\lambda}_{\mathrm{A},2}^{\mathrm{adj}}$ | −.0009 | .0369 | .0358 | .956 | −.0010 | .0229 | .0221 | .950 |
| $\widehat{\lambda}_{\mathrm{A},1}^{\mathrm{acv}}$ | −.0002 | .0353 | .0377 | .977 | −.0005 | .0221 | .0233 | .965 |
| $\widehat{\lambda}_{\mathrm{A},2}^{\mathrm{acv}}$ | .0002 | .0353 | .0376 | .978 | −.0005 | .0221 | .0233 | .964 |

| $\lambda(0,1)$ | | | | | | | | |
|---|---|---|---|---|---|---|---|---|
| | $N=200$ | | | | $N=500$ | | | |
| Estimator | Bias | ESE | ASE | ECP | Bias | ESE | ASE | ECP |
| $\widehat{\lambda}_{\mathrm{I}}$ | .0001 | .0411 | .0401 | .950 | .0001 | .0256 | .0256 | .951 |
| $\widehat{\lambda}_{\mathrm{I}}^{\mathrm{adj}}$ | .0002 | .0353 | .0342 | .952 | .0005 | .0221 | .0218 | .948 |
| $\widehat{\lambda}_{\mathrm{I}}^{\mathrm{acv}}$ | .0002 | .0352 | .0342 | .953 | .0005 | .0221 | .0218 | .947 |
| $\widehat{\lambda}_{\mathrm{A},1}^{\mathrm{adj}}$ | .0009 | .0369 | .0358 | .956 | .0010 | .0229 | .0221 | .950 |
| $\widehat{\lambda}_{\mathrm{A},2}^{\mathrm{adj}}$ | −.0005 | .0375 | .0358 | .948 | .0002 | .0237 | .0221 | .935 |
| $\widehat{\lambda}_{\mathrm{A},1}^{\mathrm{acv}}$ | .0002 | .0353 | .0376 | .978 | .0005 | .0221 | .0233 | .964 |
| $\widehat{\lambda}_{\mathrm{A},2}^{\mathrm{acv}}$ | −.0002 | .0353 | .0377 | .977 | .0005 | .0221 | .0233 | .965 |

| $\tau(1)$ | | | | | | | | |
|---|---|---|---|---|---|---|---|---|
| | $N=200$ | | | | $N=500$ | | | |
| Method | Bias | ESE | ASE | ECP | Bias | ESE | ASE | ECP |
| $\widehat{\tau}_{\mathrm{I}}$ | −.0001 | .0822 | .0808 | .951 | −.0003 | .0512 | .0512 | .951 |
| $\widehat{\tau}_{\mathrm{I}}^{\mathrm{adj}}$ | −.0004 | .0706 | .0690 | .956 | −.0011 | .0443 | .0437 | .949 |
| $\widehat{\tau}_{\mathrm{I}}^{\mathrm{acv}}$ | −.0004 | .0705 | .0690 | .957 | −.0011 | .0443 | .0437 | .947 |
| $\widehat{\tau}_{\mathrm{P}}$ | −.0001 | .0822 | .0802 | .950 | −.0003 | .0512 | .0512 | .951 |
| $\widehat{\tau}_{\mathrm{P}}^{\mathrm{acv}}$ | −.0004 | .0705 | .0683 | .953 | −.0011 | .0443 | .0436 | .947 |
| $\widehat{\tau}_{\mathrm{P}}^{\mathrm{int}}$ | −.0001 | .0822 | .0802 | .950 | −.0003 | .0512 | .0512 | .951 |
| $\widehat{\tau}_{\mathrm{P}}^{\mathrm{adj}}$ | −.0004 | .0705 | .0683 | .953 | −.0011 | .0443 | .0436 | .947 |
| $\widehat{\tau}_{\mathrm{A},1}^{\mathrm{adj}}$ | −.0004 | .0706 | .0692 | .963 | −.0011 | .0443 | .0430 | .947 |
| $\widehat{\tau}_{\mathrm{A},2}^{\mathrm{adj}}$ | −.0004 | .0706 | .0692 | .963 | −.0011 | .0443 | .0430 | .947 |
| $\widehat{\tau}_{\mathrm{A},1}^{\mathrm{acv}}$ | −.0004 | .0706 | .0732 | .971 | −.0011 | .0443 | .0454 | .960 |
| $\widehat{\tau}_{\mathrm{A},2}^{\mathrm{acv}}$ | −.0004 | .0706 | .0732 | .971 | −.0011 | .0443 | .0454 | .960 |

Web Table S2: Results from simulation study II. ESE: empirical standard error; ASE: average standard error; ECP: empirical coverage percentage of the 95% confidence interval. ASEs are from the complete two-way (CTW) variance estimator.

| $\lambda(1,0)$ | | | | | | | | |
|---|---|---|---|---|---|---|---|---|
| | $N=200$ | | | | $N=500$ | | | |
| Estimator | Bias | ESE | ASE | ECP | Bias | ESE | ASE | ECP |
| $\widehat{\lambda}_{\mathrm{I}}$ | −.0005 | .0189 | .0188 | .952 | −.0003 | .0120 | .0121 | .945 |
| $\widehat{\lambda}_{\mathrm{I}}^{\mathrm{adj}}$ | −.0007 | .0181 | .0176 | .938 | −.0004 | .0110 | .0112 | .947 |
| $\widehat{\lambda}_{\mathrm{I}}^{\mathrm{acv}}$ | −.0007 | .0180 | .0176 | .940 | −.0004 | .0111 | .0112 | .949 |
| $\widehat{\lambda}_{\mathrm{A},1}^{\mathrm{adj}}$ | −.0008 | .0183 | .0187 | .957 | −.0004 | .0114 | .0115 | .956 |
| $\widehat{\lambda}_{\mathrm{A},2}^{\mathrm{adj}}$ | −.0007 | .0187 | .0187 | .952 | −.0004 | .0113 | .0115 | .953 |
| $\widehat{\lambda}_{\mathrm{A},1}^{\mathrm{acv}}$ | −.0007 | .0181 | .0191 | .968 | −.0004 | .0111 | .0117 | .961 |
| $\widehat{\lambda}_{\mathrm{A},2}^{\mathrm{acv}}$ | −.0007 | .0181 | .0191 | .967 | −.0004 | .0111 | .0117 | .961 |

| $\lambda(0,1)$ | | | | | | | | |
|---|---|---|---|---|---|---|---|---|
| | $N=200$ | | | | $N=500$ | | | |
| Estimator | Bias | ESE | ASE | ECP | Bias | ESE | ASE | ECP |
| $\widehat{\lambda}_{\mathrm{I}}$ | .0005 | .0189 | .0188 | .952 | .0003 | .0120 | .0121 | .945 |
| $\widehat{\lambda}_{\mathrm{I}}^{\mathrm{adj}}$ | .0007 | .0181 | .0176 | .938 | .0004 | .0110 | .0112 | .947 |
| $\widehat{\lambda}_{\mathrm{I}}^{\mathrm{acv}}$ | .0007 | .0180 | .0176 | .940 | .0004 | .0111 | .0112 | .949 |
| $\widehat{\lambda}_{\mathrm{A},1}^{\mathrm{adj}}$ | .0007 | .0187 | .0187 | .952 | .0004 | .0113 | .0115 | .953 |
| $\widehat{\lambda}_{\mathrm{A},2}^{\mathrm{adj}}$ | .0008 | .0183 | .0187 | .957 | .0004 | .0114 | .0115 | .956 |
| $\widehat{\lambda}_{\mathrm{A},1}^{\mathrm{acv}}$ | .0007 | .0181 | .0191 | .967 | .0004 | .0111 | .0117 | .961 |
| $\widehat{\lambda}_{\mathrm{A},2}^{\mathrm{acv}}$ | .0007 | .0181 | .0191 | .968 | .0004 | .0111 | .0117 | .961 |

| $\tau(1)$ | | | | | | | | |
|---|---|---|---|---|---|---|---|---|
| | $N=200$ | | | | $N=500$ | | | |
| Method | Bias | ESE | ASE | ECP | Bias | ESE | ASE | ECP |
| $\widehat{\tau}_{\mathrm{I}}$ | −.0010 | .0378 | .0380 | .954 | −.0005 | .0239 | .0242 | .945 |
| $\widehat{\tau}_{\mathrm{I}}^{\mathrm{adj}}$ | −.0014 | .0361 | .0355 | .943 | −.0008 | .0221 | .0225 | .950 |
| $\widehat{\tau}_{\mathrm{I}}^{\mathrm{acv}}$ | −.0014 | .0361 | .0354 | .941 | −.0007 | .0222 | .0225 | .950 |
| $\widehat{\tau}_{\mathrm{P}}$ | −.0010 | .0378 | .0366 | .945 | −.0005 | .0239 | .0239 | .942 |
| $\widehat{\tau}_{\mathrm{P}}^{\mathrm{acv}}$ | −.0014 | .0361 | .0340 | .928 | −.0007 | .0222 | .0222 | .945 |
| $\widehat{\tau}_{\mathrm{P}}^{\mathrm{int}}$ | −.0010 | .0378 | .0367 | .945 | −.0005 | .0239 | .0239 | .942 |
| $\widehat{\tau}_{\mathrm{P}}^{\mathrm{adj}}$ | −.0014 | .0361 | .0339 | .927 | −.0007 | .0222 | .0222 | .945 |
| $\widehat{\tau}_{\mathrm{A},1}^{\mathrm{adj}}$ | −.0015 | .0361 | .0367 | .954 | −.0008 | .0222 | .0228 | .950 |
| $\widehat{\tau}_{\mathrm{A},2}^{\mathrm{adj}}$ | −.0015 | .0361 | .0367 | .954 | −.0008 | .0222 | .0228 | .950 |
| $\widehat{\tau}_{\mathrm{A},1}^{\mathrm{acv}}$ | −.0015 | .0361 | .0376 | .959 | −.0008 | .0222 | .0232 | .958 |
| $\widehat{\tau}_{\mathrm{A},2}^{\mathrm{acv}}$ | −.0015 | .0361 | .0376 | .959 | −.0008 | .0222 | .0232 | .958 |

Web Table S3: Results from simulation study III. ESE: empirical standard error; ASE: average standard error; ECP: empirical coverage percentage of the 95% confidence interval. ASEs are from the complete two-way (CTW) variance estimator.

| | $\lambda(1,0)$ | | | | | | | |
|---|---|---|---|---|---|---|---|---|
| | $N=200$ | | | | $N=500$ | | | |
| Estimator | Bias | ESE | ASE | ECP | Bias | ESE | ASE | ECP |
| $\widehat{\lambda}_{\mathrm{I}}$ | −.0001 | .0411 | .0401 | .950 | −.0001 | .0256 | .0256 | .951 |
| $\widehat{\lambda}_{\mathrm{I}}^{\mathrm{adj}}$ | −.0002 | .0412 | .0401 | .947 | −.0001 | .0256 | .0256 | .952 |
| $\widehat{\lambda}_{\mathrm{I}}^{\mathrm{acv}}$ | −.0002 | .0412 | .0401 | .947 | −.0001 | .0256 | .0256 | .952 |
| $\widehat{\lambda}_{\mathrm{A},1}^{\mathrm{adj}}$ | −.0003 | .0415 | .0433 | .967 | −.0001 | .0256 | .0269 | .958 |
| $\widehat{\lambda}_{\mathrm{A},2}^{\mathrm{adj}}$ | −.0001 | .0413 | .0433 | .969 | −.0001 | .0257 | .0269 | .956 |
| $\widehat{\lambda}_{\mathrm{A},1}^{\mathrm{acv}}$ | −.0002 | .0412 | .0434 | .970 | −.0001 | .0256 | .0269 | .959 |
| $\widehat{\lambda}_{\mathrm{A},2}^{\mathrm{acv}}$ | −.0002 | .0412 | .0434 | .970 | −.0001 | .0256 | .0269 | .959 |
| | $\lambda(0,1)$ | | | | | | | |
| | $N=200$ | | | | $N=500$ | | | |
| Estimator | Bias | ESE | ASE | ECP | Bias | ESE | ASE | ECP |
| $\widehat{\lambda}_{\mathrm{I}}$ | .0001 | .0411 | .0401 | .950 | .0001 | .0256 | .0256 | .951 |
| $\widehat{\lambda}_{\mathrm{I}}^{\mathrm{adj}}$ | .0002 | .0412 | .0401 | .947 | .0001 | .0256 | .0256 | .952 |
| $\widehat{\lambda}_{\mathrm{I}}^{\mathrm{acv}}$ | .0002 | .0412 | .0401 | .947 | .0001 | .0256 | .0256 | .952 |
| $\widehat{\lambda}_{\mathrm{A},1}^{\mathrm{adj}}$ | .0001 | .0413 | .0433 | .969 | .0001 | .0257 | .0269 | .956 |
| $\widehat{\lambda}_{\mathrm{A},2}^{\mathrm{adj}}$ | .0003 | .0415 | .0433 | .967 | .0001 | .0256 | .0269 | .958 |
| $\widehat{\lambda}_{\mathrm{A},1}^{\mathrm{acv}}$ | .0002 | .0412 | .0434 | .970 | .0001 | .0256 | .0269 | .959 |
| $\widehat{\lambda}_{\mathrm{A},2}^{\mathrm{acv}}$ | .0002 | .0412 | .0434 | .970 | .0001 | .0256 | .0269 | .959 |
| | $\tau(1)$ | | | | | | | |
| | $N=200$ | | | | $N=500$ | | | |
| Method | Bias | ESE | ASE | ECP | Bias | ESE | ASE | ECP |
| $\widehat{\tau}_{\mathrm{I}}$ | −.0001 | .0822 | .0808 | .951 | −.0003 | .0512 | .0513 | .951 |
| $\widehat{\tau}_{\mathrm{I}}^{\mathrm{adj}}$ | −.0004 | .0824 | .0807 | .950 | −.0001 | .0513 | .0513 | .952 |
| $\widehat{\tau}_{\mathrm{I}}^{\mathrm{acv}}$ | −.0004 | .0824 | .0807 | .951 | −.0001 | .0513 | .0513 | .952 |
| $\widehat{\tau}_{\mathrm{P}}$ | −.0001 | .0822 | .0802 | .950 | −.0003 | .0512 | .0511 | .951 |
| $\widehat{\tau}_{\mathrm{P}}^{\mathrm{acv}}$ | −.0004 | .0824 | .0801 | .947 | −.0001 | .0513 | .0511 | .952 |
| $\widehat{\tau}_{\mathrm{P}}^{\mathrm{int}}$ | −.0001 | .0822 | .0802 | .950 | −.0003 | .0512 | .0511 | .951 |
| $\widehat{\tau}_{\mathrm{P}}^{\mathrm{adj}}$ | −.0004 | .0824 | .0801 | .947 | −.0001 | .0513 | .0511 | .952 |
| $\widehat{\tau}_{\mathrm{A},1}^{\mathrm{adj}}$ | −.0004 | .0824 | .0844 | .960 | −.0001 | .0513 | .0527 | .956 |
| $\widehat{\tau}_{\mathrm{A},2}^{\mathrm{adj}}$ | −.0004 | .0824 | .0844 | .960 | −.0001 | .0513 | .0527 | .956 |
| $\widehat{\tau}_{\mathrm{A},1}^{\mathrm{acv}}$ | −.0004 | .0824 | .0848 | .960 | −.0001 | .0513 | .0528 | .956 |
| $\widehat{\tau}_{\mathrm{A},2}^{\mathrm{acv}}$ | −.0004 | .0824 | .0848 | .960 | −.0001 | .0513 | .0528 | .956 |

Web Table S4: Results from simulation study IV. ESE: empirical standard error; ASE: average standard error; ECP: empirical coverage percentage of the 95% confidence interval. ASEs are from the complete two-way (CTW) variance estimator.

| $\lambda(1,0)$ | | | | | | | | |
|---|---|---|---|---|---|---|---|---|
| | $N=200$ | | | | $N=500$ | | | |
| Estimator | Bias | ESE | ASE | ECP | Bias | ESE | ASE | ECP |
| $\widehat{\lambda}_{\rm I}$ | −.0005 | .0189 | .0188 | .952 | −.0003 | .0120 | .0121 | .945 |
| $\widehat{\lambda}_{\rm I}^{\rm adj}$ | −.0006 | .0190 | .0188 | .947 | −.0003 | .0120 | .0120 | .948 |
| $\widehat{\lambda}_{\rm I}^{\rm acv}$ | −.0007 | .0190 | .0188 | .944 | −.0003 | .0119 | .0120 | .948 |
| $\widehat{\lambda}_{\rm A,1}^{\rm adj}$ | −.0007 | .0192 | .0202 | .967 | −.0003 | .0120 | .0125 | .957 |
| $\widehat{\lambda}_{\rm A,2}^{\rm adj}$ | −.0006 | .0192 | .0202 | .969 | −.0003 | .0120 | .0125 | .955 |
| $\widehat{\lambda}_{\rm A,1}^{\rm acv}$ | −.0006 | .0190 | .0203 | .969 | −.0003 | .0119 | .0125 | .955 |
| $\widehat{\lambda}_{\rm A,2}^{\rm acv}$ | −.0006 | .0190 | .0203 | .969 | −.0003 | .0119 | .0125 | .955 |
| $\lambda(0,1)$ | | | | | | | | |
| | $N=200$ | | | | $N=500$ | | | |
| Estimator | Bias | ESE | ASE | ECP | Bias | ESE | ASE | ECP |
| $\widehat{\lambda}_{\rm I}$ | .0005 | .0189 | .0188 | .952 | .0003 | .0120 | .0121 | .945 |
| $\widehat{\lambda}_{\rm I}^{\rm adj}$ | .0006 | .0190 | .0188 | .947 | .0003 | .0120 | .0120 | .948 |
| $\widehat{\lambda}_{\rm I}^{\rm acv}$ | .0007 | .0190 | .0188 | .944 | .0003 | .0119 | .0120 | .948 |
| $\widehat{\lambda}_{\rm A,1}^{\rm adj}$ | .0006 | .0192 | .0202 | .969 | .0003 | .0120 | .0125 | .955 |
| $\widehat{\lambda}_{\rm A,2}^{\rm adj}$ | .0007 | .0192 | .0202 | .967 | .0003 | .0120 | .0125 | .957 |
| $\widehat{\lambda}_{\rm A,1}^{\rm acv}$ | .0006 | .0190 | .0203 | .969 | .0003 | .0119 | .0125 | .955 |
| $\widehat{\lambda}_{\rm A,2}^{\rm acv}$ | .0006 | .0190 | .0203 | .969 | .0003 | .0119 | .0125 | .955 |
| $\tau(1)$ | | | | | | | | |
| | $N=200$ | | | | $N=500$ | | | |
| Method | Bias | ESE | ASE | ECP | Bias | ESE | ASE | ECP |
| $\widehat{\tau}_{\rm I}$ | −.0010 | .0378 | .0380 | .954 | −.0005 | .0239 | .0242 | .945 |
| $\widehat{\tau}_{\rm I}^{\rm adj}$ | −.0013 | .0380 | .0379 | .947 | −.0005 | .0239 | .0241 | .948 |
| $\widehat{\tau}_{\rm I}^{\rm acv}$ | −.0013 | .0380 | .0379 | .948 | −.0005 | .0239 | .0241 | .948 |
| $\widehat{\tau}_{\rm P}$ | −.0010 | .0378 | .0367 | .945 | −.0005 | .0239 | .0239 | .942 |
| $\widehat{\tau}_{\rm P}^{\rm acv}$ | −.0013 | .0380 | .0365 | .940 | −.0005 | .0239 | .0238 | .946 |
| $\widehat{\tau}_{\rm P}^{\rm int}$ | −.0010 | .0378 | .0367 | .945 | −.0005 | .0239 | .0239 | .942 |
| $\widehat{\tau}_{\rm P}^{\rm adj}$ | −.0013 | .0380 | .0365 | .939 | −.0005 | .0239 | .0238 | .946 |
| $\widehat{\tau}_{\rm A,1}^{\rm adj}$ | −.0013 | .0380 | .0396 | .960 | −.0005 | .0239 | .0247 | .954 |
| $\widehat{\tau}_{\rm A,2}^{\rm adj}$ | −.0013 | .0380 | .0396 | .960 | −.0005 | .0239 | .0247 | .954 |
| $\widehat{\tau}_{\rm A,1}^{\rm acv}$ | −.0013 | .0380 | .0400 | .960 | −.0005 | .0239 | .0248 | .954 |
| $\widehat{\tau}_{\rm A,2}^{\rm acv}$ | −.0013 | .0380 | .0400 | .960 | −.0005 | .0239 | .0248 | .954 |

Web Table S5: Results from simulation study V under the setting in simulation study I with sample size $N = 200$. ESE: empirical standard error; ASE: average standard error; ECP: empirical coverage percentage of the 95% confidence interval. HR: the heteroskedasticity-robust variance estimator; CR: the cluster-robust variance estimator; TW: the two-way clustering variance estimator; CTW: the complete two-way clustering variance estimator.

| $\lambda(1,0)$ | | | | | | | | | |
|---|---|---|---|---|---|---|---|---|---|
| | | HR | | CR | | TW | | CTW | |
| Estimator | ESE | ASE | ECP | ASE | ECP | ASE | ECP | ASE | ECP |
| $\widehat{\lambda}_{\mathrm{I}}$ | .0411 | .0061 | .233 | .0310 | .852 | .0404 | .951 | .0401 | .950 |
| $\widehat{\lambda}_{\mathrm{I}}^{\mathrm{adj}}$ | .0353 | .0060 | .230 | .0250 | .834 | .0345 | .956 | .0342 | .952 |
| $\widehat{\lambda}_{\mathrm{I}}^{\mathrm{acv}}$ | .0352 | .0057 | .228 | .0250 | .835 | .0345 | .955 | .0342 | .953 |
| $\widehat{\lambda}_{\mathrm{A},1}^{\mathrm{adj}}$ | .0375 | .0238 | .788 | – | – | .0358 | .948 | .0358 | .948 |
| $\widehat{\lambda}_{\mathrm{A},2}^{\mathrm{adj}}$ | .0369 | .0238 | .793 | – | – | .0358 | .956 | .0358 | .956 |
| $\widehat{\lambda}_{\mathrm{A},1}^{\mathrm{acv}}$ | .0353 | .0249 | .839 | – | – | .0373 | .978 | .0377 | .977 |
| $\widehat{\lambda}_{\mathrm{A},2}^{\mathrm{acv}}$ | .0353 | .0249 | .839 | – | – | .0373 | .978 | .0376 | .978 |

| $\lambda(0,1)$ | | | | | | | | | |
|---|---|---|---|---|---|---|---|---|---|
| | | HR | | CR | | TW | | CTW | |
| Estimator | ESE | ASE | ECP | ASE | ECP | ASE | ECP | ASE | ECP |
| $\widehat{\lambda}_{\mathrm{I}}$ | .0411 | .0061 | .233 | .0262 | .777 | .0404 | .951 | .0401 | .950 |
| $\widehat{\lambda}_{\mathrm{I}}^{\mathrm{adj}}$ | .0353 | .0060 | .230 | .0241 | .821 | .0345 | .956 | .0342 | .952 |
| $\widehat{\lambda}_{\mathrm{I}}^{\mathrm{acv}}$ | .0352 | .0057 | .228 | .0241 | .820 | .0345 | .955 | .0342 | .953 |
| $\widehat{\lambda}_{\mathrm{A},1}^{\mathrm{adj}}$ | .0369 | .0238 | .793 | – | – | .0358 | .956 | .0358 | .956 |
| $\widehat{\lambda}_{\mathrm{A},2}^{\mathrm{adj}}$ | .0375 | .0238 | .788 | – | – | .0358 | .948 | .0358 | .948 |
| $\widehat{\lambda}_{\mathrm{A},1}^{\mathrm{acv}}$ | .0353 | .0249 | .839 | – | – | .0373 | .978 | .0376 | .978 |
| $\widehat{\lambda}_{\mathrm{A},2}^{\mathrm{acv}}$ | .0353 | .0249 | .839 | – | – | .0373 | .978 | .0377 | .977 |

| $\tau(1)$ | | | | | | | | | |
|---|---|---|---|---|---|---|---|---|---|
| | | HR | | CR | | TW | | CTW | |
| Estimator | ESE | ASE | ECP | ASE | ECP | ASE | ECP | ASE | ECP |
| $\widehat{\tau}_{\mathrm{I}}$ | .0822 | .0087 | .165 | .0407 | .648 | .0571 | .815 | .0808 | .951 |
| $\widehat{\tau}_{\mathrm{I}}^{\mathrm{adj}}$ | .0706 | .0085 | .168 | .0348 | .643 | .0488 | .827 | .0690 | .956 |
| $\widehat{\tau}_{\mathrm{I}}^{\mathrm{acv}}$ | .0705 | .0081 | .168 | .0350 | .649 | .0491 | .831 | .0690 | .957 |
| $\widehat{\tau}_{\mathrm{P}}$ | .0822 | .0100 | .188 | .0817 | .955 | .1152 | .996 | .0802 | .950 |
| $\widehat{\tau}_{\mathrm{P}}^{\mathrm{acv}}$ | .0705 | .0096 | .192 | .0793 | .976 | .1117 | .999 | .0683 | .953 |
| $\widehat{\tau}_{\mathrm{P}}^{\mathrm{int}}$ | .0822 | .0100 | .188 | .0809 | .951 | .1139 | .995 | .0802 | .950 |
| $\widehat{\tau}_{\mathrm{P}}^{\mathrm{adj}}$ | .0705 | .0095 | .190 | .0796 | .977 | .1121 | .999 | .0683 | .953 |
| $\widehat{\tau}_{\mathrm{A},1}^{\mathrm{adj}}$ | .0706 | .0337 | .621 | – | – | .0506 | .853 | .0692 | .963 |
| $\widehat{\tau}_{\mathrm{A},2}^{\mathrm{adj}}$ | .0706 | .0337 | .621 | – | – | .0506 | .853 | .0692 | .963 |
| $\widehat{\tau}_{\mathrm{A},1}^{\mathrm{acv}}$ | .0706 | .0356 | .656 | – | – | .0533 | .878 | .0732 | .971 |
| $\widehat{\tau}_{\mathrm{A},2}^{\mathrm{acv}}$ | .0706 | .0356 | .656 | – | – | .0533 | .878 | .0732 | .971 |

Web Table S6: Results from simulation study V under the setting in simulation study II with sample size $N = 200$. ESE: empirical standard error; ASE: average standard error; ECP: empirical coverage percentage of the 95% confidence interval. HR: the heteroskedasticity-robust variance estimator; CR: the cluster-robust variance estimator; TW: the two-way clustering variance estimator; CTW: the complete two-way clustering variance estimator.

$\lambda(1,0)$

| | | HR | | CR | | TW | | CTW | |
|---|---|---|---|---|---|---|---|---|---|
| Estimator | ESE | ASE | ECP | ASE | ECP | ASE | ECP | ASE | ECP |
| $\widehat{\lambda}_{\mathrm{I}}$ | .0189 | .0043 | .332 | .0134 | .831 | .0190 | .954 | .0188 | .952 |
| $\widehat{\lambda}_{\mathrm{I}}^{\mathrm{adj}}$ | .0181 | .0044 | .371 | .0124 | .831 | .0177 | .943 | .0176 | .938 |
| $\widehat{\lambda}_{\mathrm{I}}^{\mathrm{acv}}$ | .0180 | .0043 | .361 | .0126 | .839 | .0180 | .946 | .0176 | .940 |
| $\widehat{\lambda}_{\mathrm{A},1}^{\mathrm{adj}}$ | .0183 | .0130 | .840 | – | – | .0187 | .957 | .0187 | .957 |
| $\widehat{\lambda}_{\mathrm{A},2}^{\mathrm{adj}}$ | .0187 | .0130 | .834 | – | – | .0187 | .952 | .0187 | .952 |
| $\widehat{\lambda}_{\mathrm{A},1}^{\mathrm{acv}}$ | .0181 | .0129 | .853 | – | – | .0188 | .966 | .0191 | .968 |
| $\widehat{\lambda}_{\mathrm{A},2}^{\mathrm{acv}}$ | .0181 | .0129 | .850 | – | – | .0188 | .966 | .0191 | .967 |

$\lambda(0,1)$

| | | HR | | CR | | TW | | CTW | |
|---|---|---|---|---|---|---|---|---|---|
| Estimator | ESE | ASE | ECP | ASE | ECP | ASE | ECP | ASE | ECP |
| $\widehat{\lambda}_{\mathrm{I}}$ | .0189 | .0043 | .332 | .0137 | .853 | .0190 | .954 | .0188 | .952 |
| $\widehat{\lambda}_{\mathrm{I}}^{\mathrm{adj}}$ | .0181 | .0044 | .371 | .0128 | .842 | .0177 | .943 | .0176 | .938 |
| $\widehat{\lambda}_{\mathrm{I}}^{\mathrm{acv}}$ | .0180 | .0043 | .361 | .0130 | .844 | .0180 | .946 | .0176 | .940 |
| $\widehat{\lambda}_{\mathrm{A},1}^{\mathrm{adj}}$ | .0187 | .0130 | .834 | – | – | .0187 | .952 | .0187 | .952 |
| $\widehat{\lambda}_{\mathrm{A},2}^{\mathrm{adj}}$ | .0183 | .0130 | .840 | – | – | .0187 | .957 | .0187 | .957 |
| $\widehat{\lambda}_{\mathrm{A},1}^{\mathrm{acv}}$ | .0181 | .0129 | .850 | – | – | .0188 | .966 | .0191 | .967 |
| $\widehat{\lambda}_{\mathrm{A},2}^{\mathrm{acv}}$ | .0181 | .0129 | .853 | – | – | .0188 | .966 | .0191 | .968 |

$\tau(1)$

| | | HR | | CR | | TW | | CTW | |
|---|---|---|---|---|---|---|---|---|---|
| Estimator | ESE | ASE | ECP | ASE | ECP | ASE | ECP | ASE | ECP |
| $\widehat{\tau}_{\mathrm{I}}$ | .0378 | .0061 | .242 | .0192 | .685 | .0269 | .838 | .0380 | .954 |
| $\widehat{\tau}_{\mathrm{I}}^{\mathrm{adj}}$ | .0361 | .0062 | .260 | .0179 | .672 | .0251 | .833 | .0355 | .943 |
| $\widehat{\tau}_{\mathrm{I}}^{\mathrm{acv}}$ | .0361 | .0060 | .255 | .0186 | .695 | .0261 | .858 | .0354 | .941 |
| $\widehat{\tau}_{\mathrm{P}}$ | .0378 | .0079 | .307 | .0734 | 1.000 | .1035 | 1.000 | .0366 | .945 |
| $\widehat{\tau}_{\mathrm{P}}^{\mathrm{acv}}$ | .0361 | .0079 | .336 | .0738 | 1.000 | .1041 | 1.000 | .0340 | .928 |
| $\widehat{\tau}_{\mathrm{P}}^{\mathrm{int}}$ | .0378 | .0078 | .305 | .0714 | 1.000 | .1006 | 1.000 | .0367 | .945 |
| $\widehat{\tau}_{\mathrm{P}}^{\mathrm{adj}}$ | .0361 | .0078 | .332 | .0744 | 1.000 | .1049 | 1.000 | .0339 | .927 |
| $\widehat{\tau}_{\mathrm{A},1}^{\mathrm{adj}}$ | .0361 | .0184 | .690 | – | – | .0265 | .861 | .0367 | .954 |
| $\widehat{\tau}_{\mathrm{A},2}^{\mathrm{adj}}$ | .0361 | .0184 | .690 | – | – | .0265 | .861 | .0367 | .954 |
| $\widehat{\tau}_{\mathrm{A},1}^{\mathrm{acv}}$ | .0361 | .0187 | .703 | – | – | .0271 | .871 | .0376 | .959 |
| $\widehat{\tau}_{\mathrm{A},2}^{\mathrm{acv}}$ | .0361 | .0187 | .703 | – | – | .0271 | .871 | .0376 | .959 |

Web Table S7: Results from simulation study V under the setting in simulation study II with sample size $N = 500$. ESE: empirical standard error; ASE: average standard error; ECP: empirical coverage percentage of the 95% confidence interval. HR: the heteroskedasticity-robust variance estimator; CR: the cluster-robust variance estimator; TW: the two-way clustering variance estimator; CTW: the complete two-way clustering variance estimator.

| $\lambda(1,0)$ | | | | | | | | | |
|---|---|---|---|---|---|---|---|---|---|
| | | HR | | CR | | TW | | CTW | |
| Estimator | ESE | ASE | ECP | ASE | ECP | ASE | ECP | ASE | ECP |
| $\widehat{\lambda}_{\mathrm{I}}$ | .0120 | .0017 | .215 | .0085 | .846 | .0121 | .945 | .0121 | .945 |
| $\widehat{\lambda}_{\mathrm{I}}^{\mathrm{adj}}$ | .0111 | .0017 | .226 | .0079 | .853 | .0113 | .950 | .0112 | .947 |
| $\widehat{\lambda}_{\mathrm{I}}^{\mathrm{acv}}$ | .0111 | .0017 | .223 | .0079 | .855 | .0113 | .950 | .0112 | .949 |
| $\widehat{\lambda}_{\mathrm{A},1}^{\mathrm{adj}}$ | .0114 | .0080 | .849 | – | – | .0115 | .956 | .0115 | .956 |
| $\widehat{\lambda}_{\mathrm{A},2}^{\mathrm{adj}}$ | .0113 | .0080 | .846 | – | – | .0115 | .953 | .0115 | .953 |
| $\widehat{\lambda}_{\mathrm{A},1}^{\mathrm{acv}}$ | .0111 | .0081 | .868 | – | – | .0116 | .959 | .0117 | .961 |
| $\widehat{\lambda}_{\mathrm{A},2}^{\mathrm{acv}}$ | .0111 | .0081 | .864 | – | – | .0116 | .959 | .0117 | .961 |
| $\lambda(0,1)$ | | | | | | | | | |
| | | HR | | CR | | TW | | CTW | |
| Estimator | ESE | ASE | ECP | ASE | ECP | ASE | ECP | ASE | ECP |
| $\widehat{\lambda}_{\mathrm{I}}$ | .0120 | .0017 | .215 | .0087 | .854 | .0121 | .945 | .0121 | .945 |
| $\widehat{\lambda}_{\mathrm{I}}^{\mathrm{adj}}$ | .0111 | .0017 | .226 | .0081 | .871 | .0113 | .950 | .0112 | .947 |
| $\widehat{\lambda}_{\mathrm{I}}^{\mathrm{acv}}$ | .0111 | .0017 | .223 | .0082 | .873 | .0113 | .950 | .0112 | .949 |
| $\widehat{\lambda}_{\mathrm{A},1}^{\mathrm{adj}}$ | .0113 | .0080 | .846 | – | – | .0115 | .953 | .0115 | .953 |
| $\widehat{\lambda}_{\mathrm{A},2}^{\mathrm{adj}}$ | .0114 | .0080 | .849 | – | – | .0115 | .956 | .0115 | .956 |
| $\widehat{\lambda}_{\mathrm{A},1}^{\mathrm{acv}}$ | .0111 | .0081 | .864 | – | – | .0116 | .959 | .0117 | .961 |
| $\widehat{\lambda}_{\mathrm{A},2}^{\mathrm{acv}}$ | .0111 | .0081 | .868 | – | – | .0116 | .959 | .0117 | .961 |
| $\tau(1)$ | | | | | | | | | |
| | | HR | | CR | | TW | | CTW | |
| Estimator | ESE | ASE | ECP | ASE | ECP | ASE | ECP | ASE | ECP |
| $\widehat{\tau}_{\mathrm{I}}$ | .0239 | .0024 | .151 | .0121 | .688 | .0171 | .853 | .0242 | .945 |
| $\widehat{\tau}_{\mathrm{I}}^{\mathrm{adj}}$ | .0222 | .0024 | .149 | .0113 | .690 | .0159 | .861 | .0225 | .950 |
| $\widehat{\tau}_{\mathrm{I}}^{\mathrm{acv}}$ | .0222 | .0024 | .149 | .0115 | .697 | .0162 | .866 | .0225 | .950 |
| $\widehat{\tau}_{\mathrm{P}}$ | .0239 | .0031 | .199 | .0464 | 1.000 | .0655 | 1.000 | .0239 | .942 |
| $\widehat{\tau}_{\mathrm{P}}^{\mathrm{acv}}$ | .0222 | .0031 | .202 | .0464 | 1.000 | .0655 | 1.000 | .0222 | .945 |
| $\widehat{\tau}_{\mathrm{P}}^{\mathrm{int}}$ | .0239 | .0031 | .197 | .0459 | 1.000 | .0648 | 1.000 | .0239 | .942 |
| $\widehat{\tau}_{\mathrm{P}}^{\mathrm{adj}}$ | .0222 | .0031 | .201 | .0465 | 1.000 | .0657 | 1.000 | .0222 | .945 |
| $\widehat{\tau}_{\mathrm{A},1}^{\mathrm{adj}}$ | .0222 | .0113 | .690 | – | – | .0163 | .871 | .0228 | .950 |
| $\widehat{\tau}_{\mathrm{A},2}^{\mathrm{adj}}$ | .0222 | .0113 | .690 | – | – | .0163 | .871 | .0228 | .950 |
| $\widehat{\tau}_{\mathrm{A},1}^{\mathrm{acv}}$ | .0222 | .0115 | .698 | – | – | .0166 | .879 | .0232 | .958 |
| $\widehat{\tau}_{\mathrm{A},2}^{\mathrm{acv}}$ | .0222 | .0115 | .698 | – | – | .0166 | .879 | .0232 | .958 |

Web Table S8: Results from simulation study I for the V-type GCE estimand. ESE: empirical standard error; ASE: average standard error; ECP: empirical coverage percentage of the 95% confidence interval. ASEs are from the complete two-way (CTW) variance estimator.

| $\lambda(1,0)$ | | | | | | | | |
|---|---|---|---|---|---|---|---|---|
| | $N=200$ | | | | $N=500$ | | | |
| Estimator | Bias | ESE | ASE | ECP | Bias | ESE | ASE | ECP |
| $\widehat{\lambda}_{\mathrm{I}}$ | .0001 | .0411 | .0401 | .949 | −.0001 | .0256 | .0256 | .951 |
| $\widehat{\lambda}_{\mathrm{I}}^{\mathrm{adj}}$ | −.0001 | .0353 | .0342 | .953 | −.0005 | .0221 | .0218 | .948 |
| $\widehat{\lambda}_{\mathrm{I}}^{\mathrm{acv}}$ | −.0001 | .0352 | .0342 | .954 | −.0005 | .0221 | .0218 | .947 |
| $\widehat{\lambda}_{\mathrm{A},1}^{\mathrm{adj}}$ | .0007 | .0375 | .0358 | .948 | −.0001 | .0237 | .0221 | .934 |
| $\widehat{\lambda}_{\mathrm{A},2}^{\mathrm{adj}}$ | −.0008 | .0369 | .0358 | .956 | −.0009 | .0229 | .0221 | .950 |
| $\widehat{\lambda}_{\mathrm{A},1}^{\mathrm{acv}}$ | −.0001 | .0353 | .0377 | .977 | −.0005 | .0221 | .0233 | .966 |
| $\widehat{\lambda}_{\mathrm{A},2}^{\mathrm{acv}}$ | −.0001 | .0353 | .0376 | .978 | −.0005 | .0221 | .0233 | .964 |

| $\lambda(0,1)$ | | | | | | | | |
|---|---|---|---|---|---|---|---|---|
| | $N=200$ | | | | $N=500$ | | | |
| Estimator | Bias | ESE | ASE | ECP | Bias | ESE | ASE | ECP |
| $\widehat{\lambda}_{\mathrm{I}}$ | −.0001 | .0411 | .0401 | .949 | .0001 | .0256 | .0256 | .951 |
| $\widehat{\lambda}_{\mathrm{I}}^{\mathrm{adj}}$ | .0001 | .0353 | .0342 | .953 | .0005 | .0221 | .0218 | .948 |
| $\widehat{\lambda}_{\mathrm{I}}^{\mathrm{acv}}$ | .0001 | .0352 | .0342 | .954 | .0005 | .0221 | .0218 | .947 |
| $\widehat{\lambda}_{\mathrm{A},1}^{\mathrm{adj}}$ | .0008 | .0369 | .0358 | .956 | .0009 | .0229 | .0221 | .950 |
| $\widehat{\lambda}_{\mathrm{A},2}^{\mathrm{adj}}$ | −.0007 | .0375 | .0358 | .948 | .0001 | .0237 | .0221 | .934 |
| $\widehat{\lambda}_{\mathrm{A},1}^{\mathrm{acv}}$ | .0001 | .0353 | .0376 | .978 | .0005 | .0221 | .0233 | .964 |
| $\widehat{\lambda}_{\mathrm{A},2}^{\mathrm{acv}}$ | .0001 | .0353 | .0377 | .977 | .0005 | .0221 | .0233 | .966 |

| $\tau(1)$ | | | | | | | | |
|---|---|---|---|---|---|---|---|---|
| | $N=200$ | | | | $N=500$ | | | |
| Method | Bias | ESE | ASE | ECP | Bias | ESE | ASE | ECP |
| $\widehat{\tau}_{\mathrm{I}}$ | .0002 | .0822 | .0808 | .952 | −.0002 | .0512 | .0512 | .952 |
| $\widehat{\tau}_{\mathrm{I}}^{\mathrm{adj}}$ | −.0001 | .0706 | .0690 | .955 | −.0010 | .0443 | .0437 | .949 |
| $\widehat{\tau}_{\mathrm{I}}^{\mathrm{acv}}$ | −.0001 | .0705 | .0690 | .957 | −.0009 | .0443 | .0437 | .947 |
| $\widehat{\tau}_{\mathrm{P}}$ | .0002 | .0822 | .0802 | .949 | −.0002 | .0512 | .0512 | .951 |
| $\widehat{\tau}_{\mathrm{P}}^{\mathrm{acv}}$ | −.0001 | .0705 | .0683 | .953 | −.0009 | .0443 | .0436 | .947 |
| $\widehat{\tau}_{\mathrm{P}}^{\mathrm{int}}$ | .0002 | .0822 | .0802 | .949 | −.0002 | .0512 | .0512 | .951 |
| $\widehat{\tau}_{\mathrm{P}}^{\mathrm{adj}}$ | −.0001 | .0705 | .0683 | .953 | −.0009 | .0443 | .0436 | .947 |
| $\widehat{\tau}_{\mathrm{A},1}^{\mathrm{adj}}$ | −.0001 | .0706 | .0692 | .962 | −.0010 | .0443 | .0430 | .947 |
| $\widehat{\tau}_{\mathrm{A},2}^{\mathrm{adj}}$ | −.0001 | .0706 | .0692 | .962 | −.0010 | .0443 | .0430 | .947 |
| $\widehat{\tau}_{\mathrm{A},1}^{\mathrm{acv}}$ | −.0001 | .0706 | .0732 | .971 | −.0009 | .0443 | .0454 | .960 |
| $\widehat{\tau}_{\mathrm{A},2}^{\mathrm{acv}}$ | −.0001 | .0706 | .0732 | .971 | −.0009 | .0443 | .0454 | .960 |

Web Table S9: Results from simulation study II for the V-type GCE estimand. ESE: empirical standard error; ASE: average standard error; ECP: empirical coverage percentage of the 95% confidence interval. ASEs are from the complete two-way (CTW) variance estimator.

| $\lambda(1,0)$ | | | | | | | | |
|---|---|---|---|---|---|---|---|---|
| | $N=200$ | | | | $N=500$ | | | |
| Estimator | Bias | ESE | ASE | ECP | Bias | ESE | ASE | ECP |
| $\widehat{\lambda}_{\mathrm{I}}$ | −.0004 | .0189 | .0188 | .952 | −.0002 | .0120 | .0121 | .944 |
| $\widehat{\lambda}_{\mathrm{I}}^{\mathrm{adj}}$ | −.0006 | .0181 | .0176 | .939 | −.0003 | .0110 | .0112 | .948 |
| $\widehat{\lambda}_{\mathrm{I}}^{\mathrm{acv}}$ | −.0006 | .0180 | .0176 | .938 | −.0003 | .0111 | .0112 | .948 |
| $\widehat{\lambda}_{\mathrm{A,1}}^{\mathrm{adj}}$ | −.0006 | .0183 | .0187 | .957 | −.0003 | .0114 | .0115 | .955 |
| $\widehat{\lambda}_{\mathrm{A,2}}^{\mathrm{adj}}$ | −.0006 | .0187 | .0187 | .953 | −.0004 | .0113 | .0115 | .953 |
| $\widehat{\lambda}_{\mathrm{A,1}}^{\mathrm{acv}}$ | −.0006 | .0181 | .0191 | .967 | −.0003 | .0111 | .0117 | .961 |
| $\widehat{\lambda}_{\mathrm{A,2}}^{\mathrm{acv}}$ | −.0006 | .0181 | .0191 | .967 | −.0003 | .0111 | .0117 | .961 |

| $\lambda(0,1)$ | | | | | | | | |
|---|---|---|---|---|---|---|---|---|
| | $N=200$ | | | | $N=500$ | | | |
| Estimator | Bias | ESE | ASE | ECP | Bias | ESE | ASE | ECP |
| $\widehat{\lambda}_{\mathrm{I}}$ | .0004 | .0189 | .0188 | .952 | .0002 | .0120 | .0121 | .944 |
| $\widehat{\lambda}_{\mathrm{I}}^{\mathrm{adj}}$ | .0006 | .0181 | .0176 | .939 | .0003 | .0110 | .0112 | .948 |
| $\widehat{\lambda}_{\mathrm{I}}^{\mathrm{acv}}$ | .0006 | .0180 | .0176 | .938 | .0003 | .0111 | .0112 | .948 |
| $\widehat{\lambda}_{\mathrm{A,1}}^{\mathrm{adj}}$ | .0006 | .0187 | .0187 | .953 | .0004 | .0113 | .0115 | .953 |
| $\widehat{\lambda}_{\mathrm{A,2}}^{\mathrm{adj}}$ | .0006 | .0183 | .0187 | .957 | .0003 | .0114 | .0115 | .955 |
| $\widehat{\lambda}_{\mathrm{A,1}}^{\mathrm{acv}}$ | .0006 | .0181 | .0191 | .967 | .0003 | .0111 | .0117 | .961 |
| $\widehat{\lambda}_{\mathrm{A,2}}^{\mathrm{acv}}$ | .0006 | .0181 | .0191 | .967 | .0003 | .0111 | .0117 | .961 |

| $\tau(1)$ | | | | | | | | |
|---|---|---|---|---|---|---|---|---|
| | $N=200$ | | | | $N=500$ | | | |
| Method | Bias | ESE | ASE | ECP | Bias | ESE | ASE | ECP |
| $\widehat{\tau}_{\mathrm{I}}$ | −.0007 | .0378 | .0380 | .955 | −.0004 | .0239 | .0242 | .945 |
| $\widehat{\tau}_{\mathrm{I}}^{\mathrm{adj}}$ | −.0012 | .0361 | .0355 | .944 | −.0007 | .0221 | .0225 | .949 |
| $\widehat{\tau}_{\mathrm{I}}^{\mathrm{acv}}$ | −.0011 | .0361 | .0354 | .941 | −.0006 | .0222 | .0225 | .949 |
| $\widehat{\tau}_{\mathrm{P}}$ | −.0007 | .0378 | .0366 | .942 | −.0004 | .0239 | .0239 | .942 |
| $\widehat{\tau}_{\mathrm{P}}^{\mathrm{acv}}$ | −.0011 | .0361 | .0340 | .926 | −.0006 | .0222 | .0222 | .947 |
| $\widehat{\tau}_{\mathrm{P}}^{\mathrm{int}}$ | −.0007 | .0378 | .0367 | .942 | −.0004 | .0239 | .0239 | .942 |
| $\widehat{\tau}_{\mathrm{P}}^{\mathrm{adj}}$ | −.0011 | .0361 | .0339 | .925 | −.0006 | .0222 | .0222 | .947 |
| $\widehat{\tau}_{\mathrm{A,1}}^{\mathrm{adj}}$ | −.0012 | .0361 | .0367 | .954 | −.0007 | .0222 | .0228 | .949 |
| $\widehat{\tau}_{\mathrm{A,2}}^{\mathrm{adj}}$ | −.0012 | .0361 | .0367 | .954 | −.0007 | .0222 | .0228 | .949 |
| $\widehat{\tau}_{\mathrm{A,1}}^{\mathrm{acv}}$ | −.0012 | .0361 | .0376 | .959 | −.0007 | .0222 | .0232 | .958 |
| $\widehat{\tau}_{\mathrm{A,2}}^{\mathrm{acv}}$ | −.0012 | .0361 | .0376 | .959 | −.0007 | .0222 | .0232 | .958 |

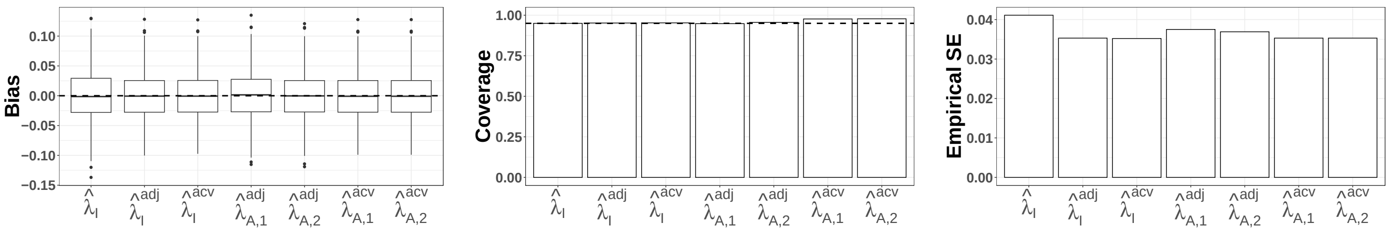


(a) Simulation study I: univariate outcome.

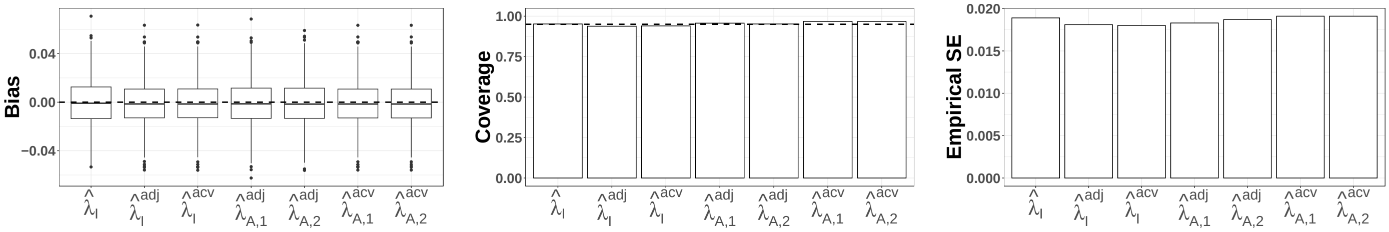


(b) Simulation study II: composite outcomes.

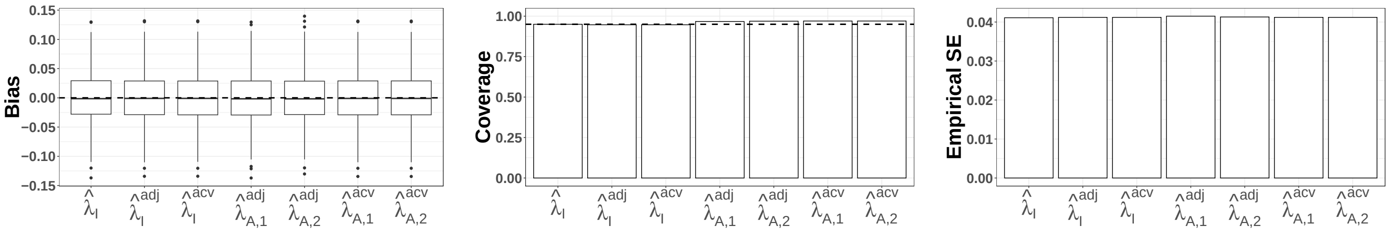


(c) Simulation study III: unrelated covariates.

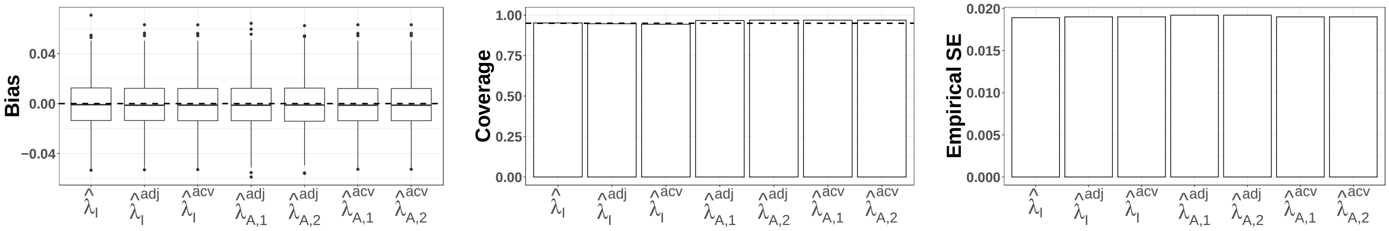


(d) Simulation study IV: noisy covariates.

Web Figure S1: Bias, coverage percentages of 95% CIs, and empirical standard errors for $\widehat{\lambda}(1, 0)$ from simulation studies I - IV. The number of units $N = 200$.

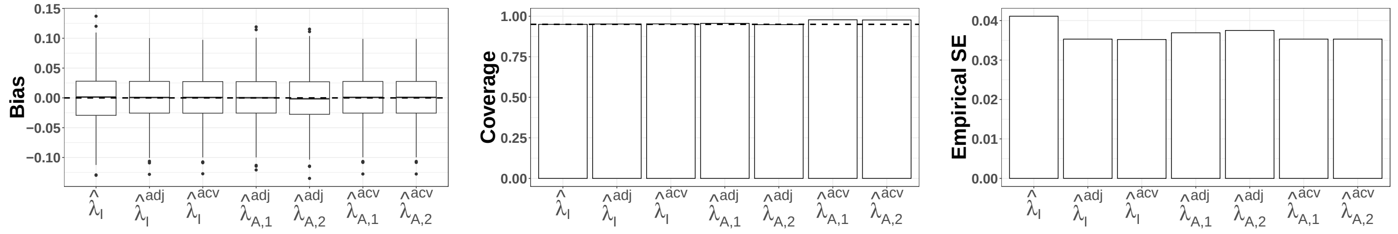


(a) Simulation study I: univariate outcome.

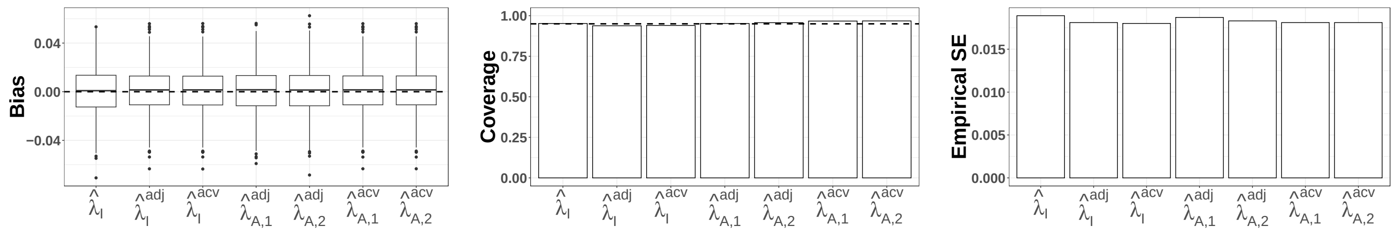


(b) Simulation study II: composite outcomes.

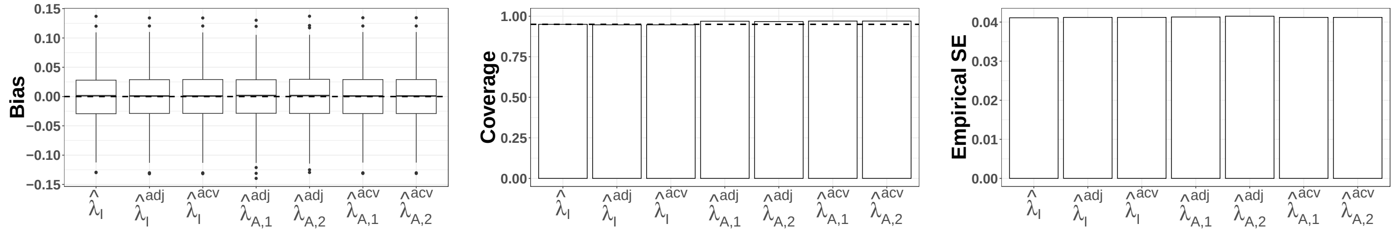


(c) Simulation study III: unrelated covariates.

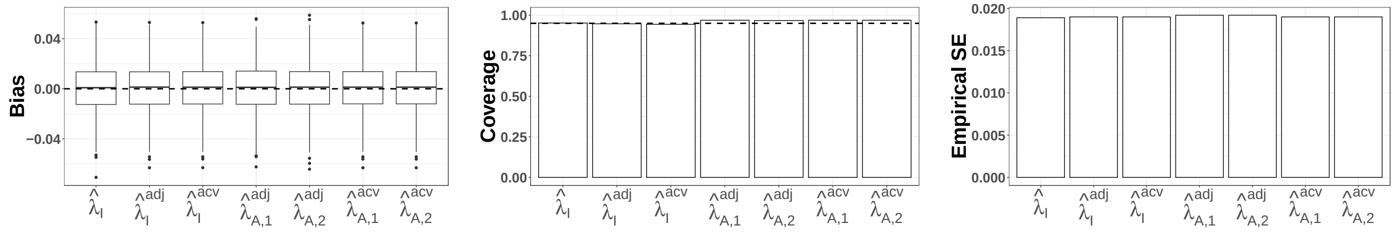


(d) Simulation study IV: noisy covariates.

Web Figure S2: Bias, coverage percentages of 95% CIs, and empirical standard errors for $\widehat{\lambda}(0,1)$ from simulation studies I - IV. The number of units $N = 200$.

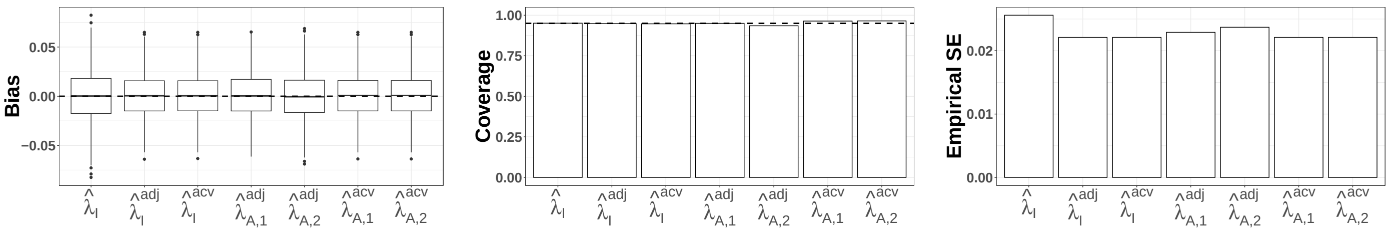


(a) Simulation study I: univariate outcome.

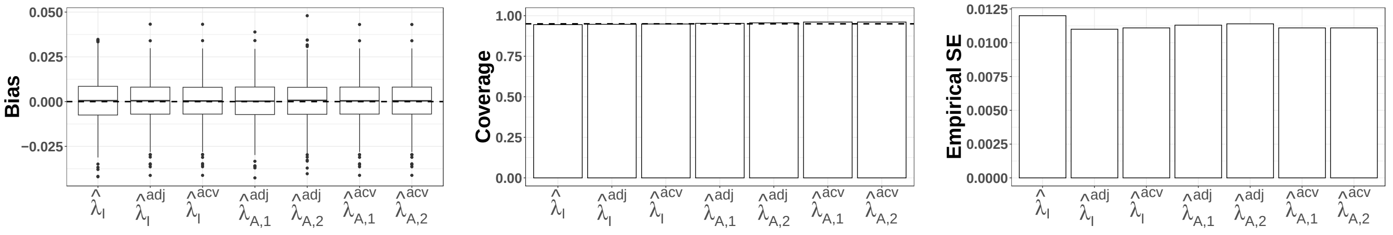


(b) Simulation study II: composite outcomes.

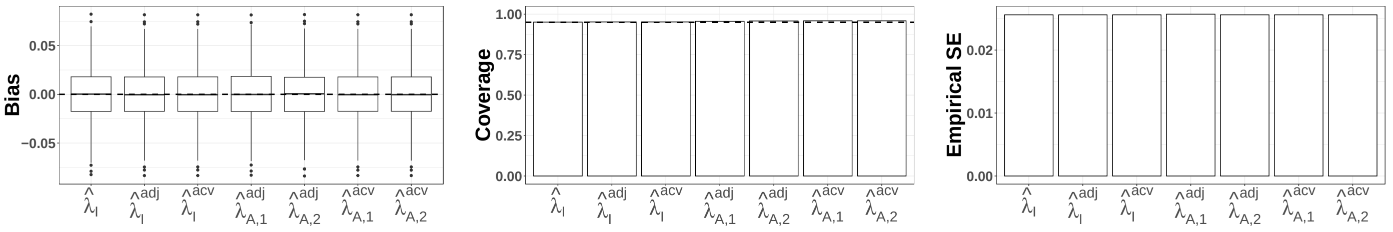


(c) Simulation study III: unrelated covariates.

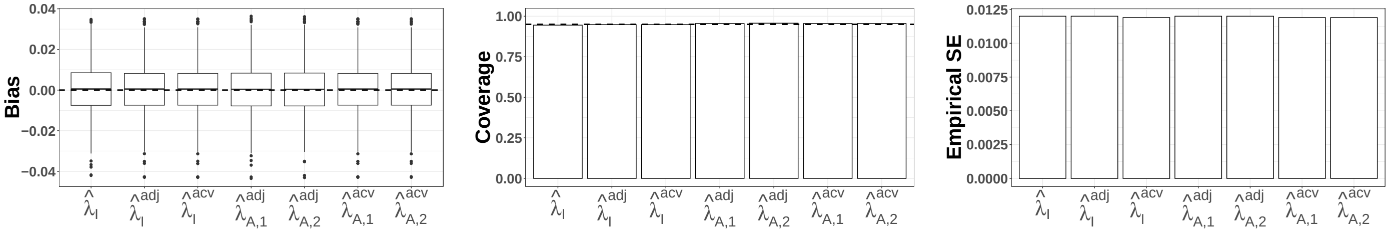


(d) Simulation study IV: noisy covariates.

Web Figure S3: Bias, coverage percentages of 95% CIs, and empirical standard errors for $\widehat{\lambda}(0,1)$ from simulation studies I - IV. The number of units $N = 500$.

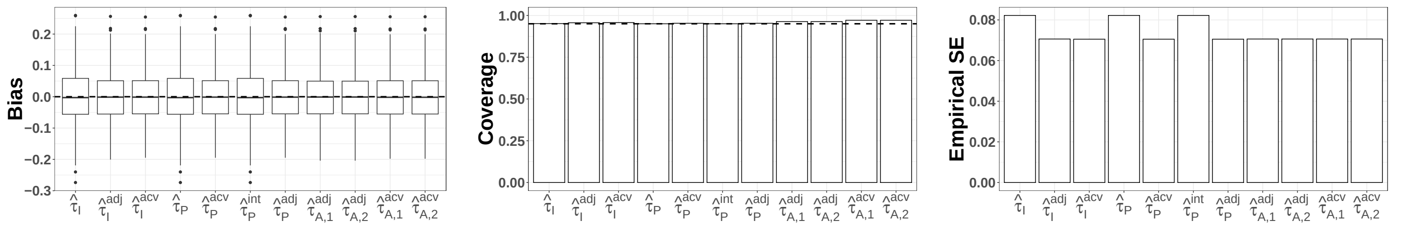


(a) Simulation study I: univariate outcome.

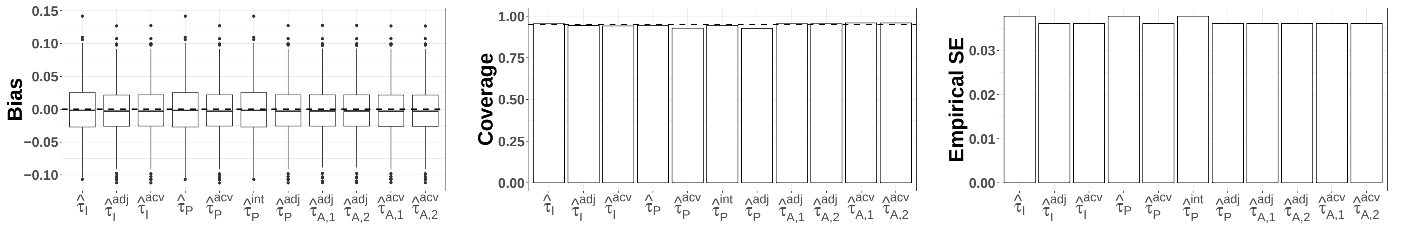


(b) Simulation study II: composite outcomes.

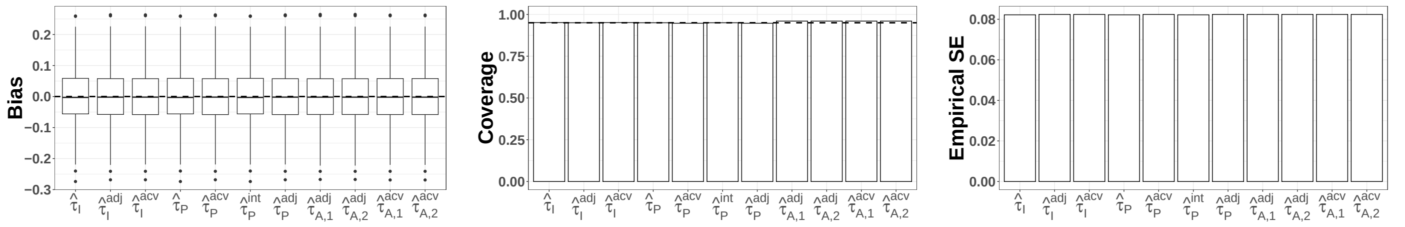


(c) Simulation study III: unrelated covariates.

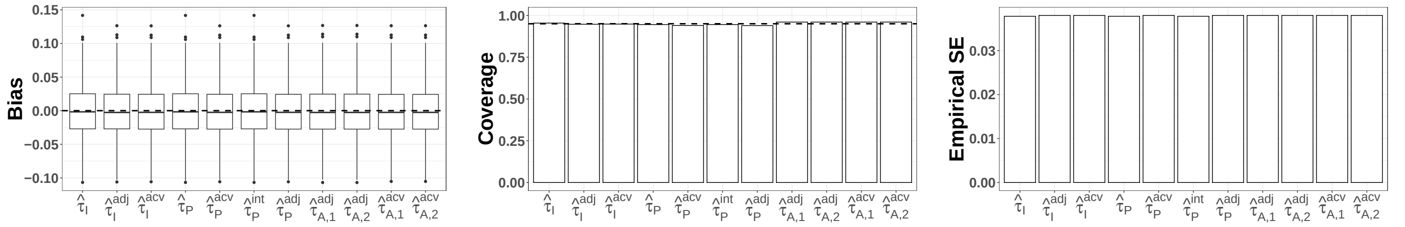


(d) Simulation study IV: noisy covariates.

Web Figure S4: Bias, coverage percentages of 95% CIs, and empirical standard errors for $\widehat{\tau}(1)$ from simulation studies I - IV. The number of units $N = 200$.

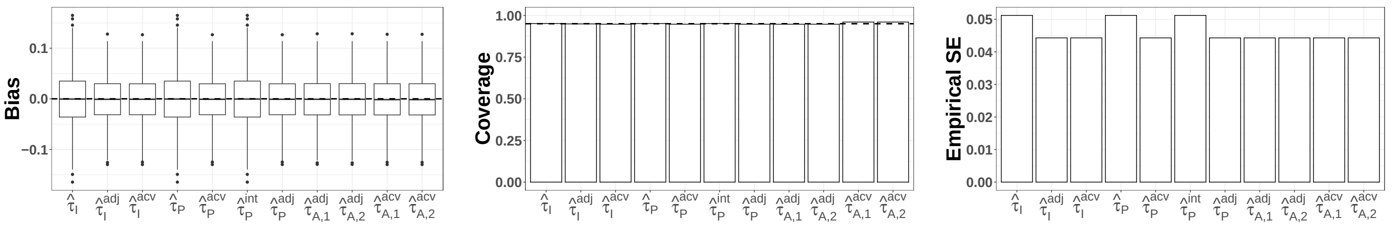


(a) Simulation study I: univariate outcome.

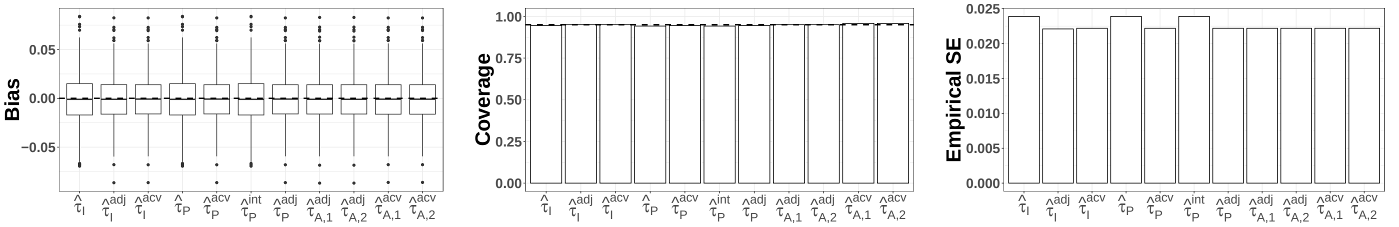


(b) Simulation study II: composite outcomes.

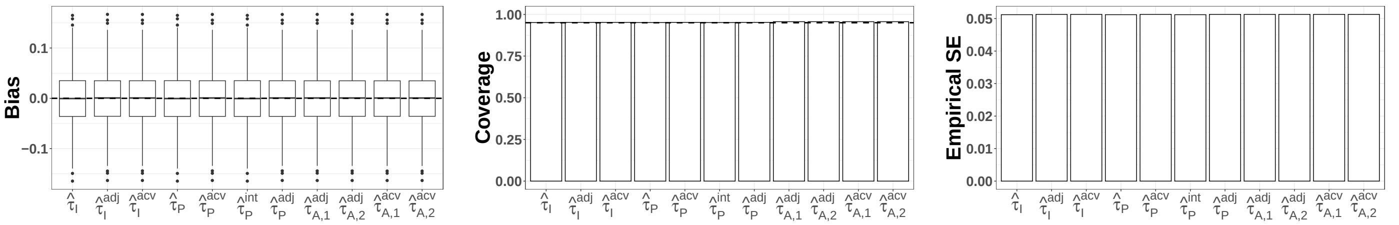


(c) Simulation study III: unrelated covariates.

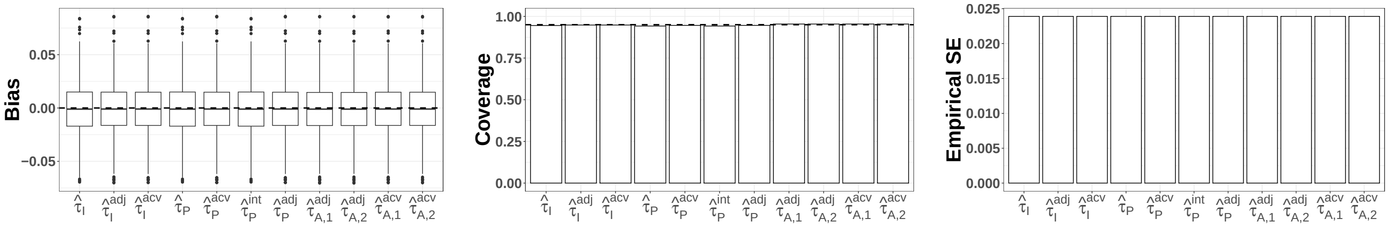


(d) Simulation study IV: noisy covariates.

Web Figure S5: Bias, coverage percentages of 95% CIs, and empirical standard errors for $\widehat{\tau}(1)$ from simulation studies I - IV. The number of units $N = 500$.
